# Supplementary material for: SAS-Prompt: Large Language Models as Numerical Optimizers for Robot Self-Improvement
Source: arXiv:2504.20459 source file (2025-04-29)
Supplement: Supplementary file 1 [file new_appendix.tex]

<q> Hit the ball as far right as possible while still landing it on the table!
Example 1:
a:0.75 b:0.75 c:0.75 d:0.75 e:1.1 f:0.75 g:0.75 h:0.75 

Landing Position:
  x      y      z      On Table
-0.2978 0.4482 0.0089   True

Paddle Motion and Ball Motion:
      paddle x  paddle y  paddle z  ball x  ball y  ball z
time                                                      
10      0.2302   -1.1065    0.4025  0.3204  0.5031  0.3763
12      0.2863   -1.1662    0.4059  0.3167  0.2917  0.3326
14      0.3394   -1.2308    0.4023  0.3203  0.0597  0.2785
16      0.3886   -1.2906    0.3897  0.2966 -0.1054  0.2222
18      0.4252   -1.3388    0.3706  0.2923 -0.3175  0.1407
20      0.4412   -1.3756    0.3473  0.2731 -0.4964  0.0613
22      0.4352   -1.4007    0.3235  0.2612 -0.6774  0.0186
24      0.4093   -1.4065    0.2994  0.2401 -0.8064  0.1655
26      0.3692   -1.3829    0.2741  0.2215 -0.9491  0.2072
28      0.3204   -1.3365    0.2549  0.2056 -1.0814  0.2411
30      0.2794   -1.2750    0.2562  0.1931 -1.2287  0.2695
32      0.2436   -1.2103    0.2735  0.1774 -1.3222  0.2769
34      0.2052   -1.1427    0.2891  0.1115 -0.9736  0.3429
36      0.1709   -1.0679    0.3111  0.0746 -0.8256  0.3610
38      0.1267   -1.0070    0.3332  0.0244 -0.6712  0.3593
40      0.0752   -0.9478    0.3548 -0.0072 -0.5266  0.3407
42      0.0160   -0.8958    0.3755 -0.0508 -0.3876  0.3178
44     -0.0495   -0.8515    0.3952 -0.0920 -0.2428  0.2859
46     -0.1201   -0.8159    0.4137 -0.1365 -0.1077  0.2295
48     -0.1943   -0.7895    0.4308 -0.1756  0.0188  0.1659
50     -0.2684   -0.7597    0.4240 -0.2118  0.1519  0.1269
52     -0.3450   -0.7363    0.4149 -0.2454  0.2761  0.0737
54     -0.4233   -0.7209    0.4054 -0.2764  0.3937  0.0038

Example 2:
a:0.9 b:0.9 c:0.9 d:0.9 e:0.8 f:0.9 g:0.9 h:0.9 

Landing Position:
  x      y      z      On Table
-0.2155 0.9221 0.0056   True

Paddle Motion and Ball Motion:
      paddle x  paddle y  paddle z  ball x  ball y  ball z
time                                                      
10      0.2451   -1.1283    0.4129  0.2910  0.5318  0.3952
12      0.3000   -1.2081    0.4211  0.2852  0.3270  0.3540
14      0.3533   -1.2977    0.4184  0.2762  0.1310  0.3112
16      0.4042   -1.3786    0.3993  0.2579 -0.0736  0.2448
18      0.4369   -1.4408    0.3696  0.2354 -0.2618  0.1672
20      0.4372   -1.4800    0.3379  0.2329 -0.4544  0.0956
22      0.4131   -1.5076    0.3093  0.2152 -0.6225  0.0141
24      0.3711   -1.5017    0.2850  0.1968 -0.7651  0.1183
26      0.3203   -1.4594    0.2625  0.1799 -0.9146  0.1995
28      0.2786   -1.3870    0.2445  0.1646 -1.0481  0.2330
30      0.2351   -1.3095    0.2442  0.1519 -1.1824  0.2654
32      0.1888   -1.2204    0.2703  0.1317 -1.3179  0.2851
34      0.1496   -1.1468    0.2925  0.0868 -0.9634  0.3631
36      0.1114   -1.0649    0.3089  0.0661 -0.8244  0.3950
38      0.0794   -0.9914    0.3289  0.0350 -0.6192  0.4198
40      0.0332   -0.9275    0.3476  0.0038 -0.4560  0.4371
42     -0.0225   -0.8723    0.3655 -0.0234 -0.2885  0.4372
44     -0.0863   -0.8278    0.3822 -0.0517 -0.1260  0.4177
46     -0.1555   -0.7940    0.3938 -0.0823  0.0320  0.3916
48     -0.2252   -0.7593    0.3758 -0.1101  0.1889  0.3501
50     -0.2981   -0.7356    0.3574 -0.1286  0.3435  0.2932
52     -0.3726   -0.7232    0.3387 -0.1440  0.4966  0.2238
54     -0.4470   -0.7222    0.3197 -0.1840  0.6407  0.1549
56     -0.5211   -0.7305    0.3192 -0.1953  0.7831  0.0589
58     -0.5938   -0.7483    0.3330 -0.2155  0.9221  0.0056

Example 3:
a:0.75 b:0.75 c:0.75 d:0.75 e:0.75 f:0.75 g:1.1 h:0.75 

Landing Position:
  x      y      z      On Table
-0.1632 0.4586 -0.0168   True

Paddle Motion and Ball Motion:
      paddle x  paddle y  paddle z  ball x  ball y  ball z
time                                                      
10      0.2315   -1.1062    0.4136  0.3153  0.5394  0.3898
12      0.2824   -1.1674    0.4246  0.2944  0.3458  0.3437
14      0.3362   -1.2326    0.4220  0.2841  0.1355  0.2974
16      0.3866   -1.2909    0.4026  0.2702 -0.0568  0.2312
18      0.4399   -1.3736    0.3547  0.2543 -0.2587  0.1548
20      0.4277   -1.3762    0.3323  0.2449 -0.4435  0.0681
22      0.4152   -1.4106    0.2942  0.2276 -0.6373 -0.0145
24      0.3903   -1.4258    0.2602  0.2127 -0.7758  0.1591
26      0.3403   -1.4091    0.2306  0.2024 -0.9183  0.1954
28      0.2915   -1.3647    0.2134  0.1731 -1.0880  0.2500
30      0.2576   -1.3013    0.2307  0.1513 -1.1942  0.2676
32      0.2409   -1.2365    0.2710  0.1514 -1.3352  0.2788
34      0.2083   -1.1642    0.2960  0.1208 -1.0172  0.3558
36      0.1547   -1.0960    0.3212  0.0808 -0.8779  0.3740
38      0.1199   -1.0353    0.3433  0.0644 -0.7141  0.4011
40      0.0687   -0.9773    0.3654  0.0453 -0.5208  0.4025
42      0.0099   -0.9272    0.3866  0.0075 -0.4068  0.3799
44     -0.0564   -0.8858    0.4068 -0.0044 -0.2777  0.3600
46     -0.1263   -0.8502    0.4153 -0.0386 -0.1359  0.3151
48     -0.1967   -0.8138    0.4007 -0.0697  0.0012  0.2626
50     -0.2711   -0.7857    0.3859 -0.0954  0.1363  0.1924
52     -0.3483   -0.7664    0.3708 -0.1243  0.2716  0.1112
54     -0.4272   -0.7563    0.3554 -0.1440  0.3981  0.0130

Example 4:
a:0.87 b:0.87 c:0.87 d:0.87 e:0.87 f:0.87 g:0.87 h:1.23 

Landing Position:
  x      y      z      On Table
-0.0872 0.7329 0.0464   True

Paddle Motion and Ball Motion:
      paddle x  paddle y  paddle z  ball x  ball y  ball z
time                                                      
10      0.2522   -1.1255    0.4102  0.3029  0.4947  0.3898
12      0.2540   -1.1556    0.4131  0.2920  0.2896  0.3518
14      0.3589   -1.2867    0.4128  0.2831  0.1095  0.3080
16      0.4108   -1.3604    0.3906  0.2680 -0.1030  0.2415
18      0.4628   -1.4576    0.3487  0.2572 -0.3017  0.1687
20      0.4536   -1.4560    0.3375  0.2395 -0.4644  0.0895
22      0.4302   -1.4725    0.3151  0.2307 -0.6590 -0.0023
24      0.3910   -1.4555    0.3062  0.2175 -0.7999  0.1095
26      0.3378   -1.4275    0.2650  0.1972 -0.9404  0.1994
28      0.2877   -1.3619    0.2420  0.1809 -1.0804  0.2265
30      0.2456   -1.2800    0.2437  0.1736 -1.2175  0.2598
32      0.2139   -1.2019    0.2732  0.1642 -1.3330  0.2664
34      0.1624   -1.0948    0.3144  0.1317 -0.9566  0.3738
36      0.1492   -1.0734    0.3052  0.0985 -0.8149  0.4101
38      0.1357   -1.0520    0.3052  0.0855 -0.6643  0.4386
40      0.1218   -1.0301    0.3052  0.0484 -0.4889  0.4506
42      0.1079   -1.0083    0.3052  0.0404 -0.3557  0.4442
44      0.0940   -0.9865    0.3052  0.0245 -0.2028  0.4283
46      0.0801   -0.9646    0.3052  0.0034 -0.0651  0.3885
48      0.0662   -0.9428    0.3052 -0.0056  0.0682  0.3521
50      0.0523   -0.9210    0.3052 -0.0261  0.2137  0.2951
52      0.0384   -0.8991    0.3052 -0.0518  0.3531  0.2277
54      0.0245   -0.8773    0.3052 -0.0592  0.5144  0.1251
56      0.0107   -0.8559    0.3052 -0.0751  0.6145  0.0399
58     -0.0032   -0.8532    0.3052 -0.0872  0.7329  0.0464

Example 5:
a:0.9 b:0.9 c:0.9 d:0.9 e:0.9 f:0.6 g:0.9 h:0.9 

Landing Position:
  x      y      z      On Table
-0.3773 1.2431 0.0208   True

Paddle Motion and Ball Motion:
      paddle x  paddle y  paddle z  ball x  ball y  ball z
time                                                      
10      0.2345   -1.1230    0.4103  0.2970  0.3899  0.3639
12      0.2855   -1.1915    0.4167  0.2787  0.1831  0.3180
14      0.3352   -1.2647    0.4095  0.2693 -0.0123  0.2641
16      0.3714   -1.3311    0.3827  0.2539 -0.2011  0.1995
18      0.3918   -1.3855    0.3475  0.2354 -0.3962  0.1181
20      0.4091   -1.4298    0.3131  0.2308 -0.5765  0.0358
22      0.3854   -1.4634    0.2788  0.2033 -0.7432  0.0715
24      0.3449   -1.4486    0.2623  0.1928 -0.8784  0.1916
26      0.2918   -1.4019    0.2439  0.1748 -1.0162  0.2237
28      0.2226   -1.3314    0.2379  0.1549 -1.1556  0.2523
30      0.1853   -1.2387    0.2565  0.1472 -1.2709  0.2773
32      0.1702   -1.1488    0.2812  0.0969 -0.9933  0.3520
34      0.1390   -1.0589    0.2988  0.0556 -0.7858  0.4118
36      0.0877   -0.9749    0.3182  0.0084 -0.5921  0.4479
38      0.0283   -0.8980    0.3369 -0.0174 -0.4130  0.4652
40     -0.0411   -0.8305    0.3549 -0.0630 -0.2312  0.4687
42     -0.1185   -0.7737    0.3720 -0.1012 -0.0498  0.4567
44     -0.2017   -0.7283    0.3860 -0.1324  0.1113  0.4374
46     -0.2844   -0.6817    0.3656 -0.1755  0.2859  0.4122
48     -0.3704   -0.6457    0.3450 -0.2235  0.4567  0.3682
50     -0.4579   -0.6207    0.3241 -0.2551  0.6170  0.3074
52     -0.5452   -0.6067    0.3031 -0.2857  0.7748  0.2407
54     -0.6317   -0.6021    0.2925 -0.3060  0.9394  0.1534
56     -0.7180   -0.6051    0.3047 -0.3455  1.0970  0.0557
58     -0.8008   -0.6310    0.3163 -0.3773  1.2431  0.0208

Example 6:
a:0.9 b:0.9 c:0.9 d:0.9 e:0.9 f:1.1 g:0.9 h:0.9 

Landing Position:
  x      y      z      On Table
-0.1330 0.6830 0.0013   True

Paddle Motion and Ball Motion:
      paddle x  paddle y  paddle z  ball x  ball y  ball z
time                                                      
10      0.2424   -1.1253    0.4146  0.3163  0.3433  0.3363
12      0.3248   -1.2067    0.4210  0.3123  0.1311  0.2828
14      0.3933   -1.2946    0.4125  0.2969 -0.0582  0.2218
16      0.4469   -1.3689    0.3855  0.2874 -0.2637  0.1562
18      0.4688   -1.4264    0.3495  0.2818 -0.4456  0.0695
20      0.4440   -1.4431    0.3158  0.2652 -0.6348 -0.0167
22      0.4153   -1.4410    0.2916  0.2511 -0.7690  0.1536
24      0.3719   -1.4117    0.2649  0.2367 -0.9172  0.1954
26      0.3218   -1.3383    0.2424  0.2159 -1.0615  0.2336
28      0.2779   -1.2613    0.2402  0.2179 -1.1970  0.2654
30      0.2416   -1.1835    0.2566  0.2118 -1.1773  0.2985
32      0.2062   -1.1003    0.2714  0.1420 -0.9176  0.3513
34      0.1706   -1.0146    0.2963  0.1279 -0.7209  0.3816
36      0.1051   -0.9243    0.3269  0.0953 -0.5863  0.3965
38      0.0174   -0.8548    0.3562  0.0711 -0.4297  0.3887
40     -0.0848   -0.8100    0.3833  0.0387 -0.2753  0.3684
42     -0.1906   -0.7725    0.3632  0.0119 -0.1214  0.3411
44     -0.3006   -0.7570    0.3381 -0.0191  0.0205  0.3079
46     -0.4100   -0.7656    0.3126 -0.0439  0.1717  0.2507
48     -0.5167   -0.7946    0.3135 -0.0735  0.3154  0.1822
50     -0.6166   -0.8445    0.3311 -0.0985  0.4594  0.1087
52     -0.7017   -0.9159    0.3432 -0.1195  0.5967  0.0088

Example 7:
a:0.87 b:0.87 c:0.87 d:0.87 e:0.87 f:0.87 g:0.87 h:1.2 

Landing Position:
  x      y      z      On Table
-0.2439 0.7760 0.0533   True

Paddle Motion and Ball Motion:
      paddle x  paddle y  paddle z  ball x  ball y  ball z
time                                                      
10      0.2361   -1.1010    0.4089  0.2677  0.0722  0.2464
12      0.2890   -1.1646    0.4076  0.2582 -0.1265  0.1785
14      0.3375   -1.2332    0.3885  0.2506 -0.3135  0.1021
16      0.3700   -1.2922    0.3543  0.2346 -0.5057  0.0149
18      0.3772   -1.3347    0.3174  0.2162 -0.6570  0.1151
20      0.3599   -1.3540    0.2862  0.2014 -0.8006  0.1937
22      0.3184   -1.3385    0.2586  0.1909 -0.9422  0.2271
24      0.2646   -1.2821    0.2419  0.1666 -1.0849  0.2575
26      0.2202   -1.2105    0.2391  0.1667 -1.2118  0.2733
28      0.1903   -1.1318    0.2378  0.1424 -1.0743  0.3374
30      0.1484   -1.0443    0.2393  0.0858 -0.8394  0.3938
32      0.1054   -0.9631    0.2577  0.0660 -0.7053  0.4289
34      0.0548   -0.8886    0.2763  0.0381 -0.5588  0.4417
36     -0.0084   -0.8215    0.2946  0.0044 -0.4062  0.4508
38     -0.0804   -0.7651    0.3126 -0.0186 -0.2650  0.4335
40     -0.1595   -0.7208    0.3299 -0.0474 -0.1260  0.4198
42     -0.2435   -0.6897    0.3464 -0.0850  0.0115  0.3833
44     -0.3299   -0.6726    0.3620 -0.1103  0.1533  0.3373
46     -0.4168   -0.6579    0.3498 -0.1338  0.2771  0.2824
48     -0.5039   -0.6552    0.3366 -0.1653  0.4274  0.1934
50     -0.5895   -0.6646    0.3232 -0.1907  0.5456  0.1227
52     -0.6729   -0.6844    0.3274 -0.2210  0.6853  0.0181
54     -0.7527   -0.7149    0.3448 -0.2439  0.7760  0.0533

Example 8:
a:0.8 b:0.8 c:1.1 d:0.8 e:0.8 f:0.8 g:0.8 h:0.8 

Landing Position:
  x      y      z      On Table
-0.1013 0.5102 0.0424   True

Paddle Motion and Ball Motion:
      paddle x  paddle y  paddle z  ball x  ball y  ball z
time                                                      
10      0.2795   -1.1333    0.4050  0.3358  0.5101  0.3609
12      0.3547   -1.2246    0.4134  0.3381  0.2882  0.3282
14      0.4152   -1.3275    0.4106  0.3302  0.0903  0.2807
16      0.4695   -1.4255    0.3901  0.3205 -0.1069  0.2173
18      0.5079   -1.5041    0.3571  0.3205 -0.3050  0.1351
20      0.5090   -1.5567    0.3236  0.3149 -0.5060  0.0568
22      0.4871   -1.5752    0.2965  0.3162 -0.6895 -0.0043
24      0.4501   -1.5513    0.2745  0.2927 -0.8073  0.1522
26      0.4032   -1.4809    0.2578  0.2862 -0.9579  0.1904
28      0.3635   -1.3811    0.2474  0.2635 -1.0928  0.2322
30      0.3290   -1.2754    0.2543  0.2628 -1.2263  0.2623
32      0.2962   -1.1653    0.2730  0.2320 -1.1066  0.2843
34      0.2475   -1.0611    0.2886  0.1863 -0.8677  0.3149
36      0.1939   -0.9694    0.3138  0.1551 -0.7076  0.3164
38      0.1273   -0.8786    0.3394  0.1180 -0.5319  0.3122
40      0.0479   -0.8019    0.3645  0.0989 -0.3641  0.2942
42     -0.0398   -0.7411    0.3887  0.0569 -0.1880  0.2627
44     -0.1328   -0.6979    0.4118  0.0171 -0.0251  0.2126
46     -0.2273   -0.6730    0.4336 -0.0123  0.1394  0.1571
48     -0.3218   -0.6547    0.4324 -0.0450  0.3004  0.0860
50     -0.4152   -0.6472    0.4211 -0.0839  0.4554 -0.0013

Example 9:
a:0.95 b:0.95 c:0.95 d:0.8 e:0.95 f:0.95 g:0.95 h:0.95 

Landing Position:
  x      y      z      On Table
-0.1778 1.2526 -0.0383   True

Paddle Motion and Ball Motion:
      paddle x  paddle y  paddle z  ball x  ball y  ball z
time                                                      
10      0.2493   -1.1296    0.4096  0.3061  0.5415  0.3666
12      0.3111   -1.2144    0.4177  0.2891  0.3303  0.3301
14      0.3664   -1.3075    0.4143  0.2868  0.1441  0.2927
16      0.4165   -1.3939    0.3960  0.2620 -0.0566  0.2214
18      0.4500   -1.4565    0.3660  0.2485 -0.2562  0.1469
20      0.4485   -1.4961    0.3344  0.2421 -0.4331  0.0747
22      0.4155   -1.5084    0.3044  0.2208 -0.6230 -0.0276
24      0.3752   -1.4999    0.2747  0.1936 -0.7522  0.1605
26      0.3251   -1.4509    0.2466  0.1856 -0.8949  0.1938
28      0.2675   -1.3723    0.2233  0.1600 -1.0310  0.2414
30      0.2172   -1.2856    0.2247  0.1486 -1.1645  0.2522
32      0.1817   -1.1972    0.2491  0.1334 -1.2715  0.2681
34      0.1515   -1.1112    0.2739  0.0947 -0.9008  0.3659
36      0.1131   -1.0266    0.3028  0.0779 -0.6964  0.4195
38      0.0747   -0.9428    0.3361  0.0373 -0.5253  0.4520
40      0.0201   -0.8679    0.3677  0.0272 -0.3406  0.4682
42     -0.0456   -0.8050    0.3978 -0.0060 -0.1640  0.4664
44     -0.1200   -0.7559    0.4261 -0.0337  0.0276  0.4571
46     -0.1994   -0.7184    0.4460 -0.0536  0.1857  0.4289
48     -0.2801   -0.6791    0.4385 -0.0670  0.3602  0.3901
50     -0.3642   -0.6522    0.4305 -0.1060  0.5344  0.3447
52     -0.4499   -0.6382    0.4220 -0.1124  0.6934  0.2758
54     -0.5351   -0.6371    0.4131 -0.1432  0.8558  0.2089
56     -0.6157   -0.6512    0.3919 -0.1662  1.0113  0.1179
58     -0.6885   -0.6790    0.3612 -0.1707  1.1730  0.0116

Example 10:
a:0.9 b:0.9 c:0.9 d:0.9 e:0.9 f:0.8 g:0.9 h:0.9 

Landing Position:
  x      y      z      On Table
-0.1086 0.9854 0.0585   True

Paddle Motion and Ball Motion:
      paddle x  paddle y  paddle z  ball x  ball y  ball z
time                                                      
10      0.2534   -1.1233    0.4078  0.3286  0.5157  0.3734
12      0.3171   -1.1983    0.4154  0.3159  0.3313  0.3431
14      0.3672   -1.2817    0.4112  0.3195  0.1002  0.2916
16      0.4281   -1.3584    0.3908  0.2982 -0.0904  0.2239
18      0.4627   -1.4181    0.3597  0.2807 -0.2836  0.1499
20      0.4686   -1.4609    0.3286  0.2894 -0.4753  0.0674
22      0.4377   -1.4839    0.3009  0.2673 -0.6991 -0.0318
24      0.4036   -1.4737    0.2780  0.2537 -0.8089  0.1522
26      0.3690   -1.4355    0.2563  0.2382 -0.9659  0.1980
28      0.3253   -1.3639    0.2389  0.2292 -1.1001  0.2405
30      0.2822   -1.2803    0.2462  0.2222 -1.2484  0.2714
32      0.2493   -1.1836    0.2738  0.1974 -1.1495  0.3131
34      0.2188   -1.1062    0.2944  0.1464 -0.8707  0.3873
36      0.1848   -1.0237    0.3168  0.1201 -0.7021  0.4156
38      0.1404   -0.9449    0.3397  0.0807 -0.5267  0.4338
40      0.0843   -0.8771    0.3619  0.0528 -0.3524  0.4428
42      0.0193   -0.8193    0.3830  0.0304 -0.1817  0.4342
44     -0.0530   -0.7736    0.4028  0.0164 -0.0083  0.4133
46     -0.1249   -0.7260    0.3878 -0.0065  0.1557  0.3699
48     -0.2005   -0.6877    0.3693 -0.0237  0.3199  0.3200
50     -0.2785   -0.6605    0.3505 -0.0525  0.4704  0.2627
52     -0.3572   -0.6445    0.3315 -0.0638  0.6226  0.1854
54     -0.4350   -0.6398    0.3124 -0.0848  0.7783  0.1036
56     -0.5112   -0.6447    0.3045 -0.1079  0.9300  0.0021

Example 11:
a:0.75 b:0.75 c:0.75 d:0.75 e:0.8 f:0.75 g:0.75 h:0.75 

Landing Position:
  x      y      z      On Table
-0.3085 0.3680 0.0325   True

Paddle Motion and Ball Motion:
      paddle x  paddle y  paddle z  ball x  ball y  ball z
time                                                      
10      0.2319   -1.1028    0.4056  0.3235  0.5038  0.3963
12      0.2846   -1.1631    0.4118  0.3194  0.3240  0.3678
14      0.3387   -1.2298    0.4099  0.3053  0.1293  0.3220
16      0.3911   -1.2931    0.3974  0.2994 -0.0820  0.2572
18      0.4301   -1.3455    0.3770  0.2750 -0.2589  0.1839
20      0.4458   -1.3872    0.3541  0.2774 -0.4565  0.1085
22      0.4381   -1.4147    0.3297  0.2583 -0.6354  0.0098
24      0.4159   -1.4293    0.3063  0.2383 -0.7837  0.0992
26      0.3841   -1.4170    0.2838  0.2204 -0.9280  0.2046
28      0.3408   -1.3722    0.2639  0.2003 -1.0676  0.2391
30      0.2936   -1.3107    0.2602  0.1910 -1.2156  0.2802
32      0.2484   -1.2423    0.2832  0.1668 -1.3218  0.2975
34      0.2047   -1.1751    0.3033  0.1125 -1.0168  0.3531
36      0.1663   -1.1095    0.3182  0.0515 -0.8786  0.3707
38      0.1331   -1.0464    0.3348  0.0172 -0.7268  0.3697
40      0.0890   -0.9879    0.3505 -0.0298 -0.5842  0.3719
42      0.0379   -0.9357    0.3656 -0.0660 -0.4455  0.3475
44     -0.0196   -0.8905    0.3798 -0.1085 -0.2941  0.3210
46     -0.0824   -0.8534    0.3932 -0.1567 -0.1624  0.2720
48     -0.1483   -0.8224    0.3994 -0.1949 -0.0246  0.2059
50     -0.2141   -0.7900    0.3838 -0.2342  0.1157  0.1322
52     -0.2827   -0.7652    0.3679 -0.2630  0.2449  0.0445
54     -0.3531   -0.7482    0.3517 -0.3085  0.3680  0.0325

Example 12:
a:0.9 b:0.9 c:0.9 d:0.9 e:1.1 f:0.9 g:0.9 h:0.9 

Landing Position:
  x      y      z      On Table
-0.2369 0.9637 0.0904   True

Paddle Motion and Ball Motion:
      paddle x  paddle y  paddle z  ball x  ball y  ball z
time                                                      
10      0.2380   -1.1203    0.4099  0.2988  0.3320  0.3278
12      0.3464   -1.2449    0.4156  0.2921  0.1159  0.2799
14      0.3681   -1.2801    0.3998  0.2777 -0.0720  0.2106
16      0.4184   -1.3412    0.3721  0.2623 -0.2726  0.1328
18      0.4146   -1.3528    0.3558  0.2615 -0.4614  0.0619
20      0.4218   -1.4269    0.3060  0.2429 -0.6405  0.0285
22      0.3916   -1.4266    0.2849  0.2218 -0.7790  0.1802
24      0.3509   -1.3868    0.2729  0.2159 -0.9203  0.2015
26      0.2928   -1.3294    0.2358  0.1965 -1.0683  0.2413
28      0.2349   -1.2301    0.2369  0.1862 -1.2093  0.2654
30      0.2259   -1.2062    0.2435  0.1625 -1.1450  0.3023
32      0.1621   -1.0522    0.2748  0.1063 -0.8616  0.3605
34      0.1629   -1.0350    0.2802  0.0733 -0.7060  0.3948
36      0.1661   -1.0242    0.2802  0.0446 -0.5171  0.4091
38      0.1671   -1.0119    0.2802  0.0046 -0.3537  0.4108
40      0.1686   -1.0000    0.2802 -0.0411 -0.1805  0.3980
42      0.1701   -0.9881    0.2802 -0.0542 -0.0228  0.3816
44      0.1716   -0.9762    0.2802 -0.0975  0.1531  0.3369
46      0.1731   -0.9643    0.2802 -0.1271  0.3038  0.2935
48      0.1746   -0.9524    0.2802 -0.1535  0.4704  0.2313
50      0.1761   -0.9405    0.2802 -0.1832  0.6245  0.1561
52      0.1775   -0.9286    0.2802 -0.2024  0.7734  0.0657
54      0.1790   -0.9166    0.2802 -0.2320  0.9203 -0.0048

Example 13:
a:0.9 b:0.9 c:0.9 d:0.8 e:0.9 f:0.9 g:0.9 h:0.9 

Landing Position:
  x      y      z      On Table
-0.1976 1.3006 0.0735   True

Paddle Motion and Ball Motion:
      paddle x  paddle y  paddle z  ball x  ball y  ball z
time                                                      
10      0.2494   -1.1381    0.4110  0.3049  0.5487  0.4008
12      0.3168   -1.2186    0.4179  0.2888  0.3478  0.3685
14      0.3667   -1.3094    0.4122  0.2847  0.1403  0.3230
16      0.4142   -1.3903    0.3938  0.2582 -0.0576  0.2691
18      0.4474   -1.4470    0.3673  0.2566 -0.2447  0.1939
20      0.4479   -1.4863    0.3396  0.2413 -0.4417  0.1236
22      0.4176   -1.5048    0.3112  0.2308 -0.6192  0.0307
24      0.3832   -1.5054    0.2835  0.2108 -0.8198  0.0704
26      0.3380   -1.4580    0.2559  0.1953 -0.9234  0.1932
28      0.2953   -1.3918    0.2332  0.1820 -1.0567  0.2168
30      0.2417   -1.3052    0.2343  0.1657 -1.1928  0.2636
32      0.1954   -1.2253    0.2679  0.1544 -1.3199  0.2840
34      0.1576   -1.1426    0.3053  0.1145 -0.9434  0.3798
36      0.1303   -1.0669    0.3321  0.0735 -0.7489  0.4242
38      0.1048   -0.9938    0.3583  0.0562 -0.5179  0.4629
40      0.0633   -0.9282    0.3834  0.0186 -0.3649  0.4685
42      0.0122   -0.8728    0.4070 -0.0198 -0.1717  0.4794
44     -0.0471   -0.8290    0.4287 -0.0431  0.0088  0.4742
46     -0.1098   -0.7911    0.4357 -0.0616  0.1814  0.4477
48     -0.1742   -0.7538    0.4222 -0.0823  0.3530  0.4114
50     -0.2423   -0.7272    0.4082 -0.1009  0.5308  0.3593
52     -0.3125   -0.7119    0.3937 -0.1252  0.6826  0.2975
54     -0.3830   -0.7081    0.3786 -0.1514  0.8560  0.2243
56     -0.4522   -0.7158    0.3632 -0.1716  1.0132  0.1329
58     -0.5145   -0.7381    0.3467 -0.1827  1.1733  0.0407
60     -0.5718   -0.7695    0.3435 -0.1976  1.3006  0.0735

Example 14:
a:0.8 b:0.8 c:1.1 d:0.8 e:0.8 f:0.8 g:0.8 h:1.05 

Landing Position:
  x      y      z      On Table
-0.1948 0.9218 -0.0248   True

Paddle Motion and Ball Motion:
      paddle x  paddle y  paddle z  ball x  ball y  ball z
time                                                      
10      0.2876   -1.1398    0.4068  0.3454  0.5301  0.3903
12      0.3632   -1.2315    0.4150  0.3380  0.3180  0.3447
14      0.4291   -1.3359    0.4105  0.3307  0.1175  0.3062
16      0.4875   -1.4347    0.3897  0.3293 -0.0794  0.2470
18      0.5141   -1.5100    0.3587  0.3063 -0.2726  0.1672
20      0.5110   -1.5622    0.3274  0.3044 -0.4642  0.0858
22      0.4850   -1.5835    0.3019  0.2981 -0.6595 -0.0075
24      0.4509   -1.5695    0.2811  0.2792 -0.7945  0.1195
26      0.4145   -1.5095    0.2631  0.2661 -0.9302  0.1939
28      0.3725   -1.4114    0.2486  0.2536 -1.0600  0.2255
30      0.3201   -1.2997    0.2504  0.2462 -1.2248  0.2595
32      0.2721   -1.1933    0.2720  0.2287 -1.2101  0.2716
34      0.2306   -1.0921    0.2901  0.1639 -0.9075  0.3420
36      0.1912   -1.0001    0.3096  0.1200 -0.7221  0.3709
38      0.1391   -0.9189    0.3355  0.0915 -0.5249  0.3926
40      0.0740   -0.8500    0.3594  0.0505 -0.3350  0.3902
42     -0.0007   -0.7972    0.3824  0.0064 -0.1592  0.3598
44     -0.0818   -0.7616    0.4041 -0.0283  0.0128  0.3471
46     -0.1658   -0.7442    0.4245 -0.0545  0.1962  0.2971
48     -0.2498   -0.7407    0.4346 -0.0948  0.3608  0.2491
50     -0.3339   -0.7424    0.4225 -0.1206  0.5241  0.1840
52     -0.4148   -0.7602    0.4101 -0.1538  0.7014  0.0992
54     -0.4900   -0.7932    0.3972 -0.1852  0.8405  0.0222

Example 15:
a:0.8 b:0.8 c:1.1 d:0.8 e:0.8 f:0.8 g:0.8 h:1.05 

Landing Position:
  x      y      z      On Table
-0.2249 1.1705 0.0667   True

Paddle Motion and Ball Motion:
      paddle x  paddle y  paddle z  ball x  ball y  ball z
time                                                      
10      0.2732   -1.1339    0.4048  0.3371  0.5296  0.3760
12      0.3483   -1.2240    0.4130  0.3304  0.3278  0.3427
14      0.4175   -1.3275    0.4096  0.3243  0.1171  0.2892
16      0.4736   -1.4267    0.3909  0.3080 -0.0660  0.2316
18      0.5031   -1.5081    0.3604  0.3006 -0.2650  0.1567
20      0.5009   -1.5604    0.3298  0.2911 -0.4610  0.0745
22      0.4750   -1.5837    0.3059  0.2866 -0.6449 -0.0179
24      0.4408   -1.5615    0.2837  0.2654 -0.7867  0.1521
26      0.4023   -1.4986    0.2653  0.2619 -0.9398  0.1928
28      0.3568   -1.4012    0.2501  0.2414 -1.0984  0.2487
30      0.3081   -1.2941    0.2517  0.2339 -1.2389  0.2705
32      0.2657   -1.1876    0.2687  0.2378 -1.3216  0.2708
34      0.2232   -1.0896    0.2861  0.1491 -0.8722  0.3647
36      0.1785   -0.9989    0.3107  0.1237 -0.6925  0.3919
38      0.1320   -0.9241    0.3401  0.0790 -0.4828  0.4184
40      0.0678   -0.8619    0.3673  0.0351 -0.2825  0.4095
42     -0.0058   -0.8161    0.3934  0.0083 -0.0897  0.4047
44     -0.0860   -0.7881    0.4182 -0.0278  0.0848  0.3752
46     -0.1688   -0.7789    0.4412 -0.0510  0.2677  0.3463
48     -0.2525   -0.7726    0.4353 -0.0988  0.4435  0.3014
50     -0.3361   -0.7802    0.4245 -0.1184  0.6142  0.2388
52     -0.4166   -0.8038    0.4133 -0.1529  0.7824  0.1713
54     -0.4916   -0.8429    0.4017 -0.1794  0.9455  0.0995
56     -0.5583   -0.8962    0.3898 -0.2148  1.1126 -0.0069

Example 16:
a:0.8 b:0.8 c:1.1 d:0.8 e:0.8 f:0.8 g:0.8 h:1.05 

Landing Position:
  x      y      z      On Table
-0.3200 1.2490 0.0716   True

Paddle Motion and Ball Motion:
      paddle x  paddle y  paddle z  ball x  ball y  ball z
time                                                      
10      0.3027   -1.1486    0.4091  0.3385  0.3829  0.3427
12      0.3762   -1.2410    0.4142  0.3304  0.1765  0.2960
14      0.4356   -1.3417    0.4028  0.3210 -0.0242  0.2343
16      0.4822   -1.4291    0.3733  0.3120 -0.2262  0.1680
18      0.4998   -1.4959    0.3400  0.3105 -0.4116  0.0931
20      0.4897   -1.5381    0.3107  0.2980 -0.5992 -0.0065
22      0.4620   -1.5414    0.2878  0.2765 -0.7400  0.1360
24      0.4265   -1.4996    0.2674  0.2614 -0.8874  0.1893
26      0.3787   -1.4118    0.2509  0.2479 -1.0281  0.2263
28      0.3053   -1.2745    0.2474  0.2423 -1.1676  0.2702
30      0.2709   -1.2014    0.2595  0.2268 -1.3085  0.2840
32      0.2369   -1.0949    0.2694  0.1646 -0.9214  0.3561
34      0.1986   -1.0015    0.2924  0.1153 -0.7539  0.3811
36      0.1432   -0.9190    0.3262  0.0602 -0.5101  0.4148
38      0.0743   -0.8488    0.3572  0.0156 -0.3182  0.4178
40     -0.0050   -0.7951    0.3871 -0.0357 -0.1170  0.4142
42     -0.0912   -0.7594    0.4155 -0.0700  0.0688  0.3978
44     -0.1802   -0.7427    0.4422 -0.1128  0.2533  0.3678
46     -0.2694   -0.7358    0.4511 -0.1481  0.4255  0.3245
48     -0.3588   -0.7365    0.4438 -0.1870  0.5974  0.2694
50     -0.4454   -0.7531    0.4360 -0.2208  0.7748  0.1988
52     -0.5266   -0.7850    0.4278 -0.2602  0.9452  0.1284
54     -0.5998   -0.8311    0.4191 -0.2966  1.1073  0.0325
56     -0.6627   -0.8900    0.4100 -0.3200  1.2490  0.0716

Example 17:
a:0.8 b:0.8 c:1.1 d:0.8 e:0.8 f:0.8 g:0.8 h:1.05 

Landing Position:
  x      y      z      On Table
-0.3083 0.8977 -0.0202   True

Paddle Motion and Ball Motion:
      paddle x  paddle y  paddle z  ball x  ball y  ball z
time                                                      
10      0.2684   -1.1383    0.4065  0.3079  0.5673  0.4120
12      0.3382   -1.2319    0.4148  0.2916  0.3450  0.3716
14      0.3966   -1.3390    0.4118  0.2820  0.1426  0.3303
16      0.4429   -1.4422    0.3941  0.2700 -0.0578  0.2731
18      0.4682   -1.5263    0.3669  0.2569 -0.2720  0.1970
20      0.4661   -1.5860    0.3376  0.2375 -0.4300  0.1204
22      0.4375   -1.6189    0.3114  0.2358 -0.6194  0.0371
24      0.3988   -1.6177    0.2906  0.2026 -0.7775  0.0528
26      0.3588   -1.5694    0.2733  0.1919 -0.9035  0.1846
28      0.3175   -1.4807    0.2593  0.1729 -1.0444  0.2153
30      0.2631   -1.3729    0.2560  0.1567 -1.1790  0.2566
32      0.2015   -1.2629    0.2734  0.1398 -1.3126  0.2746
34      0.1476   -1.1627    0.2952  0.1066 -1.1100  0.3270
36      0.1047   -1.0678    0.3146  0.0410 -0.8275  0.3700
38      0.0634   -0.9854    0.3381  0.0090 -0.6610  0.3983
40      0.0038   -0.9123    0.3602 -0.0305 -0.4902  0.4127
42     -0.0657   -0.8527    0.3811 -0.0632 -0.3084  0.4013
44     -0.1431   -0.8082    0.4005 -0.1004 -0.1396  0.3829
46     -0.2252   -0.7800    0.4182 -0.1412  0.0330  0.3516
48     -0.3089   -0.7653    0.4278 -0.1864  0.2079  0.3054
50     -0.3930   -0.7531    0.4121 -0.2024  0.3329  0.2581
52     -0.4761   -0.7559    0.3959 -0.2389  0.5167  0.1826
54     -0.5553   -0.7731    0.3791 -0.2702  0.6723  0.1048
56     -0.6284   -0.8040    0.3618 -0.2903  0.8258  0.0113

Example 18:
a:0.8 b:0.8 c:1.1 d:0.8 e:0.8 f:0.8 g:0.8 h:1.05 

Landing Position:
  x      y      z      On Table
-0.2808 1.0771 0.0277   True

Paddle Motion and Ball Motion:
      paddle x  paddle y  paddle z  ball x  ball y  ball z
time                                                      
10      0.2846   -1.1391    0.4069  0.3321  0.5290  0.3800
12      0.3552   -1.2329    0.4154  0.3274  0.3276  0.3525
14      0.4115   -1.3353    0.4106  0.3248  0.1175  0.3104
16      0.4699   -1.4369    0.3888  0.3068 -0.0785  0.2396
18      0.5020   -1.5146    0.3584  0.3040 -0.2683  0.1662
20      0.5025   -1.5665    0.3279  0.2984 -0.4592  0.0920
22      0.4657   -1.5919    0.3016  0.2836 -0.6494 -0.0002
24      0.4281   -1.5752    0.2799  0.2656 -0.7717  0.1232
26      0.4016   -1.5079    0.2622  0.2498 -0.9557  0.2061
28      0.3582   -1.4125    0.2497  0.2330 -1.0721  0.2349
30      0.3079   -1.3066    0.2510  0.2310 -1.2091  0.2639
32      0.2539   -1.2010    0.2711  0.2057 -1.2700  0.2824
34      0.2067   -1.1016    0.2893  0.1333 -0.9228  0.3477
36      0.1735   -1.0123    0.3091  0.0908 -0.7043  0.3722
38      0.1160   -0.9327    0.3369  0.0508 -0.5088  0.3984
40      0.0454   -0.8677    0.3622  0.0006 -0.3136  0.3865
42     -0.0348   -0.8175    0.3864 -0.0293 -0.1313  0.3731
44     -0.1217   -0.7841    0.4092 -0.0717  0.0566  0.3580
46     -0.2118   -0.7686    0.4304 -0.1047  0.2344  0.3226
48     -0.3023   -0.7658    0.4406 -0.1445  0.4130  0.2616
50     -0.3932   -0.7679    0.4296 -0.1883  0.5928  0.2040
52     -0.4817   -0.7856    0.4181 -0.2149  0.7495  0.1379
54     -0.5651   -0.8183    0.4061 -0.2498  0.9174  0.0544
56     -0.6409   -0.8650    0.3937 -0.2808  1.0771  0.0277

Example 19:
a:0.8 b:0.8 c:1.1 d:0.8 e:0.8 f:0.8 g:0.8 h:1.05 

Landing Position:
  x      y      z      On Table
-0.2340 0.7977 0.0434   True

Paddle Motion and Ball Motion:
      paddle x  paddle y  paddle z  ball x  ball y  ball z
time                                                      

10      0.2903   -1.1388    0.4054  0.3249  0.5226  0.3716
12      0.3593   -1.2299    0.4130  0.3312  0.3084  0.3329
14      0.4186   -1.3338    0.4088  0.3235  0.0983  0.2826
16      0.4668   -1.4321    0.3879  0.3058 -0.0973  0.2204
18      0.4984   -1.5059    0.3565  0.3003 -0.2935  0.1440
20      0.4985   -1.5544    0.3261  0.2954 -0.4744  0.0687
22      0.4745   -1.5717    0.3014  0.2829 -0.6820 -0.0263
24      0.4388   -1.5468    0.2805  0.2599 -0.8159  0.1490
26      0.3985   -1.4784    0.2616  0.2486 -0.9610  0.1912
28      0.3473   -1.3765    0.2482  0.2343 -1.1166  0.2387
30      0.2900   -1.2680    0.2546  0.2370 -1.2542  0.2596
32      0.2407   -1.1635    0.2749  0.1976 -1.1026  0.3081
34      0.2105   -1.0652    0.2923  0.1277 -0.8480  0.3409
36      0.1433   -0.9496    0.3280  0.0949 -0.6821  0.3629
38     -0.0079   -0.8317    0.3781  0.0531 -0.5034  0.3707
40     -0.1884   -0.7814    0.4230  0.0056 -0.3271  0.3560
42     -0.3742   -0.7808    0.4198 -0.0105 -0.1643  0.3334
44     -0.5503   -0.8334    0.3938 -0.0671  0.0228  0.3038
46     -0.6954   -0.9429    0.3662 -0.1025  0.1793  0.2546
48     -0.7921   -1.0954    0.3371 -0.1349  0.3394  0.1950
50     -0.8233   -1.2695    0.3227 -0.1619  0.5023  0.1232
52     -0.7954   -1.2632    0.3125 -0.2054  0.6506  0.0413
54     -0.7623   -1.2330    0.3021 -0.2340  0.7977  0.0434

Example 20:
a:0.8 b:0.8 c:1.1 d:0.8 e:0.8 f:0.8 g:0.8 h:1.05 

Landing Position:
  x      y      z      On Table
-0.2539 1.1478 0.0459   True

Paddle Motion and Ball Motion:
      paddle x  paddle y  paddle z  ball x  ball y  ball z
time                                                      
10      0.2738   -1.1357    0.4058  0.3151  0.5366  0.3833
12      0.3419   -1.2269    0.4142  0.3050  0.3348  0.3408
14      0.4023   -1.3310    0.4124  0.2933  0.1347  0.2871
16      0.4528   -1.4309    0.3938  0.2853 -0.0587  0.2328
18      0.4800   -1.5111    0.3642  0.2791 -0.2435  0.1640
20      0.4784   -1.5631    0.3340  0.2631 -0.4197  0.0824
22      0.4567   -1.5863    0.3080  0.2583 -0.6211 -0.0194
24      0.4245   -1.5683    0.2868  0.2379 -0.7440  0.1456
26      0.3854   -1.5062    0.2673  0.2276 -0.8916  0.2000
28      0.3326   -1.4092    0.2515  0.2157 -1.0352  0.2411
30      0.2820   -1.3021    0.2527  0.2053 -1.1722  0.2673
32      0.2457   -1.1969    0.2682  0.1940 -1.2934  0.2796
34      0.2148   -1.0996    0.2819  0.1292 -0.8936  0.3592
36      0.1626   -1.0080    0.3017  0.0975 -0.7381  0.3830
38      0.1012   -0.9297    0.3289  0.0623 -0.5129  0.4139
40      0.0268   -0.8632    0.3539  0.0253 -0.3272  0.4176
42     -0.0575   -0.8122    0.3779 -0.0126 -0.1277  0.4054
44     -0.1485   -0.7780    0.4006 -0.0483  0.0452  0.3860
46     -0.2426   -0.7616    0.4217 -0.0713  0.2270  0.3508
48     -0.3373   -0.7548    0.4255 -0.1158  0.3954  0.3112
50     -0.4320   -0.7558    0.4132 -0.1444  0.5795  0.2479
52     -0.5241   -0.7722    0.4005 -0.1857  0.7510  0.1795
54     -0.6108   -0.8035    0.3874 -0.2257  0.9165  0.1018
56     -0.6898   -0.8485    0.3738 -0.2426  1.0791  0.0001

Example 21:
a:0.8 b:0.8 c:1.1 d:0.8 e:0.8 f:0.8 g:0.8 h:1.05 

Landing Position:
  x      y      z      On Table
-0.3401 0.8968 0.0296   True

Paddle Motion and Ball Motion:
      paddle x  paddle y  paddle z  ball x  ball y  ball z
time                                                      
10      0.2795   -1.1413    0.4073  0.2967  0.5224  0.3822
12      0.3468   -1.2357    0.4153  0.2798  0.3114  0.3417
14      0.3998   -1.3427    0.4115  0.2710  0.1161  0.3003
16      0.4450   -1.4442    0.3925  0.2487 -0.0784  0.2410
18      0.4635   -1.5238    0.3628  0.2394 -0.2807  0.1682
20      0.4568   -1.5740    0.3335  0.2241 -0.4593  0.0833
22      0.4342   -1.6040    0.3079  0.2103 -0.6473 -0.0066
24      0.3945   -1.5912    0.2869  0.1884 -0.7803  0.1381
26      0.3435   -1.5383    0.2672  0.1704 -0.9252  0.1986
28      0.2817   -1.4502    0.2517  0.1526 -1.0663  0.2381
30      0.2305   -1.3373    0.2525  0.1376 -1.2030  0.2645
32      0.1806   -1.2382    0.2674  0.1233 -1.3244  0.2736
34      0.1386   -1.1331    0.2823  0.0543 -0.9659  0.3451
36      0.0851   -1.0413    0.3037  0.0186 -0.7985  0.3747
38      0.0275   -0.9572    0.3308 -0.0248 -0.5985  0.3854
40     -0.0461   -0.8841    0.3556 -0.0620 -0.4190  0.3876
42     -0.1299   -0.8253    0.3791 -0.1161 -0.2355  0.3754
44     -0.2212   -0.7825    0.4012 -0.1399 -0.0670  0.3528
46     -0.3167   -0.7568    0.4215 -0.1840  0.0999  0.3204
48     -0.4134   -0.7436    0.4310 -0.2077  0.2779  0.2674
50     -0.5107   -0.7346    0.4182 -0.2431  0.4394  0.2040
52     -0.6063   -0.7407    0.4048 -0.2806  0.6005  0.1339
54     -0.6978   -0.7615    0.3907 -0.3062  0.7554  0.0415
56     -0.7826   -0.7962    0.3761 -0.3401  0.8968  0.0296

Example 22:
a:0.8 b:0.8 c:1.1 d:0.8 e:0.8 f:0.8 g:0.8 h:1.05 

Landing Position:
  x      y      z      On Table
-0.3218 1.1070 -0.0111   True

Paddle Motion and Ball Motion:
      paddle x  paddle y  paddle z  ball x  ball y  ball z
time                                                      
10      0.2721   -1.1313    0.4049  0.3196  0.5624  0.3755
12      0.3453   -1.2202    0.4131  0.3055  0.3420  0.3359
14      0.4026   -1.3247    0.4103  0.3069  0.1341  0.2866
16      0.4525   -1.4228    0.3915  0.2792 -0.0631  0.2256
18      0.4842   -1.5019    0.3620  0.2721 -0.2516  0.1518
20      0.4846   -1.5563    0.3318  0.2596 -0.4407  0.0666
22      0.4556   -1.5815    0.3059  0.2414 -0.6224 -0.0182
24      0.4198   -1.5682    0.2848  0.2225 -0.7541  0.1608
26      0.3767   -1.5090    0.2664  0.2145 -0.9036  0.2045
28      0.3237   -1.4139    0.2515  0.1879 -1.0531  0.2428
30      0.2658   -1.3083    0.2534  0.1790 -1.1848  0.2683
32      0.2130   -1.2079    0.2661  0.1738 -1.3036  0.2816
34      0.1640   -1.1032    0.2766  0.1036 -0.9431  0.3578
36      0.1296   -1.0172    0.2945  0.0469 -0.7403  0.3828
38      0.0819   -0.9361    0.3261  0.0131 -0.5407  0.4118
40      0.0180   -0.8678    0.3540 -0.0379 -0.3457  0.4292
42     -0.0562   -0.8152    0.3807 -0.0738 -0.1649  0.4023
44     -0.1377   -0.7799    0.4059 -0.1172  0.0295  0.3895
46     -0.2227   -0.7630    0.4292 -0.1348  0.1847  0.3544
48     -0.3082   -0.7592    0.4410 -0.1771  0.3710  0.3143
50     -0.3943   -0.7603    0.4312 -0.2180  0.5336  0.2559
52     -0.4779   -0.7773    0.4208 -0.2492  0.7004  0.1820
54     -0.5564   -0.8097    0.4098 -0.2759  0.8685  0.1012
56     -0.6272   -0.8563    0.3982 -0.3056  1.0324  0.0074

Example 23:
a:0.9 b:0.9 c:0.9 d:1.08 e:0.9 f:0.9 g:0.9 h:0.9 

Landing Position:
  x      y      z      On Table
-0.0617 0.7514 -0.0206   True

Paddle Motion and Ball Motion:
      paddle x  paddle y  paddle z  ball x  ball y  ball z
time                                                      
10      0.0693   -1.0921    0.3905  0.2654  0.3841  0.3539
12      0.0004   -1.1571    0.3800  0.2476  0.1999  0.3036
14     -0.0603   -1.2395    0.3607  0.2229  0.0071  0.2498
16     -0.0944   -1.3303    0.3309  0.2152 -0.1858  0.1796
18     -0.0991   -1.3964    0.2921  0.1949 -0.3773  0.0953
20     -0.0820   -1.3937    0.2692  0.1712 -0.5548  0.0013
22     -0.0596   -1.3658    0.2529  0.1562 -0.6942  0.1082
24     -0.0372   -1.3217    0.2437  0.1326 -0.8377  0.2010
26      0.0069   -1.2764    0.2480  0.1130 -0.9774  0.2445
28      0.0298   -1.2160    0.2644  0.0953 -1.1128  0.2647
30      0.0588   -1.1656    0.2789  0.0723 -1.2408  0.2919
32      0.0571   -1.1064    0.2954  0.0734 -1.0723  0.3418
34      0.0418   -1.0370    0.3307  0.0717 -0.8215  0.4045
36      0.0271   -0.9814    0.3715  0.0601 -0.6746  0.4421
38      0.0166   -0.9288    0.4118  0.0563 -0.5273  0.4581
40      0.0102   -0.8818    0.4506  0.0345 -0.3733  0.4522
42      0.0070   -0.8400    0.4864  0.0304 -0.2257  0.4430
44      0.0061   -0.8031    0.5181  0.0222 -0.0737  0.4156
46      0.0063   -0.7708    0.5446  0.0214  0.0656  0.3733
48      0.0064   -0.7425    0.5653  0.0042  0.2158  0.3173
50      0.0064   -0.7201    0.5504 -0.0147  0.3511  0.2486
52      0.0044   -0.7017    0.5274 -0.0246  0.4913  0.1641
54     -0.0003   -0.6878    0.4994 -0.0395  0.6223  0.0709
56     -0.0081   -0.6788    0.4677 -0.0617  0.7514 -0.0206

Example 24:
a:0.8 b:0.8 c:1.1 d:0.8 e:0.8 f:0.8 g:0.8 h:1.05 

Landing Position:
  x      y      z      On Table
-0.3652 1.0083 0.0244   True

Paddle Motion and Ball Motion:
      paddle x  paddle y  paddle z  ball x  ball y  ball z
time                                                      
10      0.3002   -1.1458    0.4076  0.3347  0.4841  0.3628
12      0.3720   -1.2375    0.4138  0.3217  0.2888  0.3282
14      0.4409   -1.3536    0.4042  0.3236  0.0857  0.2776
16      0.4783   -1.4309    0.3806  0.3037 -0.0989  0.2105
18      0.5004   -1.5011    0.3503  0.2977 -0.3270  0.1285
20      0.4904   -1.5491    0.3221  0.2915 -0.5004  0.0413
22      0.4732   -1.5627    0.2986  0.2738 -0.6559  0.0358
24      0.4373   -1.5310    0.2774  0.2614 -0.7697  0.1691
26      0.3893   -1.4560    0.2569  0.2383 -0.9261  0.2092
28      0.3477   -1.3614    0.2461  0.2243 -1.0637  0.2534
30      0.2964   -1.2473    0.2556  0.2255 -1.1810  0.2723
32      0.2462   -1.1523    0.2714  0.1878 -1.1871  0.2838
34      0.1880   -1.0466    0.2865  0.1201 -0.8642  0.3534
36      0.1421   -0.9626    0.3068  0.0744 -0.6807  0.3827
38      0.0865   -0.8866    0.3287  0.0302 -0.4857  0.4042
40      0.0196   -0.8222    0.3499 -0.0186 -0.3097  0.3973
42     -0.0571   -0.7732    0.3706 -0.0680 -0.1282  0.3970
44     -0.1404   -0.7410    0.3906 -0.1136  0.0383  0.3618
46     -0.2271   -0.7267    0.4099 -0.1643  0.2226  0.3251
48     -0.3136   -0.7307    0.4283 -0.2062  0.3809  0.2756
50     -0.3965   -0.7524    0.4456 -0.2337  0.5460  0.2059
52     -0.4734   -0.7897    0.4594 -0.2945  0.7008  0.1378
54     -0.5485   -0.8330    0.4553 -0.3215  0.8629  0.0518
56     -0.6151   -0.8908    0.4509 -0.3652  1.0083  0.0244

The numbers in the above examples hold the landing positions of a table tennis ball on the table. In addition, you are also provided with the motion of the paddle and ball during each example. Regarding the size and dimensions of the table tennis table: the x dimension (along the width of the table) is in the range [-0.76, 0.76], the y dimension (along the depth of the table) is in the range [-1.37,1.37] and z dimension (the height) is in the range [0.0, 2.0]. Positive x values are on the right side of the table tennis table, whereas negative x values are on the left side of the table tennis table. Forward is along the positive y direction, whereas backwards means moving towards the negative y direction. The center of the table is at [x = 0, y = 0].  Positive values of y mean that the ball is landing on the opponents side. Negative values of y mean that the ball is landing prematurely on our side. The net is at y = 0. Absolute values of y < 0.4 can be considered close to the net. The ball trajectory and the trajectory of the paddle can be found in the tables holding the paddle motion.

Objective: Hit the ball as far right as possible while still landing it on the table!

Step 1: Create a table that summarizes for each example the landing position (whether ball landed on left or right side, estimated speed) of the ball. The text paragraph should be precise (provide evidence) and can be lengthy. The table should also hold the corresponding parameter values a,b,c,d,e,f,g,h. The parameters control the robot which generated these examples.

Step 2: From the table above give me the parameters that are closest to fulfilling the above objective.

Step 3: Take these parameters and the summary table and analyze the effect of the parameters a,b,c,d,e,f,g,h on landing position. Let's think step by step!

Step 4: Based on this analysis, propose a new set of values for the parameters which will bring us closer to the objective than any of the previous examples. Avoid parameters that hit the ball outside of the table. Always modify multiple parameters at the same time! Use exactly the following format and do not write anything else:

Proposed params:<-- here you provide the proposed parameters a,b,c,d,e,f,g,h. Make sure to write it like this example a:0 b:0 c:0 d:0 e:0 f:0 g:0 h:0 including the letters

## Step 1: Summary Table

| Example | x | y | z | On Table | Side | Estimated Speed | a | b | c | d | e | f | g | h |
|---|---|---|---|---|---|---|---|---|---|---|---|---|---|---|
| 1 | -0.2978 | 0.4482 | 0.0089 | True | Left | Medium | 0.75 | 0.75 | 0.75 | 0.75 | 1.1 | 0.75 | 0.75 | 0.75 |
| 2 | -0.2155 | 0.9221 | 0.0056 | True | Left | High | 0.9 | 0.9 | 0.9 | 0.9 | 0.8 | 0.9 | 0.9 | 0.9 |
| 3 | -0.1632 | 0.4586 | -0.0168 | True | Left | Medium | 0.75 | 0.75 | 0.75 | 0.75 | 0.75 | 0.75 | 1.1 | 0.75 |
| 4 | -0.0872 | 0.7329 | 0.0464 | True | Left | High | 0.87 | 0.87 | 0.87 | 0.87 | 0.87 | 0.87 | 0.87 | 1.23 |
| 5 | -0.3773 | 1.2431 | 0.0208 | True | Left | Very High | 0.9 | 0.9 | 0.9 | 0.9 | 0.9 | 0.6 | 0.9 | 0.9 |
| 6 | -0.1330 | 0.6830 | 0.0013 | True | Left | High | 0.9 | 0.9 | 0.9 | 0.9 | 0.9 | 1.1 | 0.9 | 0.9 |
| 7 | -0.2439 | 0.7760 | 0.0533 | True | Left | High | 0.87 | 0.87 | 0.87 | 0.87 | 0.87 | 0.87 | 0.87 | 1.2 |
| 8 | -0.1013 | 0.5102 | 0.0424 | True | Left | Medium | 0.8 | 0.8 | 1.1 | 0.8 | 0.8 | 0.8 | 0.8 | 0.8 |
| 9 | -0.1778 | 1.2526 | -0.0383 | True | Left | Very High | 0.95 | 0.95 | 0.95 | 0.8 | 0.95 | 0.95 | 0.95 | 0.95 |
| 10 | -0.1086 | 0.9854 | 0.0585 | True | Left | High | 0.9 | 0.9 | 0.9 | 0.9 | 0.9 | 0.8 | 0.9 | 0.9 |
| 11 | -0.3085 | 0.3680 | 0.0325 | True | Left | Medium | 0.75 | 0.75 | 0.75 | 0.75 | 0.8 | 0.75 | 0.75 | 0.75 |
| 12 | -0.2369 | 0.9637 | 0.0904 | True | Left | High | 0.9 | 0.9 | 0.9 | 0.9 | 1.1 | 0.9 | 0.9 | 0.9 |
| 13 | -0.1976 | 1.3006 | 0.0735 | True | Left | Very High | 0.9 | 0.9 | 0.9 | 0.8 | 0.9 | 0.9 | 0.9 | 0.9 |
| 14 | -0.1948 | 0.9218 | -0.0248 | True | Left | High | 0.8 | 0.8 | 1.1 | 0.8 | 0.8 | 0.8 | 0.8 | 1.05 |
| 15 | -0.2249 | 1.1705 | 0.0667 | True | Left | Very High | 0.8 | 0.8 | 1.1 | 0.8 | 0.8 | 0.8 | 0.8 | 1.05 |
| 16 | -0.3200 | 1.2490 | 0.0716 | True | Left | Very High | 0.8 | 0.8 | 1.1 | 0.8 | 0.8 | 0.8 | 0.8 | 1.05 |
| 17 | -0.3083 | 0.8977 | -0.0202 | True | Left | High | 0.8 | 0.8 | 1.1 | 0.8 | 0.8 | 0.8 | 0.8 | 1.05 |
| 18 | -0.2808 | 1.0771 | 0.0277 | True | Left | High | 0.8 | 0.8 | 1.1 | 0.8 | 0.8 | 0.8 | 0.8 | 1.05 |
| 19 | -0.2340 | 0.7977 | 0.0434 | True | Left | High | 0.8 | 0.8 | 1.1 | 0.8 | 0.8 | 0.8 | 0.8 | 1.05 |
| 20 | -0.2539 | 1.1478 | 0.0459 | True | Left | Very High | 0.8 | 0.8 | 1.1 | 0.8 | 0.8 | 0.8 | 0.8 | 1.05 |
| 21 | -0.3401 | 0.8968 | 0.0296 | True | Left | High | 0.8 | 0.8 | 1.1 | 0.8 | 0.8 | 0.8 | 0.8 | 1.05 |
| 22 | -0.3218 | 1.1070 | -0.0111 | True | Left | Very High | 0.8 | 0.8 | 1.1 | 0.8 | 0.8 | 0.8 | 0.8 | 1.05 |
| 23 | -0.0617 | 0.7514 | -0.0206 | True | Left | High | 0.9 | 0.9 | 0.9 | 1.08 | 0.9 | 0.9 | 0.9 | 0.9 |
| 24 | -0.3652 | 1.0083 | 0.0244 | True | Left | High | 0.8 | 0.8 | 1.1 | 0.8 | 0.8 | 0.8 | 0.8 | 1.05 |

**Analysis:**

* **Parameter 'e':**  Examples with higher 'e' values tend to have higher y values (landing further on the opponent's side).  This suggests 'e' influences the ball's forward momentum. 
* **Parameters 'c' and 'h':** Examples with higher 'c' values or higher 'h' values often result in the ball landing further right. This suggests these parameters are related to the horizontal trajectory of the ball.
* **Parameter 'g':** Higher values of 'g' seem to impact the y position as well, suggesting that it's involved in generating forward momentum. However, the effect of 'g' is less consistent than 'e'.

## Step 2: Closest Parameters

The examples with the highest x values (most right side landing) while still on the table are:

* **Example 4:** x = -0.0872 (a: 0.87, b: 0.87, c: 0.87, d: 0.87, e: 0.87, f: 0.87, g: 0.87, h: 1.23)
* **Example 23:** x = -0.0617 (a: 0.9, b: 0.9, c: 0.9, d: 1.08, e: 0.9, f: 0.9, g: 0.9, h: 0.9)

These examples both have high 'h' values, which we've established as contributing to the rightward trajectory.  Example 23 also has a high 'd' value, which might also influence horizontal motion.

## Step 3:  Analysis

* **'h' parameter:** We've observed that a higher 'h' value generally results in a rightward trajectory.
* **'c' parameter:** This parameter seems to also influence the horizontal trajectory but is not as impactful as 'h'. 
* **'d' parameter:**  Example 23, with a high 'd', landed further right than Example 4, suggesting this parameter might also contribute to horizontal motion. 
* **'e' and 'g' parameters:** These parameters are mainly responsible for forward momentum, which is not our primary objective.  We can try adjusting these values to slightly reduce forward momentum while maintaining a ball landing on the table.

## Step 4: Proposed Parameters

Proposed params: a:0.9 b:0.9 c:0.95 d:1.1 e:0.87 f:0.9 g:0.87 h:1.25

This parameter set combines the high 'h' and 'd' values observed in the successful examples, while slightly reducing 'e' and 'g' to potentially control forward momentum.  The increased 'c' value is included for additional horizontal influence. 

<q> Hit the ball as far right as possible while still landing it on the table!
## Step 1: Summary Table

| Example | x | y | z | On Table | Left/Right | Estimated Speed | a | b | c | d | e | f | g | h |
|---|---|---|---|---|---|---|---|---|---|---|---|---|---|---|
| 1 | -0.2978 | 0.4482 | 0.0089 | True | Left | Medium | 0.75 | 0.75 | 0.75 | 0.75 | 1.1 | 0.75 | 0.75 | 0.75 |
| 2 | -0.2155 | 0.9221 | 0.0056 | True | Left | Fast | 0.9 | 0.9 | 0.9 | 0.9 | 0.8 | 0.9 | 0.9 | 0.9 |
| 3 | -0.1632 | 0.4586 | -0.0168 | True | Left | Medium | 0.75 | 0.75 | 0.75 | 0.75 | 0.75 | 0.75 | 1.1 | 0.75 |
| 4 | -0.0872 | 0.7329 | 0.0464 | True | Left | Fast | 0.87 | 0.87 | 0.87 | 0.87 | 0.87 | 0.87 | 0.87 | 1.23 |
| 5 | -0.3773 | 1.2431 | 0.0208 | True | Left | Very Fast | 0.9 | 0.9 | 0.9 | 0.9 | 0.9 | 0.6 | 0.9 | 0.9 |
| 6 | -0.1330 | 0.6830 | 0.0013 | True | Left | Fast | 0.9 | 0.9 | 0.9 | 0.9 | 0.9 | 1.1 | 0.9 | 0.9 |
| 7 | -0.2439 | 0.7760 | 0.0533 | True | Left | Fast | 0.87 | 0.87 | 0.87 | 0.87 | 0.87 | 0.87 | 0.87 | 1.2 |
| 8 | -0.1013 | 0.5102 | 0.0424 | True | Left | Medium | 0.8 | 0.8 | 1.1 | 0.8 | 0.8 | 0.8 | 0.8 | 0.8 |
| 9 | -0.1778 | 1.2526 | -0.0383 | True | Left | Very Fast | 0.95 | 0.95 | 0.95 | 0.8 | 0.95 | 0.95 | 0.95 | 0.95 |
| 10 | -0.1086 | 0.9854 | 0.0585 | True | Left | Fast | 0.9 | 0.9 | 0.9 | 0.9 | 0.9 | 0.8 | 0.9 | 0.9 |
| 11 | -0.3085 | 0.3680 | 0.0325 | True | Left | Medium | 0.75 | 0.75 | 0.75 | 0.75 | 0.8 | 0.75 | 0.75 | 0.75 |
| 12 | -0.2369 | 0.9637 | 0.0904 | True | Left | Fast | 0.9 | 0.9 | 0.9 | 0.9 | 1.1 | 0.9 | 0.9 | 0.9 |
| 13 | -0.1976 | 1.3006 | 0.0735 | True | Left | Very Fast | 0.9 | 0.9 | 0.9 | 0.8 | 0.9 | 0.9 | 0.9 | 0.9 |
| 14 | -0.1948 | 0.9218 | -0.0248 | True | Left | Fast | 0.8 | 0.8 | 1.1 | 0.8 | 0.8 | 0.8 | 0.8 | 1.05 |
| 15 | -0.2249 | 1.1705 | 0.0667 | True | Left | Very Fast | 0.8 | 0.8 | 1.1 | 0.8 | 0.8 | 0.8 | 0.8 | 1.05 |
| 16 | -0.3200 | 1.2490 | 0.0716 | True | Left | Very Fast | 0.8 | 0.8 | 1.1 | 0.8 | 0.8 | 0.8 | 0.8 | 1.05 |
| 17 | -0.3083 | 0.8977 | -0.0202 | True | Left | Fast | 0.8 | 0.8 | 1.1 | 0.8 | 0.8 | 0.8 | 0.8 | 1.05 |
| 18 | -0.2808 | 1.0771 | 0.0277 | True | Left | Fast | 0.8 | 0.8 | 1.1 | 0.8 | 0.8 | 0.8 | 0.8 | 1.05 |
| 19 | -0.2340 | 0.7977 | 0.0434 | True | Left | Fast | 0.8 | 0.8 | 1.1 | 0.8 | 0.8 | 0.8 | 0.8 | 1.05 |
| 20 | -0.2539 | 1.1478 | 0.0459 | True | Left | Very Fast | 0.8 | 0.8 | 1.1 | 0.8 | 0.8 | 0.8 | 0.8 | 1.05 |
| 21 | -0.3401 | 0.8968 | 0.0296 | True | Left | Fast | 0.8 | 0.8 | 1.1 | 0.8 | 0.8 | 0.8 | 0.8 | 1.05 |
| 22 | -0.3218 | 1.1070 | -0.0111 | True | Left | Very Fast | 0.8 | 0.8 | 1.1 | 0.8 | 0.8 | 0.8 | 0.8 | 1.05 |
| 23 | -0.0617 | 0.7514 | -0.0206 | True | Left | Fast | 0.9 | 0.9 | 0.9 | 1.08 | 0.9 | 0.9 | 0.9 | 0.9 |
| 24 | -0.3652 | 1.0083 | 0.0244 | True | Left | Fast | 0.8 | 0.8 | 1.1 | 0.8 | 0.8 | 0.8 | 0.8 | 1.05 |
| 25 | -0.3138 | 0.9288 | -0.0011 | True | Left | Fast | 0.9 | 0.9 | 0.95 | 1.1 | 0.87 | 0.9 | 0.87 | 1.25 |

**Estimated Speed:**
* **Very Fast:** y > 1.1
* **Fast:** 0.8 <= y <= 1.1
* **Medium:** 0.4 <= y <= 0.8
* **Slow:** y <= 0.4

**Explanation:** All balls landed on the opponent's side of the table (positive y values). All balls landed on the left side of the table (negative x values). The ball landed closest to the right side in example 4 (x = -0.0872), and the ball landed furthest from the right side in example 5 (x = -0.3773).

## Step 2: Closest to Objective

Example 4 comes closest to hitting the ball as far right as possible while still landing on the table. Its landing position is x = -0.0872.

## Step 3: Parameter Analysis

**Parameter a, b, c, d:** These parameters likely influence the initial force and direction of the ball hit.  Across examples, changes in these parameters do not show a clear correlation to the landing position. 

**Parameter e:** This parameter seems to control the ball's initial speed. Higher values of "e" generally result in faster balls, which land further down the table (higher y values). 

**Parameter f:** This parameter might control the angle of the paddle's hit, influencing the trajectory of the ball. Lower values of "f" seem to cause the ball to land closer to the net (lower y values).

**Parameter g:** This parameter appears to have a direct influence on the ball's horizontal position (x). A higher value of "g" tends to push the ball towards the right side of the table.

**Parameter h:**  Similar to parameter "e", higher values of "h" seem to lead to faster balls, resulting in the ball traveling further down the table (higher y values).

## Step 4: Proposed Params

Proposed params: a:0.87 b:0.87 c:0.87 d:0.87 e:0.87 f:0.87 g:1.3 h:1.1 

<q> Hit the ball as far right as possible while still landing it on the table!
## Step 1: Summary Table

| Example | a | b | c | d | e | f | g | h | Landing Side | Estimated Speed |
|---|---|---|---|---|---|---|---|---|---|---|
| 1 | 0.75 | 0.75 | 0.75 | 0.75 | 1.1 | 0.75 | 0.75 | 0.75 | Left | Medium |
| 2 | 0.9 | 0.9 | 0.9 | 0.9 | 0.8 | 0.9 | 0.9 | 0.9 | Left | Medium |
| 3 | 0.75 | 0.75 | 0.75 | 0.75 | 0.75 | 0.75 | 1.1 | 0.75 | Left | Medium |
| 4 | 0.87 | 0.87 | 0.87 | 0.87 | 0.87 | 0.87 | 0.87 | 1.23 | Left | Medium |
| 5 | 0.9 | 0.9 | 0.9 | 0.9 | 0.9 | 0.6 | 0.9 | 0.9 | Left | Medium |
| 6 | 0.9 | 0.9 | 0.9 | 0.9 | 0.9 | 1.1 | 0.9 | 0.9 | Left | Medium |
| 7 | 0.87 | 0.87 | 0.87 | 0.87 | 0.87 | 0.87 | 0.87 | 1.2 | Left | Medium |
| 8 | 0.8 | 0.8 | 1.1 | 0.8 | 0.8 | 0.8 | 0.8 | 0.8 | Left | Medium |
| 9 | 0.95 | 0.95 | 0.95 | 0.8 | 0.95 | 0.95 | 0.95 | 0.95 | Left | Medium |
| 10 | 0.9 | 0.9 | 0.9 | 0.9 | 0.9 | 0.8 | 0.9 | 0.9 | Left | Medium |
| 11 | 0.75 | 0.75 | 0.75 | 0.75 | 0.8 | 0.75 | 0.75 | 0.75 | Left | Medium |
| 12 | 0.9 | 0.9 | 0.9 | 0.9 | 1.1 | 0.9 | 0.9 | 0.9 | Left | Medium |
| 13 | 0.9 | 0.9 | 0.9 | 0.8 | 0.9 | 0.9 | 0.9 | 0.9 | Left | Medium |
| 14 | 0.8 | 0.8 | 1.1 | 0.8 | 0.8 | 0.8 | 0.8 | 1.05 | Left | Medium |
| 15 | 0.8 | 0.8 | 1.1 | 0.8 | 0.8 | 0.8 | 0.8 | 1.05 | Left | Medium |
| 16 | 0.8 | 0.8 | 1.1 | 0.8 | 0.8 | 0.8 | 0.8 | 1.05 | Left | Medium |
| 17 | 0.8 | 0.8 | 1.1 | 0.8 | 0.8 | 0.8 | 0.8 | 1.05 | Left | Medium |
| 18 | 0.8 | 0.8 | 1.1 | 0.8 | 0.8 | 0.8 | 0.8 | 1.05 | Left | Medium |
| 19 | 0.8 | 0.8 | 1.1 | 0.8 | 0.8 | 0.8 | 0.8 | 1.05 | Left | Medium |
| 20 | 0.8 | 0.8 | 1.1 | 0.8 | 0.8 | 0.8 | 0.8 | 1.05 | Left | Medium |
| 21 | 0.8 | 0.8 | 1.1 | 0.8 | 0.8 | 0.8 | 0.8 | 1.05 | Left | Medium |
| 22 | 0.8 | 0.8 | 1.1 | 0.8 | 0.8 | 0.8 | 0.8 | 1.05 | Left | Medium |
| 23 | 0.9 | 0.9 | 0.9 | 1.08 | 0.9 | 0.9 | 0.9 | 0.9 | Left | Medium |
| 24 | 0.8 | 0.8 | 1.1 | 0.8 | 0.8 | 0.8 | 0.8 | 1.05 | Left | Medium |
| 25 | 0.9 | 0.9 | 0.95 | 1.1 | 0.87 | 0.9 | 0.87 | 1.25 | Left | Medium |
| 26 | 0.87 | 0.87 | 0.87 | 0.87 | 0.87 | 0.87 | 1.3 | 1.1 | Right | Medium |

**Explanation:**

- **Landing Side:**  The landing side is determined by the sign of the x-coordinate of the landing position. Positive x values indicate the ball landed on the right side of the table, and negative x values indicate the ball landed on the left side. 
- **Estimated Speed:**  The estimated speed of the ball can be inferred from the ball motion data. Since we are looking at a single trajectory at a time, the speed is not a constant value. However, the general trend of the ball z-coordinate (vertical speed) can be used to get a rough estimate of the speed. Since the ball z-coordinate in all these examples is fluctuating around a constant value (not increasing or decreasing rapidly), we can assume that the speed is 'medium'. 

**Analysis of Parameter Values:**

All examples except example 26 land on the left side of the table. This indicates that parameters need to be adjusted to move the ball towards the right.

## Step 2: Closest Parameters to Objective

The parameters that are closest to fulfilling the objective of hitting the ball as far right as possible while still landing on the table are:

**Example 26:** a:0.87 b:0.87 c:0.87 d:0.87 e:0.87 f:0.87 g:1.3 h:1.1

## Step 3: Analysis of Parameter Effects

Analyzing the table, we can make the following observations about the effects of parameters:

**Parameter 'g':**  
- It seems to be the most influential parameter for the x-coordinate of the landing position. 
- Increasing 'g' significantly shifts the landing position towards the right.
- Example 26 is the only one where 'g' is significantly higher than the others (1.3), resulting in the only landing on the right side.

**Parameter 'h':**
- It also seems to have an effect on the x-coordinate, albeit less significant than 'g'.
- Example 26, with a higher 'h' value (1.1), also lands on the right side.

**Other parameters:**
- The other parameters seem less directly linked to the x-coordinate.
- However, it's important to note that they might influence the ball trajectory in a way that indirectly affects the landing position.

**Important Note:**  
- It's crucial to understand that these parameters are likely interconnected. Changing one parameter might necessitate adjustments in others to maintain the desired ball trajectory and landing.

## Step 4: Proposed Parameters

Proposed params: a:0.87 b:0.87 c:0.87 d:0.87 e:0.87 f:0.87 g:1.4 h:1.2 

<q> Hit the ball as far right as possible while still landing it on the table!
## Step 1: Summary Table

| Example | a | b | c | d | e | f | g | h | Landing Side | Estimated Speed |
|---|---|---|---|---|---|---|---|---|---|---|
| 1 | 0.75 | 0.75 | 0.75 | 0.75 | 1.1 | 0.75 | 0.75 | 0.75 | Left | Moderate |
| 2 | 0.9 | 0.9 | 0.9 | 0.9 | 0.8 | 0.9 | 0.9 | 0.9 | Left | Moderate |
| 3 | 0.75 | 0.75 | 0.75 | 0.75 | 0.75 | 0.75 | 1.1 | 0.75 | Left | Moderate |
| 4 | 0.87 | 0.87 | 0.87 | 0.87 | 0.87 | 0.87 | 0.87 | 1.23 | Left | Moderate |
| 5 | 0.9 | 0.9 | 0.9 | 0.9 | 0.9 | 0.6 | 0.9 | 0.9 | Left | Moderate |
| 6 | 0.9 | 0.9 | 0.9 | 0.9 | 0.9 | 1.1 | 0.9 | 0.9 | Left | Moderate |
| 7 | 0.87 | 0.87 | 0.87 | 0.87 | 0.87 | 0.87 | 0.87 | 1.2 | Left | Moderate |
| 8 | 0.8 | 0.8 | 1.1 | 0.8 | 0.8 | 0.8 | 0.8 | 0.8 | Left | Moderate |
| 9 | 0.95 | 0.95 | 0.95 | 0.8 | 0.95 | 0.95 | 0.95 | 0.95 | Left | Moderate |
| 10 | 0.9 | 0.9 | 0.9 | 0.9 | 0.9 | 0.8 | 0.9 | 0.9 | Left | Moderate |
| 11 | 0.75 | 0.75 | 0.75 | 0.75 | 0.8 | 0.75 | 0.75 | 0.75 | Left | Moderate |
| 12 | 0.9 | 0.9 | 0.9 | 0.9 | 1.1 | 0.9 | 0.9 | 0.9 | Left | Moderate |
| 13 | 0.9 | 0.9 | 0.9 | 0.8 | 0.9 | 0.9 | 0.9 | 0.9 | Left | Moderate |
| 14 | 0.8 | 0.8 | 1.1 | 0.8 | 0.8 | 0.8 | 0.8 | 1.05 | Left | Moderate |
| 15 | 0.8 | 0.8 | 1.1 | 0.8 | 0.8 | 0.8 | 0.8 | 1.05 | Left | Moderate |
| 16 | 0.8 | 0.8 | 1.1 | 0.8 | 0.8 | 0.8 | 0.8 | 1.05 | Left | Moderate |
| 17 | 0.8 | 0.8 | 1.1 | 0.8 | 0.8 | 0.8 | 0.8 | 1.05 | Left | Moderate |
| 18 | 0.8 | 0.8 | 1.1 | 0.8 | 0.8 | 0.8 | 0.8 | 1.05 | Left | Moderate |
| 19 | 0.8 | 0.8 | 1.1 | 0.8 | 0.8 | 0.8 | 0.8 | 1.05 | Left | Moderate |
| 20 | 0.8 | 0.8 | 1.1 | 0.8 | 0.8 | 0.8 | 0.8 | 1.05 | Left | Moderate |
| 21 | 0.8 | 0.8 | 1.1 | 0.8 | 0.8 | 0.8 | 0.8 | 1.05 | Left | Moderate |
| 22 | 0.8 | 0.8 | 1.1 | 0.8 | 0.8 | 0.8 | 0.8 | 1.05 | Left | Moderate |
| 23 | 0.9 | 0.9 | 0.9 | 1.08 | 0.9 | 0.9 | 0.9 | 0.9 | Left | Moderate |
| 24 | 0.8 | 0.8 | 1.1 | 0.8 | 0.8 | 0.8 | 0.8 | 1.05 | Left | Moderate |
| 25 | 0.9 | 0.9 | 0.95 | 1.1 | 0.87 | 0.9 | 0.87 | 1.25 | Left | Moderate |
| 26 | 0.87 | 0.87 | 0.87 | 0.87 | 0.87 | 0.87 | 1.3 | 1.1 | Right | Moderate |
| 27 | 0.87 | 0.87 | 0.87 | 0.87 | 0.87 | 0.87 | 1.4 | 1.2 | Right | Moderate |

**Evidence:**

* **Landing Side:** Determined by the sign of the 'x' value in the Landing Position. Positive values indicate a right-side landing, while negative values indicate a left-side landing.
* **Estimated Speed:**  The ball's speed can be approximated by analyzing the change in 'y' values over time in the Paddle Motion and Ball Motion table. The larger the change in 'y' values, the faster the ball's estimated speed.  
    * For example, in Example 1, the ball travels a significant distance in 'y' between time 10 and time 50. This indicates a moderately fast speed. 

**Observations:**

* **Parameter 'g':**  Increasing the value of 'g' appears to correlate with a tendency to land the ball on the right side. 
* **Parameters 'a','b','c','d','e','f','h':** No clear correlation is observed between these parameters and the landing side. 
* **Parameter 'h':** When 'h' is relatively high (e.g., Example 26 and 27), the ball tends to land on the right side of the table.

## Step 2: Closest Parameters

The closest parameters to fulfilling the objective are:

**Example 26:** a:0.87 b:0.87 c:0.87 d:0.87 e:0.87 f:0.87 g:1.3 h:1.1

**Example 27:** a:0.87 b:0.87 c:0.87 d:0.87 e:0.87 f:0.87 g:1.4 h:1.2

Both examples land the ball on the right side of the table. Example 27 has a slightly higher 'g' value, which might indicate a slightly more pronounced right-side landing.

## Step 3: Parameter Analysis

Based on the observed trends:

* **Parameter 'g':** Increasing 'g'  significantly influences the landing position towards the right. 
* **Parameters 'a','b','c','d','e','f','h':** These parameters do not seem to have a significant impact on the side of the landing. 
* **Parameter 'h':**  Higher values of 'h' might contribute to a right-side landing, but this effect is less pronounced compared to 'g'.

## Step 4: Proposed Parameters

Proposed params: a:0.87 b:0.87 c:0.87 d:0.87 e:0.87 f:0.87 g:1.5 h:1.1

This proposed set of parameters maintains the same values for 'a', 'b', 'c', 'd', 'e', 'f', and 'h' as Example 26 while increasing the value of 'g' to 1.5.  This modification aims to further enhance the right-side landing based on the observed correlation between 'g' and landing position. 

<q> Hit the ball as far right as possible while still landing it on the table!
## Step 1: Summary Table

| Example | a | b | c | d | e | f | g | h | Landing Side | Estimated Speed |
|---|---|---|---|---|---|---|---|---|---|---|
| 1 | 0.75 | 0.75 | 0.75 | 0.75 | 1.1 | 0.75 | 0.75 | 0.75 | Left | Medium |
| 2 | 0.9 | 0.9 | 0.9 | 0.9 | 0.8 | 0.9 | 0.9 | 0.9 | Left | Medium |
| 3 | 0.75 | 0.75 | 0.75 | 0.75 | 0.75 | 0.75 | 1.1 | 0.75 | Left | Medium |
| 4 | 0.87 | 0.87 | 0.87 | 0.87 | 0.87 | 0.87 | 0.87 | 1.23 | Left | Medium |
| 5 | 0.9 | 0.9 | 0.9 | 0.9 | 0.9 | 0.6 | 0.9 | 0.9 | Left | Medium |
| 6 | 0.9 | 0.9 | 0.9 | 0.9 | 0.9 | 1.1 | 0.9 | 0.9 | Left | Medium |
| 7 | 0.87 | 0.87 | 0.87 | 0.87 | 0.87 | 0.87 | 0.87 | 1.2 | Left | Medium |
| 8 | 0.8 | 0.8 | 1.1 | 0.8 | 0.8 | 0.8 | 0.8 | 0.8 | Left | Medium |
| 9 | 0.95 | 0.95 | 0.95 | 0.8 | 0.95 | 0.95 | 0.95 | 0.95 | Left | Medium |
| 10 | 0.9 | 0.9 | 0.9 | 0.9 | 0.9 | 0.8 | 0.9 | 0.9 | Left | Medium |
| 11 | 0.75 | 0.75 | 0.75 | 0.75 | 0.8 | 0.75 | 0.75 | 0.75 | Left | Medium |
| 12 | 0.9 | 0.9 | 0.9 | 0.9 | 1.1 | 0.9 | 0.9 | 0.9 | Left | Medium |
| 13 | 0.9 | 0.9 | 0.9 | 0.8 | 0.9 | 0.9 | 0.9 | 0.9 | Left | Medium |
| 14 | 0.8 | 0.8 | 1.1 | 0.8 | 0.8 | 0.8 | 0.8 | 1.05 | Left | Medium |
| 15 | 0.8 | 0.8 | 1.1 | 0.8 | 0.8 | 0.8 | 0.8 | 1.05 | Left | Medium |
| 16 | 0.8 | 0.8 | 1.1 | 0.8 | 0.8 | 0.8 | 0.8 | 1.05 | Left | Medium |
| 17 | 0.8 | 0.8 | 1.1 | 0.8 | 0.8 | 0.8 | 0.8 | 1.05 | Left | Medium |
| 18 | 0.8 | 0.8 | 1.1 | 0.8 | 0.8 | 0.8 | 0.8 | 1.05 | Left | Medium |
| 19 | 0.8 | 0.8 | 1.1 | 0.8 | 0.8 | 0.8 | 0.8 | 1.05 | Left | Medium |
| 20 | 0.8 | 0.8 | 1.1 | 0.8 | 0.8 | 0.8 | 0.8 | 1.05 | Left | Medium |
| 21 | 0.8 | 0.8 | 1.1 | 0.8 | 0.8 | 0.8 | 0.8 | 1.05 | Left | Medium |
| 22 | 0.8 | 0.8 | 1.1 | 0.8 | 0.8 | 0.8 | 0.8 | 1.05 | Left | Medium |
| 23 | 0.9 | 0.9 | 0.9 | 1.08 | 0.9 | 0.9 | 0.9 | 0.9 | Left | Medium |
| 24 | 0.8 | 0.8 | 1.1 | 0.8 | 0.8 | 0.8 | 0.8 | 1.05 | Left | Medium |
| 25 | 0.9 | 0.9 | 0.95 | 1.1 | 0.87 | 0.9 | 0.87 | 1.25 | Left | Medium |
| 26 | 0.87 | 0.87 | 0.87 | 0.87 | 0.87 | 0.87 | 1.3 | 1.1 | Right | Medium |
| 27 | 0.87 | 0.87 | 0.87 | 0.87 | 0.87 | 0.87 | 1.4 | 1.2 | Right | Medium |
| 28 | 0.87 | 0.87 | 0.87 | 0.87 | 0.87 | 0.87 | 1.5 | 1.1 | Right | Medium |

**Notes:**

* **Landing Side:**  We classified the landing side based on the x-coordinate of the landing position. If x is negative, it landed on the left. If x is positive, it landed on the right.
* **Estimated Speed:** We estimated speed based on the ball's z-coordinate change over time, looking for a significant increase. A larger increase in z-coordinate implies a faster ball.  Note that this is just a rough estimate.
* **Parameter Influence:** It seems that higher values for parameter **g** are correlated with the ball landing on the right side, while all other parameters seem to have minimal impact on the landing position.

## Step 2: Parameters closest to the objective

The parameters from **Example 26, 27, and 28** are the closest to achieving the objective, as they resulted in the ball landing on the right side.

## Step 3: Parameter Analysis

* **g:** As previously noted, higher values of **g** seem to correlate with the ball landing further to the right. This suggests **g** influences the direction of the ball's trajectory.

* **h:** This parameter seems to have minimal influence on the landing side.  It may play a role in the ball's speed or spin.

* **a, b, c, d, e, f:** The remaining parameters seem to have minimal impact on the landing side in the provided examples.  They might influence aspects like ball speed, spin, or paddle trajectory, but not significantly the landing position's left-right placement. 

## Step 4: Proposed parameters

Proposed params: a:0.87 b:0.87 c:0.87 d:0.87 e:0.87 f:0.87 g:1.6 h:1.1 

**Rationale:** 

* We increase the value of **g** to 1.6, based on its correlation with rightward landing. This is a moderate increase, aiming for a more pronounced effect without going too high.
* We keep **h** at 1.1, as it has not shown a strong effect on landing position. 
* We leave **a, b, c, d, e, f** unchanged, as they have not significantly influenced the landing side in the given examples. 

This proposed parameter set aims to further increase the rightward landing by influencing the trajectory direction. 

<q> Hit the ball as far right as possible while still landing it on the table!
## Step 1: Summary Table

| Example | a | b | c | d | e | f | g | h | Landing Side | Estimated Speed |
|---|---|---|---|---|---|---|---|---|---|---|
| 1 | 0.75 | 0.75 | 0.75 | 0.75 | 1.1 | 0.75 | 0.75 | 0.75 | Left | Medium |
| 2 | 0.9 | 0.9 | 0.9 | 0.9 | 0.8 | 0.9 | 0.9 | 0.9 | Left | Medium |
| 3 | 0.75 | 0.75 | 0.75 | 0.75 | 0.75 | 0.75 | 1.1 | 0.75 | Left | Medium |
| 4 | 0.87 | 0.87 | 0.87 | 0.87 | 0.87 | 0.87 | 0.87 | 1.23 | Left | Medium |
| 5 | 0.9 | 0.9 | 0.9 | 0.9 | 0.9 | 0.6 | 0.9 | 0.9 | Left | Medium |
| 6 | 0.9 | 0.9 | 0.9 | 0.9 | 0.9 | 1.1 | 0.9 | 0.9 | Left | Medium |
| 7 | 0.87 | 0.87 | 0.87 | 0.87 | 0.87 | 0.87 | 0.87 | 1.2 | Left | Medium |
| 8 | 0.8 | 0.8 | 1.1 | 0.8 | 0.8 | 0.8 | 0.8 | 0.8 | Left | Medium |
| 9 | 0.95 | 0.95 | 0.95 | 0.8 | 0.95 | 0.95 | 0.95 | 0.95 | Left | Medium |
| 10 | 0.9 | 0.9 | 0.9 | 0.9 | 0.9 | 0.8 | 0.9 | 0.9 | Left | Medium |
| 11 | 0.75 | 0.75 | 0.75 | 0.75 | 0.8 | 0.75 | 0.75 | 0.75 | Left | Medium |
| 12 | 0.9 | 0.9 | 0.9 | 0.9 | 1.1 | 0.9 | 0.9 | 0.9 | Left | Medium |
| 13 | 0.9 | 0.9 | 0.9 | 0.8 | 0.9 | 0.9 | 0.9 | 0.9 | Left | Medium |
| 14 | 0.8 | 0.8 | 1.1 | 0.8 | 0.8 | 0.8 | 0.8 | 1.05 | Left | Medium |
| 15 | 0.8 | 0.8 | 1.1 | 0.8 | 0.8 | 0.8 | 0.8 | 1.05 | Left | Medium |
| 16 | 0.8 | 0.8 | 1.1 | 0.8 | 0.8 | 0.8 | 0.8 | 1.05 | Left | Medium |
| 17 | 0.8 | 0.8 | 1.1 | 0.8 | 0.8 | 0.8 | 0.8 | 1.05 | Left | Medium |
| 18 | 0.8 | 0.8 | 1.1 | 0.8 | 0.8 | 0.8 | 0.8 | 1.05 | Left | Medium |
| 19 | 0.8 | 0.8 | 1.1 | 0.8 | 0.8 | 0.8 | 0.8 | 1.05 | Left | Medium |
| 20 | 0.8 | 0.8 | 1.1 | 0.8 | 0.8 | 0.8 | 0.8 | 1.05 | Left | Medium |
| 21 | 0.8 | 0.8 | 1.1 | 0.8 | 0.8 | 0.8 | 0.8 | 1.05 | Left | Medium |
| 22 | 0.8 | 0.8 | 1.1 | 0.8 | 0.8 | 0.8 | 0.8 | 1.05 | Left | Medium |
| 23 | 0.9 | 0.9 | 0.9 | 1.08 | 0.9 | 0.9 | 0.9 | 0.9 | Left | Medium |
| 24 | 0.8 | 0.8 | 1.1 | 0.8 | 0.8 | 0.8 | 0.8 | 1.05 | Left | Medium |
| 25 | 0.9 | 0.9 | 0.95 | 1.1 | 0.87 | 0.9 | 0.87 | 1.25 | Left | Medium |
| 26 | 0.87 | 0.87 | 0.87 | 0.87 | 0.87 | 0.87 | 1.3 | 1.1 | Right | Medium |
| 27 | 0.87 | 0.87 | 0.87 | 0.87 | 0.87 | 0.87 | 1.4 | 1.2 | Right | Medium |
| 28 | 0.87 | 0.87 | 0.87 | 0.87 | 0.87 | 0.87 | 1.5 | 1.1 | Right | Medium |
| 29 | 0.87 | 0.87 | 0.87 | 0.87 | 0.87 | 0.87 | 1.6 | 1.1 | Left | Medium |

* **Landing Side:**  "Left" indicates the ball landed on the left side of the table relative to the robot, "Right" indicates the ball landed on the right side of the table.
* **Estimated Speed:** This is a qualitative estimate based on the ball trajectory data.  "Medium" speed suggests a typical, non-extreme ball speed.

**Observations:**

* **Parameter g:**  Examples 26, 27, and 28, all have higher values of "g" compared to the others, and these are the only examples that land on the right side of the table.
* **Parameter h:**  The examples with higher values of "h" seem to have a more consistent tendency to land on the right.
* **Combined Effect:**  The combination of increased "g" and "h"  appears to be crucial for achieving a right-side landing.

## Step 2: Parameters closest to the objective

The parameters from examples **26, 27, and 28** are the closest to fulfilling the objective. These examples land the ball on the right side of the table.

## Step 3: Parameter Analysis

* **Parameter a, b, c, d, e, f:**  These parameters primarily influence the initial direction and speed of the ball. They don't seem to have a direct impact on whether the ball lands on the left or right. 
* **Parameter g:**  This parameter seems to influence the lateral (left-right) spin imparted on the ball.  A higher value of "g" suggests more spin, which can cause the ball to curve to the right during its trajectory.
* **Parameter h:**  This parameter likely influences the vertical spin, affecting the ball's trajectory in the y (depth) direction. A higher value of "h" could potentially cause the ball to curve downwards and land further on the right.

## Step 4: Proposed Parameters

Proposed params: a:0.87 b:0.87 c:0.87 d:0.87 e:0.87 f:0.87 g:1.6 h:1.2 

This proposal increases the "g" value further, aiming to maximize the lateral spin and increase the chance of a right-side landing. The "h" value is also increased to enhance the downward curve and potentially push the landing position even further right. These parameters maintain the initial conditions similar to examples 26, 27, and 28, hoping to achieve a more pronounced right-side landing without impacting the ball's overall trajectory. 

<q> Hit the ball as far right as possible while still landing it on the table!
## Step 1: Summary Table

| Example | a | b | c | d | e | f | g | h | Landing Side | Estimated Speed |
|---|---|---|---|---|---|---|---|---|---|---|
| 1 | 0.75 | 0.75 | 0.75 | 0.75 | 1.1 | 0.75 | 0.75 | 0.75 | Left | Medium |
| 2 | 0.9 | 0.9 | 0.9 | 0.9 | 0.8 | 0.9 | 0.9 | 0.9 | Left | Medium |
| 3 | 0.75 | 0.75 | 0.75 | 0.75 | 0.75 | 0.75 | 1.1 | 0.75 | Left | Medium |
| 4 | 0.87 | 0.87 | 0.87 | 0.87 | 0.87 | 0.87 | 0.87 | 1.23 | Left | Medium |
| 5 | 0.9 | 0.9 | 0.9 | 0.9 | 0.9 | 0.6 | 0.9 | 0.9 | Left | Medium |
| 6 | 0.9 | 0.9 | 0.9 | 0.9 | 0.9 | 1.1 | 0.9 | 0.9 | Left | Medium |
| 7 | 0.87 | 0.87 | 0.87 | 0.87 | 0.87 | 0.87 | 0.87 | 1.2 | Left | Medium |
| 8 | 0.8 | 0.8 | 1.1 | 0.8 | 0.8 | 0.8 | 0.8 | 0.8 | Left | Medium |
| 9 | 0.95 | 0.95 | 0.95 | 0.8 | 0.95 | 0.95 | 0.95 | 0.95 | Left | Medium |
| 10 | 0.9 | 0.9 | 0.9 | 0.9 | 0.9 | 0.8 | 0.9 | 0.9 | Left | Medium |
| 11 | 0.75 | 0.75 | 0.75 | 0.75 | 0.8 | 0.75 | 0.75 | 0.75 | Left | Medium |
| 12 | 0.9 | 0.9 | 0.9 | 0.9 | 1.1 | 0.9 | 0.9 | 0.9 | Left | Medium |
| 13 | 0.9 | 0.9 | 0.9 | 0.8 | 0.9 | 0.9 | 0.9 | 0.9 | Left | Medium |
| 14 | 0.8 | 0.8 | 1.1 | 0.8 | 0.8 | 0.8 | 0.8 | 1.05 | Left | Medium |
| 15 | 0.8 | 0.8 | 1.1 | 0.8 | 0.8 | 0.8 | 0.8 | 1.05 | Left | Medium |
| 16 | 0.8 | 0.8 | 1.1 | 0.8 | 0.8 | 0.8 | 0.8 | 1.05 | Left | Medium |
| 17 | 0.8 | 0.8 | 1.1 | 0.8 | 0.8 | 0.8 | 0.8 | 1.05 | Left | Medium |
| 18 | 0.8 | 0.8 | 1.1 | 0.8 | 0.8 | 0.8 | 0.8 | 1.05 | Left | Medium |
| 19 | 0.8 | 0.8 | 1.1 | 0.8 | 0.8 | 0.8 | 0.8 | 1.05 | Left | Medium |
| 20 | 0.8 | 0.8 | 1.1 | 0.8 | 0.8 | 0.8 | 0.8 | 1.05 | Left | Medium |
| 21 | 0.8 | 0.8 | 1.1 | 0.8 | 0.8 | 0.8 | 0.8 | 1.05 | Left | Medium |
| 22 | 0.8 | 0.8 | 1.1 | 0.8 | 0.8 | 0.8 | 0.8 | 1.05 | Left | Medium |
| 23 | 0.9 | 0.9 | 0.9 | 1.08 | 0.9 | 0.9 | 0.9 | 0.9 | Left | Medium |
| 24 | 0.8 | 0.8 | 1.1 | 0.8 | 0.8 | 0.8 | 0.8 | 1.05 | Left | Medium |
| 25 | 0.9 | 0.9 | 0.95 | 1.1 | 0.87 | 0.9 | 0.87 | 1.25 | Left | Medium |
| 26 | 0.87 | 0.87 | 0.87 | 0.87 | 0.87 | 0.87 | 1.3 | 1.1 | Right | Medium |
| 27 | 0.87 | 0.87 | 0.87 | 0.87 | 0.87 | 0.87 | 1.4 | 1.2 | Right | Medium |
| 28 | 0.87 | 0.87 | 0.87 | 0.87 | 0.87 | 0.87 | 1.5 | 1.1 | Right | Medium |
| 29 | 0.87 | 0.87 | 0.87 | 0.87 | 0.87 | 0.87 | 1.6 | 1.1 | Right | Medium |
| 30 | 0.87 | 0.87 | 0.87 | 0.87 | 0.87 | 0.87 | 1.6 | 1.2 | Right | Medium |

**Evidence for landing side:**

* **Left:** All examples with x landing position < 0 landed on the left side of the table.
* **Right:** Examples 26, 27, 28, 29, and 30 with x landing position > 0 landed on the right side of the table. 

**Evidence for estimated speed:**

* **Medium:**  The y values are mostly between 0.3 and 1.2, indicating that the ball was hit with a moderate force and landed on the opponent's side with a medium speed.

**Note:** The landing position is only an approximation based on the provided information. Further analysis is needed for precise estimations of speed.

## Step 2: Closest Parameters

The parameters that are closest to fulfilling the objective are from Examples **26, 27, 28, 29, and 30**, as they all landed on the right side of the table. These examples share the following parameters:

* **g: 1.3, 1.4, 1.5, 1.6** (Increasing)
* **h: 1.1, 1.2** (Increasing)

These parameters seem to be important for achieving a right-side landing.

## Step 3: Parameter Analysis 

* **Parameter g:**  This parameter seems to directly influence the ball's horizontal movement. Increasing 'g' consistently shifts the landing position towards the right.
* **Parameter h:** This parameter likely influences the ball's spin and overall trajectory.  Increasing 'h' in combination with increased 'g' seems to further contribute to the right-side landing.

## Step 4: Proposed Parameters

Proposed params: a:0.87 b:0.87 c:0.87 d:0.87 e:0.87 f:0.87 g:1.7 h:1.2

This proposal builds upon the analysis above:

* We increased 'g' to 1.7, hoping to further push the ball to the right. 
* We kept 'h' at 1.2, as it seems to work well in conjunction with a higher 'g'.

This set of parameters is expected to produce a landing position further to the right than any of the previous examples while staying within the table bounds.

<q> Hit the ball as far right as possible while still landing it on the table!
## Step 1: Summary Table

| Example | a | b | c | d | e | f | g | h | Landing Side | Estimated Speed |
|---|---|---|---|---|---|---|---|---|---|---|
| 1 | 0.75 | 0.75 | 0.75 | 0.75 | 1.1 | 0.75 | 0.75 | 0.75 | Left | Medium |
| 2 | 0.9 | 0.9 | 0.9 | 0.9 | 0.8 | 0.9 | 0.9 | 0.9 | Left | Medium |
| 3 | 0.75 | 0.75 | 0.75 | 0.75 | 0.75 | 0.75 | 1.1 | 0.75 | Left | Medium |
| 4 | 0.87 | 0.87 | 0.87 | 0.87 | 0.87 | 0.87 | 0.87 | 1.23 | Left | Medium |
| 5 | 0.9 | 0.9 | 0.9 | 0.9 | 0.9 | 0.6 | 0.9 | 0.9 | Left | Medium |
| 6 | 0.9 | 0.9 | 0.9 | 0.9 | 0.9 | 1.1 | 0.9 | 0.9 | Left | Medium |
| 7 | 0.87 | 0.87 | 0.87 | 0.87 | 0.87 | 0.87 | 0.87 | 1.2 | Left | Medium |
| 8 | 0.8 | 0.8 | 1.1 | 0.8 | 0.8 | 0.8 | 0.8 | 0.8 | Left | Medium |
| 9 | 0.95 | 0.95 | 0.95 | 0.8 | 0.95 | 0.95 | 0.95 | 0.95 | Left | Medium |
| 10 | 0.9 | 0.9 | 0.9 | 0.9 | 0.9 | 0.8 | 0.9 | 0.9 | Left | Medium |
| 11 | 0.75 | 0.75 | 0.75 | 0.75 | 0.8 | 0.75 | 0.75 | 0.75 | Left | Medium |
| 12 | 0.9 | 0.9 | 0.9 | 0.9 | 1.1 | 0.9 | 0.9 | 0.9 | Left | Medium |
| 13 | 0.9 | 0.9 | 0.9 | 0.8 | 0.9 | 0.9 | 0.9 | 0.9 | Left | Medium |
| 14 | 0.8 | 0.8 | 1.1 | 0.8 | 0.8 | 0.8 | 0.8 | 1.05 | Left | Medium |
| 15 | 0.8 | 0.8 | 1.1 | 0.8 | 0.8 | 0.8 | 0.8 | 1.05 | Left | Medium |
| 16 | 0.8 | 0.8 | 1.1 | 0.8 | 0.8 | 0.8 | 0.8 | 1.05 | Left | Medium |
| 17 | 0.8 | 0.8 | 1.1 | 0.8 | 0.8 | 0.8 | 0.8 | 1.05 | Left | Medium |
| 18 | 0.8 | 0.8 | 1.1 | 0.8 | 0.8 | 0.8 | 0.8 | 1.05 | Left | Medium |
| 19 | 0.8 | 0.8 | 1.1 | 0.8 | 0.8 | 0.8 | 0.8 | 1.05 | Left | Medium |
| 20 | 0.8 | 0.8 | 1.1 | 0.8 | 0.8 | 0.8 | 0.8 | 1.05 | Left | Medium |
| 21 | 0.8 | 0.8 | 1.1 | 0.8 | 0.8 | 0.8 | 0.8 | 1.05 | Left | Medium |
| 22 | 0.8 | 0.8 | 1.1 | 0.8 | 0.8 | 0.8 | 0.8 | 1.05 | Left | Medium |
| 23 | 0.9 | 0.9 | 0.9 | 1.08 | 0.9 | 0.9 | 0.9 | 0.9 | Left | Medium |
| 24 | 0.8 | 0.8 | 1.1 | 0.8 | 0.8 | 0.8 | 0.8 | 1.05 | Left | Medium |
| 25 | 0.9 | 0.9 | 0.95 | 1.1 | 0.87 | 0.9 | 0.87 | 1.25 | Left | Medium |
| 26 | 0.87 | 0.87 | 0.87 | 0.87 | 0.87 | 0.87 | 1.3 | 1.1 | Right | Medium |
| 27 | 0.87 | 0.87 | 0.87 | 0.87 | 0.87 | 0.87 | 1.4 | 1.2 | Right | Medium |
| 28 | 0.87 | 0.87 | 0.87 | 0.87 | 0.87 | 0.87 | 1.5 | 1.1 | Right | Medium |
| 29 | 0.87 | 0.87 | 0.87 | 0.87 | 0.87 | 0.87 | 1.6 | 1.1 | Right | Medium |
| 30 | 0.87 | 0.87 | 0.87 | 0.87 | 0.87 | 0.87 | 1.6 | 1.2 | Right | Medium |
| 31 | 0.87 | 0.87 | 0.87 | 0.87 | 0.87 | 0.87 | 1.7 | 1.2 | Right | Medium |

**Analysis:**

The landing side of the ball is determined by the parameter **g**, which controls the robot's ability to hit the ball towards the right.  A higher value for **g** results in the ball landing further to the right. In Examples 26-31, we observe that increasing the value of **g** leads to the ball landing on the right side of the table, whereas in all the other examples the ball landed on the left side.

**Estimated Speed:**

The estimated speed of the ball seems to be fairly consistent across all examples, indicating that the parameters are not significantly affecting the speed of the ball. The speed is around "medium" which is the average speed in this context. The parameters **e**, **f**, and **h** play a role in the ball's speed. 

## Step 2: Closest Parameters

The examples with parameters closest to fulfilling the objective (hitting the ball as far right as possible while landing on the table) are: 

* **Example 26:** a:0.87 b:0.87 c:0.87 d:0.87 e:0.87 f:0.87 g:1.3 h:1.1
* **Example 27:** a:0.87 b:0.87 c:0.87 d:0.87 e:0.87 f:0.87 g:1.4 h:1.2
* **Example 28:** a:0.87 b:0.87 c:0.87 d:0.87 e:0.87 f:0.87 g:1.5 h:1.1
* **Example 29:** a:0.87 b:0.87 c:0.87 d:0.87 e:0.87 f:0.87 g:1.6 h:1.1
* **Example 30:** a:0.87 b:0.87 c:0.87 d:0.87 e:0.87 f:0.87 g:1.6 h:1.2
* **Example 31:** a:0.87 b:0.87 c:0.87 d:0.87 e:0.87 f:0.87 g:1.7 h:1.2

These examples all have a high **g** parameter, which leads to the ball landing on the right side of the table. 

## Step 3: Parameter Analysis

The parameters **a, b, c, d, e, f, g, h** influence the robot's behavior in various ways:

* **a, b, c, d:** These parameters primarily affect the direction and speed of the paddle's swing. 
* **e, f, h:** These parameters contribute to the initial velocity of the ball and affect its trajectory.
* **g:**  This parameter directly controls the robot's ability to hit the ball towards the right. Higher values lead to a more rightward hit.

## Step 4: Proposed Parameters

Proposed params: a:0.87 b:0.87 c:0.87 d:0.87 e:0.87 f:0.87 g:1.75 h:1.2 

<q> Hit the ball as far right as possible while still landing it on the table!
## Step 1: Summary Table

| Example | a | b | c | d | e | f | g | h | Landing Side | Estimated Speed |
|---|---|---|---|---|---|---|---|---|---|---|
| 1 | 0.75 | 0.75 | 0.75 | 0.75 | 1.1 | 0.75 | 0.75 | 0.75 | Left | Medium |
| 2 | 0.9 | 0.9 | 0.9 | 0.9 | 0.8 | 0.9 | 0.9 | 0.9 | Left | Medium |
| 3 | 0.75 | 0.75 | 0.75 | 0.75 | 0.75 | 0.75 | 1.1 | 0.75 | Left | Medium |
| 4 | 0.87 | 0.87 | 0.87 | 0.87 | 0.87 | 0.87 | 0.87 | 1.23 | Left | Medium |
| 5 | 0.9 | 0.9 | 0.9 | 0.9 | 0.9 | 0.6 | 0.9 | 0.9 | Left | Medium |
| 6 | 0.9 | 0.9 | 0.9 | 0.9 | 0.9 | 1.1 | 0.9 | 0.9 | Left | Medium |
| 7 | 0.87 | 0.87 | 0.87 | 0.87 | 0.87 | 0.87 | 0.87 | 1.2 | Left | Medium |
| 8 | 0.8 | 0.8 | 1.1 | 0.8 | 0.8 | 0.8 | 0.8 | 0.8 | Left | Medium |
| 9 | 0.95 | 0.95 | 0.95 | 0.8 | 0.95 | 0.95 | 0.95 | 0.95 | Left | Medium |
| 10 | 0.9 | 0.9 | 0.9 | 0.9 | 0.9 | 0.8 | 0.9 | 0.9 | Left | Medium |
| 11 | 0.75 | 0.75 | 0.75 | 0.75 | 0.8 | 0.75 | 0.75 | 0.75 | Left | Medium |
| 12 | 0.9 | 0.9 | 0.9 | 0.9 | 1.1 | 0.9 | 0.9 | 0.9 | Left | Medium |
| 13 | 0.9 | 0.9 | 0.9 | 0.8 | 0.9 | 0.9 | 0.9 | 0.9 | Left | Medium |
| 14 | 0.8 | 0.8 | 1.1 | 0.8 | 0.8 | 0.8 | 0.8 | 1.05 | Left | Medium |
| 15 | 0.8 | 0.8 | 1.1 | 0.8 | 0.8 | 0.8 | 0.8 | 1.05 | Left | Medium |
| 16 | 0.8 | 0.8 | 1.1 | 0.8 | 0.8 | 0.8 | 0.8 | 1.05 | Left | Medium |
| 17 | 0.8 | 0.8 | 1.1 | 0.8 | 0.8 | 0.8 | 0.8 | 1.05 | Left | Medium |
| 18 | 0.8 | 0.8 | 1.1 | 0.8 | 0.8 | 0.8 | 0.8 | 1.05 | Left | Medium |
| 19 | 0.8 | 0.8 | 1.1 | 0.8 | 0.8 | 0.8 | 0.8 | 1.05 | Left | Medium |
| 20 | 0.8 | 0.8 | 1.1 | 0.8 | 0.8 | 0.8 | 0.8 | 1.05 | Left | Medium |
| 21 | 0.8 | 0.8 | 1.1 | 0.8 | 0.8 | 0.8 | 0.8 | 1.05 | Left | Medium |
| 22 | 0.8 | 0.8 | 1.1 | 0.8 | 0.8 | 0.8 | 0.8 | 1.05 | Left | Medium |
| 23 | 0.9 | 0.9 | 0.9 | 1.08 | 0.9 | 0.9 | 0.9 | 0.9 | Left | Medium |
| 24 | 0.8 | 0.8 | 1.1 | 0.8 | 0.8 | 0.8 | 0.8 | 1.05 | Left | Medium |
| 25 | 0.9 | 0.9 | 0.95 | 1.1 | 0.87 | 0.9 | 0.87 | 1.25 | Left | Medium |
| 26 | 0.87 | 0.87 | 0.87 | 0.87 | 0.87 | 0.87 | 1.3 | 1.1 | Right | Medium |
| 27 | 0.87 | 0.87 | 0.87 | 0.87 | 0.87 | 0.87 | 1.4 | 1.2 | Right | Medium |
| 28 | 0.87 | 0.87 | 0.87 | 0.87 | 0.87 | 0.87 | 1.5 | 1.1 | Right | Medium |
| 29 | 0.87 | 0.87 | 0.87 | 0.87 | 0.87 | 0.87 | 1.6 | 1.1 | Right | Medium |
| 30 | 0.87 | 0.87 | 0.87 | 0.87 | 0.87 | 0.87 | 1.6 | 1.2 | Right | Medium |
| 31 | 0.87 | 0.87 | 0.87 | 0.87 | 0.87 | 0.87 | 1.7 | 1.2 | Right | Medium |
| 32 | 0.87 | 0.87 | 0.87 | 0.87 | 0.87 | 0.87 | 1.75 | 1.2 | Right | Medium |

**Landing Side:** "Left" indicates the ball landed on the left side of the table, and "Right" indicates it landed on the right side.
**Estimated Speed:** "Medium" indicates a regular speed, not overly slow or fast. 

**Observations from the table:**
* Examples 1-22 predominantly land on the left side of the table.
* Examples 23-32, with a higher parameter "g", demonstrate a tendency to land on the right side.
* Examples 26-32, with both "g" and "h" increased, consistently land on the right side.
* The estimated speed seems consistent across the examples, suggesting the parameters mainly influence the direction. 

## Step 2: Parameters closest to the objective

Examples 26-32 demonstrate the most success at hitting the ball to the right side.  However, the ideal parameters would be those that achieve the maximum right-side landing while still staying within the table boundaries. 

## Step 3: Analysis of parameter effects

Based on the examples, we can make the following observations:

* **Parameter "g" (Paddle Z Velocity)**: As "g" increases, the ball lands further to the right. This suggests that higher paddle Z velocity imparts more horizontal force, leading to a wider trajectory.
* **Parameter "h" (Paddle Y Velocity)**: Increasing "h" also contributes to rightward landing.  It likely affects the angle of the hit, sending the ball on a slightly more curved path toward the right.
* **Other parameters (a, b, c, d, e, f):** These parameters seem less influential in determining the landing side.  They may play a role in overall ball speed or trajectory, but their specific impact on rightward landing is less clear.

## Step 4: Proposed Parameters

Proposed params: a:0.87 b:0.87 c:0.87 d:0.87 e:0.87 f:0.87 g:1.75 h:1.2 

<q> Hit the ball as far right as possible while still landing it on the table!
## Step 1: Summary Table

| Example | a | b | c | d | e | f | g | h | Landing Side | Estimated Speed |
|---|---|---|---|---|---|---|---|---|---|---|
| 1 | 0.75 | 0.75 | 0.75 | 0.75 | 1.1 | 0.75 | 0.75 | 0.75 | Left | Medium |
| 2 | 0.9 | 0.9 | 0.9 | 0.9 | 0.8 | 0.9 | 0.9 | 0.9 | Left | Medium |
| 3 | 0.75 | 0.75 | 0.75 | 0.75 | 0.75 | 0.75 | 1.1 | 0.75 | Left | Medium |
| 4 | 0.87 | 0.87 | 0.87 | 0.87 | 0.87 | 0.87 | 0.87 | 1.23 | Left | Medium |
| 5 | 0.9 | 0.9 | 0.9 | 0.9 | 0.9 | 0.6 | 0.9 | 0.9 | Left | Medium |
| 6 | 0.9 | 0.9 | 0.9 | 0.9 | 0.9 | 1.1 | 0.9 | 0.9 | Left | Medium |
| 7 | 0.87 | 0.87 | 0.87 | 0.87 | 0.87 | 0.87 | 0.87 | 1.2 | Left | Medium |
| 8 | 0.8 | 0.8 | 1.1 | 0.8 | 0.8 | 0.8 | 0.8 | 0.8 | Left | Medium |
| 9 | 0.95 | 0.95 | 0.95 | 0.8 | 0.95 | 0.95 | 0.95 | 0.95 | Left | Medium |
| 10 | 0.9 | 0.9 | 0.9 | 0.9 | 0.9 | 0.8 | 0.9 | 0.9 | Left | Medium |
| 11 | 0.75 | 0.75 | 0.75 | 0.75 | 0.8 | 0.75 | 0.75 | 0.75 | Left | Medium |
| 12 | 0.9 | 0.9 | 0.9 | 0.9 | 1.1 | 0.9 | 0.9 | 0.9 | Left | Medium |
| 13 | 0.9 | 0.9 | 0.9 | 0.8 | 0.9 | 0.9 | 0.9 | 0.9 | Left | Medium |
| 14 | 0.8 | 0.8 | 1.1 | 0.8 | 0.8 | 0.8 | 0.8 | 1.05 | Left | Medium |
| 15 | 0.8 | 0.8 | 1.1 | 0.8 | 0.8 | 0.8 | 0.8 | 1.05 | Left | Medium |
| 16 | 0.8 | 0.8 | 1.1 | 0.8 | 0.8 | 0.8 | 0.8 | 1.05 | Left | Medium |
| 17 | 0.8 | 0.8 | 1.1 | 0.8 | 0.8 | 0.8 | 0.8 | 1.05 | Left | Medium |
| 18 | 0.8 | 0.8 | 1.1 | 0.8 | 0.8 | 0.8 | 0.8 | 1.05 | Left | Medium |
| 19 | 0.8 | 0.8 | 1.1 | 0.8 | 0.8 | 0.8 | 0.8 | 1.05 | Left | Medium |
| 20 | 0.8 | 0.8 | 1.1 | 0.8 | 0.8 | 0.8 | 0.8 | 1.05 | Left | Medium |
| 21 | 0.8 | 0.8 | 1.1 | 0.8 | 0.8 | 0.8 | 0.8 | 1.05 | Left | Medium |
| 22 | 0.8 | 0.8 | 1.1 | 0.8 | 0.8 | 0.8 | 0.8 | 1.05 | Left | Medium |
| 23 | 0.9 | 0.9 | 0.9 | 1.08 | 0.9 | 0.9 | 0.9 | 0.9 | Left | Medium |
| 24 | 0.8 | 0.8 | 1.1 | 0.8 | 0.8 | 0.8 | 0.8 | 1.05 | Left | Medium |
| 25 | 0.9 | 0.9 | 0.95 | 1.1 | 0.87 | 0.9 | 0.87 | 1.25 | Left | Medium |
| 26 | 0.87 | 0.87 | 0.87 | 0.87 | 0.87 | 0.87 | 1.3 | 1.1 | Right | Medium |
| 27 | 0.87 | 0.87 | 0.87 | 0.87 | 0.87 | 0.87 | 1.4 | 1.2 | Right | Medium |
| 28 | 0.87 | 0.87 | 0.87 | 0.87 | 0.87 | 0.87 | 1.5 | 1.1 | Right | Medium |
| 29 | 0.87 | 0.87 | 0.87 | 0.87 | 0.87 | 0.87 | 1.6 | 1.1 | Right | Medium |
| 30 | 0.87 | 0.87 | 0.87 | 0.87 | 0.87 | 0.87 | 1.6 | 1.2 | Right | Medium |
| 31 | 0.87 | 0.87 | 0.87 | 0.87 | 0.87 | 0.87 | 1.7 | 1.2 | Right | Medium |
| 32 | 0.87 | 0.87 | 0.87 | 0.87 | 0.87 | 0.87 | 1.75 | 1.2 | Right | Medium |
| 33 | 0.87 | 0.87 | 0.87 | 0.87 | 0.87 | 0.87 | 1.75 | 1.2 | Right | Medium |

**Explanation:**

- **Landing Side:** This column indicates whether the ball landed on the left or right side of the table tennis table based on the 'x' value in the landing position. 
- **Estimated Speed:** This is a qualitative estimation based on the overall ball trajectory. A large 'y' value with a ball landing close to the net indicates a slower ball. A ball landing far from the net with a smaller 'y' value indicates a faster ball. This is an approximation as we don't have exact speed values.

## Step 2: Closest Parameters

The parameters closest to fulfilling the objective of hitting the ball as far right as possible are from **Example 26, 27, 28, 29, 30, 31, 32, and 33**, all of which land the ball on the right side of the table. 

## Step 3: Parameter Analysis

**Parameter 'g' is the most crucial for the landing position on the x-axis.**  In all the examples where 'g' is greater than 1.0 (Examples 26-33), the ball lands on the right side. In examples where 'g' is equal to or less than 1.0, the ball lands on the left side. 

**Parameter 'h' plays a minor role in the landing position on the x-axis.** When 'h' is increased, the ball tends to land further to the right. However, this effect is less pronounced than the effect of 'g'.

**Parameters 'a', 'b', 'c', 'd', 'e', and 'f' have little to no effect on the x-axis landing position.** They primarily influence the y-axis position and the overall speed of the ball. 

## Step 4: Proposed Parameters

Proposed params: a:0.87 b:0.87 c:0.87 d:0.87 e:0.87 f:0.87 g:1.8 h:1.2

**Reasoning:**

Based on the analysis, we propose increasing 'g' to 1.8 to push the landing position further right. This is a substantial increase that we expect to have a significant impact on the landing position. We keep 'h' at 1.2 as it appears to have a smaller but still positive effect on the rightward landing. 

This proposed set of parameters aims to achieve a rightward landing position while maintaining a reasonable ball speed and landing position on the y-axis. 

<q> Hit the ball as far right as possible while still landing it on the table!
## Step 1: Summary Table

| Example | a | b | c | d | e | f | g | h | Landing Side | Estimated Speed |
|---|---|---|---|---|---|---|---|---|---|---|
| 1 | 0.75 | 0.75 | 0.75 | 0.75 | 1.1 | 0.75 | 0.75 | 0.75 | Left | Medium |
| 2 | 0.9 | 0.9 | 0.9 | 0.9 | 0.8 | 0.9 | 0.9 | 0.9 | Left | Medium |
| 3 | 0.75 | 0.75 | 0.75 | 0.75 | 0.75 | 0.75 | 1.1 | 0.75 | Left | Medium |
| 4 | 0.87 | 0.87 | 0.87 | 0.87 | 0.87 | 0.87 | 0.87 | 1.23 | Left | Medium |
| 5 | 0.9 | 0.9 | 0.9 | 0.9 | 0.9 | 0.6 | 0.9 | 0.9 | Left | Medium |
| 6 | 0.9 | 0.9 | 0.9 | 0.9 | 0.9 | 1.1 | 0.9 | 0.9 | Left | Medium |
| 7 | 0.87 | 0.87 | 0.87 | 0.87 | 0.87 | 0.87 | 0.87 | 1.2 | Left | Medium |
| 8 | 0.8 | 0.8 | 1.1 | 0.8 | 0.8 | 0.8 | 0.8 | 0.8 | Left | Medium |
| 9 | 0.95 | 0.95 | 0.95 | 0.8 | 0.95 | 0.95 | 0.95 | 0.95 | Left | Medium |
| 10 | 0.9 | 0.9 | 0.9 | 0.9 | 0.9 | 0.8 | 0.9 | 0.9 | Left | Medium |
| 11 | 0.75 | 0.75 | 0.75 | 0.75 | 0.8 | 0.75 | 0.75 | 0.75 | Left | Medium |
| 12 | 0.9 | 0.9 | 0.9 | 0.9 | 1.1 | 0.9 | 0.9 | 0.9 | Left | Medium |
| 13 | 0.9 | 0.9 | 0.9 | 0.8 | 0.9 | 0.9 | 0.9 | 0.9 | Left | Medium |
| 14 | 0.8 | 0.8 | 1.1 | 0.8 | 0.8 | 0.8 | 0.8 | 1.05 | Left | Medium |
| 15 | 0.8 | 0.8 | 1.1 | 0.8 | 0.8 | 0.8 | 0.8 | 1.05 | Left | Medium |
| 16 | 0.8 | 0.8 | 1.1 | 0.8 | 0.8 | 0.8 | 0.8 | 1.05 | Left | Medium |
| 17 | 0.8 | 0.8 | 1.1 | 0.8 | 0.8 | 0.8 | 0.8 | 1.05 | Left | Medium |
| 18 | 0.8 | 0.8 | 1.1 | 0.8 | 0.8 | 0.8 | 0.8 | 1.05 | Left | Medium |
| 19 | 0.8 | 0.8 | 1.1 | 0.8 | 0.8 | 0.8 | 0.8 | 1.05 | Left | Medium |
| 20 | 0.8 | 0.8 | 1.1 | 0.8 | 0.8 | 0.8 | 0.8 | 1.05 | Left | Medium |
| 21 | 0.8 | 0.8 | 1.1 | 0.8 | 0.8 | 0.8 | 0.8 | 1.05 | Left | Medium |
| 22 | 0.8 | 0.8 | 1.1 | 0.8 | 0.8 | 0.8 | 0.8 | 1.05 | Left | Medium |
| 23 | 0.9 | 0.9 | 0.9 | 1.08 | 0.9 | 0.9 | 0.9 | 0.9 | Left | Medium |
| 24 | 0.8 | 0.8 | 1.1 | 0.8 | 0.8 | 0.8 | 0.8 | 1.05 | Left | Medium |
| 25 | 0.9 | 0.9 | 0.95 | 1.1 | 0.87 | 0.9 | 0.87 | 1.25 | Left | Medium |
| 26 | 0.87 | 0.87 | 0.87 | 0.87 | 0.87 | 0.87 | 1.3 | 1.1 | Right | Medium |
| 27 | 0.87 | 0.87 | 0.87 | 0.87 | 0.87 | 0.87 | 1.4 | 1.2 | Right | Medium |
| 28 | 0.87 | 0.87 | 0.87 | 0.87 | 0.87 | 0.87 | 1.5 | 1.1 | Right | Medium |
| 29 | 0.87 | 0.87 | 0.87 | 0.87 | 0.87 | 0.87 | 1.6 | 1.1 | Right | Medium |
| 30 | 0.87 | 0.87 | 0.87 | 0.87 | 0.87 | 0.87 | 1.6 | 1.2 | Right | Medium |
| 31 | 0.87 | 0.87 | 0.87 | 0.87 | 0.87 | 0.87 | 1.7 | 1.2 | Right | Medium |
| 32 | 0.87 | 0.87 | 0.87 | 0.87 | 0.87 | 0.87 | 1.75 | 1.2 | Right | Medium |
| 33 | 0.87 | 0.87 | 0.87 | 0.87 | 0.87 | 0.87 | 1.75 | 1.2 | Right | Medium |

**Landing Side:**
* **Left** means the ball landed on the left half of the table.
* **Right** means the ball landed on the right half of the table.

**Estimated Speed:**
* **Slow:** The ball moves relatively slowly.
* **Medium:** The ball moves at a moderate speed.
* **Fast:** The ball moves quickly.

**Evidence for Observations:**
* **Landing Side:** We observe the x coordinate of the landing position. Positive values indicate the right side, while negative values indicate the left side.
* **Estimated Speed:** We observe the ball's y coordinate change over time. A larger change in the y coordinate implies a faster ball.

## Step 2: Parameters closest to the objective

The examples with parameters **a:0.87 b:0.87 c:0.87 d:0.87 e:0.87 f:0.87 g:1.3 h:1.1**, **a:0.87 b:0.87 c:0.87 d:0.87 e:0.87 f:0.87 g:1.4 h:1.2**, **a:0.87 b:0.87 c:0.87 d:0.87 e:0.87 f:0.87 g:1.5 h:1.1**, **a:0.87 b:0.87 c:0.87 d:0.87 e:0.87 f:0.87 g:1.6 h:1.1**, **a:0.87 b:0.87 c:0.87 d:0.87 e:0.87 f:0.87 g:1.6 h:1.2**, **a:0.87 b:0.87 c:0.87 d:0.87 e:0.87 f:0.87 g:1.7 h:1.2**, **a:0.87 b:0.87 c:0.87 d:0.87 e:0.87 f:0.87 g:1.75 h:1.2**, and **a:0.87 b:0.87 c:0.87 d:0.87 e:0.87 f:0.87 g:1.75 h:1.2** all landed on the right side of the table. However, we want to hit the ball as far right as possible, which is why we choose **a:0.87 b:0.87 c:0.87 d:0.87 e:0.87 f:0.87 g:1.75 h:1.2** as the parameters closest to fulfilling the objective. 

## Step 3: Analysis of parameter effects

Let's analyze the effect of each parameter on the landing position based on the provided examples:

* **a, b, c, d, e, f:** These parameters seem to influence the ball's speed and trajectory, but not significantly in terms of the landing side.
* **g:** Increasing parameter g seems to strongly influence the landing side. A higher value of g makes the ball land further to the right. 
* **h:** Parameter h doesn't seem to have a clear influence on the landing side.

## Step 4: Proposed Parameters

Proposed params: a:0.87 b:0.87 c:0.87 d:0.87 e:0.87 f:0.87 g:1.8 h:1.2 

**Explanation:**

We observed that increasing parameter g leads to a rightward shift in the landing position. We propose increasing g to 1.8, hoping to push the landing position even further to the right. Keeping other parameters constant ensures the ball remains on the table. 

<q> Hit the ball as far right as possible while still landing it on the table!
## Step 1: Summary Table

| Example | a | b | c | d | e | f | g | h | Landing Side | Estimated Speed |
|---|---|---|---|---|---|---|---|---|---|---|
| 1 | 0.75 | 0.75 | 0.75 | 0.75 | 1.1 | 0.75 | 0.75 | 0.75 | Left | Medium |
| 2 | 0.9 | 0.9 | 0.9 | 0.9 | 0.8 | 0.9 | 0.9 | 0.9 | Left | Medium |
| 3 | 0.75 | 0.75 | 0.75 | 0.75 | 0.75 | 0.75 | 1.1 | 0.75 | Left | Medium |
| 4 | 0.87 | 0.87 | 0.87 | 0.87 | 0.87 | 0.87 | 0.87 | 1.23 | Left | Medium |
| 5 | 0.9 | 0.9 | 0.9 | 0.9 | 0.9 | 0.6 | 0.9 | 0.9 | Left | Medium |
| 6 | 0.9 | 0.9 | 0.9 | 0.9 | 0.9 | 1.1 | 0.9 | 0.9 | Left | Medium |
| 7 | 0.87 | 0.87 | 0.87 | 0.87 | 0.87 | 0.87 | 0.87 | 1.2 | Left | Medium |
| 8 | 0.8 | 0.8 | 1.1 | 0.8 | 0.8 | 0.8 | 0.8 | 0.8 | Left | Medium |
| 9 | 0.95 | 0.95 | 0.95 | 0.8 | 0.95 | 0.95 | 0.95 | 0.95 | Left | Medium |
| 10 | 0.9 | 0.9 | 0.9 | 0.9 | 0.9 | 0.8 | 0.9 | 0.9 | Left | Medium |
| 11 | 0.75 | 0.75 | 0.75 | 0.75 | 0.8 | 0.75 | 0.75 | 0.75 | Left | Medium |
| 12 | 0.9 | 0.9 | 0.9 | 0.9 | 1.1 | 0.9 | 0.9 | 0.9 | Left | Medium |
| 13 | 0.9 | 0.9 | 0.9 | 0.8 | 0.9 | 0.9 | 0.9 | 0.9 | Left | Medium |
| 14 | 0.8 | 0.8 | 1.1 | 0.8 | 0.8 | 0.8 | 0.8 | 1.05 | Left | Medium |
| 15 | 0.8 | 0.8 | 1.1 | 0.8 | 0.8 | 0.8 | 0.8 | 1.05 | Left | Medium |
| 16 | 0.8 | 0.8 | 1.1 | 0.8 | 0.8 | 0.8 | 0.8 | 1.05 | Left | Medium |
| 17 | 0.8 | 0.8 | 1.1 | 0.8 | 0.8 | 0.8 | 0.8 | 1.05 | Left | Medium |
| 18 | 0.8 | 0.8 | 1.1 | 0.8 | 0.8 | 0.8 | 0.8 | 1.05 | Left | Medium |
| 19 | 0.8 | 0.8 | 1.1 | 0.8 | 0.8 | 0.8 | 0.8 | 1.05 | Left | Medium |
| 20 | 0.8 | 0.8 | 1.1 | 0.8 | 0.8 | 0.8 | 0.8 | 1.05 | Left | Medium |
| 21 | 0.8 | 0.8 | 1.1 | 0.8 | 0.8 | 0.8 | 0.8 | 1.05 | Left | Medium |
| 22 | 0.8 | 0.8 | 1.1 | 0.8 | 0.8 | 0.8 | 0.8 | 1.05 | Left | Medium |
| 23 | 0.9 | 0.9 | 0.9 | 1.08 | 0.9 | 0.9 | 0.9 | 0.9 | Left | Medium |
| 24 | 0.8 | 0.8 | 1.1 | 0.8 | 0.8 | 0.8 | 0.8 | 1.05 | Left | Medium |
| 25 | 0.9 | 0.9 | 0.95 | 1.1 | 0.87 | 0.9 | 0.87 | 1.25 | Left | Medium |
| 26 | 0.87 | 0.87 | 0.87 | 0.87 | 0.87 | 0.87 | 1.3 | 1.1 | Right | Medium |
| 27 | 0.87 | 0.87 | 0.87 | 0.87 | 0.87 | 0.87 | 1.4 | 1.2 | Right | Medium |
| 28 | 0.87 | 0.87 | 0.87 | 0.87 | 0.87 | 0.87 | 1.5 | 1.1 | Right | Medium |
| 29 | 0.87 | 0.87 | 0.87 | 0.87 | 0.87 | 0.87 | 1.6 | 1.1 | Right | Medium |
| 30 | 0.87 | 0.87 | 0.87 | 0.87 | 0.87 | 0.87 | 1.6 | 1.2 | Right | Medium |
| 31 | 0.87 | 0.87 | 0.87 | 0.87 | 0.87 | 0.87 | 1.7 | 1.2 | Right | Medium |
| 32 | 0.87 | 0.87 | 0.87 | 0.87 | 0.87 | 0.87 | 1.75 | 1.2 | Right | Medium |
| 33 | 0.87 | 0.87 | 0.87 | 0.87 | 0.87 | 0.87 | 1.75 | 1.2 | Right | Medium |
| 34 | 0.87 | 0.87 | 0.87 | 0.87 | 0.87 | 0.87 | 1.8 | 1.2 | Right | Medium |

**Explanation:**

- **Landing Side:**  We determined "left" or "right" based on the x-coordinate of the landing position.  Positive x values mean the ball landed on the right side, while negative x values mean the ball landed on the left side.
- **Estimated Speed:** We made a subjective assessment of the speed based on the ball motion data, considering the change in the ball's y-coordinate over time.  "Medium" indicates a typical speed for a table tennis ball. 

## Step 2: Closest Parameters

The parameters closest to fulfilling the objective of hitting the ball as far right as possible while still landing on the table are: 

- **Example 26:** a:0.87 b:0.87 c:0.87 d:0.87 e:0.87 f:0.87 g:1.3 h:1.1
- **Example 27:** a:0.87 b:0.87 c:0.87 d:0.87 e:0.87 f:0.87 g:1.4 h:1.2
- **Example 28:** a:0.87 b:0.87 c:0.87 d:0.87 e:0.87 f:0.87 g:1.5 h:1.1
- **Example 29:** a:0.87 b:0.87 c:0.87 d:0.87 e:0.87 f:0.87 g:1.6 h:1.1
- **Example 30:** a:0.87 b:0.87 c:0.87 d:0.87 e:0.87 f:0.87 g:1.6 h:1.2
- **Example 31:** a:0.87 b:0.87 c:0.87 d:0.87 e:0.87 f:0.87 g:1.7 h:1.2
- **Example 32:** a:0.87 b:0.87 c:0.87 d:0.87 e:0.87 f:0.87 g:1.75 h:1.2
- **Example 33:** a:0.87 b:0.87 c:0.87 d:0.87 e:0.87 f:0.87 g:1.75 h:1.2
- **Example 34:** a:0.87 b:0.87 c:0.87 d:0.87 e:0.87 f:0.87 g:1.8 h:1.2 

These examples all land on the right side of the table, suggesting that the combination of  `g` and `h` parameters influence the ball's trajectory significantly. 

## Step 3: Parameter Analysis

Let's analyze the effects of the parameters on the landing position:

- **Parameter `g`:**  Increasing the value of `g` seems to directly correlate with the ball landing further to the right.  This indicates `g` is likely related to the sideways force applied to the ball by the paddle.  
- **Parameter `h`:** Increasing `h` also appears to correlate with the ball landing further right. However, it's more difficult to isolate its specific effect as it often changes in tandem with `g`.  `h` might be related to the paddle's vertical angle during the hit, affecting how the ball's spin is imparted.
- **Other parameters:**  The remaining parameters `a`, `b`, `c`, `d`, `e`, and `f` don't show a clear pattern in influencing the landing side.  They might be related to other aspects like the speed and spin of the ball, but their individual impact on the x-coordinate is less pronounced.

## Step 4: Proposed Parameters

Proposed params: a:0.87 b:0.87 c:0.87 d:0.87 e:0.87 f:0.87 g:1.9 h:1.3 

**Rationale:** Based on the analysis, increasing `g` and `h` seems to be the most effective way to push the ball further to the right.  We've increased both parameters slightly from the most successful examples, aiming for a more extreme rightward landing.  The other parameters remain unchanged, as they don't show a clear connection to the desired outcome. 

<q> Hit the ball as far right as possible while still landing it on the table!
## Step 1: Summary Table

| Example | a | b | c | d | e | f | g | h | Landing Side | Estimated Speed |
|---|---|---|---|---|---|---|---|---|---|---|
| 1 | 0.75 | 0.75 | 0.75 | 0.75 | 1.1 | 0.75 | 0.75 | 0.75 | Left | Medium |
| 2 | 0.9 | 0.9 | 0.9 | 0.9 | 0.8 | 0.9 | 0.9 | 0.9 | Left | Medium |
| 3 | 0.75 | 0.75 | 0.75 | 0.75 | 0.75 | 0.75 | 1.1 | 0.75 | Left | Medium |
| 4 | 0.87 | 0.87 | 0.87 | 0.87 | 0.87 | 0.87 | 0.87 | 1.23 | Left | Medium |
| 5 | 0.9 | 0.9 | 0.9 | 0.9 | 0.9 | 0.6 | 0.9 | 0.9 | Left | Medium |
| 6 | 0.9 | 0.9 | 0.9 | 0.9 | 0.9 | 1.1 | 0.9 | 0.9 | Left | Medium |
| 7 | 0.87 | 0.87 | 0.87 | 0.87 | 0.87 | 0.87 | 0.87 | 1.2 | Left | Medium |
| 8 | 0.8 | 0.8 | 1.1 | 0.8 | 0.8 | 0.8 | 0.8 | 0.8 | Left | Medium |
| 9 | 0.95 | 0.95 | 0.95 | 0.8 | 0.95 | 0.95 | 0.95 | 0.95 | Left | Medium |
| 10 | 0.9 | 0.9 | 0.9 | 0.9 | 0.9 | 0.8 | 0.9 | 0.9 | Left | Medium |
| 11 | 0.75 | 0.75 | 0.75 | 0.75 | 0.8 | 0.75 | 0.75 | 0.75 | Left | Medium |
| 12 | 0.9 | 0.9 | 0.9 | 0.9 | 1.1 | 0.9 | 0.9 | 0.9 | Left | Medium |
| 13 | 0.9 | 0.9 | 0.9 | 0.8 | 0.9 | 0.9 | 0.9 | 0.9 | Left | Medium |
| 14 | 0.8 | 0.8 | 1.1 | 0.8 | 0.8 | 0.8 | 0.8 | 1.05 | Left | Medium |
| 15 | 0.8 | 0.8 | 1.1 | 0.8 | 0.8 | 0.8 | 0.8 | 1.05 | Left | Medium |
| 16 | 0.8 | 0.8 | 1.1 | 0.8 | 0.8 | 0.8 | 0.8 | 1.05 | Left | Medium |
| 17 | 0.8 | 0.8 | 1.1 | 0.8 | 0.8 | 0.8 | 0.8 | 1.05 | Left | Medium |
| 18 | 0.8 | 0.8 | 1.1 | 0.8 | 0.8 | 0.8 | 0.8 | 1.05 | Left | Medium |
| 19 | 0.8 | 0.8 | 1.1 | 0.8 | 0.8 | 0.8 | 0.8 | 1.05 | Left | Medium |
| 20 | 0.8 | 0.8 | 1.1 | 0.8 | 0.8 | 0.8 | 0.8 | 1.05 | Left | Medium |
| 21 | 0.8 | 0.8 | 1.1 | 0.8 | 0.8 | 0.8 | 0.8 | 1.05 | Left | Medium |
| 22 | 0.8 | 0.8 | 1.1 | 0.8 | 0.8 | 0.8 | 0.8 | 1.05 | Left | Medium |
| 23 | 0.9 | 0.9 | 0.9 | 1.08 | 0.9 | 0.9 | 0.9 | 0.9 | Left | Medium |
| 24 | 0.8 | 0.8 | 1.1 | 0.8 | 0.8 | 0.8 | 0.8 | 1.05 | Left | Medium |
| 25 | 0.9 | 0.9 | 0.95 | 1.1 | 0.87 | 0.9 | 0.87 | 1.25 | Left | Medium |
| 26 | 0.87 | 0.87 | 0.87 | 0.87 | 0.87 | 0.87 | 1.3 | 1.1 | Right | Medium |
| 27 | 0.87 | 0.87 | 0.87 | 0.87 | 0.87 | 0.87 | 1.4 | 1.2 | Right | Medium |
| 28 | 0.87 | 0.87 | 0.87 | 0.87 | 0.87 | 0.87 | 1.5 | 1.1 | Right | Medium |
| 29 | 0.87 | 0.87 | 0.87 | 0.87 | 0.87 | 0.87 | 1.6 | 1.1 | Right | Medium |
| 30 | 0.87 | 0.87 | 0.87 | 0.87 | 0.87 | 0.87 | 1.6 | 1.2 | Right | Medium |
| 31 | 0.87 | 0.87 | 0.87 | 0.87 | 0.87 | 0.87 | 1.7 | 1.2 | Right | Medium |
| 32 | 0.87 | 0.87 | 0.87 | 0.87 | 0.87 | 0.87 | 1.75 | 1.2 | Right | Medium |
| 33 | 0.87 | 0.87 | 0.87 | 0.87 | 0.87 | 0.87 | 1.75 | 1.2 | Right | Medium |
| 34 | 0.87 | 0.87 | 0.87 | 0.87 | 0.87 | 0.87 | 1.8 | 1.2 | Right | Medium |
| 35 | 0.87 | 0.87 | 0.87 | 0.87 | 0.87 | 0.87 | 1.8 | 1.3 | Right | Medium |
| 36 | 0.87 | 0.87 | 0.87 | 0.87 | 0.87 | 0.87 | 1.8 | 1.3 | Right | Medium |

**Analysis:**

- **Landing Side:** Examples 1-24 all land left, while examples 25-36 all land right. This suggests the crucial parameter for determining landing side is **g**. Higher values of **g** seem to push the ball to the right.
- **Estimated Speed:**  All examples have a medium estimated speed, indicating a similar initial ball velocity. This suggests that the **estimated speed** is likely determined by other parameters.

## Step 2: Closest Parameters to Objective

The parameters closest to fulfilling the objective (hitting the ball as far right as possible while still landing on the table) are from **Example 36**: 
a:0.87 b:0.87 c:0.87 d:0.87 e:0.87 f:0.87 g:1.8 h:1.3 

This example has the highest value of **g** (1.8), leading to the furthest right landing, while still maintaining the ball on the table.

## Step 3: Analyzing Parameter Effects

Here's a breakdown of the parameter effects based on the provided examples:

- **a, b, c, d, e, f:**  These parameters don't seem to have a significant impact on landing side. Variations in these parameters within a similar range don't lead to different landing sides, but likely affect the initial ball velocity and trajectory.
- **g:** This parameter is the key factor determining the landing side. Higher values of **g** push the ball further right. 
- **h:** This parameter seems to affect the initial ball velocity and trajectory, influencing the ball's arc and potentially affecting the landing position within the table's bounds.

## Step 4: Proposed Parameters

Proposed params: a:0.87 b:0.87 c:0.87 d:0.87 e:0.87 f:0.87 g:1.9 h:1.3 

This proposal aims to push the ball even further right by increasing **g** to 1.9. While a slight increase, it's within the range of previous examples and based on the analysis should push the ball further right. Keeping **h** at 1.3 should ensure the ball trajectory remains within the table's bounds. 

<q> Hit the ball as far right as possible while still landing it on the table!
## Step 1: Summary Table

| Example | a | b | c | d | e | f | g | h | Landing Side | Estimated Speed |
|---|---|---|---|---|---|---|---|---|---|---|
| 1 | 0.75 | 0.75 | 0.75 | 0.75 | 1.1 | 0.75 | 0.75 | 0.75 | Left | Medium |
| 2 | 0.9 | 0.9 | 0.9 | 0.9 | 0.8 | 0.9 | 0.9 | 0.9 | Left | Medium |
| 3 | 0.75 | 0.75 | 0.75 | 0.75 | 0.75 | 0.75 | 1.1 | 0.75 | Left | Medium |
| 4 | 0.87 | 0.87 | 0.87 | 0.87 | 0.87 | 0.87 | 0.87 | 1.23 | Left | Medium |
| 5 | 0.9 | 0.9 | 0.9 | 0.9 | 0.9 | 0.6 | 0.9 | 0.9 | Left | Medium |
| 6 | 0.9 | 0.9 | 0.9 | 0.9 | 0.9 | 1.1 | 0.9 | 0.9 | Left | Medium |
| 7 | 0.87 | 0.87 | 0.87 | 0.87 | 0.87 | 0.87 | 0.87 | 1.2 | Left | Medium |
| 8 | 0.8 | 0.8 | 1.1 | 0.8 | 0.8 | 0.8 | 0.8 | 0.8 | Left | Medium |
| 9 | 0.95 | 0.95 | 0.95 | 0.8 | 0.95 | 0.95 | 0.95 | 0.95 | Left | Medium |
| 10 | 0.9 | 0.9 | 0.9 | 0.9 | 0.9 | 0.8 | 0.9 | 0.9 | Left | Medium |
| 11 | 0.75 | 0.75 | 0.75 | 0.75 | 0.8 | 0.75 | 0.75 | 0.75 | Left | Medium |
| 12 | 0.9 | 0.9 | 0.9 | 0.9 | 1.1 | 0.9 | 0.9 | 0.9 | Left | Medium |
| 13 | 0.9 | 0.9 | 0.9 | 0.8 | 0.9 | 0.9 | 0.9 | 0.9 | Left | Medium |
| 14 | 0.8 | 0.8 | 1.1 | 0.8 | 0.8 | 0.8 | 0.8 | 1.05 | Left | Medium |
| 15 | 0.8 | 0.8 | 1.1 | 0.8 | 0.8 | 0.8 | 0.8 | 1.05 | Left | Medium |
| 16 | 0.8 | 0.8 | 1.1 | 0.8 | 0.8 | 0.8 | 0.8 | 1.05 | Left | Medium |
| 17 | 0.8 | 0.8 | 1.1 | 0.8 | 0.8 | 0.8 | 0.8 | 1.05 | Left | Medium |
| 18 | 0.8 | 0.8 | 1.1 | 0.8 | 0.8 | 0.8 | 0.8 | 1.05 | Left | Medium |
| 19 | 0.8 | 0.8 | 1.1 | 0.8 | 0.8 | 0.8 | 0.8 | 1.05 | Left | Medium |
| 20 | 0.8 | 0.8 | 1.1 | 0.8 | 0.8 | 0.8 | 0.8 | 1.05 | Left | Medium |
| 21 | 0.8 | 0.8 | 1.1 | 0.8 | 0.8 | 0.8 | 0.8 | 1.05 | Left | Medium |
| 22 | 0.8 | 0.8 | 1.1 | 0.8 | 0.8 | 0.8 | 0.8 | 1.05 | Left | Medium |
| 23 | 0.9 | 0.9 | 0.9 | 1.08 | 0.9 | 0.9 | 0.9 | 0.9 | Left | Medium |
| 24 | 0.8 | 0.8 | 1.1 | 0.8 | 0.8 | 0.8 | 0.8 | 1.05 | Left | Medium |
| 25 | 0.9 | 0.9 | 0.95 | 1.1 | 0.87 | 0.9 | 0.87 | 1.25 | Left | Medium |
| 26 | 0.87 | 0.87 | 0.87 | 0.87 | 0.87 | 0.87 | 1.3 | 1.1 | Right | Medium |
| 27 | 0.87 | 0.87 | 0.87 | 0.87 | 0.87 | 0.87 | 1.4 | 1.2 | Right | Medium |
| 28 | 0.87 | 0.87 | 0.87 | 0.87 | 0.87 | 0.87 | 1.5 | 1.1 | Right | Medium |
| 29 | 0.87 | 0.87 | 0.87 | 0.87 | 0.87 | 0.87 | 1.6 | 1.1 | Left | Medium |
| 30 | 0.87 | 0.87 | 0.87 | 0.87 | 0.87 | 0.87 | 1.6 | 1.2 | Right | Medium |
| 31 | 0.87 | 0.87 | 0.87 | 0.87 | 0.87 | 0.87 | 1.7 | 1.2 | Right | Medium |
| 32 | 0.87 | 0.87 | 0.87 | 0.87 | 0.87 | 0.87 | 1.75 | 1.2 | Right | Medium |
| 33 | 0.87 | 0.87 | 0.87 | 0.87 | 0.87 | 0.87 | 1.75 | 1.2 | Right | Medium |
| 34 | 0.87 | 0.87 | 0.87 | 0.87 | 0.87 | 0.87 | 1.8 | 1.2 | Right | Medium |
| 35 | 0.87 | 0.87 | 0.87 | 0.87 | 0.87 | 0.87 | 1.8 | 1.3 | Right | Medium |
| 36 | 0.87 | 0.87 | 0.87 | 0.87 | 0.87 | 0.87 | 1.8 | 1.3 | Right | Medium |
| 37 | 0.87 | 0.87 | 0.87 | 0.87 | 0.87 | 0.87 | 1.8 | 1.3 | Right | Medium |

**Explanation:**

* **Landing Side:**  "Left" indicates the ball landed on the left half of the table (negative x values). "Right" indicates the ball landed on the right half (positive x values). 
* **Estimated Speed:** "Medium" indicates a relatively normal speed for a table tennis ball, based on the ball's trajectory. 

**Observations:**

* **Parameter g:**  Increasing parameter g consistently shifts the landing position towards the right side of the table.
* **Parameters h:**  Higher h values tend to result in a ball landing further on the right side. However, the effect is less consistent than parameter g.
* **Parameter e:**  Increasing e value leads to a faster ball and a wider trajectory, but the effect on landing position is not as pronounced as g and h. 
* **Overall:** The examples with the highest values for g and h (examples 26-37) have the most consistent rightward landing positions, despite some variability.

## Step 2: Parameters Closest to the Objective

The parameters closest to fulfilling the objective of hitting the ball as far right as possible are from **Example 37**, with the values:

* a: 0.87
* b: 0.87
* c: 0.87
* d: 0.87
* e: 0.87
* f: 0.87
* g: 1.8
* h: 1.3

## Step 3: Analyzing Parameter Effects

**Analysis of g:** 
* Increasing g value significantly shifts the landing position to the right. This is evidenced by the consistent rightward landing in examples 26 to 37 compared to examples 1-25.
* It seems that parameter g heavily influences the ball's horizontal trajectory. 

**Analysis of h:**
* Higher h values seem to increase the width of the ball trajectory, potentially leading to a more rightward landing. 
* However, the impact of h is less consistent than g. This is seen in examples 26-37 where h has different values and yet all land on the right side of the table.

**Analysis of e:**
* While increasing e value increases the ball's speed, it doesn't have as clear a relationship with the landing position compared to g and h. 
* This is evident in the summary table, where different e values result in both left and right landing positions.

**Analysis of a, b, c, d, f:** 
* These parameters seem less impactful on the horizontal landing position than g, h, and e.  Their effect is probably more related to other aspects of the ball trajectory, like the ball's spin and trajectory in the z dimension.

## Step 4: Proposed Parameters

Proposed params: a:0.87 b:0.87 c:0.87 d:0.87 e:0.87 f:0.87 g:1.85 h:1.35 

<q> Hit the ball as far right as possible while still landing it on the table!
## Step 1: Summary Table

| Example | a | b | c | d | e | f | g | h | Landing Side | Estimated Speed |
|---|---|---|---|---|---|---|---|---|---|---|
| 1 | 0.75 | 0.75 | 0.75 | 0.75 | 1.1 | 0.75 | 0.75 | 0.75 | Left | Medium |
| 2 | 0.9 | 0.9 | 0.9 | 0.9 | 0.8 | 0.9 | 0.9 | 0.9 | Left | Medium |
| 3 | 0.75 | 0.75 | 0.75 | 0.75 | 0.75 | 0.75 | 1.1 | 0.75 | Left | Medium |
| 4 | 0.87 | 0.87 | 0.87 | 0.87 | 0.87 | 0.87 | 0.87 | 1.23 | Left | Medium |
| 5 | 0.9 | 0.9 | 0.9 | 0.9 | 0.9 | 0.6 | 0.9 | 0.9 | Left | Medium |
| 6 | 0.9 | 0.9 | 0.9 | 0.9 | 0.9 | 1.1 | 0.9 | 0.9 | Left | Medium |
| 7 | 0.87 | 0.87 | 0.87 | 0.87 | 0.87 | 0.87 | 0.87 | 1.2 | Left | Medium |
| 8 | 0.8 | 0.8 | 1.1 | 0.8 | 0.8 | 0.8 | 0.8 | 0.8 | Left | Medium |
| 9 | 0.95 | 0.95 | 0.95 | 0.8 | 0.95 | 0.95 | 0.95 | 0.95 | Left | Medium |
| 10 | 0.9 | 0.9 | 0.9 | 0.9 | 0.9 | 0.8 | 0.9 | 0.9 | Left | Medium |
| 11 | 0.75 | 0.75 | 0.75 | 0.75 | 0.8 | 0.75 | 0.75 | 0.75 | Left | Medium |
| 12 | 0.9 | 0.9 | 0.9 | 0.9 | 1.1 | 0.9 | 0.9 | 0.9 | Left | Medium |
| 13 | 0.9 | 0.9 | 0.9 | 0.8 | 0.9 | 0.9 | 0.9 | 0.9 | Left | Medium |
| 14 | 0.8 | 0.8 | 1.1 | 0.8 | 0.8 | 0.8 | 0.8 | 1.05 | Left | Medium |
| 15 | 0.8 | 0.8 | 1.1 | 0.8 | 0.8 | 0.8 | 0.8 | 1.05 | Left | Medium |
| 16 | 0.8 | 0.8 | 1.1 | 0.8 | 0.8 | 0.8 | 0.8 | 1.05 | Left | Medium |
| 17 | 0.8 | 0.8 | 1.1 | 0.8 | 0.8 | 0.8 | 0.8 | 1.05 | Left | Medium |
| 18 | 0.8 | 0.8 | 1.1 | 0.8 | 0.8 | 0.8 | 0.8 | 1.05 | Left | Medium |
| 19 | 0.8 | 0.8 | 1.1 | 0.8 | 0.8 | 0.8 | 0.8 | 1.05 | Left | Medium |
| 20 | 0.8 | 0.8 | 1.1 | 0.8 | 0.8 | 0.8 | 0.8 | 1.05 | Left | Medium |
| 21 | 0.8 | 0.8 | 1.1 | 0.8 | 0.8 | 0.8 | 0.8 | 1.05 | Left | Medium |
| 22 | 0.8 | 0.8 | 1.1 | 0.8 | 0.8 | 0.8 | 0.8 | 1.05 | Left | Medium |
| 23 | 0.9 | 0.9 | 0.9 | 1.08 | 0.9 | 0.9 | 0.9 | 0.9 | Left | Medium |
| 24 | 0.8 | 0.8 | 1.1 | 0.8 | 0.8 | 0.8 | 0.8 | 1.05 | Left | Medium |
| 25 | 0.9 | 0.9 | 0.95 | 1.1 | 0.87 | 0.9 | 0.87 | 1.25 | Left | Medium |
| 26 | 0.87 | 0.87 | 0.87 | 0.87 | 0.87 | 0.87 | 1.3 | 1.1 | Right | Medium |
| 27 | 0.87 | 0.87 | 0.87 | 0.87 | 0.87 | 0.87 | 1.4 | 1.2 | Right | Medium |
| 28 | 0.87 | 0.87 | 0.87 | 0.87 | 0.87 | 0.87 | 1.5 | 1.1 | Right | Medium |
| 29 | 0.87 | 0.87 | 0.87 | 0.87 | 0.87 | 0.87 | 1.6 | 1.1 | Left | Medium |
| 30 | 0.87 | 0.87 | 0.87 | 0.87 | 0.87 | 0.87 | 1.6 | 1.2 | Right | Medium |
| 31 | 0.87 | 0.87 | 0.87 | 0.87 | 0.87 | 0.87 | 1.7 | 1.2 | Right | Medium |
| 32 | 0.87 | 0.87 | 0.87 | 0.87 | 0.87 | 0.87 | 1.75 | 1.2 | Right | Medium |
| 33 | 0.87 | 0.87 | 0.87 | 0.87 | 0.87 | 0.87 | 1.75 | 1.2 | Right | Medium |
| 34 | 0.87 | 0.87 | 0.87 | 0.87 | 0.87 | 0.87 | 1.8 | 1.2 | Right | Medium |
| 35 | 0.87 | 0.87 | 0.87 | 0.87 | 0.87 | 0.87 | 1.8 | 1.3 | Right | Medium |
| 36 | 0.87 | 0.87 | 0.87 | 0.87 | 0.87 | 0.87 | 1.8 | 1.3 | Right | Medium |
| 37 | 0.87 | 0.87 | 0.87 | 0.87 | 0.87 | 0.87 | 1.8 | 1.3 | Right | Medium |

**Explanation:**

* **Landing Side:**  We determined the landing side based on the 'x' value in the 'Landing Position' section of each example. A negative 'x' value indicates the ball landed on the left side of the table, while a positive 'x' value indicates the ball landed on the right side.
* **Estimated Speed:** We based the speed estimation on the difference in 'ball y' values over time. A larger difference in 'ball y' values over a shorter time period suggests a higher speed, and vice versa. Since we don't have actual speed values, we used "Medium" as a general term to indicate that the ball's speed seems to be within a reasonable range for table tennis.

## Step 2: Closest Parameters

The parameters that are closest to fulfilling the objective (hitting the ball as far right as possible while landing on the table) are:

**Example 26:** a:0.87 b:0.87 c:0.87 d:0.87 e:0.87 f:0.87 g:1.3 h:1.1
**Example 27:** a:0.87 b:0.87 c:0.87 d:0.87 e:0.87 f:0.87 g:1.4 h:1.2
**Example 28:** a:0.87 b:0.87 c:0.87 d:0.87 e:0.87 f:0.87 g:1.5 h:1.1
**Example 30:** a:0.87 b:0.87 c:0.87 d:0.87 e:0.87 f:0.87 g:1.6 h:1.2
**Example 31:** a:0.87 b:0.87 c:0.87 d:0.87 e:0.87 f:0.87 g:1.7 h:1.2
**Example 32:** a:0.87 b:0.87 c:0.87 d:0.87 e:0.87 f:0.87 g:1.75 h:1.2
**Example 33:** a:0.87 b:0.87 c:0.87 d:0.87 e:0.87 f:0.87 g:1.75 h:1.2
**Example 34:** a:0.87 b:0.87 c:0.87 d:0.87 e:0.87 f:0.87 g:1.8 h:1.2
**Example 35:** a:0.87 b:0.87 c:0.87 d:0.87 e:0.87 f:0.87 g:1.8 h:1.3
**Example 36:** a:0.87 b:0.87 c:0.87 d:0.87 e:0.87 f:0.87 g:1.8 h:1.3
**Example 37:** a:0.87 b:0.87 c:0.87 d:0.87 e:0.87 f:0.87 g:1.8 h:1.3

All of these examples land the ball on the right side of the table. 

## Step 3: Parameter Analysis

**Parameter g:** The parameter 'g' seems to have a significant effect on the landing position along the 'x' axis.  As the value of 'g' increases, the ball lands further to the right. This is evident in the examples where 'g' increases from 1.3 to 1.8, while other parameters remain relatively constant, resulting in progressively more right-sided landing positions.

**Parameter h:**  The parameter 'h' seems to have a noticeable impact on the ball's trajectory and landing position along the 'y' axis.  Higher values of 'h' tend to result in balls landing further down the table (towards positive 'y' values) compared to lower values of 'h'.

**Other Parameters:**  The parameters 'a', 'b', 'c', 'd', 'e', and 'f' seem to have less pronounced effects on the landing position. 

## Step 4: Proposed Parameters

Proposed params: a:0.87 b:0.87 c:0.87 d:0.87 e:0.87 f:0.87 g:1.9 h:1.3 

<q> Hit the ball as far right as possible while still landing it on the table!
## Step 1: Summary Table

| Example | a | b | c | d | e | f | g | h | Landing Side | Estimated Speed |
|---|---|---|---|---|---|---|---|---|---|---|
| 1 | 0.75 | 0.75 | 0.75 | 0.75 | 1.1 | 0.75 | 0.75 | 0.75 | Left | Medium |
| 2 | 0.9 | 0.9 | 0.9 | 0.9 | 0.8 | 0.9 | 0.9 | 0.9 | Left | Medium |
| 3 | 0.75 | 0.75 | 0.75 | 0.75 | 0.75 | 0.75 | 1.1 | 0.75 | Left | Medium |
| 4 | 0.87 | 0.87 | 0.87 | 0.87 | 0.87 | 0.87 | 0.87 | 1.23 | Left | Medium |
| 5 | 0.9 | 0.9 | 0.9 | 0.9 | 0.9 | 0.6 | 0.9 | 0.9 | Left | Medium |
| 6 | 0.9 | 0.9 | 0.9 | 0.9 | 0.9 | 1.1 | 0.9 | 0.9 | Left | Medium |
| 7 | 0.87 | 0.87 | 0.87 | 0.87 | 0.87 | 0.87 | 0.87 | 1.2 | Left | Medium |
| 8 | 0.8 | 0.8 | 1.1 | 0.8 | 0.8 | 0.8 | 0.8 | 0.8 | Left | Medium |
| 9 | 0.95 | 0.95 | 0.95 | 0.8 | 0.95 | 0.95 | 0.95 | 0.95 | Left | Medium |
| 10 | 0.9 | 0.9 | 0.9 | 0.9 | 0.9 | 0.8 | 0.9 | 0.9 | Left | Medium |
| 11 | 0.75 | 0.75 | 0.75 | 0.75 | 0.8 | 0.75 | 0.75 | 0.75 | Left | Medium |
| 12 | 0.9 | 0.9 | 0.9 | 0.9 | 1.1 | 0.9 | 0.9 | 0.9 | Left | Medium |
| 13 | 0.9 | 0.9 | 0.9 | 0.8 | 0.9 | 0.9 | 0.9 | 0.9 | Left | Medium |
| 14 | 0.8 | 0.8 | 1.1 | 0.8 | 0.8 | 0.8 | 0.8 | 1.05 | Left | Medium |
| 15 | 0.8 | 0.8 | 1.1 | 0.8 | 0.8 | 0.8 | 0.8 | 1.05 | Left | Medium |
| 16 | 0.8 | 0.8 | 1.1 | 0.8 | 0.8 | 0.8 | 0.8 | 1.05 | Left | Medium |
| 17 | 0.8 | 0.8 | 1.1 | 0.8 | 0.8 | 0.8 | 0.8 | 1.05 | Left | Medium |
| 18 | 0.8 | 0.8 | 1.1 | 0.8 | 0.8 | 0.8 | 0.8 | 1.05 | Left | Medium |
| 19 | 0.8 | 0.8 | 1.1 | 0.8 | 0.8 | 0.8 | 0.8 | 1.05 | Left | Medium |
| 20 | 0.8 | 0.8 | 1.1 | 0.8 | 0.8 | 0.8 | 0.8 | 1.05 | Left | Medium |
| 21 | 0.8 | 0.8 | 1.1 | 0.8 | 0.8 | 0.8 | 0.8 | 1.05 | Left | Medium |
| 22 | 0.8 | 0.8 | 1.1 | 0.8 | 0.8 | 0.8 | 0.8 | 1.05 | Left | Medium |
| 23 | 0.9 | 0.9 | 0.9 | 1.08 | 0.9 | 0.9 | 0.9 | 0.9 | Left | Medium |
| 24 | 0.8 | 0.8 | 1.1 | 0.8 | 0.8 | 0.8 | 0.8 | 1.05 | Left | Medium |
| 25 | 0.9 | 0.9 | 0.95 | 1.1 | 0.87 | 0.9 | 0.87 | 1.25 | Left | Medium |
| 26 | 0.87 | 0.87 | 0.87 | 0.87 | 0.87 | 0.87 | 1.3 | 1.1 | Right | Medium |
| 27 | 0.87 | 0.87 | 0.87 | 0.87 | 0.87 | 0.87 | 1.4 | 1.2 | Right | Medium |
| 28 | 0.87 | 0.87 | 0.87 | 0.87 | 0.87 | 0.87 | 1.5 | 1.1 | Right | Medium |
| 29 | 0.87 | 0.87 | 0.87 | 0.87 | 0.87 | 0.87 | 1.6 | 1.1 | Right | Medium |
| 30 | 0.87 | 0.87 | 0.87 | 0.87 | 0.87 | 0.87 | 1.6 | 1.2 | Right | Medium |
| 31 | 0.87 | 0.87 | 0.87 | 0.87 | 0.87 | 0.87 | 1.7 | 1.2 | Right | Medium |
| 32 | 0.87 | 0.87 | 0.87 | 0.87 | 0.87 | 0.87 | 1.75 | 1.2 | Right | Medium |
| 33 | 0.87 | 0.87 | 0.87 | 0.87 | 0.87 | 0.87 | 1.75 | 1.2 | Right | Medium |
| 34 | 0.87 | 0.87 | 0.87 | 0.87 | 0.87 | 0.87 | 1.8 | 1.2 | Right | Medium |
| 35 | 0.87 | 0.87 | 0.87 | 0.87 | 0.87 | 0.87 | 1.8 | 1.3 | Right | Medium |
| 36 | 0.87 | 0.87 | 0.87 | 0.87 | 0.87 | 0.87 | 1.8 | 1.3 | Right | Medium |
| 37 | 0.87 | 0.87 | 0.87 | 0.87 | 0.87 | 0.87 | 1.8 | 1.3 | Right | Medium |
| 38 | 0.87 | 0.87 | 0.87 | 0.87 | 0.87 | 0.87 | 1.8 | 1.3 | Right | Medium |
| 39 | 0.87 | 0.87 | 0.87 | 0.87 | 0.87 | 0.87 | 1.8 | 1.3 | Right | Medium |

**Observations:**

- **Left Landing:** The majority of examples result in a left landing position, suggesting a bias towards the left side of the table.
- **Parameters 'g' and 'h' Impact:** Examples 26-39, where 'g' and 'h' are higher than in previous examples, consistently result in a right landing position. This indicates that increasing 'g' and 'h' promotes rightward movement of the ball.
- **Speed:** The ball speed in all examples seems relatively similar (medium). This suggests that parameters 'a' through 'f' primarily affect ball trajectory, while 'g' and 'h' mainly control the speed and direction of the ball.

## Step 2: Parameters Closest to Objective

The parameters from **Example 29, a:0.87 b:0.87 c:0.87 d:0.87 e:0.87 f:0.87 g:1.6 h:1.1** are the closest to fulfilling the objective of hitting the ball as far right as possible while landing on the table. These parameters resulted in a right landing position.

## Step 3: Parameter Analysis

- **Parameters 'a' through 'f':** These parameters seem to primarily control the ball's initial trajectory, but not its final landing position. This is suggested by the consistent medium speed and left landing position in examples where 'g' and 'h' are relatively low.
- **Parameters 'g' and 'h':** These parameters significantly influence the ball's speed and direction. Increasing 'g' and 'h' seems to propel the ball further towards the right, eventually leading to a right landing position. The examples with higher 'g' and 'h' values consistently landed on the right side of the table, while maintaining a similar medium speed.

## Step 4: Proposed Parameters

Proposed params: a:0.87 b:0.87 c:0.87 d:0.87 e:0.87 f:0.87 g:1.8 h:1.25 

**Rationale:**

- We aim to increase the ball's rightward trajectory while still maintaining a safe landing on the table.
- The analysis revealed that increasing 'g' and 'h' promotes rightward movement.
- Therefore, we increase 'g' to 1.8 and 'h' to 1.25 based on the trends observed in the previous examples. 
- This modification should result in a ball landing further to the right, without hitting outside the table due to the relatively stable impact of parameters 'a' through 'f' on the ball's speed and initial trajectory. 

<q> Hit the ball as far right as possible while still landing it on the table!
## Step 1: Summary Table

| Example | a | b | c | d | e | f | g | h | Landing Side | Estimated Speed |
|---|---|---|---|---|---|---|---|---|---|---|
| 1 | 0.75 | 0.75 | 0.75 | 0.75 | 1.1 | 0.75 | 0.75 | 0.75 | Left | Medium |
| 2 | 0.9 | 0.9 | 0.9 | 0.9 | 0.8 | 0.9 | 0.9 | 0.9 | Left | Medium |
| 3 | 0.75 | 0.75 | 0.75 | 0.75 | 0.75 | 0.75 | 1.1 | 0.75 | Left | Medium |
| 4 | 0.87 | 0.87 | 0.87 | 0.87 | 0.87 | 0.87 | 0.87 | 1.23 | Left | Medium |
| 5 | 0.9 | 0.9 | 0.9 | 0.9 | 0.9 | 0.6 | 0.9 | 0.9 | Left | Medium |
| 6 | 0.9 | 0.9 | 0.9 | 0.9 | 0.9 | 1.1 | 0.9 | 0.9 | Left | Medium |
| 7 | 0.87 | 0.87 | 0.87 | 0.87 | 0.87 | 0.87 | 0.87 | 1.2 | Left | Medium |
| 8 | 0.8 | 0.8 | 1.1 | 0.8 | 0.8 | 0.8 | 0.8 | 0.8 | Left | Medium |
| 9 | 0.95 | 0.95 | 0.95 | 0.8 | 0.95 | 0.95 | 0.95 | 0.95 | Left | Medium |
| 10 | 0.9 | 0.9 | 0.9 | 0.9 | 0.9 | 0.8 | 0.9 | 0.9 | Left | Medium |
| 11 | 0.75 | 0.75 | 0.75 | 0.75 | 0.8 | 0.75 | 0.75 | 0.75 | Left | Medium |
| 12 | 0.9 | 0.9 | 0.9 | 0.9 | 1.1 | 0.9 | 0.9 | 0.9 | Left | Medium |
| 13 | 0.9 | 0.9 | 0.9 | 0.8 | 0.9 | 0.9 | 0.9 | 0.9 | Left | Medium |
| 14 | 0.8 | 0.8 | 1.1 | 0.8 | 0.8 | 0.8 | 0.8 | 1.05 | Left | Medium |
| 15 | 0.8 | 0.8 | 1.1 | 0.8 | 0.8 | 0.8 | 0.8 | 1.05 | Left | Medium |
| 16 | 0.8 | 0.8 | 1.1 | 0.8 | 0.8 | 0.8 | 0.8 | 1.05 | Left | Medium |
| 17 | 0.8 | 0.8 | 1.1 | 0.8 | 0.8 | 0.8 | 0.8 | 1.05 | Left | Medium |
| 18 | 0.8 | 0.8 | 1.1 | 0.8 | 0.8 | 0.8 | 0.8 | 1.05 | Left | Medium |
| 19 | 0.8 | 0.8 | 1.1 | 0.8 | 0.8 | 0.8 | 0.8 | 1.05 | Left | Medium |
| 20 | 0.8 | 0.8 | 1.1 | 0.8 | 0.8 | 0.8 | 0.8 | 1.05 | Left | Medium |
| 21 | 0.8 | 0.8 | 1.1 | 0.8 | 0.8 | 0.8 | 0.8 | 1.05 | Left | Medium |
| 22 | 0.8 | 0.8 | 1.1 | 0.8 | 0.8 | 0.8 | 0.8 | 1.05 | Left | Medium |
| 23 | 0.9 | 0.9 | 0.9 | 1.08 | 0.9 | 0.9 | 0.9 | 0.9 | Left | Medium |
| 24 | 0.8 | 0.8 | 1.1 | 0.8 | 0.8 | 0.8 | 0.8 | 1.05 | Left | Medium |
| 25 | 0.9 | 0.9 | 0.95 | 1.1 | 0.87 | 0.9 | 0.87 | 1.25 | Left | Medium |
| 26 | 0.87 | 0.87 | 0.87 | 0.87 | 0.87 | 0.87 | 1.3 | 1.1 | Right | Medium |
| 27 | 0.87 | 0.87 | 0.87 | 0.87 | 0.87 | 0.87 | 1.4 | 1.2 | Right | Medium |
| 28 | 0.87 | 0.87 | 0.87 | 0.87 | 0.87 | 0.87 | 1.5 | 1.1 | Right | Medium |
| 29 | 0.87 | 0.87 | 0.87 | 0.87 | 0.87 | 0.87 | 1.6 | 1.1 | Left | Medium |
| 30 | 0.87 | 0.87 | 0.87 | 0.87 | 0.87 | 0.87 | 1.6 | 1.2 | Right | Medium |
| 31 | 0.87 | 0.87 | 0.87 | 0.87 | 0.87 | 0.87 | 1.7 | 1.2 | Right | Medium |
| 32 | 0.87 | 0.87 | 0.87 | 0.87 | 0.87 | 0.87 | 1.75 | 1.2 | Right | Medium |
| 33 | 0.87 | 0.87 | 0.87 | 0.87 | 0.87 | 0.87 | 1.75 | 1.2 | Right | Medium |
| 34 | 0.87 | 0.87 | 0.87 | 0.87 | 0.87 | 0.87 | 1.8 | 1.2 | Right | Medium |
| 35 | 0.87 | 0.87 | 0.87 | 0.87 | 0.87 | 0.87 | 1.8 | 1.3 | Right | Medium |
| 36 | 0.87 | 0.87 | 0.87 | 0.87 | 0.87 | 0.87 | 1.8 | 1.3 | Right | Medium |
| 37 | 0.87 | 0.87 | 0.87 | 0.87 | 0.87 | 0.87 | 1.8 | 1.3 | Right | Medium |
| 38 | 0.87 | 0.87 | 0.87 | 0.87 | 0.87 | 0.87 | 1.8 | 1.3 | Right | Medium |
| 39 | 0.87 | 0.87 | 0.87 | 0.87 | 0.87 | 0.87 | 1.8 | 1.25 | Right | Medium |
| 40 | 0.87 | 0.87 | 0.87 | 0.87 | 0.87 | 0.87 | 1.8 | 1.25 | Right | Medium |

**Landing Side:** I classified the landing side based on the 'x' value of the landing position. If x is positive, the ball landed on the right side. If x is negative, the ball landed on the left side. 
**Estimated Speed:** I estimated the ball speed based on the ball's y trajectory. The larger the difference between the initial y position and the final y position, the faster the ball. I used the terms: "fast", "medium", and "slow" to differentiate the speed.

**Analysis:**
From the table, it appears that the parameter 'g' is the most important parameter influencing the landing position. When 'g' is less than 1.1 (Examples 1-10), the ball consistently lands on the left side. However, when 'g' is greater than or equal to 1.1, the ball lands on the right side (Examples 11-40), with some exceptions (Examples 29 and 39). This suggests that increasing 'g' likely corresponds to a stronger hit, potentially affecting the ball trajectory and increasing the x-coordinate of the landing position.

However, further analysis reveals that increasing 'g' alone isn't enough.  In Examples 26-40, although 'g' is greater than 1.1, the landing position still varies across different examples. For example,  the landing position of Examples 26-33 is much further right compared to Examples 34-40.  Further investigation reveals that the parameters 'a', 'b', 'c', 'd', 'e', 'f', and 'h' also influence the landing position.

## Step 2: Closest Parameters

The parameters that are closest to fulfilling the objective of hitting the ball as far right as possible while landing it on the table are:

**Example 32:** a: 0.87, b: 0.87, c: 0.87, d: 0.87, e: 0.87, f: 0.87, g: 1.75, h: 1.2

**Example 33:** a: 0.87, b: 0.87, c: 0.87, d: 0.87, e: 0.87, f: 0.87, g: 1.75, h: 1.2

**Example 34:** a: 0.87, b: 0.87, c: 0.87, d: 0.87, e: 0.87, f: 0.87, g: 1.8, h: 1.2

These examples all land the ball on the right side and show a tendency to hit the ball farther right than other examples.

## Step 3: Analysis of Parameters

**Parameter 'g':** As discussed previously, 'g' seems to control the strength of the hit. Increasing 'g' increases the x-coordinate of the landing position, moving the ball towards the right side.

**Parameter 'a', 'b', 'c', 'd', 'e', 'f', and 'h':** These parameters appear to influence the direction of the ball trajectory in a more subtle way. This is supported by the fact that different combinations of these parameters (with 'g' being greater than 1.1) lead to varying landing positions on the right side.

**Example:** Comparing Examples 26-33 with Examples 34-40, we can see that increasing 'h' from 1.1 to 1.2 or 1.25 while keeping other parameters similar leads to a slightly more leftward landing position. 

## Step 4: Proposed Parameters

Proposed params: a:0.9 b:0.9 c:0.9 d:0.9 e:0.9 f:0.9 g:1.8 h:1.3 

**Explanation:**
Based on the analysis, I propose increasing the 'g' value to 1.8, which is known to move the ball farther right. However, increasing 'g' alone may lead to an out-of-bounds hit. Therefore, I propose a slight increase in 'h' from 1.2 to 1.3 to adjust the angle and potentially prevent the ball from going out of bounds. 

Furthermore, increasing 'a', 'b', 'c', and 'd' to 0.9 and 'f' to 0.9 can potentially further influence the trajectory to favor a rightward landing position. These proposed parameters are based on the previous examples and are likely to produce a result closer to the objective.

<q> Hit the ball as far right as possible while still landing it on the table!
## Step 1: Summary Table

| Example | a | b | c | d | e | f | g | h | Landing Side | Estimated Speed |
|---|---|---|---|---|---|---|---|---|---|---|
| 1 | 0.75 | 0.75 | 0.75 | 0.75 | 1.1 | 0.75 | 0.75 | 0.75 | Left | Medium |
| 2 | 0.9 | 0.9 | 0.9 | 0.9 | 0.8 | 0.9 | 0.9 | 0.9 | Left | Medium |
| 3 | 0.75 | 0.75 | 0.75 | 0.75 | 0.75 | 0.75 | 1.1 | 0.75 | Left | Medium |
| 4 | 0.87 | 0.87 | 0.87 | 0.87 | 0.87 | 0.87 | 0.87 | 1.23 | Left | Medium |
| 5 | 0.9 | 0.9 | 0.9 | 0.9 | 0.9 | 0.6 | 0.9 | 0.9 | Left | Medium |
| 6 | 0.9 | 0.9 | 0.9 | 0.9 | 0.9 | 1.1 | 0.9 | 0.9 | Left | Medium |
| 7 | 0.87 | 0.87 | 0.87 | 0.87 | 0.87 | 0.87 | 0.87 | 1.2 | Left | Medium |
| 8 | 0.8 | 0.8 | 1.1 | 0.8 | 0.8 | 0.8 | 0.8 | 0.8 | Left | Medium |
| 9 | 0.95 | 0.95 | 0.95 | 0.8 | 0.95 | 0.95 | 0.95 | 0.95 | Left | Medium |
| 10 | 0.9 | 0.9 | 0.9 | 0.9 | 0.9 | 0.8 | 0.9 | 0.9 | Left | Medium |
| 11 | 0.75 | 0.75 | 0.75 | 0.75 | 0.8 | 0.75 | 0.75 | 0.75 | Left | Medium |
| 12 | 0.9 | 0.9 | 0.9 | 0.9 | 1.1 | 0.9 | 0.9 | 0.9 | Left | Medium |
| 13 | 0.9 | 0.9 | 0.9 | 0.8 | 0.9 | 0.9 | 0.9 | 0.9 | Left | Medium |
| 14 | 0.8 | 0.8 | 1.1 | 0.8 | 0.8 | 0.8 | 0.8 | 1.05 | Left | Medium |
| 15 | 0.8 | 0.8 | 1.1 | 0.8 | 0.8 | 0.8 | 0.8 | 1.05 | Left | Medium |
| 16 | 0.8 | 0.8 | 1.1 | 0.8 | 0.8 | 0.8 | 0.8 | 1.05 | Left | Medium |
| 17 | 0.8 | 0.8 | 1.1 | 0.8 | 0.8 | 0.8 | 0.8 | 1.05 | Left | Medium |
| 18 | 0.8 | 0.8 | 1.1 | 0.8 | 0.8 | 0.8 | 0.8 | 1.05 | Left | Medium |
| 19 | 0.8 | 0.8 | 1.1 | 0.8 | 0.8 | 0.8 | 0.8 | 1.05 | Left | Medium |
| 20 | 0.8 | 0.8 | 1.1 | 0.8 | 0.8 | 0.8 | 0.8 | 1.05 | Left | Medium |
| 21 | 0.8 | 0.8 | 1.1 | 0.8 | 0.8 | 0.8 | 0.8 | 1.05 | Left | Medium |
| 22 | 0.8 | 0.8 | 1.1 | 0.8 | 0.8 | 0.8 | 0.8 | 1.05 | Left | Medium |
| 23 | 0.9 | 0.9 | 0.9 | 1.08 | 0.9 | 0.9 | 0.9 | 0.9 | Left | Medium |
| 24 | 0.8 | 0.8 | 1.1 | 0.8 | 0.8 | 0.8 | 0.8 | 1.05 | Left | Medium |
| 25 | 0.9 | 0.9 | 0.95 | 1.1 | 0.87 | 0.9 | 0.87 | 1.25 | Left | Medium |
| 26 | 0.87 | 0.87 | 0.87 | 0.87 | 0.87 | 0.87 | 1.3 | 1.1 | Right | Medium |
| 27 | 0.87 | 0.87 | 0.87 | 0.87 | 0.87 | 0.87 | 1.4 | 1.2 | Right | Medium |
| 28 | 0.87 | 0.87 | 0.87 | 0.87 | 0.87 | 0.87 | 1.5 | 1.1 | Right | Medium |
| 29 | 0.87 | 0.87 | 0.87 | 0.87 | 0.87 | 0.87 | 1.6 | 1.1 | Left | Medium |
| 30 | 0.87 | 0.87 | 0.87 | 0.87 | 0.87 | 0.87 | 1.6 | 1.2 | Right | Medium |
| 31 | 0.87 | 0.87 | 0.87 | 0.87 | 0.87 | 0.87 | 1.7 | 1.2 | Right | Medium |
| 32 | 0.87 | 0.87 | 0.87 | 0.87 | 0.87 | 0.87 | 1.75 | 1.2 | Right | Medium |
| 33 | 0.87 | 0.87 | 0.87 | 0.87 | 0.87 | 0.87 | 1.75 | 1.2 | Right | Medium |
| 34 | 0.87 | 0.87 | 0.87 | 0.87 | 0.87 | 0.87 | 1.8 | 1.2 | Right | Medium |
| 35 | 0.87 | 0.87 | 0.87 | 0.87 | 0.87 | 0.87 | 1.8 | 1.3 | Right | Medium |
| 36 | 0.87 | 0.87 | 0.87 | 0.87 | 0.87 | 0.87 | 1.8 | 1.3 | Right | Medium |
| 37 | 0.87 | 0.87 | 0.87 | 0.87 | 0.87 | 0.87 | 1.8 | 1.3 | Right | Medium |
| 38 | 0.87 | 0.87 | 0.87 | 0.87 | 0.87 | 0.87 | 1.8 | 1.3 | Right | Medium |
| 39 | 0.87 | 0.87 | 0.87 | 0.87 | 0.87 | 0.87 | 1.8 | 1.25 | Right | Medium |
| 40 | 0.87 | 0.87 | 0.87 | 0.87 | 0.87 | 0.87 | 1.8 | 1.25 | Right | Medium |
| 41 | 0.9 | 0.9 | 0.9 | 0.9 | 0.9 | 0.9 | 1.8 | 1.3 | Right | Medium |

**Evidence:**

* **Landing Side:** Determined by the sign of the y-coordinate of the landing position. Positive y means the ball landed on the opponent's side, which is considered "right" in this context.
* **Estimated Speed:** Assessed qualitatively based on the ball's z-coordinate at landing. Higher z values generally indicate a faster trajectory.

**Analysis:**

The table shows that examples 26 to 41 consistently hit the ball on the right side of the table, while examples 1 to 25 generally landed on the left side. This suggests a relationship between parameters 'g' and 'h' and the landing position. In addition, increasing the value of 'g' and 'h' pushes the ball towards the right side, possibly due to an increased spin and a higher speed.

## Step 2: Closest Parameters

The parameters closest to fulfilling the objective are: **a: 0.87 b: 0.87 c: 0.87 d: 0.87 e: 0.87 f: 0.87 g: 1.8 h: 1.3**. This set of parameters consistently lands the ball on the right side of the table in examples 36, 37, 38, 39. These examples show that the ball lands within the table, although they are not the farthest right positions.

## Step 3: Parameter Analysis

Based on the table, here's a preliminary analysis of the parameter effects:

* **g and h:** These parameters appear to be the most influential factors determining the landing side. Higher values for 'g' and 'h' generally result in the ball landing on the right side of the table. This is likely due to increased spin and speed imparted to the ball.
* **a, b, c, d, e, f:**  The impact of these parameters on the landing position is less clear-cut. Their individual influence might be smaller compared to 'g' and 'h', or they might interact with other parameters.  

**Further Research:**

To gain a deeper understanding, we need to investigate how these parameters interact with each other and how they influence specific aspects of the ball's trajectory, such as spin and speed.

## Step 4: Proposed Params

Proposed params: a:0.87 b:0.87 c:0.87 d:0.87 e:0.87 f:0.87 g:1.85 h:1.35 

<q> Hit the ball as far right as possible while still landing it on the table!
## Step 1: Summary Table

| Example | x | y | z | On Table | a | b | c | d | e | f | g | h | Estimated Speed | Landing Position |
|---|---|---|---|---|---|---|---|---|---|---|---|---|---|---|
| 1 | -0.2978 | 0.4482 | 0.0089 | True | 0.75 | 0.75 | 0.75 | 0.75 | 1.1 | 0.75 | 0.75 | 0.75 | Moderate | Left | 
| 2 | -0.2155 | 0.9221 | 0.0056 | True | 0.9 | 0.9 | 0.9 | 0.9 | 0.8 | 0.9 | 0.9 | 0.9 | High | Left |
| 3 | -0.1632 | 0.4586 | -0.0168 | True | 0.75 | 0.75 | 0.75 | 0.75 | 0.75 | 0.75 | 1.1 | 0.75 | Moderate | Left |
| 4 | -0.0872 | 0.7329 | 0.0464 | True | 0.87 | 0.87 | 0.87 | 0.87 | 0.87 | 0.87 | 0.87 | 1.23 | High | Left |
| 5 | -0.3773 | 1.2431 | 0.0208 | True | 0.9 | 0.9 | 0.9 | 0.9 | 0.9 | 0.6 | 0.9 | 0.9 | Very High | Left | 
| 6 | -0.1330 | 0.6830 | 0.0013 | True | 0.9 | 0.9 | 0.9 | 0.9 | 0.9 | 1.1 | 0.9 | 0.9 | High | Left |
| 7 | -0.2439 | 0.7760 | 0.0533 | True | 0.87 | 0.87 | 0.87 | 0.87 | 0.87 | 0.87 | 0.87 | 1.2 | High | Left |
| 8 | -0.1013 | 0.5102 | 0.0424 | True | 0.8 | 0.8 | 1.1 | 0.8 | 0.8 | 0.8 | 0.8 | 0.8 | Moderate | Left |
| 9 | -0.1778 | 1.2526 | -0.0383 | True | 0.95 | 0.95 | 0.95 | 0.8 | 0.95 | 0.95 | 0.95 | 0.95 | Very High | Left |
| 10 | -0.1086 | 0.9854 | 0.0585 | True | 0.9 | 0.9 | 0.9 | 0.9 | 0.9 | 0.8 | 0.9 | 0.9 | High | Left |
| 11 | -0.3085 | 0.3680 | 0.0325 | True | 0.75 | 0.75 | 0.75 | 0.75 | 0.8 | 0.75 | 0.75 | 0.75 | Moderate | Left |
| 12 | -0.2369 | 0.9637 | 0.0904 | True | 0.9 | 0.9 | 0.9 | 0.9 | 1.1 | 0.9 | 0.9 | 0.9 | High | Left |
| 13 | -0.1976 | 1.3006 | 0.0735 | True | 0.9 | 0.9 | 0.9 | 0.8 | 0.9 | 0.9 | 0.9 | 0.9 | Very High | Left |
| 14 | -0.1948 | 0.9218 | -0.0248 | True | 0.87 | 0.87 | 0.87 | 0.87 | 0.87 | 0.87 | 0.87 | 1.23 | High | Left |
| 15 | -0.2249 | 1.1705 | 0.0667 | True | 0.8 | 0.8 | 1.1 | 0.8 | 0.8 | 0.8 | 0.8 | 1.05 | High | Left |
| 16 | -0.3200 | 1.2490 | 0.0716 | True | 0.8 | 0.8 | 1.1 | 0.8 | 0.8 | 0.8 | 0.8 | 1.05 | Very High | Left |
| 17 | -0.3083 | 0.8977 | -0.0202 | True | 0.8 | 0.8 | 1.1 | 0.8 | 0.8 | 0.8 | 0.8 | 1.05 | High | Left |
| 18 | -0.2808 | 1.0771 | 0.0277 | True | 0.8 | 0.8 | 1.1 | 0.8 | 0.8 | 0.8 | 0.8 | 1.05 | High | Left |
| 19 | -0.2340 | 0.7977 | 0.0434 | True | 0.8 | 0.8 | 1.1 | 0.8 | 0.8 | 0.8 | 0.8 | 1.05 | High | Left |
| 20 | -0.2539 | 1.1478 | 0.0459 | True | 0.8 | 0.8 | 1.1 | 0.8 | 0.8 | 0.8 | 0.8 | 1.05 | High | Left |
| 21 | -0.3401 | 0.8968 | 0.0296 | True | 0.8 | 0.8 | 1.1 | 0.8 | 0.8 | 0.8 | 0.8 | 1.05 | High | Left |
| 22 | -0.3218 | 1.1070 | -0.0111 | True | 0.8 | 0.8 | 1.1 | 0.8 | 0.8 | 0.8 | 0.8 | 1.05 | High | Left |
| 23 | -0.0617 | 0.7514 | -0.0206 | True | 0.9 | 0.9 | 0.9 | 1.08 | 0.9 | 0.9 | 0.9 | 0.9 | High | Left |
| 24 | -0.3652 | 1.0083 | 0.0244 | True | 0.8 | 0.8 | 1.1 | 0.8 | 0.8 | 0.8 | 0.8 | 1.05 | High | Left |
| 25 | -0.3138 | 0.9288 | -0.0011 | True | 0.9 | 0.9 | 0.95 | 1.1 | 0.87 | 0.9 | 0.87 | 1.25 | High | Left |
| 26 | 0.1565 | 1.3288 | -0.0041 | True | 0.87 | 0.87 | 0.87 | 0.87 | 0.87 | 0.87 | 1.3 | 1.1 | Very High | Right |
| 27 | 0.2216 | 0.8511 | -0.0216 | True | 0.87 | 0.87 | 0.87 | 0.87 | 0.87 | 0.87 | 1.4 | 1.2 | High | Right |
| 28 | 0.1558 | 1.2585 | 0.0018 | True | 0.87 | 0.87 | 0.87 | 0.87 | 0.87 | 0.87 | 1.5 | 1.1 | Very High | Right |
| 29 | -0.0163 | 0.3197 | 0.0062 | True | 0.87 | 0.87 | 0.87 | 0.87 | 0.87 | 0.87 | 1.6 | 1.1 | Moderate | Left |
| 30 | 0.3805 | 1.1173 | 0.0001 | True | 0.87 | 0.87 | 0.87 | 0.87 | 0.87 | 0.87 | 1.6 | 1.2 | High | Right |
| 31 | 0.3154 | 0.7692 | -0.0131 | True | 0.87 | 0.87 | 0.87 | 0.87 | 0.87 | 0.87 | 1.7 | 1.2 | High | Right |
| 32 | 0.2168 | 0.7894 | -0.0223 | True | 0.87 | 0.87 | 0.87 | 0.87 | 0.87 | 0.87 | 1.75 | 1.2 | High | Right |
| 33 | 0.3294 | 1.1164 | 0.0054 | True | 0.87 | 0.87 | 0.87 | 0.87 | 0.87 | 0.87 | 1.75 | 1.2 | High | Right |
| 34 | 0.3945 | 1.0290 | 0.0042 | True | 0.87 | 0.87 | 0.87 | 0.87 | 0.87 | 0.87 | 1.8 | 1.2 | High | Right |
| 35 | 0.3908 | 1.0880 | -0.0342 | True | 0.87 | 0.87 | 0.87 | 0.87 | 0.87 | 0.87 | 1.8 | 1.3 | High | Right |
| 36 | 0.1182 | 0.6111 | -0.0026 | True | 0.87 | 0.87 | 0.87 | 0.87 | 0.87 | 0.87 | 1.8 | 1.3 | Moderate | Right |
| 37 | 0.1182 | 0.6111 | -0.0026 | True | 0.87 | 0.87 | 0.87 | 0.87 | 0.87 | 0.87 | 1.8 | 1.3 | Moderate | Right |
| 38 | 0.1755 | 0.8370 | -0.0033 | True | 0.87 | 0.87 | 0.87 | 0.87 | 0.87 | 0.87 | 1.8 | 1.3 | High | Right |
| 39 | 0.4139 | 1.4451 | -0.0086 | False | 0.87 | 0.87 | 0.87 | 0.87 | 0.87 | 0.87 | 1.8 | 1.25 | Very High | Right |
| 40 | 0.4455 | 1.3888 | -0.0355 | False | 0.9 | 0.9 | 0.9 | 0.9 | 0.9 | 0.9 | 1.8 | 1.3 | Very High | Right |
| 41 | 0.4455 | 1.3888 | -0.0355 | False | 0.9 | 0.9 | 0.9 | 0.9 | 0.9 | 0.9 | 1.8 | 1.3 | Very High | Right |

**Explanation:**

The table summarizes the landing position of the ball for each example, along with the corresponding parameter values (a-h). The estimated speed of the ball was determined based on the y-coordinate of the landing position. The higher the y-coordinate, the faster the ball was hit. 

* **Examples 1-22:** These examples demonstrate that increasing parameter **g** generally results in a faster ball speed and a landing position further on the opponent's side of the table. However, none of these examples resulted in a right landing position. 
* **Examples 23-41:**  These examples show that increasing **g** along with other parameters like **c** and **d** can push the ball to the right side of the table. Examples 26-37 consistently hit the ball on the right side of the table. Examples 38-41 also hit the ball on the right side of the table but landed outside of the table due to the high speed.  

## Step 2: Parameters that are closest to fulfilling the objective

The closest parameters to fulfilling the objective of hitting the ball as far right as possible while still landing on the table are: 
**a:0.87 b:0.87 c:0.87 d:0.87 e:0.87 f:0.87 g:1.4 h:1.2** (Example 27). 

This example consistently lands the ball on the right side of the table with a moderate speed. 

## Step 3: Analyzing the effect of parameters on landing position

Based on the table, we can observe the following trends:

* **Parameter g:**  Higher values of **g** generally lead to a faster ball speed and a landing position further down the table. It also influences the landing position along the x-axis, pushing the ball towards the right side of the table. 
* **Parameter c:** Increasing **c** seems to shift the landing position towards the right, potentially affecting the ball's direction. 
* **Parameter d:**  Increasing **d** appears to contribute to a more right landing position, potentially impacting the ball's spin. 
* **Parameter h:** Increasing **h** generally leads to a faster ball speed and a landing position further down the table. 
* **Parameter e:**  Increasing **e** can make the ball go slightly further to the left.  
* **Parameters a, b, f:** These parameters do not appear to have a significant impact on the landing position, although they may play a role in the ball's spin or trajectory.

## Step 4: Proposed Parameters

Proposed params: a:0.87 b:0.87 c:1.05 d:1.05 e:0.87 f:0.87 g:1.45 h:1.25 

<q> Hit the ball as far right as possible while still landing it on the table!
## Step 1: Summary Table

| Example | a | b | c | d | e | f | g | h | Landing Side | Estimated Speed |
|---|---|---|---|---|---|---|---|---|---|---|
| 1 | 0.75 | 0.75 | 0.75 | 0.75 | 1.1 | 0.75 | 0.75 | 0.75 | Left | Medium |
| 2 | 0.9 | 0.9 | 0.9 | 0.9 | 0.8 | 0.9 | 0.9 | 0.9 | Left | Medium |
| 3 | 0.75 | 0.75 | 0.75 | 0.75 | 0.75 | 0.75 | 1.1 | 0.75 | Left | Medium |
| 4 | 0.87 | 0.87 | 0.87 | 0.87 | 0.87 | 0.87 | 0.87 | 1.23 | Left | Medium |
| 5 | 0.9 | 0.9 | 0.9 | 0.9 | 0.9 | 0.6 | 0.9 | 0.9 | Left | Medium |
| 6 | 0.9 | 0.9 | 0.9 | 0.9 | 0.9 | 1.1 | 0.9 | 0.9 | Left | Medium |
| 7 | 0.87 | 0.87 | 0.87 | 0.87 | 0.87 | 0.87 | 0.87 | 1.2 | Left | Medium |
| 8 | 0.8 | 0.8 | 1.1 | 0.8 | 0.8 | 0.8 | 0.8 | 0.8 | Left | Medium |
| 9 | 0.95 | 0.95 | 0.95 | 0.8 | 0.95 | 0.95 | 0.95 | 0.95 | Left | Medium |
| 10 | 0.9 | 0.9 | 0.9 | 0.9 | 0.9 | 0.8 | 0.9 | 0.9 | Left | Medium |
| 11 | 0.75 | 0.75 | 0.75 | 0.75 | 0.8 | 0.75 | 0.75 | 0.75 | Left | Medium |
| 12 | 0.9 | 0.9 | 0.9 | 0.9 | 1.1 | 0.9 | 0.9 | 0.9 | Left | Medium |
| 13 | 0.9 | 0.9 | 0.9 | 0.8 | 0.9 | 0.9 | 0.9 | 0.9 | Left | Medium |
| 14 | 0.8 | 0.8 | 1.1 | 0.8 | 0.8 | 0.8 | 0.8 | 1.05 | Left | Medium |
| 15 | 0.8 | 0.8 | 1.1 | 0.8 | 0.8 | 0.8 | 0.8 | 1.05 | Left | Medium |
| 16 | 0.8 | 0.8 | 1.1 | 0.8 | 0.8 | 0.8 | 0.8 | 1.05 | Left | Medium |
| 17 | 0.8 | 0.8 | 1.1 | 0.8 | 0.8 | 0.8 | 0.8 | 1.05 | Left | Medium |
| 18 | 0.8 | 0.8 | 1.1 | 0.8 | 0.8 | 0.8 | 0.8 | 1.05 | Left | Medium |
| 19 | 0.8 | 0.8 | 1.1 | 0.8 | 0.8 | 0.8 | 0.8 | 1.05 | Left | Medium |
| 20 | 0.8 | 0.8 | 1.1 | 0.8 | 0.8 | 0.8 | 0.8 | 1.05 | Left | Medium |
| 21 | 0.8 | 0.8 | 1.1 | 0.8 | 0.8 | 0.8 | 0.8 | 1.05 | Left | Medium |
| 22 | 0.8 | 0.8 | 1.1 | 0.8 | 0.8 | 0.8 | 0.8 | 1.05 | Left | Medium |
| 23 | 0.9 | 0.9 | 0.9 | 1.08 | 0.9 | 0.9 | 0.9 | 0.9 | Left | Medium |
| 24 | 0.8 | 0.8 | 1.1 | 0.8 | 0.8 | 0.8 | 0.8 | 1.05 | Left | Medium |
| 25 | 0.9 | 0.9 | 0.95 | 1.1 | 0.87 | 0.9 | 0.87 | 1.25 | Left | Medium |
| 26 | 0.87 | 0.87 | 0.87 | 0.87 | 0.87 | 0.87 | 1.3 | 1.1 | Right | Medium |
| 27 | 0.87 | 0.87 | 0.87 | 0.87 | 0.87 | 0.87 | 1.4 | 1.2 | Right | Medium |
| 28 | 0.87 | 0.87 | 0.87 | 0.87 | 0.87 | 0.87 | 1.5 | 1.1 | Right | Medium |
| 29 | 0.87 | 0.87 | 0.87 | 0.87 | 0.87 | 0.87 | 1.6 | 1.1 | Left | Medium |
| 30 | 0.87 | 0.87 | 0.87 | 0.87 | 0.87 | 0.87 | 1.6 | 1.2 | Right | Medium |
| 31 | 0.87 | 0.87 | 0.87 | 0.87 | 0.87 | 0.87 | 1.7 | 1.2 | Right | Medium |
| 32 | 0.87 | 0.87 | 0.87 | 0.87 | 0.87 | 0.87 | 1.75 | 1.2 | Right | Medium |
| 33 | 0.87 | 0.87 | 0.87 | 0.87 | 0.87 | 0.87 | 1.75 | 1.2 | Right | Medium |
| 34 | 0.87 | 0.87 | 0.87 | 0.87 | 0.87 | 0.87 | 1.8 | 1.2 | Right | Medium |
| 35 | 0.87 | 0.87 | 0.87 | 0.87 | 0.87 | 0.87 | 1.8 | 1.3 | Right | Medium |
| 36 | 0.87 | 0.87 | 0.87 | 0.87 | 0.87 | 0.87 | 1.8 | 1.3 | Right | Medium |
| 37 | 0.87 | 0.87 | 0.87 | 0.87 | 0.87 | 0.87 | 1.8 | 1.3 | Right | Medium |
| 38 | 0.87 | 0.87 | 0.87 | 0.87 | 0.87 | 0.87 | 1.8 | 1.3 | Right | Medium |
| 39 | 0.87 | 0.87 | 0.87 | 0.87 | 0.87 | 0.87 | 1.8 | 1.25 | Right | Medium |
| 40 | 0.87 | 0.87 | 0.87 | 0.87 | 0.87 | 0.87 | 1.8 | 1.25 | Right | Medium |
| 41 | 0.9 | 0.9 | 0.9 | 0.9 | 0.9 | 0.9 | 1.8 | 1.3 | Right | Medium |
| 42 | 0.9 | 0.9 | 0.9 | 0.9 | 0.9 | 0.9 | 1.8 | 1.3 | Right | Medium |
| 43 | 0.87 | 0.87 | 1.05 | 1.05 | 0.87 | 0.87 | 1.45 | 1.25 | Right | Medium |

**Explanation:** 
To determine the landing side, we look at the `y` value of the landing position. If the `y` value is positive, the ball landed on the opponent's side (right). If the `y` value is negative, the ball landed on our side (left). 

The estimated speed of the ball is based on the difference in `y` values between consecutive time steps. A larger difference indicates a faster ball. For simplicity, we use the categories "slow", "medium", and "fast" to describe the speed. 

All examples have a "medium" speed ball except for Example 23 which has a slightly faster ball.

## Step 2: Closest Parameters

The parameters closest to fulfilling the objective are:

**Example 26**: a:0.87 b:0.87 c:0.87 d:0.87 e:0.87 f:0.87 g:1.3 h:1.1

**Example 27**: a:0.87 b:0.87 c:0.87 d:0.87 e:0.87 f:0.87 g:1.4 h:1.2

**Example 28**: a:0.87 b:0.87 c:0.87 d:0.87 e:0.87 f:0.87 g:1.5 h:1.1

**Example 30**: a:0.87 b:0.87 c:0.87 d:0.87 e:0.87 f:0.87 g:1.6 h:1.2

**Example 31**: a:0.87 b:0.87 c:0.87 d:0.87 e:0.87 f:0.87 g:1.7 h:1.2

**Example 32**: a:0.87 b:0.87 c:0.87 d:0.87 e:0.87 f:0.87 g:1.75 h:1.2

**Example 33**: a:0.87 b:0.87 c:0.87 d:0.87 e:0.87 f:0.87 g:1.75 h:1.2

**Example 34**: a:0.87 b:0.87 c:0.87 d:0.87 e:0.87 f:0.87 g:1.8 h:1.2

**Example 35**: a:0.87 b:0.87 c:0.87 d:0.87 e:0.87 f:0.87 g:1.8 h:1.3

**Example 36**: a:0.87 b:0.87 c:0.87 d:0.87 e:0.87 f:0.87 g:1.8 h:1.3

**Example 37**: a:0.87 b:0.87 c:0.87 d:0.87 e:0.87 f:0.87 g:1.8 h:1.3

**Example 38**: a:0.87 b:0.87 c:0.87 d:0.87 e:0.87 f:0.87 g:1.8 h:1.3

**Example 39**: a:0.87 b:0.87 c:0.87 d:0.87 e:0.87 f:0.87 g:1.8 h:1.25

**Example 40**: a:0.87 b:0.87 c:0.87 d:0.87 e:0.87 f:0.87 g:1.8 h:1.25

**Example 41**: a:0.9 b:0.9 c:0.9 d:0.9 e:0.9 f:0.9 g:1.8 h:1.3

**Example 42**: a:0.9 b:0.9 c:0.9 d:0.9 e:0.9 f:0.9 g:1.8 h:1.3

**Example 43**: a:0.87 b:0.87 c:1.05 d:1.05 e:0.87 f:0.87 g:1.45 h:1.25

These examples have the ball landing on the right side of the table, indicating success in hitting the ball as far right as possible. 

## Step 3: Parameter Analysis

The parameters a, b, c, d, e, f, g, and h control various aspects of the robot's movement and ball trajectory. Let's analyze their impact:

* **a, b, c, d**: These parameters control the paddle's movement in the x and y direction.  Larger values result in a wider and deeper paddle movement respectively. In the successful examples, these parameters are generally between 0.8 and 1.0, indicating a balanced paddle movement. 

* **e**: This parameter influences the paddle's forward movement in the y direction. Larger values lead to a greater forward swing. In the successful examples, values are mostly between 0.8 and 1.0. 

* **f**: This parameter controls the backward movement of the paddle. A larger value implies a greater backward swing. Examples with values around 1.0 or higher tend to land the ball on the right side of the table. 

* **g**: This parameter controls the speed of the robot's swing. A higher value means a faster swing. Examples with values above 1.4 consistently land the ball on the right side.

* **h**: This parameter controls the speed at which the ball is hit. A higher value means a faster hit. Examples with values around 1.1 to 1.3 seem to be performing well.

## Step 4: Proposed Parameters

Based on the analysis above, we can propose the following parameters:

Proposed params: a:0.9 b:0.9 c:0.9 d:0.9 e:0.9 f:1.1 g:1.6 h:1.25

**Rationale:**

* **a, b, c, d**: We maintain these values at 0.9 for balanced paddle movement. 
* **e**: We keep the forward swing at 0.9 for a more controlled movement.
* **f**: We increase the backward swing to 1.1, hoping to enhance the rightward push.
* **g**: Increasing the swing speed to 1.6 should further contribute to landing the ball on the right side. 
* **h**: We slightly increase the hit speed to 1.25 to ensure a powerful hit. 

These proposed parameters combine the insights from the successful examples while aiming to further optimize the rightward landing position. It's important to note that these are just predictions, and further testing and adjustments may be needed to fine-tune the robot's performance. 

<q> Hit the ball as far right as possible while still landing it on the table!
## Step 1: Summary Table

| Example | a | b | c | d | e | f | g | h | Landing Side | Estimated Speed |
|---|---|---|---|---|---|---|---|---|---|---|
| 1 | 0.75 | 0.75 | 0.75 | 0.75 | 1.1 | 0.75 | 0.75 | 0.75 | Left | Medium |
| 2 | 0.9 | 0.9 | 0.9 | 0.9 | 0.8 | 0.9 | 0.9 | 0.9 | Left | Medium |
| 3 | 0.75 | 0.75 | 0.75 | 0.75 | 0.75 | 0.75 | 1.1 | 0.75 | Left | Medium |
| 4 | 0.87 | 0.87 | 0.87 | 0.87 | 0.87 | 0.87 | 0.87 | 1.23 | Left | Medium |
| 5 | 0.9 | 0.9 | 0.9 | 0.9 | 0.9 | 0.6 | 0.9 | 0.9 | Left | Medium |
| 6 | 0.9 | 0.9 | 0.9 | 0.9 | 0.9 | 1.1 | 0.9 | 0.9 | Left | Medium |
| 7 | 0.87 | 0.87 | 0.87 | 0.87 | 0.87 | 0.87 | 0.87 | 1.2 | Left | Medium |
| 8 | 0.8 | 0.8 | 1.1 | 0.8 | 0.8 | 0.8 | 0.8 | 0.8 | Left | Medium |
| 9 | 0.95 | 0.95 | 0.95 | 0.8 | 0.95 | 0.95 | 0.95 | 0.95 | Left | Medium |
| 10 | 0.9 | 0.9 | 0.9 | 0.9 | 0.9 | 0.8 | 0.9 | 0.9 | Left | Medium |
| 11 | 0.75 | 0.75 | 0.75 | 0.75 | 0.8 | 0.75 | 0.75 | 0.75 | Left | Medium |
| 12 | 0.9 | 0.9 | 0.9 | 0.9 | 1.1 | 0.9 | 0.9 | 0.9 | Left | Medium |
| 13 | 0.9 | 0.9 | 0.9 | 0.8 | 0.9 | 0.9 | 0.9 | 0.9 | Left | Medium |
| 14 | 0.8 | 0.8 | 1.1 | 0.8 | 0.8 | 0.8 | 0.8 | 1.05 | Left | Medium |
| 15 | 0.8 | 0.8 | 1.1 | 0.8 | 0.8 | 0.8 | 0.8 | 1.05 | Left | Medium |
| 16 | 0.8 | 0.8 | 1.1 | 0.8 | 0.8 | 0.8 | 0.8 | 1.05 | Left | Medium |
| 17 | 0.8 | 0.8 | 1.1 | 0.8 | 0.8 | 0.8 | 0.8 | 1.05 | Left | Medium |
| 18 | 0.8 | 0.8 | 1.1 | 0.8 | 0.8 | 0.8 | 0.8 | 1.05 | Left | Medium |
| 19 | 0.8 | 0.8 | 1.1 | 0.8 | 0.8 | 0.8 | 0.8 | 1.05 | Left | Medium |
| 20 | 0.8 | 0.8 | 1.1 | 0.8 | 0.8 | 0.8 | 0.8 | 1.05 | Left | Medium |
| 21 | 0.8 | 0.8 | 1.1 | 0.8 | 0.8 | 0.8 | 0.8 | 1.05 | Left | Medium |
| 22 | 0.8 | 0.8 | 1.1 | 0.8 | 0.8 | 0.8 | 0.8 | 1.05 | Left | Medium |
| 23 | 0.9 | 0.9 | 0.9 | 1.08 | 0.9 | 0.9 | 0.9 | 0.9 | Left | Medium |
| 24 | 0.8 | 0.8 | 1.1 | 0.8 | 0.8 | 0.8 | 0.8 | 1.05 | Left | Medium |
| 25 | 0.9 | 0.9 | 0.95 | 1.1 | 0.87 | 0.9 | 0.87 | 1.25 | Left | Medium |
| 26 | 0.87 | 0.87 | 0.87 | 0.87 | 0.87 | 0.87 | 1.3 | 1.1 | Right | Medium |
| 27 | 0.87 | 0.87 | 0.87 | 0.87 | 0.87 | 0.87 | 1.4 | 1.2 | Right | Medium |
| 28 | 0.87 | 0.87 | 0.87 | 0.87 | 0.87 | 0.87 | 1.5 | 1.1 | Right | Medium |
| 29 | 0.87 | 0.87 | 0.87 | 0.87 | 0.87 | 0.87 | 1.6 | 1.1 | Right | Medium |
| 30 | 0.87 | 0.87 | 0.87 | 0.87 | 0.87 | 0.87 | 1.6 | 1.2 | Right | Medium |
| 31 | 0.87 | 0.87 | 0.87 | 0.87 | 0.87 | 0.87 | 1.7 | 1.2 | Right | Medium |
| 32 | 0.87 | 0.87 | 0.87 | 0.87 | 0.87 | 0.87 | 1.75 | 1.2 | Right | Medium |
| 33 | 0.87 | 0.87 | 0.87 | 0.87 | 0.87 | 0.87 | 1.75 | 1.2 | Right | Medium |
| 34 | 0.87 | 0.87 | 0.87 | 0.87 | 0.87 | 0.87 | 1.8 | 1.2 | Right | Medium |
| 35 | 0.87 | 0.87 | 0.87 | 0.87 | 0.87 | 0.87 | 1.8 | 1.3 | Right | Medium |
| 36 | 0.87 | 0.87 | 0.87 | 0.87 | 0.87 | 0.87 | 1.8 | 1.3 | Right | Medium |
| 37 | 0.87 | 0.87 | 0.87 | 0.87 | 0.87 | 0.87 | 1.8 | 1.3 | Right | Medium |
| 38 | 0.87 | 0.87 | 0.87 | 0.87 | 0.87 | 0.87 | 1.8 | 1.3 | Right | Medium |
| 39 | 0.87 | 0.87 | 0.87 | 0.87 | 0.87 | 0.87 | 1.8 | 1.25 | Right | Medium |
| 40 | 0.87 | 0.87 | 0.87 | 0.87 | 0.87 | 0.87 | 1.8 | 1.25 | Right | Medium |
| 41 | 0.9 | 0.9 | 0.9 | 0.9 | 0.9 | 0.9 | 1.8 | 1.3 | Right | Medium |
| 42 | 0.9 | 0.9 | 0.9 | 0.9 | 0.9 | 0.9 | 1.8 | 1.3 | Right | Medium |
| 43 | 0.87 | 0.87 | 1.05 | 1.05 | 0.87 | 0.87 | 1.45 | 1.25 | Right | Medium |
| 44 | 0.9 | 0.9 | 0.9 | 0.9 | 0.9 | 1.1 | 1.6 | 1.25 | Right | Medium |

**Explanation:**

- **Landing Side:** We analyzed the x-coordinate of the landing position. Positive values indicate the ball landed on the right side of the table, negative values indicate the ball landed on the left side. 
- **Estimated Speed:** We qualitatively assessed the ball's speed based on the ball's motion data. A larger change in ball position over time generally corresponds to a faster ball. We categorized speeds into three groups: Slow, Medium, and Fast. 

**Observations:**

- Parameters **g** and **h** seem to have the most significant impact on the landing position. Higher values of **g** consistently push the ball towards the right side of the table. Similarly, higher values of **h** lead to a greater rightward drift. 
- There is a noticeable trend where examples with **g** above 1.4 and **h** above 1.2 consistently result in landing positions on the right side of the table. This is also reflected in the landing side column of the table. 

## Step 2: Closest Parameters

The parameters closest to fulfilling the objective are: 

- Example 26: a:0.87 b:0.87 c:0.87 d:0.87 e:0.87 f:0.87 **g:1.3 h:1.1** 
- Example 27: a:0.87 b:0.87 c:0.87 d:0.87 e:0.87 f:0.87 **g:1.4 h:1.2** 
- Example 28: a:0.87 b:0.87 c:0.87 d:0.87 e:0.87 f:0.87 **g:1.5 h:1.1**
- Example 29: a:0.87 b:0.87 c:0.87 d:0.87 e:0.87 f:0.87 **g:1.6 h:1.1**
- Example 30: a:0.87 b:0.87 c:0.87 d:0.87 e:0.87 f:0.87 **g:1.6 h:1.2**
- Example 31: a:0.87 b:0.87 c:0.87 d:0.87 e:0.87 f:0.87 **g:1.7 h:1.2**
- Example 32: a:0.87 b:0.87 c:0.87 d:0.87 e:0.87 f:0.87 **g:1.75 h:1.2**
- Example 33: a:0.87 b:0.87 c:0.87 d:0.87 e:0.87 f:0.87 **g:1.75 h:1.2**
- Example 34: a:0.87 b:0.87 c:0.87 d:0.87 e:0.87 f:0.87 **g:1.8 h:1.2**
- Example 35: a:0.87 b:0.87 c:0.87 d:0.87 e:0.87 f:0.87 **g:1.8 h:1.3**
- Example 36: a:0.87 b:0.87 c:0.87 d:0.87 e:0.87 f:0.87 **g:1.8 h:1.3**
- Example 37: a:0.87 b:0.87 c:0.87 d:0.87 e:0.87 f:0.87 **g:1.8 h:1.3**
- Example 38: a:0.87 b:0.87 c:0.87 d:0.87 e:0.87 f:0.87 **g:1.8 h:1.3**
- Example 39: a:0.87 b:0.87 c:0.87 d:0.87 e:0.87 f:0.87 **g:1.8 h:1.25**
- Example 40: a:0.87 b:0.87 c:0.87 d:0.87 e:0.87 f:0.87 **g:1.8 h:1.25**
- Example 41: a:0.9 b:0.9 c:0.9 d:0.9 e:0.9 f:0.9 **g:1.8 h:1.3**
- Example 42: a:0.9 b:0.9 c:0.9 d:0.9 e:0.9 f:0.9 **g:1.8 h:1.3**
- Example 43: a:0.87 b:0.87 c:1.05 d:1.05 e:0.87 f:0.87 **g:1.45 h:1.25**
- Example 44: a:0.9 b:0.9 c:0.9 d:0.9 e:0.9 f:1.1 **g:1.6 h:1.25**

These examples all land on the right side of the table. The ball landing position is consistently further on the right for examples with higher **g** and **h** values. However, we want to aim for the rightmost position while still staying on the table.

## Step 3: Parameter Analysis

Let's analyze the effect of the parameters on the landing position:

- **g:** This parameter influences the angle of the paddle during the hit. Higher **g** values seem to create a more pronounced angle, leading to a trajectory that curves more towards the right. 
- **h:**  This parameter controls the force applied during the hit. A higher **h** value generally results in a faster ball and a longer trajectory. 
- **a, b, c, d, e, f:** These parameters likely influence other aspects of the robot's motion, such as the paddle's position, orientation, and speed, but their effects on the landing position are not as pronounced as **g** and **h**.

## Step 4: Proposed Parameters

Proposed params: a:0.87 b:0.87 c:0.95 d:0.9 e:0.87 f:0.87 g:1.85 h:1.3

**Explanation:**

- We are increasing **g** to 1.85 from 1.8 to try to push the ball even further to the right. 
- **h** is maintained at 1.3 to ensure the ball still lands on the table. We are aiming for a longer trajectory with enough horizontal velocity to reach further right.
- We are also adjusting **c** to 0.95 to create a slight upward angle on the paddle. This could potentially allow the ball to stay on the table for a longer duration.
- **d** is adjusted to 0.9 to slow down the paddle slightly. This might allow for a more controlled hit.

This set of parameters should increase the x-coordinate of the landing position while still ensuring that the ball lands on the table. Further fine-tuning might be necessary to achieve optimal performance. 

<q> Hit the ball as far right as possible while still landing it on the table!
## Step 1: Summary Table

| Example | a | b | c | d | e | f | g | h | Landing Side | Estimated Speed |
|---|---|---|---|---|---|---|---|---|---|---|
| 1 | 0.75 | 0.75 | 0.75 | 0.75 | 1.1 | 0.75 | 0.75 | 0.75 | Left | Medium |
| 2 | 0.9 | 0.9 | 0.9 | 0.9 | 0.8 | 0.9 | 0.9 | 0.9 | Left | Medium |
| 3 | 0.75 | 0.75 | 0.75 | 0.75 | 0.75 | 0.75 | 1.1 | 0.75 | Left | Medium |
| 4 | 0.87 | 0.87 | 0.87 | 0.87 | 0.87 | 0.87 | 0.87 | 1.23 | Left | Medium |
| 5 | 0.9 | 0.9 | 0.9 | 0.9 | 0.9 | 0.6 | 0.9 | 0.9 | Left | Medium |
| 6 | 0.9 | 0.9 | 0.9 | 0.9 | 0.9 | 1.1 | 0.9 | 0.9 | Left | Medium |
| 7 | 0.87 | 0.87 | 0.87 | 0.87 | 0.87 | 0.87 | 0.87 | 1.2 | Left | Medium |
| 8 | 0.8 | 0.8 | 1.1 | 0.8 | 0.8 | 0.8 | 0.8 | 0.8 | Left | Medium |
| 9 | 0.95 | 0.95 | 0.95 | 0.8 | 0.95 | 0.95 | 0.95 | 0.95 | Left | Medium |
| 10 | 0.9 | 0.9 | 0.9 | 0.9 | 0.9 | 0.8 | 0.9 | 0.9 | Left | Medium |
| 11 | 0.75 | 0.75 | 0.75 | 0.75 | 0.8 | 0.75 | 0.75 | 0.75 | Left | Medium |
| 12 | 0.9 | 0.9 | 0.9 | 0.9 | 1.1 | 0.9 | 0.9 | 0.9 | Left | Medium |
| 13 | 0.9 | 0.9 | 0.9 | 0.8 | 0.9 | 0.9 | 0.9 | 0.9 | Left | Medium |
| 14 | 0.8 | 0.8 | 1.1 | 0.8 | 0.8 | 0.8 | 0.8 | 1.05 | Left | Medium |
| 15 | 0.8 | 0.8 | 1.1 | 0.8 | 0.8 | 0.8 | 0.8 | 1.05 | Left | Medium |
| 16 | 0.8 | 0.8 | 1.1 | 0.8 | 0.8 | 0.8 | 0.8 | 1.05 | Left | Medium |
| 17 | 0.8 | 0.8 | 1.1 | 0.8 | 0.8 | 0.8 | 0.8 | 1.05 | Left | Medium |
| 18 | 0.8 | 0.8 | 1.1 | 0.8 | 0.8 | 0.8 | 0.8 | 1.05 | Left | Medium |
| 19 | 0.8 | 0.8 | 1.1 | 0.8 | 0.8 | 0.8 | 0.8 | 1.05 | Left | Medium |
| 20 | 0.8 | 0.8 | 1.1 | 0.8 | 0.8 | 0.8 | 0.8 | 1.05 | Left | Medium |
| 21 | 0.8 | 0.8 | 1.1 | 0.8 | 0.8 | 0.8 | 0.8 | 1.05 | Left | Medium |
| 22 | 0.8 | 0.8 | 1.1 | 0.8 | 0.8 | 0.8 | 0.8 | 1.05 | Left | Medium |
| 23 | 0.9 | 0.9 | 0.9 | 1.08 | 0.9 | 0.9 | 0.9 | 0.9 | Left | Medium |
| 24 | 0.8 | 0.8 | 1.1 | 0.8 | 0.8 | 0.8 | 0.8 | 1.05 | Left | Medium |
| 25 | 0.9 | 0.9 | 0.95 | 1.1 | 0.87 | 0.9 | 0.87 | 1.25 | Left | Medium |
| 26 | 0.87 | 0.87 | 0.87 | 0.87 | 0.87 | 0.87 | 1.3 | 1.1 | Right | Medium |
| 27 | 0.87 | 0.87 | 0.87 | 0.87 | 0.87 | 0.87 | 1.4 | 1.2 | Right | Medium |
| 28 | 0.87 | 0.87 | 0.87 | 0.87 | 0.87 | 0.87 | 1.5 | 1.1 | Right | Medium |
| 29 | 0.87 | 0.87 | 0.87 | 0.87 | 0.87 | 0.87 | 1.6 | 1.1 | Right | Medium |
| 30 | 0.87 | 0.87 | 0.87 | 0.87 | 0.87 | 0.87 | 1.6 | 1.2 | Right | Medium |
| 31 | 0.87 | 0.87 | 0.87 | 0.87 | 0.87 | 0.87 | 1.7 | 1.2 | Right | Medium |
| 32 | 0.87 | 0.87 | 0.87 | 0.87 | 0.87 | 0.87 | 1.75 | 1.2 | Right | Medium |
| 33 | 0.87 | 0.87 | 0.87 | 0.87 | 0.87 | 0.87 | 1.75 | 1.2 | Right | Medium |
| 34 | 0.87 | 0.87 | 0.87 | 0.87 | 0.87 | 0.87 | 1.8 | 1.2 | Right | Medium |
| 35 | 0.87 | 0.87 | 0.87 | 0.87 | 0.87 | 0.87 | 1.8 | 1.3 | Right | Medium |
| 36 | 0.87 | 0.87 | 0.87 | 0.87 | 0.87 | 0.87 | 1.8 | 1.3 | Right | Medium |
| 37 | 0.87 | 0.87 | 0.87 | 0.87 | 0.87 | 0.87 | 1.8 | 1.3 | Right | Medium |
| 38 | 0.87 | 0.87 | 0.87 | 0.87 | 0.87 | 0.87 | 1.8 | 1.3 | Right | Medium |
| 39 | 0.87 | 0.87 | 0.87 | 0.87 | 0.87 | 0.87 | 1.8 | 1.25 | Right | Medium |
| 40 | 0.87 | 0.87 | 0.87 | 0.87 | 0.87 | 0.87 | 1.8 | 1.25 | Right | Medium |
| 41 | 0.9 | 0.9 | 0.9 | 0.9 | 0.9 | 0.9 | 1.8 | 1.3 | Right | Medium |
| 42 | 0.87 | 0.87 | 1.05 | 1.05 | 0.87 | 0.87 | 1.45 | 1.25 | Right | Medium |
| 43 | 0.9 | 0.9 | 0.9 | 0.9 | 0.9 | 1.1 | 1.6 | 1.25 | Right | Medium |
| 44 | 0.87 | 0.87 | 0.95 | 0.9 | 0.87 | 0.87 | 1.8 | 1.3 | Right | Medium |
| 45 | 0.8 | 0.8 | 1.1 | 0.8 | 0.8 | 0.8 | 0.8 | 1.05 | Left | Medium |

**Explanation:**

- **Landing Side:** This column indicates whether the ball landed on the left or right side of the table based on the provided "x" coordinate of the landing position. Positive "x" values indicate the right side, while negative "x" values indicate the left side.
- **Estimated Speed:** This column provides a subjective estimation of the ball's speed based on the provided ball motion data. "Medium" is used here because the ball's speed seems to be consistent across all examples, and no significant variation in speed is observed. 
- **Parameter Values:** Parameters "a" through "h" control different aspects of the robot's movement and the ball's trajectory. These values are listed for each example.

**Key Observations:**

- Examples 26 through 45 show a clear trend of the ball landing on the right side of the table.
- The examples hitting the ball on the right side mostly share similar values for parameters "g" and "h" (both values are above 1, with "g" usually higher than "h").  
- Parameter "e" (which has a value higher than 1 in examples 1 and 12, both hitting the ball on the left side) does not seem to have a significant influence on the landing side of the ball.

## Step 2: Parameters Closest to Objective

The parameters closest to fulfilling the objective of hitting the ball as far right as possible are found in examples 26, 27, 28, 29, 30, 31, 32, 33, 34, 35, 36, 37, 38, 39, 40, 41, 42, 43, 44, and 45.  All of these examples successfully land the ball on the right side of the table.

## Step 3: Parameter Analysis

- **Parameters "g" and "h":**  These parameters seem to have the most significant influence on the landing position. Higher values of "g" and "h" result in the ball landing further to the right. This is likely due to these parameters controlling the robot's movement and influencing the ball's initial trajectory, leading to a more pronounced curve towards the right.
- **Parameter "a" and "b":** These parameters, while not directly controlling the landing side, can influence the ball's initial speed and trajectory.  Higher values of "a" and "b" could potentially lead to a faster ball speed and a more pronounced curve.
- **Parameter "c" and "d":** These parameters primarily control the robot's movement in the x-dimension (width of the table). Higher values of "c" and "d" would generally result in the paddle being positioned further to the right, potentially leading to a ball that curves more towards the right.
- **Parameter "f":**  This parameter seems to have a less direct influence on the landing side. While a higher value of "f" could potentially influence the initial trajectory, its effect on the final landing position is less significant compared to other parameters.

## Step 4: Proposed Params

Proposed params: a:0.95 b:0.95 c:1.1 d:1.1 e:0.9 f:0.9 g:1.8 h:1.3

**Explanation:**

- **a:0.95 b:0.95:**  These values are increased slightly from previous examples to potentially increase the ball's initial speed and add a more pronounced curve towards the right.
- **c:1.1 d:1.1:** These values are increased to move the paddle further to the right, enhancing the ball's initial curve towards the right. 
- **e:0.9 f:0.9:** These parameters are not significantly changed, as they seem to have a less pronounced impact on the landing side. 
- **g:1.8 h:1.3:** These values are increased further based on the observed trend that higher values of "g" and "h" result in the ball landing further to the right. This should lead to a significant improvement in landing the ball on the right side of the table.

These proposed parameters aim to combine the positive effects of each parameter to achieve a more pronounced curve towards the right and potentially improve the final landing position. The adjustment is made by increasing the value of "g", "h", "a", "b", "c", and "d" in the hopes of achieving the goal. It is important to note that the exact effect of each parameter may vary depending on the specific robot configuration and dynamics, and experimentation is required to verify the effectiveness of these proposed parameters.

----------------------->

<q> Hit the ball as far right as possible
--------------- Backhand Stroke Examples:

--------------- Forehand Stroke Examples:

Example 1:
a:0.75 b:0.75 c:0.75 d:0.75 e:1.1 f:0.75 g:0.75 h:0.75 

Landing Position:
  x      y      z      On Table
-0.2978 0.4482 0.0089   True

Paddle Motion and Ball Motion:
      paddle x  paddle y  paddle z  ball x  ball y  ball z
time                                                      
10      0.2302   -1.1065    0.4025  0.3204  0.5031  0.3763
12      0.2863   -1.1662    0.4059  0.3167  0.2917  0.3326
14      0.3394   -1.2308    0.4023  0.3203  0.0597  0.2785
16      0.3886   -1.2906    0.3897  0.2966 -0.1054  0.2222
18      0.4252   -1.3388    0.3706  0.2923 -0.3175  0.1407
20      0.4412   -1.3756    0.3473  0.2731 -0.4964  0.0613
22      0.4352   -1.4007    0.3235  0.2612 -0.6774  0.0186
24      0.4093   -1.4065    0.2994  0.2401 -0.8064  0.1655
26      0.3692   -1.3829    0.2741  0.2215 -0.9491  0.2072
28      0.3204   -1.3365    0.2549  0.2056 -1.0814  0.2411
30      0.2794   -1.2750    0.2562  0.1931 -1.2287  0.2695
32      0.2436   -1.2103    0.2735  0.1774 -1.3222  0.2769
34      0.2052   -1.1427    0.2891  0.1115 -0.9736  0.3429
36      0.1709   -1.0679    0.3111  0.0746 -0.8256  0.3610
38      0.1267   -1.0070    0.3332  0.0244 -0.6712  0.3593
40      0.0752   -0.9478    0.3548 -0.0072 -0.5266  0.3407
42      0.0160   -0.8958    0.3755 -0.0508 -0.3876  0.3178
44     -0.0495   -0.8515    0.3952 -0.0920 -0.2428  0.2859
46     -0.1201   -0.8159    0.4137 -0.1365 -0.1077  0.2295
48     -0.1943   -0.7895    0.4308 -0.1756  0.0188  0.1659
50     -0.2684   -0.7597    0.4240 -0.2118  0.1519  0.1269
52     -0.3450   -0.7363    0.4149 -0.2454  0.2761  0.0737
54     -0.4233   -0.7209    0.4054 -0.2764  0.3937  0.0038

Example 2:
a:0.9 b:0.9 c:0.9 d:0.9 e:0.8 f:0.9 g:0.9 h:0.9 

Landing Position:
  x      y      z      On Table
-0.2155 0.9221 0.0056   True

Paddle Motion and Ball Motion:
      paddle x  paddle y  paddle z  ball x  ball y  ball z
time                                                      
10      0.2451   -1.1283    0.4129  0.2910  0.5318  0.3952
12      0.3000   -1.2081    0.4211  0.2852  0.3270  0.3540
14      0.3533   -1.2977    0.4184  0.2762  0.1310  0.3112
16      0.4042   -1.3786    0.3993  0.2579 -0.0736  0.2448
18      0.4369   -1.4408    0.3696  0.2354 -0.2618  0.1672
20      0.4372   -1.4800    0.3379  0.2329 -0.4544  0.0956
22      0.4131   -1.5076    0.3093  0.2152 -0.6225  0.0141
24      0.3711   -1.5017    0.2850  0.1968 -0.7651  0.1183
26      0.3203   -1.4594    0.2625  0.1799 -0.9146  0.1995
28      0.2786   -1.3870    0.2445  0.1646 -1.0481  0.2330
30      0.2351   -1.3095    0.2442  0.1519 -1.1824  0.2654
32      0.1888   -1.2204    0.2703  0.1317 -1.3179  0.2851
34      0.1496   -1.1468    0.2925  0.0868 -0.9634  0.3631
36      0.1114   -1.0649    0.3089  0.0661 -0.8244  0.3950
38      0.0794   -0.9914    0.3289  0.0350 -0.6192  0.4198
40      0.0332   -0.9275    0.3476  0.0038 -0.4560  0.4371
42     -0.0225   -0.8723    0.3655 -0.0234 -0.2885  0.4372
44     -0.0863   -0.8278    0.3822 -0.0517 -0.1260  0.4177
46     -0.1555   -0.7940    0.3938 -0.0823  0.0320  0.3916
48     -0.2252   -0.7593    0.3758 -0.1101  0.1889  0.3501
50     -0.2981   -0.7356    0.3574 -0.1286  0.3435  0.2932
52     -0.3726   -0.7232    0.3387 -0.1440  0.4966  0.2238
54     -0.4470   -0.7222    0.3197 -0.1840  0.6407  0.1549
56     -0.5211   -0.7305    0.3192 -0.1953  0.7831  0.0589
58     -0.5938   -0.7483    0.3330 -0.2155  0.9221  0.0056

Example 3:
a:0.75 b:0.75 c:0.75 d:0.75 e:0.75 f:0.75 g:1.1 h:0.75 

Landing Position:
  x      y      z      On Table
-0.1632 0.4586 -0.0168   True

Paddle Motion and Ball Motion:
      paddle x  paddle y  paddle z  ball x  ball y  ball z
time                                                      
10      0.2315   -1.1062    0.4136  0.3153  0.5394  0.3898
12      0.2824   -1.1674    0.4246  0.2944  0.3458  0.3437
14      0.3362   -1.2326    0.4220  0.2841  0.1355  0.2974
16      0.3866   -1.2909    0.4026  0.2702 -0.0568  0.2312
18      0.4399   -1.3736    0.3547  0.2543 -0.2587  0.1548
20      0.4277   -1.3762    0.3323  0.2449 -0.4435  0.0681
22      0.4152   -1.4106    0.2942  0.2276 -0.6373 -0.0145
24      0.3903   -1.4258    0.2602  0.2127 -0.7758  0.1591
26      0.3403   -1.4091    0.2306  0.2024 -0.9183  0.1954
28      0.2915   -1.3647    0.2134  0.1731 -1.0880  0.2500
30      0.2576   -1.3013    0.2307  0.1513 -1.1942  0.2676
32      0.2409   -1.2365    0.2710  0.1514 -1.3352  0.2788
34      0.2083   -1.1642    0.2960  0.1208 -1.0172  0.3558
36      0.1547   -1.0960    0.3212  0.0808 -0.8779  0.3740
38      0.1199   -1.0353    0.3433  0.0644 -0.7141  0.4011
40      0.0687   -0.9773    0.3654  0.0453 -0.5208  0.4025
42      0.0099   -0.9272    0.3866  0.0075 -0.4068  0.3799
44     -0.0564   -0.8858    0.4068 -0.0044 -0.2777  0.3600
46     -0.1263   -0.8502    0.4153 -0.0386 -0.1359  0.3151
48     -0.1967   -0.8138    0.4007 -0.0697  0.0012  0.2626
50     -0.2711   -0.7857    0.3859 -0.0954  0.1363  0.1924
52     -0.3483   -0.7664    0.3708 -0.1243  0.2716  0.1112
54     -0.4272   -0.7563    0.3554 -0.1440  0.3981  0.0130

Example 4:
a:0.87 b:0.87 c:0.87 d:0.87 e:0.87 f:0.87 g:0.87 h:1.23 

Landing Position:
  x      y      z      On Table
-0.0872 0.7329 0.0464   True

Paddle Motion and Ball Motion:
      paddle x  paddle y  paddle z  ball x  ball y  ball z
time                                                      
10      0.2522   -1.1255    0.4102  0.3029  0.4947  0.3898
12      0.2540   -1.1556    0.4131  0.2920  0.2896  0.3518
14      0.3589   -1.2867    0.4128  0.2831  0.1095  0.3080
16      0.4108   -1.3604    0.3906  0.2680 -0.1030  0.2415
18      0.4628   -1.4576    0.3487  0.2572 -0.3017  0.1687
20      0.4536   -1.4560    0.3375  0.2395 -0.4644  0.0895
22      0.4302   -1.4725    0.3151  0.2307 -0.6590 -0.0023
24      0.3910   -1.4555    0.3062  0.2175 -0.7999  0.1095
26      0.3378   -1.4275    0.2650  0.1972 -0.9404  0.1994
28      0.2877   -1.3619    0.2420  0.1809 -1.0804  0.2265
30      0.2456   -1.2800    0.2437  0.1736 -1.2175  0.2598
32      0.2139   -1.2019    0.2732  0.1642 -1.3330  0.2664
34      0.1624   -1.0948    0.3144  0.1317 -0.9566  0.3738
36      0.1492   -1.0734    0.3052  0.0985 -0.8149  0.4101
38      0.1357   -1.0520    0.3052  0.0855 -0.6643  0.4386
40      0.1218   -1.0301    0.3052  0.0484 -0.4889  0.4506
42      0.1079   -1.0083    0.3052  0.0404 -0.3557  0.4442
44      0.0940   -0.9865    0.3052  0.0245 -0.2028  0.4283
46      0.0801   -0.9646    0.3052  0.0034 -0.0651  0.3885
48      0.0662   -0.9428    0.3052 -0.0056  0.0682  0.3521
50      0.0523   -0.9210    0.3052 -0.0261  0.2137  0.2951
52      0.0384   -0.8991    0.3052 -0.0518  0.3531  0.2277
54      0.0245   -0.8773    0.3052 -0.0592  0.5144  0.1251
56      0.0107   -0.8559    0.3052 -0.0751  0.6145  0.0399
58     -0.0032   -0.8532    0.3052 -0.0872  0.7329  0.0464

Example 5:
a:0.9 b:0.9 c:0.9 d:0.9 e:0.9 f:0.6 g:0.9 h:0.9 

Landing Position:
  x      y      z      On Table
-0.3773 1.2431 0.0208   True

Paddle Motion and Ball Motion:
      paddle x  paddle y  paddle z  ball x  ball y  ball z
time                                                      
10      0.2345   -1.1230    0.4103  0.2970  0.3899  0.3639
12      0.2855   -1.1915    0.4167  0.2787  0.1831  0.3180
14      0.3352   -1.2647    0.4095  0.2693 -0.0123  0.2641
16      0.3714   -1.3311    0.3827  0.2539 -0.2011  0.1995
18      0.3918   -1.3855    0.3475  0.2354 -0.3962  0.1181
20      0.4091   -1.4298    0.3131  0.2308 -0.5765  0.0358
22      0.3854   -1.4634    0.2788  0.2033 -0.7432  0.0715
24      0.3449   -1.4486    0.2623  0.1928 -0.8784  0.1916
26      0.2918   -1.4019    0.2439  0.1748 -1.0162  0.2237
28      0.2226   -1.3314    0.2379  0.1549 -1.1556  0.2523
30      0.1853   -1.2387    0.2565  0.1472 -1.2709  0.2773
32      0.1702   -1.1488    0.2812  0.0969 -0.9933  0.3520
34      0.1390   -1.0589    0.2988  0.0556 -0.7858  0.4118
36      0.0877   -0.9749    0.3182  0.0084 -0.5921  0.4479
38      0.0283   -0.8980    0.3369 -0.0174 -0.4130  0.4652
40     -0.0411   -0.8305    0.3549 -0.0630 -0.2312  0.4687
42     -0.1185   -0.7737    0.3720 -0.1012 -0.0498  0.4567
44     -0.2017   -0.7283    0.3860 -0.1324  0.1113  0.4374
46     -0.2844   -0.6817    0.3656 -0.1755  0.2859  0.4122
48     -0.3704   -0.6457    0.3450 -0.2235  0.4567  0.3682
50     -0.4579   -0.6207    0.3241 -0.2551  0.6170  0.3074
52     -0.5452   -0.6067    0.3031 -0.2857  0.7748  0.2407
54     -0.6317   -0.6021    0.2925 -0.3060  0.9394  0.1534
56     -0.7180   -0.6051    0.3047 -0.3455  1.0970  0.0557
58     -0.8008   -0.6310    0.3163 -0.3773  1.2431  0.0208

Example 6:
a:0.9 b:0.9 c:0.9 d:0.9 e:0.9 f:1.1 g:0.9 h:0.9 

Landing Position:
  x      y      z      On Table
-0.1330 0.6830 0.0013   True

Paddle Motion and Ball Motion:
      paddle x  paddle y  paddle z  ball x  ball y  ball z
time                                                      
10      0.2424   -1.1253    0.4146  0.3163  0.3433  0.3363
12      0.3248   -1.2067    0.4210  0.3123  0.1311  0.2828
14      0.3933   -1.2946    0.4125  0.2969 -0.0582  0.2218
16      0.4469   -1.3689    0.3855  0.2874 -0.2637  0.1562
18      0.4688   -1.4264    0.3495  0.2818 -0.4456  0.0695
20      0.4440   -1.4431    0.3158  0.2652 -0.6348 -0.0167
22      0.4153   -1.4410    0.2916  0.2511 -0.7690  0.1536
24      0.3719   -1.4117    0.2649  0.2367 -0.9172  0.1954
26      0.3218   -1.3383    0.2424  0.2159 -1.0615  0.2336
28      0.2779   -1.2613    0.2402  0.2179 -1.1970  0.2654
30      0.2416   -1.1835    0.2566  0.2118 -1.1773  0.2985
32      0.2062   -1.1003    0.2714  0.1420 -0.9176  0.3513
34      0.1706   -1.0146    0.2963  0.1279 -0.7209  0.3816
36      0.1051   -0.9243    0.3269  0.0953 -0.5863  0.3965
38      0.0174   -0.8548    0.3562  0.0711 -0.4297  0.3887
40     -0.0848   -0.8100    0.3833  0.0387 -0.2753  0.3684
42     -0.1906   -0.7725    0.3632  0.0119 -0.1214  0.3411
44     -0.3006   -0.7570    0.3381 -0.0191  0.0205  0.3079
46     -0.4100   -0.7656    0.3126 -0.0439  0.1717  0.2507
48     -0.5167   -0.7946    0.3135 -0.0735  0.3154  0.1822
50     -0.6166   -0.8445    0.3311 -0.0985  0.4594  0.1087
52     -0.7017   -0.9159    0.3432 -0.1195  0.5967  0.0088

Example 7:
a:0.87 b:0.87 c:0.87 d:0.87 e:0.87 f:0.87 g:0.87 h:1.2 

Landing Position:
  x      y      z      On Table
-0.2439 0.7760 0.0533   True

Paddle Motion and Ball Motion:
      paddle x  paddle y  paddle z  ball x  ball y  ball z
time                                                      
10      0.2361   -1.1010    0.4089  0.2677  0.0722  0.2464
12      0.2890   -1.1646    0.4076  0.2582 -0.1265  0.1785
14      0.3375   -1.2332    0.3885  0.2506 -0.3135  0.1021
16      0.3700   -1.2922    0.3543  0.2346 -0.5057  0.0149
18      0.3772   -1.3347    0.3174  0.2162 -0.6570  0.1151
20      0.3599   -1.3540    0.2862  0.2014 -0.8006  0.1937
22      0.3184   -1.3385    0.2586  0.1909 -0.9422  0.2271
24      0.2646   -1.2821    0.2419  0.1666 -1.0849  0.2575
26      0.2202   -1.2105    0.2391  0.1667 -1.2118  0.2733
28      0.1903   -1.1318    0.2378  0.1424 -1.0743  0.3374
30      0.1484   -1.0443    0.2393  0.0858 -0.8394  0.3938
32      0.1054   -0.9631    0.2577  0.0660 -0.7053  0.4289
34      0.0548   -0.8886    0.2763  0.0381 -0.5588  0.4417
36     -0.0084   -0.8215    0.2946  0.0044 -0.4062  0.4508
38     -0.0804   -0.7651    0.3126 -0.0186 -0.2650  0.4335
40     -0.1595   -0.7208    0.3299 -0.0474 -0.1260  0.4198
42     -0.2435   -0.6897    0.3464 -0.0850  0.0115  0.3833
44     -0.3299   -0.6726    0.3620 -0.1103  0.1533  0.3373
46     -0.4168   -0.6579    0.3498 -0.1338  0.2771  0.2824
48     -0.5039   -0.6552    0.3366 -0.1653  0.4274  0.1934
50     -0.5895   -0.6646    0.3232 -0.1907  0.5456  0.1227
52     -0.6729   -0.6844    0.3274 -0.2210  0.6853  0.0181
54     -0.7527   -0.7149    0.3448 -0.2439  0.7760  0.0533

Example 8:
a:0.8 b:0.8 c:1.1 d:0.8 e:0.8 f:0.8 g:0.8 h:0.8 

Landing Position:
  x      y      z      On Table
-0.1013 0.5102 0.0424   True

Paddle Motion and Ball Motion:
      paddle x  paddle y  paddle z  ball x  ball y  ball z
time                                                      
10      0.2795   -1.1333    0.4050  0.3358  0.5101  0.3609
12      0.3547   -1.2246    0.4134  0.3381  0.2882  0.3282
14      0.4152   -1.3275    0.4106  0.3302  0.0903  0.2807
16      0.4695   -1.4255    0.3901  0.3205 -0.1069  0.2173
18      0.5079   -1.5041    0.3571  0.3205 -0.3050  0.1351
20      0.5090   -1.5567    0.3236  0.3149 -0.5060  0.0568
22      0.4871   -1.5752    0.2965  0.3162 -0.6895 -0.0043
24      0.4501   -1.5513    0.2745  0.2927 -0.8073  0.1522
26      0.4032   -1.4809    0.2578  0.2862 -0.9579  0.1904
28      0.3635   -1.3811    0.2474  0.2635 -1.0928  0.2322
30      0.3290   -1.2754    0.2543  0.2628 -1.2263  0.2623
32      0.2962   -1.1653    0.2730  0.2320 -1.1066  0.2843
34      0.2475   -1.0611    0.2886  0.1863 -0.8677  0.3149
36      0.1939   -0.9694    0.3138  0.1551 -0.7076  0.3164
38      0.1273   -0.8786    0.3394  0.1180 -0.5319  0.3122
40      0.0479   -0.8019    0.3645  0.0989 -0.3641  0.2942
42     -0.0398   -0.7411    0.3887  0.0569 -0.1880  0.2627
44     -0.1328   -0.6979    0.4118  0.0171 -0.0251  0.2126
46     -0.2273   -0.6730    0.4336 -0.0123  0.1394  0.1571
48     -0.3218   -0.6547    0.4324 -0.0450  0.3004  0.0860
50     -0.4152   -0.6472    0.4211 -0.0839  0.4554 -0.0013

Example 9:
a:0.95 b:0.95 c:0.95 d:0.8 e:0.95 f:0.95 g:0.95 h:0.95 

Landing Position:
  x      y      z      On Table
-0.1778 1.2526 -0.0383   True

Paddle Motion and Ball Motion:
      paddle x  paddle y  paddle z  ball x  ball y  ball z
time                                                      
10      0.2493   -1.1296    0.4096  0.3061  0.5415  0.3666
12      0.3111   -1.2144    0.4177  0.2891  0.3303  0.3301
14      0.3664   -1.3075    0.4143  0.2868  0.1441  0.2927
16      0.4165   -1.3939    0.3960  0.2620 -0.0566  0.2214
18      0.4500   -1.4565    0.3660  0.2485 -0.2562  0.1469
20      0.4485   -1.4961    0.3344  0.2421 -0.4331  0.0747
22      0.4155   -1.5084    0.3044  0.2208 -0.6230 -0.0276
24      0.3752   -1.4999    0.2747  0.1936 -0.7522  0.1605
26      0.3251   -1.4509    0.2466  0.1856 -0.8949  0.1938
28      0.2675   -1.3723    0.2233  0.1600 -1.0310  0.2414
30      0.2172   -1.2856    0.2247  0.1486 -1.1645  0.2522
32      0.1817   -1.1972    0.2491  0.1334 -1.2715  0.2681
34      0.1515   -1.1112    0.2739  0.0947 -0.9008  0.3659
36      0.1131   -1.0266    0.3028  0.0779 -0.6964  0.4195
38      0.0747   -0.9428    0.3361  0.0373 -0.5253  0.4520
40      0.0201   -0.8679    0.3677  0.0272 -0.3406  0.4682
42     -0.0456   -0.8050    0.3978 -0.0060 -0.1640  0.4664
44     -0.1200   -0.7559    0.4261 -0.0337  0.0276  0.4571
46     -0.1994   -0.7184    0.4460 -0.0536  0.1857  0.4289
48     -0.2801   -0.6791    0.4385 -0.0670  0.3602  0.3901
50     -0.3642   -0.6522    0.4305 -0.1060  0.5344  0.3447
52     -0.4499   -0.6382    0.4220 -0.1124  0.6934  0.2758
54     -0.5351   -0.6371    0.4131 -0.1432  0.8558  0.2089
56     -0.6157   -0.6512    0.3919 -0.1662  1.0113  0.1179
58     -0.6885   -0.6790    0.3612 -0.1707  1.1730  0.0116

Example 10:
a:0.9 b:0.9 c:0.9 d:0.9 e:0.9 f:0.8 g:0.9 h:0.9 

Landing Position:
  x      y      z      On Table
-0.1086 0.9854 0.0585   True

Paddle Motion and Ball Motion:
      paddle x  paddle y  paddle z  ball x  ball y  ball z
time                                                      
10      0.2534   -1.1233    0.4078  0.3286  0.5157  0.3734
12      0.3171   -1.1983    0.4154  0.3159  0.3313  0.3431
14      0.3672   -1.2817    0.4112  0.3195  0.1002  0.2916
16      0.4281   -1.3584    0.3908  0.2982 -0.0904  0.2239
18      0.4627   -1.4181    0.3597  0.2807 -0.2836  0.1499
20      0.4686   -1.4609    0.3286  0.2894 -0.4753  0.0674
22      0.4377   -1.4839    0.3009  0.2673 -0.6991 -0.0318
24      0.4036   -1.4737    0.2780  0.2537 -0.8089  0.1522
26      0.3690   -1.4355    0.2563  0.2382 -0.9659  0.1980
28      0.3253   -1.3639    0.2389  0.2292 -1.1001  0.2405
30      0.2822   -1.2803    0.2462  0.2222 -1.2484  0.2714
32      0.2493   -1.1836    0.2738  0.1974 -1.1495  0.3131
34      0.2188   -1.1062    0.2944  0.1464 -0.8707  0.3873
36      0.1848   -1.0237    0.3168  0.1201 -0.7021  0.4156
38      0.1404   -0.9449    0.3397  0.0807 -0.5267  0.4338
40      0.0843   -0.8771    0.3619  0.0528 -0.3524  0.4428
42      0.0193   -0.8193    0.3830  0.0304 -0.1817  0.4342
44     -0.0530   -0.7736    0.4028  0.0164 -0.0083  0.4133
46     -0.1249   -0.7260    0.3878 -0.0065  0.1557  0.3699
48     -0.2005   -0.6877    0.3693 -0.0237  0.3199  0.3200
50     -0.2785   -0.6605    0.3505 -0.0525  0.4704  0.2627
52     -0.3572   -0.6445    0.3315 -0.0638  0.6226  0.1854
54     -0.4350   -0.6398    0.3124 -0.0848  0.7783  0.1036
56     -0.5112   -0.6447    0.3045 -0.1079  0.9300  0.0021

Example 11:
a:0.75 b:0.75 c:0.75 d:0.75 e:0.8 f:0.75 g:0.75 h:0.75 

Landing Position:
  x      y      z      On Table
-0.3085 0.3680 0.0325   True

Paddle Motion and Ball Motion:
      paddle x  paddle y  paddle z  ball x  ball y  ball z
time                                                      
10      0.2319   -1.1028    0.4056  0.3235  0.5038  0.3963
12      0.2846   -1.1631    0.4118  0.3194  0.3240  0.3678
14      0.3387   -1.2298    0.4099  0.3053  0.1293  0.3220
16      0.3911   -1.2931    0.3974  0.2994 -0.0820  0.2572
18      0.4301   -1.3455    0.3770  0.2750 -0.2589  0.1839
20      0.4458   -1.3872    0.3541  0.2774 -0.4565  0.1085
22      0.4381   -1.4147    0.3297  0.2583 -0.6354  0.0098
24      0.4159   -1.4293    0.3063  0.2383 -0.7837  0.0992
26      0.3841   -1.4170    0.2838  0.2204 -0.9280  0.2046
28      0.3408   -1.3722    0.2639  0.2003 -1.0676  0.2391
30      0.2936   -1.3107    0.2602  0.1910 -1.2156  0.2802
32      0.2484   -1.2423    0.2832  0.1668 -1.3218  0.2975
34      0.2047   -1.1751    0.3033  0.1125 -1.0168  0.3531
36      0.1663   -1.1095    0.3182  0.0515 -0.8786  0.3707
38      0.1331   -1.0464    0.3348  0.0172 -0.7268  0.3697
40      0.0890   -0.9879    0.3505 -0.0298 -0.5842  0.3719
42      0.0379   -0.9357    0.3656 -0.0660 -0.4455  0.3475
44     -0.0196   -0.8905    0.3798 -0.1085 -0.2941  0.3210
46     -0.0824   -0.8534    0.3932 -0.1567 -0.1624  0.2720
48     -0.1483   -0.8224    0.3994 -0.1949 -0.0246  0.2059
50     -0.2141   -0.7900    0.3838 -0.2342  0.1157  0.1322
52     -0.2827   -0.7652    0.3679 -0.2630  0.2449  0.0445
54     -0.3531   -0.7482    0.3517 -0.3085  0.3680  0.0325

Example 12:
a:0.9 b:0.9 c:0.9 d:0.9 e:1.1 f:0.9 g:0.9 h:0.9 

Landing Position:
  x      y      z      On Table
-0.2369 0.9637 0.0904   True

Paddle Motion and Ball Motion:
      paddle x  paddle y  paddle z  ball x  ball y  ball z
time                                                      
10      0.2380   -1.1203    0.4099  0.2988  0.3320  0.3278
12      0.3464   -1.2449    0.4156  0.2921  0.1159  0.2799
14      0.3681   -1.2801    0.3998  0.2777 -0.0720  0.2106
16      0.4184   -1.3412    0.3721  0.2623 -0.2726  0.1328
18      0.4146   -1.3528    0.3558  0.2615 -0.4614  0.0619
20      0.4218   -1.4269    0.3060  0.2429 -0.6405  0.0285
22      0.3916   -1.4266    0.2849  0.2218 -0.7790  0.1802
24      0.3509   -1.3868    0.2729  0.2159 -0.9203  0.2015
26      0.2928   -1.3294    0.2358  0.1965 -1.0683  0.2413
28      0.2349   -1.2301    0.2369  0.1862 -1.2093  0.2654
30      0.2259   -1.2062    0.2435  0.1625 -1.1450  0.3023
32      0.1621   -1.0522    0.2748  0.1063 -0.8616  0.3605
34      0.1629   -1.0350    0.2802  0.0733 -0.7060  0.3948
36      0.1661   -1.0242    0.2802  0.0446 -0.5171  0.4091
38      0.1671   -1.0119    0.2802  0.0046 -0.3537  0.4108
40      0.1686   -1.0000    0.2802 -0.0411 -0.1805  0.3980
42      0.1701   -0.9881    0.2802 -0.0542 -0.0228  0.3816
44      0.1716   -0.9762    0.2802 -0.0975  0.1531  0.3369
46      0.1731   -0.9643    0.2802 -0.1271  0.3038  0.2935
48      0.1746   -0.9524    0.2802 -0.1535  0.4704  0.2313
50      0.1761   -0.9405    0.2802 -0.1832  0.6245  0.1561
52      0.1775   -0.9286    0.2802 -0.2024  0.7734  0.0657
54      0.1790   -0.9166    0.2802 -0.2320  0.9203 -0.0048

Example 13:
a:0.9 b:0.9 c:0.9 d:0.8 e:0.9 f:0.9 g:0.9 h:0.9 

Landing Position:
  x      y      z      On Table
-0.1976 1.3006 0.0735   True

Paddle Motion and Ball Motion:
      paddle x  paddle y  paddle z  ball x  ball y  ball z
time                                                      
10      0.2494   -1.1381    0.4110  0.3049  0.5487  0.4008
12      0.3168   -1.2186    0.4179  0.2888  0.3478  0.3685
14      0.3667   -1.3094    0.4122  0.2847  0.1403  0.3230
16      0.4142   -1.3903    0.3938  0.2582 -0.0576  0.2691
18      0.4474   -1.4470    0.3673  0.2566 -0.2447  0.1939
20      0.4479   -1.4863    0.3396  0.2413 -0.4417  0.1236
22      0.4176   -1.5048    0.3112  0.2308 -0.6192  0.0307
24      0.3832   -1.5054    0.2835  0.2108 -0.8198  0.0704
26      0.3380   -1.4580    0.2559  0.1953 -0.9234  0.1932
28      0.2953   -1.3918    0.2332  0.1820 -1.0567  0.2168
30      0.2417   -1.3052    0.2343  0.1657 -1.1928  0.2636
32      0.1954   -1.2253    0.2679  0.1544 -1.3199  0.2840
34      0.1576   -1.1426    0.3053  0.1145 -0.9434  0.3798
36      0.1303   -1.0669    0.3321  0.0735 -0.7489  0.4242
38      0.1048   -0.9938    0.3583  0.0562 -0.5179  0.4629
40      0.0633   -0.9282    0.3834  0.0186 -0.3649  0.4685
42      0.0122   -0.8728    0.4070 -0.0198 -0.1717  0.4794
44     -0.0471   -0.8290    0.4287 -0.0431  0.0088  0.4742
46     -0.1098   -0.7911    0.4357 -0.0616  0.1814  0.4477
48     -0.1742   -0.7538    0.4222 -0.0823  0.3530  0.4114
50     -0.2423   -0.7272    0.4082 -0.1009  0.5308  0.3593
52     -0.3125   -0.7119    0.3937 -0.1252  0.6826  0.2975
54     -0.3830   -0.7081    0.3786 -0.1514  0.8560  0.2243
56     -0.4522   -0.7158    0.3632 -0.1716  1.0132  0.1329
58     -0.5145   -0.7381    0.3467 -0.1827  1.1733  0.0407
60     -0.5718   -0.7695    0.3435 -0.1976  1.3006  0.0735

Example 14:
a:0.8 b:0.8 c:1.1 d:0.8 e:0.8 f:0.8 g:0.8 h:1.05 

Landing Position:
  x      y      z      On Table
-0.1948 0.9218 -0.0248   True

Paddle Motion and Ball Motion:
      paddle x  paddle y  paddle z  ball x  ball y  ball z
time                                                      
10      0.2876   -1.1398    0.4068  0.3454  0.5301  0.3903
12      0.3632   -1.2315    0.4150  0.3380  0.3180  0.3447
14      0.4291   -1.3359    0.4105  0.3307  0.1175  0.3062
16      0.4875   -1.4347    0.3897  0.3293 -0.0794  0.2470
18      0.5141   -1.5100    0.3587  0.3063 -0.2726  0.1672
20      0.5110   -1.5622    0.3274  0.3044 -0.4642  0.0858
22      0.4850   -1.5835    0.3019  0.2981 -0.6595 -0.0075
24      0.4509   -1.5695    0.2811  0.2792 -0.7945  0.1195
26      0.4145   -1.5095    0.2631  0.2661 -0.9302  0.1939
28      0.3725   -1.4114    0.2486  0.2536 -1.0600  0.2255
30      0.3201   -1.2997    0.2504  0.2462 -1.2248  0.2595
32      0.2721   -1.1933    0.2720  0.2287 -1.2101  0.2716
34      0.2306   -1.0921    0.2901  0.1639 -0.9075  0.3420
36      0.1912   -1.0001    0.3096  0.1200 -0.7221  0.3709
38      0.1391   -0.9189    0.3355  0.0915 -0.5249  0.3926
40      0.0740   -0.8500    0.3594  0.0505 -0.3350  0.3902
42     -0.0007   -0.7972    0.3824  0.0064 -0.1592  0.3598
44     -0.0818   -0.7616    0.4041 -0.0283  0.0128  0.3471
46     -0.1658   -0.7442    0.4245 -0.0545  0.1962  0.2971
48     -0.2498   -0.7407    0.4346 -0.0948  0.3608  0.2491
50     -0.3339   -0.7424    0.4225 -0.1206  0.5241  0.1840
52     -0.4148   -0.7602    0.4101 -0.1538  0.7014  0.0992
54     -0.4900   -0.7932    0.3972 -0.1852  0.8405  0.0222

Example 15:
a:0.8 b:0.8 c:1.1 d:0.8 e:0.8 f:0.8 g:0.8 h:1.05 

Landing Position:
  x      y      z      On Table
-0.2249 1.1705 0.0667   True

Paddle Motion and Ball Motion:
      paddle x  paddle y  paddle z  ball x  ball y  ball z
time                                                      
10      0.2732   -1.1339    0.4048  0.3371  0.5296  0.3760
12      0.3483   -1.2240    0.4130  0.3304  0.3278  0.3427
14      0.4175   -1.3275    0.4096  0.3243  0.1171  0.2892
16      0.4736   -1.4267    0.3909  0.3080 -0.0660  0.2316
18      0.5031   -1.5081    0.3604  0.3006 -0.2650  0.1567
20      0.5009   -1.5604    0.3298  0.2911 -0.4610  0.0745
22      0.4750   -1.5837    0.3059  0.2866 -0.6449 -0.0179
24      0.4408   -1.5615    0.2837  0.2654 -0.7867  0.1521
26      0.4023   -1.4986    0.2653  0.2619 -0.9398  0.1928
28      0.3568   -1.4012    0.2501  0.2414 -1.0984  0.2487
30      0.3081   -1.2941    0.2517  0.2339 -1.2389  0.2705
32      0.2657   -1.1876    0.2687  0.2378 -1.3216  0.2708
34      0.2232   -1.0896    0.2861  0.1491 -0.8722  0.3647
36      0.1785   -0.9989    0.3107  0.1237 -0.6925  0.3919
38      0.1320   -0.9241    0.3401  0.0790 -0.4828  0.4184
40      0.0678   -0.8619    0.3673  0.0351 -0.2825  0.4095
42     -0.0058   -0.8161    0.3934  0.0083 -0.0897  0.4047
44     -0.0860   -0.7881    0.4182 -0.0278  0.0848  0.3752
46     -0.1688   -0.7789    0.4412 -0.0510  0.2677  0.3463
48     -0.2525   -0.7726    0.4353 -0.0988  0.4435  0.3014
50     -0.3361   -0.7802    0.4245 -0.1184  0.6142  0.2388
52     -0.4166   -0.8038    0.4133 -0.1529  0.7824  0.1713
54     -0.4916   -0.8429    0.4017 -0.1794  0.9455  0.0995
56     -0.5583   -0.8962    0.3898 -0.2148  1.1126 -0.0069

Example 16:
a:0.8 b:0.8 c:1.1 d:0.8 e:0.8 f:0.8 g:0.8 h:1.05 

Landing Position:
  x      y      z      On Table
-0.3200 1.2490 0.0716   True

Paddle Motion and Ball Motion:
      paddle x  paddle y  paddle z  ball x  ball y  ball z
time                                                      
10      0.3027   -1.1486    0.4091  0.3385  0.3829  0.3427
12      0.3762   -1.2410    0.4142  0.3304  0.1765  0.2960
14      0.4356   -1.3417    0.4028  0.3210 -0.0242  0.2343
16      0.4822   -1.4291    0.3733  0.3120 -0.2262  0.1680
18      0.4998   -1.4959    0.3400  0.3105 -0.4116  0.0931
20      0.4897   -1.5381    0.3107  0.2980 -0.5992 -0.0065
22      0.4620   -1.5414    0.2878  0.2765 -0.7400  0.1360
24      0.4265   -1.4996    0.2674  0.2614 -0.8874  0.1893
26      0.3787   -1.4118    0.2509  0.2479 -1.0281  0.2263
28      0.3053   -1.2745    0.2474  0.2423 -1.1676  0.2702
30      0.2709   -1.2014    0.2595  0.2268 -1.3085  0.2840
32      0.2369   -1.0949    0.2694  0.1646 -0.9214  0.3561
34      0.1986   -1.0015    0.2924  0.1153 -0.7539  0.3811
36      0.1432   -0.9190    0.3262  0.0602 -0.5101  0.4148
38      0.0743   -0.8488    0.3572  0.0156 -0.3182  0.4178
40     -0.0050   -0.7951    0.3871 -0.0357 -0.1170  0.4142
42     -0.0912   -0.7594    0.4155 -0.0700  0.0688  0.3978
44     -0.1802   -0.7427    0.4422 -0.1128  0.2533  0.3678
46     -0.2694   -0.7358    0.4511 -0.1481  0.4255  0.3245
48     -0.3588   -0.7365    0.4438 -0.1870  0.5974  0.2694
50     -0.4454   -0.7531    0.4360 -0.2208  0.7748  0.1988
52     -0.5266   -0.7850    0.4278 -0.2602  0.9452  0.1284
54     -0.5998   -0.8311    0.4191 -0.2966  1.1073  0.0325
56     -0.6627   -0.8900    0.4100 -0.3200  1.2490  0.0716

Example 17:
a:0.8 b:0.8 c:1.1 d:0.8 e:0.8 f:0.8 g:0.8 h:1.05 

Landing Position:
  x      y      z      On Table
-0.3083 0.8977 -0.0202   True

Paddle Motion and Ball Motion:
      paddle x  paddle y  paddle z  ball x  ball y  ball z
time                                                      
10      0.2684   -1.1383    0.4065  0.3079  0.5673  0.4120
12      0.3382   -1.2319    0.4148  0.2916  0.3450  0.3716
14      0.3966   -1.3390    0.4118  0.2820  0.1426  0.3303
16      0.4429   -1.4422    0.3941  0.2700 -0.0578  0.2731
18      0.4682   -1.5263    0.3669  0.2569 -0.2720  0.1970
20      0.4661   -1.5860    0.3376  0.2375 -0.4300  0.1204
22      0.4375   -1.6189    0.3114  0.2358 -0.6194  0.0371
24      0.3988   -1.6177    0.2906  0.2026 -0.7775  0.0528
26      0.3588   -1.5694    0.2733  0.1919 -0.9035  0.1846
28      0.3175   -1.4807    0.2593  0.1729 -1.0444  0.2153
30      0.2631   -1.3729    0.2560  0.1567 -1.1790  0.2566
32      0.2015   -1.2629    0.2734  0.1398 -1.3126  0.2746
34      0.1476   -1.1627    0.2952  0.1066 -1.1100  0.3270
36      0.1047   -1.0678    0.3146  0.0410 -0.8275  0.3700
38      0.0634   -0.9854    0.3381  0.0090 -0.6610  0.3983
40      0.0038   -0.9123    0.3602 -0.0305 -0.4902  0.4127
42     -0.0657   -0.8527    0.3811 -0.0632 -0.3084  0.4013
44     -0.1431   -0.8082    0.4005 -0.1004 -0.1396  0.3829
46     -0.2252   -0.7800    0.4182 -0.1412  0.0330  0.3516
48     -0.3089   -0.7653    0.4278 -0.1864  0.2079  0.3054
50     -0.3930   -0.7531    0.4121 -0.2024  0.3329  0.2581
52     -0.4761   -0.7559    0.3959 -0.2389  0.5167  0.1826
54     -0.5553   -0.7731    0.3791 -0.2702  0.6723  0.1048
56     -0.6284   -0.8040    0.3618 -0.2903  0.8258  0.0113

Example 18:
a:0.8 b:0.8 c:1.1 d:0.8 e:0.8 f:0.8 g:0.8 h:1.05 

Landing Position:
  x      y      z      On Table
-0.2808 1.0771 0.0277   True

Paddle Motion and Ball Motion:
      paddle x  paddle y  paddle z  ball x  ball y  ball z
time                                                      
10      0.2846   -1.1391    0.4069  0.3321  0.5290  0.3800
12      0.3552   -1.2329    0.4154  0.3274  0.3276  0.3525
14      0.4115   -1.3353    0.4106  0.3248  0.1175  0.3104
16      0.4699   -1.4369    0.3888  0.3068 -0.0785  0.2396
18      0.5020   -1.5146    0.3584  0.3040 -0.2683  0.1662
20      0.5025   -1.5665    0.3279  0.2984 -0.4592  0.0920
22      0.4657   -1.5919    0.3016  0.2836 -0.6494 -0.0002
24      0.4281   -1.5752    0.2799  0.2656 -0.7717  0.1232
26      0.4016   -1.5079    0.2622  0.2498 -0.9557  0.2061
28      0.3582   -1.4125    0.2497  0.2330 -1.0721  0.2349
30      0.3079   -1.3066    0.2510  0.2310 -1.2091  0.2639
32      0.2539   -1.2010    0.2711  0.2057 -1.2700  0.2824
34      0.2067   -1.1016    0.2893  0.1333 -0.9228  0.3477
36      0.1735   -1.0123    0.3091  0.0908 -0.7043  0.3722
38      0.1160   -0.9327    0.3369  0.0508 -0.5088  0.3984
40      0.0454   -0.8677    0.3622  0.0006 -0.3136  0.3865
42     -0.0348   -0.8175    0.3864 -0.0293 -0.1313  0.3731
44     -0.1217   -0.7841    0.4092 -0.0717  0.0566  0.3580
46     -0.2118   -0.7686    0.4304 -0.1047  0.2344  0.3226
48     -0.3023   -0.7658    0.4406 -0.1445  0.4130  0.2616
50     -0.3932   -0.7679    0.4296 -0.1883  0.5928  0.2040
52     -0.4817   -0.7856    0.4181 -0.2149  0.7495  0.1379
54     -0.5651   -0.8183    0.4061 -0.2498  0.9174  0.0544
56     -0.6409   -0.8650    0.3937 -0.2808  1.0771  0.0277

Example 19:
a:0.8 b:0.8 c:1.1 d:0.8 e:0.8 f:0.8 g:0.8 h:1.05 

Landing Position:
  x      y      z      On Table
-0.2340 0.7977 0.0434   True

Paddle Motion and Ball Motion:
      paddle x  paddle y  paddle z  ball x  ball y  ball z
time                                                      

10      0.2903   -1.1388    0.4054  0.3249  0.5226  0.3716
12      0.3593   -1.2299    0.4130  0.3312  0.3084  0.3329
14      0.4186   -1.3338    0.4088  0.3235  0.0983  0.2826
16      0.4668   -1.4321    0.3879  0.3058 -0.0973  0.2204
18      0.4984   -1.5059    0.3565  0.3003 -0.2935  0.1440
20      0.4985   -1.5544    0.3261  0.2954 -0.4744  0.0687
22      0.4745   -1.5717    0.3014  0.2829 -0.6820 -0.0263
24      0.4388   -1.5468    0.2805  0.2599 -0.8159  0.1490
26      0.3985   -1.4784    0.2616  0.2486 -0.9610  0.1912
28      0.3473   -1.3765    0.2482  0.2343 -1.1166  0.2387
30      0.2900   -1.2680    0.2546  0.2370 -1.2542  0.2596
32      0.2407   -1.1635    0.2749  0.1976 -1.1026  0.3081
34      0.2105   -1.0652    0.2923  0.1277 -0.8480  0.3409
36      0.1433   -0.9496    0.3280  0.0949 -0.6821  0.3629
38     -0.0079   -0.8317    0.3781  0.0531 -0.5034  0.3707
40     -0.1884   -0.7814    0.4230  0.0056 -0.3271  0.3560
42     -0.3742   -0.7808    0.4198 -0.0105 -0.1643  0.3334
44     -0.5503   -0.8334    0.3938 -0.0671  0.0228  0.3038
46     -0.6954   -0.9429    0.3662 -0.1025  0.1793  0.2546
48     -0.7921   -1.0954    0.3371 -0.1349  0.3394  0.1950
50     -0.8233   -1.2695    0.3227 -0.1619  0.5023  0.1232
52     -0.7954   -1.2632    0.3125 -0.2054  0.6506  0.0413
54     -0.7623   -1.2330    0.3021 -0.2340  0.7977  0.0434

Example 20:
a:0.8 b:0.8 c:1.1 d:0.8 e:0.8 f:0.8 g:0.8 h:1.05 

Landing Position:
  x      y      z      On Table
-0.2539 1.1478 0.0459   True

Paddle Motion and Ball Motion:
      paddle x  paddle y  paddle z  ball x  ball y  ball z
time                                                      
10      0.2738   -1.1357    0.4058  0.3151  0.5366  0.3833
12      0.3419   -1.2269    0.4142  0.3050  0.3348  0.3408
14      0.4023   -1.3310    0.4124  0.2933  0.1347  0.2871
16      0.4528   -1.4309    0.3938  0.2853 -0.0587  0.2328
18      0.4800   -1.5111    0.3642  0.2791 -0.2435  0.1640
20      0.4784   -1.5631    0.3340  0.2631 -0.4197  0.0824
22      0.4567   -1.5863    0.3080  0.2583 -0.6211 -0.0194
24      0.4245   -1.5683    0.2868  0.2379 -0.7440  0.1456
26      0.3854   -1.5062    0.2673  0.2276 -0.8916  0.2000
28      0.3326   -1.4092    0.2515  0.2157 -1.0352  0.2411
30      0.2820   -1.3021    0.2527  0.2053 -1.1722  0.2673
32      0.2457   -1.1969    0.2682  0.1940 -1.2934  0.2796
34      0.2148   -1.0996    0.2819  0.1292 -0.8936  0.3592
36      0.1626   -1.0080    0.3017  0.0975 -0.7381  0.3830
38      0.1012   -0.9297    0.3289  0.0623 -0.5129  0.4139
40      0.0268   -0.8632    0.3539  0.0253 -0.3272  0.4176
42     -0.0575   -0.8122    0.3779 -0.0126 -0.1277  0.4054
44     -0.1485   -0.7780    0.4006 -0.0483  0.0452  0.3860
46     -0.2426   -0.7616    0.4217 -0.0713  0.2270  0.3508
48     -0.3373   -0.7548    0.4255 -0.1158  0.3954  0.3112
50     -0.4320   -0.7558    0.4132 -0.1444  0.5795  0.2479
52     -0.5241   -0.7722    0.4005 -0.1857  0.7510  0.1795
54     -0.6108   -0.8035    0.3874 -0.2257  0.9165  0.1018
56     -0.6898   -0.8485    0.3738 -0.2426  1.0791  0.0001

Example 21:
a:0.8 b:0.8 c:1.1 d:0.8 e:0.8 f:0.8 g:0.8 h:1.05 

Landing Position:
  x      y      z      On Table
-0.3401 0.8968 0.0296   True

Paddle Motion and Ball Motion:
      paddle x  paddle y  paddle z  ball x  ball y  ball z
time                                                      
10      0.2795   -1.1413    0.4073  0.2967  0.5224  0.3822
12      0.3468   -1.2357    0.4153  0.2798  0.3114  0.3417
14      0.3998   -1.3427    0.4115  0.2710  0.1161  0.3003
16      0.4450   -1.4442    0.3925  0.2487 -0.0784  0.2410
18      0.4635   -1.5238    0.3628  0.2394 -0.2807  0.1682
20      0.4568   -1.5740    0.3335  0.2241 -0.4593  0.0833
22      0.4342   -1.6040    0.3079  0.2103 -0.6473 -0.0066
24      0.3945   -1.5912    0.2869  0.1884 -0.7803  0.1381
26      0.3435   -1.5383    0.2672  0.1704 -0.9252  0.1986
28      0.2817   -1.4502    0.2517  0.1526 -1.0663  0.2381
30      0.2305   -1.3373    0.2525  0.1376 -1.2030  0.2645
32      0.1806   -1.2382    0.2674  0.1233 -1.3244  0.2736
34      0.1386   -1.1331    0.2823  0.0543 -0.9659  0.3451
36      0.0851   -1.0413    0.3037  0.0186 -0.7985  0.3747
38      0.0275   -0.9572    0.3308 -0.0248 -0.5985  0.3854
40     -0.0461   -0.8841    0.3556 -0.0620 -0.4190  0.3876
42     -0.1299   -0.8253    0.3791 -0.1161 -0.2355  0.3754
44     -0.2212   -0.7825    0.4012 -0.1399 -0.0670  0.3528
46     -0.3167   -0.7568    0.4215 -0.1840  0.0999  0.3204
48     -0.4134   -0.7436    0.4310 -0.2077  0.2779  0.2674
50     -0.5107   -0.7346    0.4182 -0.2431  0.4394  0.2040
52     -0.6063   -0.7407    0.4048 -0.2806  0.6005  0.1339
54     -0.6978   -0.7615    0.3907 -0.3062  0.7554  0.0415
56     -0.7826   -0.7962    0.3761 -0.3401  0.8968  0.0296

Example 22:
a:0.8 b:0.8 c:1.1 d:0.8 e:0.8 f:0.8 g:0.8 h:1.05 

Landing Position:
  x      y      z      On Table
-0.3218 1.1070 -0.0111   True

Paddle Motion and Ball Motion:
      paddle x  paddle y  paddle z  ball x  ball y  ball z
time                                                      
10      0.2721   -1.1313    0.4049  0.3196  0.5624  0.3755
12      0.3453   -1.2202    0.4131  0.3055  0.3420  0.3359
14      0.4026   -1.3247    0.4103  0.3069  0.1341  0.2866
16      0.4525   -1.4228    0.3915  0.2792 -0.0631  0.2256
18      0.4842   -1.5019    0.3620  0.2721 -0.2516  0.1518
20      0.4846   -1.5563    0.3318  0.2596 -0.4407  0.0666
22      0.4556   -1.5815    0.3059  0.2414 -0.6224 -0.0182
24      0.4198   -1.5682    0.2848  0.2225 -0.7541  0.1608
26      0.3767   -1.5090    0.2664  0.2145 -0.9036  0.2045
28      0.3237   -1.4139    0.2515  0.1879 -1.0531  0.2428
30      0.2658   -1.3083    0.2534  0.1790 -1.1848  0.2683
32      0.2130   -1.2079    0.2661  0.1738 -1.3036  0.2816
34      0.1640   -1.1032    0.2766  0.1036 -0.9431  0.3578
36      0.1296   -1.0172    0.2945  0.0469 -0.7403  0.3828
38      0.0819   -0.9361    0.3261  0.0131 -0.5407  0.4118
40      0.0180   -0.8678    0.3540 -0.0379 -0.3457  0.4292
42     -0.0562   -0.8152    0.3807 -0.0738 -0.1649  0.4023
44     -0.1377   -0.7799    0.4059 -0.1172  0.0295  0.3895
46     -0.2227   -0.7630    0.4292 -0.1348  0.1847  0.3544
48     -0.3082   -0.7592    0.4410 -0.1771  0.3710  0.3143
50     -0.3943   -0.7603    0.4312 -0.2180  0.5336  0.2559
52     -0.4779   -0.7773    0.4208 -0.2492  0.7004  0.1820
54     -0.5564   -0.8097    0.4098 -0.2759  0.8685  0.1012
56     -0.6272   -0.8563    0.3982 -0.3056  1.0324  0.0074

Example 23:
a:0.9 b:0.9 c:0.9 d:1.08 e:0.9 f:0.9 g:0.9 h:0.9 

Landing Position:
  x      y      z      On Table
-0.0617 0.7514 -0.0206   True

Paddle Motion and Ball Motion:
      paddle x  paddle y  paddle z  ball x  ball y  ball z
time                                                      
10      0.0693   -1.0921    0.3905  0.2654  0.3841  0.3539
12      0.0004   -1.1571    0.3800  0.2476  0.1999  0.3036
14     -0.0603   -1.2395    0.3607  0.2229  0.0071  0.2498
16     -0.0944   -1.3303    0.3309  0.2152 -0.1858  0.1796
18     -0.0991   -1.3964    0.2921  0.1949 -0.3773  0.0953
20     -0.0820   -1.3937    0.2692  0.1712 -0.5548  0.0013
22     -0.0596   -1.3658    0.2529  0.1562 -0.6942  0.1082
24     -0.0372   -1.3217    0.2437  0.1326 -0.8377  0.2010
26      0.0069   -1.2764    0.2480  0.1130 -0.9774  0.2445
28      0.0298   -1.2160    0.2644  0.0953 -1.1128  0.2647
30      0.0588   -1.1656    0.2789  0.0723 -1.2408  0.2919
32      0.0571   -1.1064    0.2954  0.0734 -1.0723  0.3418
34      0.0418   -1.0370    0.3307  0.0717 -0.8215  0.4045
36      0.0271   -0.9814    0.3715  0.0601 -0.6746  0.4421
38      0.0166   -0.9288    0.4118  0.0563 -0.5273  0.4581
40      0.0102   -0.8818    0.4506  0.0345 -0.3733  0.4522
42      0.0070   -0.8400    0.4864  0.0304 -0.2257  0.4430
44      0.0061   -0.8031    0.5181  0.0222 -0.0737  0.4156
46      0.0063   -0.7708    0.5446  0.0214  0.0656  0.3733
48      0.0064   -0.7425    0.5653  0.0042  0.2158  0.3173
50      0.0064   -0.7201    0.5504 -0.0147  0.3511  0.2486
52      0.0044   -0.7017    0.5274 -0.0246  0.4913  0.1641
54     -0.0003   -0.6878    0.4994 -0.0395  0.6223  0.0709
56     -0.0081   -0.6788    0.4677 -0.0617  0.7514 -0.0206

Example 24:
a:0.8 b:0.8 c:1.1 d:0.8 e:0.8 f:0.8 g:0.8 h:1.05 

Landing Position:
  x      y      z      On Table
-0.3652 1.0083 0.0244   True

Paddle Motion and Ball Motion:
      paddle x  paddle y  paddle z  ball x  ball y  ball z
time                                                      
10      0.3002   -1.1458    0.4076  0.3347  0.4841  0.3628
12      0.3720   -1.2375    0.4138  0.3217  0.2888  0.3282
14      0.4409   -1.3536    0.4042  0.3236  0.0857  0.2776
16      0.4783   -1.4309    0.3806  0.3037 -0.0989  0.2105
18      0.5004   -1.5011    0.3503  0.2977 -0.3270  0.1285
20      0.4904   -1.5491    0.3221  0.2915 -0.5004  0.0413
22      0.4732   -1.5627    0.2986  0.2738 -0.6559  0.0358
24      0.4373   -1.5310    0.2774  0.2614 -0.7697  0.1691
26      0.3893   -1.4560    0.2569  0.2383 -0.9261  0.2092
28      0.3477   -1.3614    0.2461  0.2243 -1.0637  0.2534
30      0.2964   -1.2473    0.2556  0.2255 -1.1810  0.2723
32      0.2462   -1.1523    0.2714  0.1878 -1.1871  0.2838
34      0.1880   -1.0466    0.2865  0.1201 -0.8642  0.3534
36      0.1421   -0.9626    0.3068  0.0744 -0.6807  0.3827
38      0.0865   -0.8866    0.3287  0.0302 -0.4857  0.4042
40      0.0196   -0.8222    0.3499 -0.0186 -0.3097  0.3973
42     -0.0571   -0.7732    0.3706 -0.0680 -0.1282  0.3970
44     -0.1404   -0.7410    0.3906 -0.1136  0.0383  0.3618
46     -0.2271   -0.7267    0.4099 -0.1643  0.2226  0.3251
48     -0.3136   -0.7307    0.4283 -0.2062  0.3809  0.2756
50     -0.3965   -0.7524    0.4456 -0.2337  0.5460  0.2059
52     -0.4734   -0.7897    0.4594 -0.2945  0.7008  0.1378
54     -0.5485   -0.8330    0.4553 -0.3215  0.8629  0.0518
56     -0.6151   -0.8908    0.4509 -0.3652  1.0083  0.0244

--------------- Forehand Stroke Examples:

The numbers in the above examples hold the landing positions of a table tennis ball on the table. The total set of examples is divided into examples for forehand strokes and examples for backhand strokes. In addition, you are also provided with the motion of the paddle and ball during each example. Regarding the size and dimensions of the table tennis table: the x dimension (along the width of the table) is in the range [-0.76, 0.76], the y dimension (along the depth of the table) is in the range [-1.37,1.37] and z dimension (the height) is in the range [0.0, 2.0]. Positive x values are on the right side of the table tennis table, whereas negative x values are on the left side of the table tennis table. Forward is along the positive y direction, whereas backwards means moving towards the negative y direction. The center of the table is at [x = 0, y = 0].  Positive values of y mean that the ball is landing on the opponents side. Negative values of y mean that the ball is landing prematurely on our side. The net is at y = 0. Absolute values of y < 0.4 can be considered close to the net. The ball trajectory and the trajectory of the paddle can be found in the tables holding the paddle motion.

Objective: Hit the ball as far right as possible

Step 1: Create a table that summarizes for each example the landing position (how far on left/right, the peak height, estimated speed) of the ball. The text paragraph should be precise (provide evidence) and can be lengthy. The table should also hold the corresponding parameter values a,b,c,d,e,f,g,h as well as the strokestyle. The parameters control the robot which generated these examples.

Step 2: From the table above give me the parameters that are closest to fulfilling the above objective.

Step 3: Take these parameters and the summary table and analyze the effect of the parameters a,b,c,d,e,f,g,h on landing position. Let's think step by step!

Step 4: Based on this analysis, propose a new set of values for the parameters which will bring us closer to the objective than any of the previous examples. Avoid parameters that hit the ball outside of the table. Use exactly the following format and do not write anything else:

Proposed params:<-- here you provide the proposed parameters a,b,c,d,e,f,g,h. Make sure to write it like this example a:0 b:0 c:0 d:0 e:0 f:0 g:0 h:0 including the letters
Best strokestyle:<-- here you provide whether the proposed stroke is FH (forehand) or BH (backhand); always make sure to have this strokestyle specification in all your responses! DO NOT OMIT THIS!!

## Step 1: Summary Table

| Example | Stroke Style | x (Landing Position) | z (Peak Height) | Estimated Speed | a | b | c | d | e | f | g | h |
|---|---|---|---|---|---|---|---|---|---|---|---|---|
| 1 | FH | -0.2978 | 0.3763 | Medium | 0.75 | 0.75 | 0.75 | 0.75 | 1.1 | 0.75 | 0.75 | 0.75 |
| 2 | FH | -0.2155 | 0.3952 | Medium | 0.9 | 0.9 | 0.9 | 0.9 | 0.8 | 0.9 | 0.9 | 0.9 |
| 3 | FH | -0.1632 | 0.3898 | Medium | 0.75 | 0.75 | 0.75 | 0.75 | 0.75 | 0.75 | 1.1 | 0.75 |
| 4 | FH | -0.0872 | 0.3898 | Medium | 0.87 | 0.87 | 0.87 | 0.87 | 0.87 | 0.87 | 0.87 | 1.23 |
| 5 | FH | -0.3773 | 0.3639 | Medium | 0.9 | 0.9 | 0.9 | 0.9 | 0.9 | 0.6 | 0.9 | 0.9 |
| 6 | FH | -0.1330 | 0.3363 | Medium | 0.9 | 0.9 | 0.9 | 0.9 | 0.9 | 1.1 | 0.9 | 0.9 |
| 7 | FH | -0.2439 | 0.2464 | Medium | 0.87 | 0.87 | 0.87 | 0.87 | 0.87 | 0.87 | 0.87 | 1.2 |
| 8 | FH | -0.1013 | 0.3609 | Medium | 0.8 | 0.8 | 1.1 | 0.8 | 0.8 | 0.8 | 0.8 | 0.8 |
| 9 | FH | -0.1778 | 0.3666 | Medium | 0.95 | 0.95 | 0.95 | 0.8 | 0.95 | 0.95 | 0.95 | 0.95 |
| 10 | FH | -0.1086 | 0.3734 | Medium | 0.9 | 0.9 | 0.9 | 0.9 | 0.9 | 0.8 | 0.9 | 0.9 |
| 11 | FH | -0.3085 | 0.3963 | Medium | 0.75 | 0.75 | 0.75 | 0.75 | 0.8 | 0.75 | 0.75 | 0.75 |
| 12 | FH | -0.2369 | 0.3278 | Medium | 0.9 | 0.9 | 0.9 | 0.9 | 1.1 | 0.9 | 0.9 | 0.9 |
| 13 | FH | -0.1976 | 0.4008 | Medium | 0.9 | 0.9 | 0.9 | 0.8 | 0.9 | 0.9 | 0.9 | 0.9 |
| 14 | FH | -0.1948 | 0.3903 | Medium | 0.8 | 0.8 | 1.1 | 0.8 | 0.8 | 0.8 | 0.8 | 1.05 |
| 15 | FH | -0.2249 | 0.3760 | Medium | 0.8 | 0.8 | 1.1 | 0.8 | 0.8 | 0.8 | 0.8 | 1.05 |
| 16 | FH | -0.3200 | 0.3427 | Medium | 0.8 | 0.8 | 1.1 | 0.8 | 0.8 | 0.8 | 0.8 | 1.05 |
| 17 | FH | -0.3083 | 0.4120 | Medium | 0.8 | 0.8 | 1.1 | 0.8 | 0.8 | 0.8 | 0.8 | 1.05 |
| 18 | FH | -0.2808 | 0.3800 | Medium | 0.8 | 0.8 | 1.1 | 0.8 | 0.8 | 0.8 | 0.8 | 1.05 |
| 19 | FH | -0.2340 | 0.3716 | Medium | 0.8 | 0.8 | 1.1 | 0.8 | 0.8 | 0.8 | 0.8 | 1.05 |
| 20 | FH | -0.2539 | 0.3833 | Medium | 0.8 | 0.8 | 1.1 | 0.8 | 0.8 | 0.8 | 0.8 | 1.05 |
| 21 | FH | -0.3401 | 0.3822 | Medium | 0.8 | 0.8 | 1.1 | 0.8 | 0.8 | 0.8 | 0.8 | 1.05 |
| 22 | FH | -0.3218 | 0.3755 | Medium | 0.8 | 0.8 | 1.1 | 0.8 | 0.8 | 0.8 | 0.8 | 1.05 |
| 23 | FH | -0.0617 | 0.3539 | Medium | 0.9 | 0.9 | 0.9 | 1.08 | 0.9 | 0.9 | 0.9 | 0.9 |
| 24 | FH | -0.3652 | 0.3628 | Medium | 0.8 | 0.8 | 1.1 | 0.8 | 0.8 | 0.8 | 0.8 | 1.05 |

**Observations:**

* **Landing Position:**  Most examples land the ball in the negative x range, meaning they land on the left side of the table. The most right landing is achieved in example 4 with x = -0.0872.
* **Peak Height:** The peak height of the ball varies but mostly stays in the range of 0.3 to 0.4, with the highest peak at 0.4120 in example 17.
* **Speed:** The estimated speed seems to be relatively consistent across examples, suggesting a medium speed for all strokes.
* **Parameters:** The parameters "a" to "h" have a varied influence on the ball trajectory, which is further explored in the next steps.

## Step 2: Closest Parameters to Objective

The parameters closest to fulfilling the objective (hitting the ball as far right as possible) are:

**Example 4: a:0.87 b:0.87 c:0.87 d:0.87 e:0.87 f:0.87 g:0.87 h:1.23** 

This example lands the ball at x = -0.0872, which is the most right landing position out of all the examples provided.

## Step 3: Parameter Analysis

Based on the provided data and the summary table, here's a preliminary analysis of the parameters:

* **a, b, c, d:** These parameters seem to primarily influence the initial direction of the paddle and the ball. Higher values tend to result in a more pronounced forward motion of the paddle and ball, leading to a higher trajectory and a slightly more rightward landing position.  For example, Example 2 (a,b,c,d = 0.9) lands slightly more to the right than Example 1 (a,b,c,d = 0.75).
* **e:** This parameter appears to affect the angle of the paddle relative to the ball.  Higher values of "e" seem to lead to a steeper paddle angle and a higher trajectory. 
* **f:**  A higher value for "f" suggests a more pronounced downward motion of the paddle at the start of the stroke, which results in a steeper trajectory.
* **g:** This parameter, with higher values, seems to correspond to a longer paddle contact with the ball, which can result in a faster ball speed and a more rightward landing position.
* **h:** This parameter appears to heavily impact the force and spin applied to the ball.  A higher "h" value corresponds to a more powerful hit and a higher arc, potentially leading to a further landing position. 

It's important to note that these are just initial observations based on the provided data. A more comprehensive analysis would require a larger dataset and potentially advanced statistical methods.

## Step 4: Parameter Proposal

Proposed params: **a:0.9 b:0.9 c:0.9 d:0.9 e:0.9 f:1.1 g:1.1 h:1.25**

Best strokestyle: **FH**

**Explanation:**

* We increased **"a"**, **"b"**, **"c"**, and **"d"** to 0.9, aiming to improve the initial paddle and ball movement and potentially push the ball slightly more to the right.
* **"e"** is set to 0.9, hoping for a steeper angle that contributes to a higher trajectory.
* **"f"** is increased to 1.1, aiming for a more pronounced downward motion of the paddle, which might help in controlling the trajectory.
* We increased **"g"** to 1.1 for a longer paddle contact, hoping for a faster ball speed and a more rightward landing position.
* Finally, we increased **"h"** to 1.25 for a more powerful hit and potentially a further landing position.

This combination of parameters attempts to optimize the stroke for a more powerful and accurate hit, aiming to achieve a landing position further right than any of the previous examples while remaining within the table boundaries. 

<q> Hit the ball as far right as possible
## Step 1: Summary Table

| Example | Stroke | a | b | c | d | e | f | g | h | x (landing) | Peak Height (z) | Estimated Speed |
|---|---|---|---|---|---|---|---|---|---|---|---|---|
| 1 | FH | 0.75 | 0.75 | 0.75 | 0.75 | 1.1 | 0.75 | 0.75 | 0.75 | -0.2978 | 0.4059 (at time 12) | Medium |
| 2 | FH | 0.9 | 0.9 | 0.9 | 0.9 | 0.8 | 0.9 | 0.9 | 0.9 | -0.2155 | 0.4211 (at time 12) | Medium |
| 3 | FH | 0.75 | 0.75 | 0.75 | 0.75 | 0.75 | 0.75 | 1.1 | 0.75 | -0.1632 | 0.4246 (at time 12) | Medium |
| 4 | FH | 0.87 | 0.87 | 0.87 | 0.87 | 0.87 | 0.87 | 0.87 | 1.23 | -0.0872 | 0.4131 (at time 12) | Medium |
| 5 | FH | 0.9 | 0.9 | 0.9 | 0.9 | 0.9 | 0.6 | 0.9 | 0.9 | -0.3773 | 0.4167 (at time 12) | Medium |
| 6 | FH | 0.9 | 0.9 | 0.9 | 0.9 | 0.9 | 1.1 | 0.9 | 0.9 | -0.1330 | 0.4210 (at time 12) | Medium |
| 7 | FH | 0.87 | 0.87 | 0.87 | 0.87 | 0.87 | 0.87 | 0.87 | 1.2 | -0.2439 | 0.4089 (at time 10) | Medium |
| 8 | FH | 0.8 | 0.8 | 1.1 | 0.8 | 0.8 | 0.8 | 0.8 | 0.8 | -0.1013 | 0.4134 (at time 12) | Medium |
| 9 | FH | 0.95 | 0.95 | 0.95 | 0.8 | 0.95 | 0.95 | 0.95 | 0.95 | -0.1778 | 0.4177 (at time 12) | Medium |
| 10 | FH | 0.9 | 0.9 | 0.9 | 0.9 | 0.9 | 0.8 | 0.9 | 0.9 | -0.1086 | 0.4154 (at time 12) | Medium |
| 11 | FH | 0.75 | 0.75 | 0.75 | 0.75 | 0.8 | 0.75 | 0.75 | 0.75 | -0.3085 | 0.4118 (at time 12) | Medium |
| 12 | FH | 0.9 | 0.9 | 0.9 | 0.9 | 1.1 | 0.9 | 0.9 | 0.9 | -0.2369 | 0.4156 (at time 12) | Medium |
| 13 | FH | 0.9 | 0.9 | 0.9 | 0.8 | 0.9 | 0.9 | 0.9 | 0.9 | -0.1976 | 0.4179 (at time 12) | Medium |
| 14 | FH | 0.8 | 0.8 | 1.1 | 0.8 | 0.8 | 0.8 | 0.8 | 1.05 | -0.1948 | 0.4150 (at time 12) | Medium |
| 15 | FH | 0.8 | 0.8 | 1.1 | 0.8 | 0.8 | 0.8 | 0.8 | 1.05 | -0.2249 | 0.4130 (at time 12) | Medium |
| 16 | FH | 0.8 | 0.8 | 1.1 | 0.8 | 0.8 | 0.8 | 0.8 | 1.05 | -0.3200 | 0.4142 (at time 12) | Medium |
| 17 | FH | 0.8 | 0.8 | 1.1 | 0.8 | 0.8 | 0.8 | 0.8 | 1.05 | -0.3083 | 0.4148 (at time 12) | Medium |
| 18 | FH | 0.8 | 0.8 | 1.1 | 0.8 | 0.8 | 0.8 | 0.8 | 1.05 | -0.2808 | 0.4154 (at time 12) | Medium |
| 19 | FH | 0.8 | 0.8 | 1.1 | 0.8 | 0.8 | 0.8 | 0.8 | 1.05 | -0.2340 | 0.4130 (at time 12) | Medium |
| 20 | FH | 0.8 | 0.8 | 1.1 | 0.8 | 0.8 | 0.8 | 0.8 | 1.05 | -0.2539 | 0.4142 (at time 12) | Medium |
| 21 | FH | 0.8 | 0.8 | 1.1 | 0.8 | 0.8 | 0.8 | 0.8 | 1.05 | -0.3401 | 0.4153 (at time 12) | Medium |
| 22 | FH | 0.8 | 0.8 | 1.1 | 0.8 | 0.8 | 0.8 | 0.8 | 1.05 | -0.3218 | 0.4131 (at time 12) | Medium |
| 23 | BH | 0.9 | 0.9 | 0.9 | 1.08 | 0.9 | 0.9 | 0.9 | 0.9 | -0.0617 | 0.3905 (at time 10) | Medium |
| 24 | FH | 0.8 | 0.8 | 1.1 | 0.8 | 0.8 | 0.8 | 0.8 | 1.05 | -0.3652 | 0.4138 (at time 12) | Medium |
| 25 | FH | 0.9 | 0.9 | 0.9 | 0.9 | 0.9 | 1.1 | 1.1 | 1.25 | 0.0797 | 0.4248 (at time 12) | Medium | 

**Analysis of the Summary Table:**

- **Landing Position:** The goal is to hit the ball as far right as possible. Positive x values indicate the ball landing on the right side of the table.  The forehand strokes generally have a more negative x landing position than the backhand strokes. 
- **Peak Height:** The peak height of the ball is generally around 0.4. This is a good indication that the ball is clearing the net (at z = 0.0).
- **Estimated Speed:** The estimated speed for all the examples is Medium. This indicates that the speed of the ball is appropriate for table tennis.

**Note:** The estimated speed was determined based on the time taken for the ball to travel. A longer time suggests a slower speed, while a shorter time suggests a faster speed. 

## Step 2: Closest Parameters

The closest parameters to fulfilling the objective are:

**Example 25:  a:0.9 b:0.9 c:0.9 d:0.9 e:0.9 f:1.1 g:1.1 h:1.25** 

This example is the only one with a positive x landing position, meaning the ball landed on the right side of the table.

## Step 3: Analysis of Parameter Effects

**Parameter a, b, c, d:** These parameters seem to influence the initial trajectory of the ball, but their impact on the final landing position is less clear from the data. 

**Parameter e:** A higher value of 'e' (like in example 1) seems to result in a more negative x landing position, meaning the ball lands further to the left.

**Parameter f:** A higher value of 'f' (like in examples 6 and 25) seems to shift the landing position towards positive x values, meaning further to the right.

**Parameter g:**  A higher value of 'g' (like in examples 3, 8, 14, 15, 16, 17, 18, 19, 20, 21, 22, 24, and 25) does not seem to have a consistent influence on the final landing position. However, it could be affecting the initial trajectory, leading to slightly different landing positions.

**Parameter h:** A higher value of 'h' (like in examples 4, 7, and 25) generally results in a more positive x landing position, meaning further to the right. This parameter seems to be crucial for hitting the ball farther right.

## Step 4: Proposed Parameters

Proposed params: **a:0.9 b:0.9 c:0.9 d:0.9 e:0.8 f:1.1 g:1.1 h:1.35**
Best strokestyle: **FH** 

**Explanation:**

-  We are using the parameters from Example 25 as a base since it is the only one that achieved a positive x landing position.
-  Slightly increasing 'h' to 1.35 could potentially result in a further right landing position.  
- Keeping other parameters like 'g' relatively high could further improve the trajectory and result in a more favorable outcome. 
- This combination aims to enhance the impact of parameter 'h' and maximize the ball's movement to the right. 

**Important Note:** The above analysis is based on the limited data provided. More examples and experimentation with these parameters are required for a more conclusive understanding of their individual and combined effects on the ball trajectory and landing position. 

<q> Hit the ball as far right as possible
## Step 1: Summary Table

| Example | Stroke | a | b | c | d | e | f | g | h | x (landing) |  y (landing) |  z (landing) |  Peak Height | Estimated Speed |
|---|---|---|---|---|---|---|---|---|---|---|---|---|---|---|
| 1 | FH | 0.75 | 0.75 | 0.75 | 0.75 | 1.1 | 0.75 | 0.75 | 0.75 | -0.2978 | 0.4482 | 0.0089 | 0.5031 | Medium |
| 2 | FH | 0.9 | 0.9 | 0.9 | 0.9 | 0.8 | 0.9 | 0.9 | 0.9 | -0.2155 | 0.9221 | 0.0056 | 0.5318 | Medium |
| 3 | FH | 0.75 | 0.75 | 0.75 | 0.75 | 0.75 | 0.75 | 1.1 | 0.75 | -0.1632 | 0.4586 | -0.0168 | 0.5394 | Medium |
| 4 | FH | 0.87 | 0.87 | 0.87 | 0.87 | 0.87 | 0.87 | 0.87 | 1.23 | -0.0872 | 0.7329 | 0.0464 | 0.4947 | Medium |
| 5 | FH | 0.9 | 0.9 | 0.9 | 0.9 | 0.9 | 0.6 | 0.9 | 0.9 | -0.3773 | 1.2431 | 0.0208 | 0.3899 | Medium |
| 6 | FH | 0.9 | 0.9 | 0.9 | 0.9 | 0.9 | 1.1 | 0.9 | 0.9 | -0.1330 | 0.6830 | 0.0013 | 0.3433 | Medium |
| 7 | FH | 0.87 | 0.87 | 0.87 | 0.87 | 0.87 | 0.87 | 0.87 | 1.2 | -0.2439 | 0.7760 | 0.0533 | 0.0722 | Medium |
| 8 | FH | 0.8 | 0.8 | 1.1 | 0.8 | 0.8 | 0.8 | 0.8 | 0.8 | -0.1013 | 0.5102 | 0.0424 | 0.5101 | Medium |
| 9 | FH | 0.95 | 0.95 | 0.95 | 0.8 | 0.95 | 0.95 | 0.95 | 0.95 | -0.1778 | 1.2526 | -0.0383 | 0.5415 | Medium |
| 10 | FH | 0.9 | 0.9 | 0.9 | 0.9 | 0.9 | 0.8 | 0.9 | 0.9 | -0.1086 | 0.9854 | 0.0585 | 0.5157 | Medium |
| 11 | FH | 0.75 | 0.75 | 0.75 | 0.75 | 0.8 | 0.75 | 0.75 | 0.75 | -0.3085 | 0.3680 | 0.0325 | 0.5038 | Medium |
| 12 | FH | 0.9 | 0.9 | 0.9 | 0.9 | 1.1 | 0.9 | 0.9 | 0.9 | -0.2369 | 0.9637 | 0.0904 | 0.3320 | Medium |
| 13 | FH | 0.9 | 0.9 | 0.9 | 0.8 | 0.9 | 0.9 | 0.9 | 0.9 | -0.1976 | 1.3006 | 0.0735 | 0.5487 | Medium |
| 14 | FH | 0.8 | 0.8 | 1.1 | 0.8 | 0.8 | 0.8 | 0.8 | 1.05 | -0.1948 | 0.9218 | -0.0248 | 0.5301 | Medium |
| 15 | FH | 0.8 | 0.8 | 1.1 | 0.8 | 0.8 | 0.8 | 0.8 | 1.05 | -0.2249 | 1.1705 | 0.0667 | 0.5296 | Medium |
| 16 | FH | 0.8 | 0.8 | 1.1 | 0.8 | 0.8 | 0.8 | 0.8 | 1.05 | -0.3200 | 1.2490 | 0.0716 | 0.3829 | Medium |
| 17 | FH | 0.8 | 0.8 | 1.1 | 0.8 | 0.8 | 0.8 | 0.8 | 1.05 | -0.3083 | 0.8977 | -0.0202 | 0.5673 | Medium |
| 18 | FH | 0.8 | 0.8 | 1.1 | 0.8 | 0.8 | 0.8 | 0.8 | 1.05 | -0.2808 | 1.0771 | 0.0277 | 0.5290 | Medium |
| 19 | FH | 0.8 | 0.8 | 1.1 | 0.8 | 0.8 | 0.8 | 0.8 | 1.05 | -0.2340 | 0.7977 | 0.0434 | 0.5226 | Medium |
| 20 | FH | 0.8 | 0.8 | 1.1 | 0.8 | 0.8 | 0.8 | 0.8 | 1.05 | -0.2539 | 1.1478 | 0.0459 | 0.5366 | Medium |
| 21 | FH | 0.8 | 0.8 | 1.1 | 0.8 | 0.8 | 0.8 | 0.8 | 1.05 | -0.3401 | 0.8968 | 0.0296 | 0.5224 | Medium |
| 22 | FH | 0.8 | 0.8 | 1.1 | 0.8 | 0.8 | 0.8 | 0.8 | 1.05 | -0.3218 | 1.1070 | -0.0111 | 0.5624 | Medium |
| 23 | BH | 0.9 | 0.9 | 0.9 | 1.08 | 0.9 | 0.9 | 0.9 | 0.9 | -0.0617 | 0.7514 | -0.0206 | 0.3841 | Medium |
| 24 | FH | 0.8 | 0.8 | 1.1 | 0.8 | 0.8 | 0.8 | 0.8 | 1.05 | -0.3652 | 1.0083 | 0.0244 | 0.4841 | Medium |
| 25 | FH | 0.9 | 0.9 | 0.9 | 0.9 | 0.9 | 1.1 | 1.1 | 1.25 | 0.0797 | 0.9861 | -0.0120 | 0.3946 | Medium |
| 26 | BH | 0.8 | 0.8 | 0.8 | 0.8 | 0.9 | 1.0 | 1.0 | 1.1 | -0.2737 | 0.7205 | -0.0163 | 0.3723 | Medium | 
| 27 | FH | 0.9 | 0.9 | 0.9 | 0.9 | 0.8 | 1.1 | 1.1 | 1.35 | 0.0200 | 1.1711 | -0.4000 | 1.4708 | Medium |

**Explanation:** 
The table summarizes the landing positions (x, y, z) of the ball, its peak height during the trajectory, and an estimated speed based on the total time it took for the ball to land.  The "x (landing)" column indicates how far the ball lands on the left or right side of the table.  Positive values mean the ball landed on the right side, and negative values indicate the left side.  The "y (landing)" column reveals the ball's distance from the net.  The "z (landing)" column shows the ball's height upon landing.  Peak height is the maximum height achieved by the ball during its trajectory. The values of a, b, c, d, e, f, g, h represent the parameters of the robot which generated the examples.  These parameters control various aspects of the robot's motion, including the swing direction and paddle velocity.

## Step 2: Parameters Closest to Objective

The parameters that are closest to fulfilling the objective of hitting the ball as far right as possible are: **Example 25** with parameters **a:0.9 b:0.9 c:0.9 d:0.9 e:0.9 f:1.1 g:1.1 h:1.25** and a **FH** stroke.

**Justification:** 
Example 25 results in a landing position of **x: 0.0797**, which is the furthest right landing position in the provided examples. 

## Step 3: Parameter Analysis

The provided parameters **a, b, c, d, e, f, g, h** influence the robot's motion and the ball's trajectory in different ways.

* **a, b, c, d:** These parameters define the orientation of the paddle during the impact with the ball.  The higher the value of these parameters, the more tilted the paddle is towards the intended direction of the ball.  Generally, increasing the values of a, b, c, d results in the ball traveling further to the right.

* **e:** This parameter determines the paddle's velocity during impact.  A higher value of "e" means the paddle strikes the ball with greater velocity, resulting in a faster ball trajectory and a greater distance covered.

* **f, g:** These parameters influence the swing direction of the paddle. A higher value of "f" corresponds to a more open swing, potentially resulting in a more horizontal ball trajectory. A higher value of "g" corresponds to a swing that is more closed to the body, potentially resulting in a more vertical ball trajectory. 

* **h:** This parameter controls the swing speed.  A higher value of "h" indicates a faster swing, which can lead to increased ball speed and a greater impact on the ball's trajectory.

**Analysis based on the examples:**
* Examples 14, 15, 16, 17, 18, 19, 20, 21, 22, 24 all have a similar "g" and "h" value and also share a similar "c" value. The results of these examples reveal that  increasing the value of "c" seems to shift the ball trajectory towards the right.
* The examples with "h" values in the range [1.25, 1.35] (Example 25 and Example 27) demonstrate that increasing "h" does indeed influence the ball trajectory to some extent. 
* Example 23 demonstrates that by increasing the value of "d" the ball hits further to the right.

## Step 4: New Parameters

Proposed params: **a: 0.95 b: 0.95 c: 1.15 d: 1.08 e: 1.0 f: 1.1 g: 1.0 h: 1.3**
Best strokestyle: **FH** 

This set of parameters is based on the analysis of the previous examples. We are increasing the values of "c", "d", "e" and "h" based on the trend observed in the previous examples. This should result in a stronger, faster, and more precise hit, further enhancing the rightward trajectory. We are keeping the value of "g" at 1.0 which seemed to be a value that resulted in a good hit in many of the examples. The proposed parameters are chosen to be within the observed ranges that were successful in the previous examples. 

<q> Hit the ball as far right as possible
## Step 1: Summary Table

| Example | Stroke | a | b | c | d | e | f | g | h | x (landing) |  y (landing) |  z (landing) |  On Table | Peak Height (z) | Estimated Speed |
|---|---|---|---|---|---|---|---|---|---|---|---|---|---|---|
| 1 | FH | 0.75 | 0.75 | 0.75 | 0.75 | 1.1 | 0.75 | 0.75 | 0.75 | -0.2978 | 0.4482 | 0.0089 | True | 0.4059 | Medium |
| 2 | FH | 0.9 | 0.9 | 0.9 | 0.9 | 0.8 | 0.9 | 0.9 | 0.9 | -0.2155 | 0.9221 | 0.0056 | True | 0.4211 | Medium |
| 3 | FH | 0.75 | 0.75 | 0.75 | 0.75 | 0.75 | 0.75 | 1.1 | 0.75 | -0.1632 | 0.4586 | -0.0168 | True | 0.4246 | Medium |
| 4 | FH | 0.87 | 0.87 | 0.87 | 0.87 | 0.87 | 0.87 | 0.87 | 1.23 | -0.0872 | 0.7329 | 0.0464 | True | 0.4128 | Medium |
| 5 | FH | 0.9 | 0.9 | 0.9 | 0.9 | 0.9 | 0.6 | 0.9 | 0.9 | -0.3773 | 1.2431 | 0.0208 | True | 0.4167 | Medium |
| 6 | FH | 0.9 | 0.9 | 0.9 | 0.9 | 0.9 | 1.1 | 0.9 | 0.9 | -0.1330 | 0.6830 | 0.0013 | True | 0.4210 | Medium |
| 7 | FH | 0.87 | 0.87 | 0.87 | 0.87 | 0.87 | 0.87 | 0.87 | 1.2 | -0.2439 | 0.7760 | 0.0533 | True | 0.4076 | Medium |
| 8 | FH | 0.8 | 0.8 | 1.1 | 0.8 | 0.8 | 0.8 | 0.8 | 0.8 | -0.1013 | 0.5102 | 0.0424 | True | 0.4134 | Medium |
| 9 | FH | 0.95 | 0.95 | 0.95 | 0.8 | 0.95 | 0.95 | 0.95 | 0.95 | -0.1778 | 1.2526 | -0.0383 | True | 0.4177 | Medium |
| 10 | FH | 0.9 | 0.9 | 0.9 | 0.9 | 0.9 | 0.8 | 0.9 | 0.9 | -0.1086 | 0.9854 | 0.0585 | True | 0.4154 | Medium |
| 11 | FH | 0.75 | 0.75 | 0.75 | 0.75 | 0.8 | 0.75 | 0.75 | 0.75 | -0.3085 | 0.3680 | 0.0325 | True | 0.4118 | Medium |
| 12 | FH | 0.9 | 0.9 | 0.9 | 0.9 | 1.1 | 0.9 | 0.9 | 0.9 | -0.2369 | 0.9637 | 0.0904 | True | 0.4156 | Medium |
| 13 | FH | 0.9 | 0.9 | 0.9 | 0.8 | 0.9 | 0.9 | 0.9 | 0.9 | -0.1976 | 1.3006 | 0.0735 | True | 0.4179 | Medium |
| 14 | FH | 0.8 | 0.8 | 1.1 | 0.8 | 0.8 | 0.8 | 0.8 | 1.05 | -0.1948 | 0.9218 | -0.0248 | True | 0.4150 | Medium |
| 15 | FH | 0.8 | 0.8 | 1.1 | 0.8 | 0.8 | 0.8 | 0.8 | 1.05 | -0.2249 | 1.1705 | 0.0667 | True | 0.4130 | Medium |
| 16 | FH | 0.8 | 0.8 | 1.1 | 0.8 | 0.8 | 0.8 | 0.8 | 1.05 | -0.3200 | 1.2490 | 0.0716 | True | 0.4142 | Medium |
| 17 | FH | 0.8 | 0.8 | 1.1 | 0.8 | 0.8 | 0.8 | 0.8 | 1.05 | -0.3083 | 0.8977 | -0.0202 | True | 0.4148 | Medium |
| 18 | FH | 0.8 | 0.8 | 1.1 | 0.8 | 0.8 | 0.8 | 0.8 | 1.05 | -0.2808 | 1.0771 | 0.0277 | True | 0.4154 | Medium |
| 19 | FH | 0.8 | 0.8 | 1.1 | 0.8 | 0.8 | 0.8 | 0.8 | 1.05 | -0.2340 | 0.7977 | 0.0434 | True | 0.4130 | Medium |
| 20 | FH | 0.8 | 0.8 | 1.1 | 0.8 | 0.8 | 0.8 | 0.8 | 1.05 | -0.2539 | 1.1478 | 0.0459 | True | 0.4142 | Medium |
| 21 | FH | 0.8 | 0.8 | 1.1 | 0.8 | 0.8 | 0.8 | 0.8 | 1.05 | -0.3401 | 0.8968 | 0.0296 | True | 0.4153 | Medium |
| 22 | FH | 0.8 | 0.8 | 1.1 | 0.8 | 0.8 | 0.8 | 0.8 | 1.05 | -0.3218 | 1.1070 | -0.0111 | True | 0.4131 | Medium |
| 23 | BH | 0.9 | 0.9 | 0.9 | 1.08 | 0.9 | 0.9 | 0.9 | 0.9 | -0.0617 | 0.7514 | -0.0206 | True | 0.3800 | Medium |
| 24 | FH | 0.8 | 0.8 | 1.1 | 0.8 | 0.8 | 0.8 | 0.8 | 1.05 | -0.3652 | 1.0083 | 0.0244 | True | 0.4138 | Medium |
| 25 | FH | 0.9 | 0.9 | 0.9 | 0.9 | 0.9 | 1.1 | 1.1 | 1.25 | 0.0797 | 0.9861 | -0.0120 | True | 0.4248 | Medium |
| 26 | FH | 0.95 | 0.95 | 1.15 | 1.08 | 1.0 | 1.1 | 1.0 | 1.3 | 0.0457 | 0.8913 | -0.0472 | True | 0.4239 | Medium |
| 27 | FH | 0.9 | 0.9 | 0.9 | 0.9 | 0.8 | 1.1 | 1.1 | 1.35 | 0.0200 | 1.1711 | -0.4000 | True | 0.3939 | Medium |
| 28 | FH | 0.95 | 0.95 | 1.15 | 1.08 | 1.0 | 1.1 | 1.0 | 1.3 | -0.0170 | 1.5435 | -0.0223 | False | 0.4246 | Medium | 

 **Observations:**
 
 - **Landing Position:** The objective is to hit the ball as far right as possible.  Examples 25, 26, and 27  demonstrate the most positive x values (farthest to the right), with values of 0.0797, 0.0457, and 0.0200, respectively.
 - **On Table:** Example 28  is the only one to land outside the table. 
 - **Parameter Influence:** 
    - **c and g:** These parameters appear to heavily influence the landing position of the ball on the x-axis. Larger values of c and g seem to result in a ball landing further to the right.  
    - **h:**  Larger values of h generally result in the ball being hit further on the y-axis.  
    - **f:**  Higher values of 'f' push the ball slightly towards the net.

 ## Step 2:  Parameters Closest to Objective

The parameters from **Example 25** (a:0.9, b:0.9, c:0.9, d:0.9, e:0.9, f:1.1, g:1.1, h:1.25)  are closest to fulfilling the objective, landing the ball farthest to the right on the table. 

 ## Step 3: Parameter Analysis

* **a, b, d, e:** These parameters don't seem to have a significant effect on the landing position of the ball in the x-direction. While they might influence other aspects of the stroke, their primary impact is not on the x-axis.
* **c:**  A larger value of "c" leads to the ball landing further to the right on the table. This parameter seems to control the angle of the paddle during the hit, which directly affects the ball's horizontal trajectory.  
* **g:**  Similar to "c", a higher value of "g" results in a more positive x-landing position. This parameter likely controls the paddle's forward momentum during the hit, impacting the ball's horizontal velocity.
* **f:**  This parameter primarily influences the ball's depth (y-axis).  A larger value of "f" can push the ball towards the net, indicating a shorter stroke or less backswing.  
* **h:**  A higher "h" value can result in the ball being hit further on the y-axis, making the stroke more aggressive. This parameter likely controls the paddle's speed and force during the hit.

 ## Step 4: Proposed Parameters and Stroke

Proposed params: a:0.9 b:0.9 c:1.0  d:0.9 e:0.9 f:1.1 g:1.2 h:1.25 
Best strokestyle: FH 

<q> Hit the ball as far right as possible
## Step 1: Summary Table

| Example | Stroke | a | b | c | d | e | f | g | h | x (landing) |  y (landing) |  z (landing) | On Table | Peak Height (estimated) | Speed (estimated) |
|---|---|---|---|---|---|---|---|---|---|---|---|---|---|---|---|
| 1 | FH | 0.75 | 0.75 | 0.75 | 0.75 | 1.1 | 0.75 | 0.75 | 0.75 | -0.2978 | 0.4482 | 0.0089 | True | 0.3763 | 0.27 |
| 2 | FH | 0.9 | 0.9 | 0.9 | 0.9 | 0.8 | 0.9 | 0.9 | 0.9 | -0.2155 | 0.9221 | 0.0056 | True | 0.3952 | 0.31 |
| 3 | FH | 0.75 | 0.75 | 0.75 | 0.75 | 0.75 | 0.75 | 1.1 | 0.75 | -0.1632 | 0.4586 | -0.0168 | True | 0.3898 | 0.28 |
| 4 | FH | 0.87 | 0.87 | 0.87 | 0.87 | 0.87 | 0.87 | 0.87 | 1.23 | -0.0872 | 0.7329 | 0.0464 | True | 0.3898 | 0.28 |
| 5 | FH | 0.9 | 0.9 | 0.9 | 0.9 | 0.9 | 0.6 | 0.9 | 0.9 | -0.3773 | 1.2431 | 0.0208 | True | 0.3639 | 0.28 |
| 6 | FH | 0.9 | 0.9 | 0.9 | 0.9 | 0.9 | 1.1 | 0.9 | 0.9 | -0.1330 | 0.6830 | 0.0013 | True | 0.3363 | 0.26 |
| 7 | FH | 0.87 | 0.87 | 0.87 | 0.87 | 0.87 | 0.87 | 0.87 | 1.2 | -0.2439 | 0.7760 | 0.0533 | True | 0.2464 | 0.20 |
| 8 | FH | 0.8 | 0.8 | 1.1 | 0.8 | 0.8 | 0.8 | 0.8 | 0.8 | -0.1013 | 0.5102 | 0.0424 | True | 0.3609 | 0.27 |
| 9 | FH | 0.95 | 0.95 | 0.95 | 0.8 | 0.95 | 0.95 | 0.95 | 0.95 | -0.1778 | 1.2526 | -0.0383 | True | 0.3666 | 0.27 |
| 10 | FH | 0.9 | 0.9 | 0.9 | 0.9 | 0.9 | 0.8 | 0.9 | 0.9 | -0.1086 | 0.9854 | 0.0585 | True | 0.3734 | 0.27 |
| 11 | FH | 0.75 | 0.75 | 0.75 | 0.75 | 0.8 | 0.75 | 0.75 | 0.75 | -0.3085 | 0.3680 | 0.0325 | True | 0.3963 | 0.27 |
| 12 | FH | 0.9 | 0.9 | 0.9 | 0.9 | 1.1 | 0.9 | 0.9 | 0.9 | -0.2369 | 0.9637 | 0.0904 | True | 0.3278 | 0.26 |
| 13 | FH | 0.9 | 0.9 | 0.9 | 0.8 | 0.9 | 0.9 | 0.9 | 0.9 | -0.1976 | 1.3006 | 0.0735 | True | 0.4008 | 0.29 |
| 14 | FH | 0.8 | 0.8 | 1.1 | 0.8 | 0.8 | 0.8 | 0.8 | 1.05 | -0.1948 | 0.9218 | -0.0248 | True | 0.3903 | 0.28 |
| 15 | FH | 0.8 | 0.8 | 1.1 | 0.8 | 0.8 | 0.8 | 0.8 | 1.05 | -0.2249 | 1.1705 | 0.0667 | True | 0.3760 | 0.27 |
| 16 | FH | 0.8 | 0.8 | 1.1 | 0.8 | 0.8 | 0.8 | 0.8 | 1.05 | -0.3200 | 1.2490 | 0.0716 | True | 0.3427 | 0.26 |
| 17 | FH | 0.8 | 0.8 | 1.1 | 0.8 | 0.8 | 0.8 | 0.8 | 1.05 | -0.3083 | 0.8977 | -0.0202 | True | 0.4120 | 0.28 |
| 18 | FH | 0.8 | 0.8 | 1.1 | 0.8 | 0.8 | 0.8 | 0.8 | 1.05 | -0.2808 | 1.0771 | 0.0277 | True | 0.3800 | 0.27 |
| 19 | FH | 0.8 | 0.8 | 1.1 | 0.8 | 0.8 | 0.8 | 0.8 | 1.05 | -0.2340 | 0.7977 | 0.0434 | True | 0.3716 | 0.27 |
| 20 | FH | 0.8 | 0.8 | 1.1 | 0.8 | 0.8 | 0.8 | 0.8 | 1.05 | -0.2539 | 1.1478 | 0.0459 | True | 0.3833 | 0.27 |
| 21 | FH | 0.8 | 0.8 | 1.1 | 0.8 | 0.8 | 0.8 | 0.8 | 1.05 | -0.3401 | 0.8968 | 0.0296 | True | 0.3822 | 0.27 |
| 22 | FH | 0.8 | 0.8 | 1.1 | 0.8 | 0.8 | 0.8 | 0.8 | 1.05 | -0.3218 | 1.1070 | -0.0111 | True | 0.3755 | 0.27 |
| 23 | BH | 0.9 | 0.9 | 0.9 | 1.08 | 0.9 | 0.9 | 0.9 | 0.9 | -0.0617 | 0.7514 | -0.0206 | True | 0.3539 | 0.23 |
| 24 | FH | 0.8 | 0.8 | 1.1 | 0.8 | 0.8 | 0.8 | 0.8 | 1.05 | -0.3652 | 1.0083 | 0.0244 | True | 0.3628 | 0.26 |
| 25 | FH | 0.9 | 0.9 | 0.9 | 0.9 | 0.9 | 1.1 | 1.1 | 1.25 | 0.0797 | 0.9861 | -0.0120 | True | 0.3474 | 0.25 |
| 26 | FH | 0.9 | 0.9 | 0.9 | 0.9 | 0.9 | 1.1 | 1.1 | 1.25 | 0.0797 | 0.9861 | -0.0120 | True | 0.3474 | 0.25 |
| 27 | FH | 0.9 | 0.9 | 0.9 | 0.9 | 0.8 | 1.1 | 1.1 | 1.35 | 0.0200 | 1.1711 | -0.4000 | True | 1.4708 | 0.26 |
| 28 | FH | 0.95 | 0.95 | 1.15 | 1.08 | 1.0 | 1.1 | 1.0 | 1.3 | -0.0170 | 1.5435 | -0.0223 | False | 0.5294 | 0.26 |
| 29 | FH | 0.9 | 0.9 | 1.0 | 0.9 | 0.9 | 1.1 | 1.2 | 1.25 | 0.1132 | 1.4299 | -0.0298 | False | 0.4761 | 0.27 |

**Analysis of Landing Positions:**

The objective is to hit the ball as far right as possible.  Analyzing the x (landing) values in the table, we observe:

* **Examples 1-13:**  These examples are all forehand strokes. The x (landing) values are all negative, indicating the ball lands to the left of the table center. The further away from zero, the further left the ball landed.
* **Examples 14-24:**  These are also forehand strokes, with x (landing) values generally between -0.10 and -0.36,  again indicating the ball lands left of center.  There is some variation, with some landing slightly further right than others.
* **Examples 25-29:** These examples show a different pattern. The x (landing) values are all positive, indicating the ball landed to the right of the table center. This is promising for our objective. 

**Peak Height and Speed:**

* **Generally**, the examples with higher parameter values for 'g' (paddle angle) tend to have higher peak heights.
* **Examples 25-29:** The speed of these strokes seems to be somewhat slower than the previous examples.

**Important Note:**

* **Examples 28 and 29:** These examples showcase a strong rightward bias. However, the ball lands off the table, making them unsuitable for our objective.

## Step 2:  Parameters Closest to Objective

Based on the table, **Examples 25, 26, and 27** come closest to fulfilling the objective, as they all landed on the right side of the table. However, they all land slightly too far forward. 

**Parameters of Examples 25 and 26:**

* a: 0.9
* b: 0.9
* c: 0.9
* d: 0.9
* e: 0.9
* f: 1.1
* g: 1.1
* h: 1.25

**Parameters of Example 27:**

* a: 0.9
* b: 0.9
* c: 0.9
* d: 0.9
* e: 0.8
* f: 1.1
* g: 1.1
* h: 1.35

## Step 3: Parameter Analysis 

**Parameter 'g' (Paddle Angle):**

* A higher 'g' value (like in Examples 25-29) results in a higher ball trajectory, sending the ball further towards the opponent's side (positive y values).

**Parameter 'h' (Paddle Speed):**

* A higher 'h' value (like in Examples 25-29) seems to result in a slightly slower ball speed. This could be due to the robot's mechanics.

**Other Parameters (a, b, c, d, e, f):**

* These parameters seem to have less of a direct impact on the landing position. However, they likely play a role in the trajectory and speed, indirectly affecting the outcome.

## Step 4: Proposed Parameters

**Proposed params:** a:0.9 b:0.9 c:0.9 d:0.9 e:0.8 f:1.1 g:1.1 h:1.25
**Best strokestyle:** FH 

<q> Hit the ball as far right as possible
## Step 1: Summary Table

| Example | Stroke | a | b | c | d | e | f | g | h | x (landing) |  y (landing) |  z (landing) | On Table | Peak Height (estimated) | Speed (estimated) |
|---|---|---|---|---|---|---|---|---|---|---|---|---|---|---|---|
| 1 | FH | 0.75 | 0.75 | 0.75 | 0.75 | 1.1 | 0.75 | 0.75 | 0.75 | -0.2978 | 0.4482 | 0.0089 | True | 0.37 | Medium |
| 2 | FH | 0.9 | 0.9 | 0.9 | 0.9 | 0.8 | 0.9 | 0.9 | 0.9 | -0.2155 | 0.9221 | 0.0056 | True | 0.36 | Medium |
| 3 | FH | 0.75 | 0.75 | 0.75 | 0.75 | 0.75 | 0.75 | 1.1 | 0.75 | -0.1632 | 0.4586 | -0.0168 | True | 0.35 | Medium |
| 4 | FH | 0.87 | 0.87 | 0.87 | 0.87 | 0.87 | 0.87 | 0.87 | 1.23 | -0.0872 | 0.7329 | 0.0464 | True | 0.35 | Medium |
| 5 | FH | 0.9 | 0.9 | 0.9 | 0.9 | 0.9 | 0.6 | 0.9 | 0.9 | -0.3773 | 1.2431 | 0.0208 | True | 0.35 | Medium |
| 6 | FH | 0.9 | 0.9 | 0.9 | 0.9 | 0.9 | 1.1 | 0.9 | 0.9 | -0.1330 | 0.6830 | 0.0013 | True | 0.35 | Medium |
| 7 | FH | 0.87 | 0.87 | 0.87 | 0.87 | 0.87 | 0.87 | 0.87 | 1.2 | -0.2439 | 0.7760 | 0.0533 | True | 0.34 | Medium |
| 8 | FH | 0.8 | 0.8 | 1.1 | 0.8 | 0.8 | 0.8 | 0.8 | 0.8 | -0.1013 | 0.5102 | 0.0424 | True | 0.33 | Medium |
| 9 | FH | 0.95 | 0.95 | 0.95 | 0.8 | 0.95 | 0.95 | 0.95 | 0.95 | -0.1778 | 1.2526 | -0.0383 | True | 0.33 | Medium |
| 10 | FH | 0.9 | 0.9 | 0.9 | 0.9 | 0.9 | 0.8 | 0.9 | 0.9 | -0.1086 | 0.9854 | 0.0585 | True | 0.33 | Medium |
| 11 | FH | 0.75 | 0.75 | 0.75 | 0.75 | 0.8 | 0.75 | 0.75 | 0.75 | -0.3085 | 0.3680 | 0.0325 | True | 0.33 | Medium |
| 12 | FH | 0.9 | 0.9 | 0.9 | 0.9 | 1.1 | 0.9 | 0.9 | 0.9 | -0.2369 | 0.9637 | 0.0904 | True | 0.33 | Medium |
| 13 | FH | 0.9 | 0.9 | 0.9 | 0.8 | 0.9 | 0.9 | 0.9 | 0.9 | -0.1976 | 1.3006 | 0.0735 | True | 0.32 | Medium |
| 14 | FH | 0.8 | 0.8 | 1.1 | 0.8 | 0.8 | 0.8 | 0.8 | 1.05 | -0.1948 | 0.9218 | -0.0248 | True | 0.32 | Medium |
| 15 | FH | 0.8 | 0.8 | 1.1 | 0.8 | 0.8 | 0.8 | 0.8 | 1.05 | -0.2249 | 1.1705 | 0.0667 | True | 0.32 | Medium |
| 16 | FH | 0.8 | 0.8 | 1.1 | 0.8 | 0.8 | 0.8 | 0.8 | 1.05 | -0.3200 | 1.2490 | 0.0716 | True | 0.31 | Medium |
| 17 | FH | 0.8 | 0.8 | 1.1 | 0.8 | 0.8 | 0.8 | 0.8 | 1.05 | -0.3083 | 0.8977 | -0.0202 | True | 0.31 | Medium |
| 18 | FH | 0.8 | 0.8 | 1.1 | 0.8 | 0.8 | 0.8 | 0.8 | 1.05 | -0.2808 | 1.0771 | 0.0277 | True | 0.31 | Medium |
| 19 | FH | 0.8 | 0.8 | 1.1 | 0.8 | 0.8 | 0.8 | 0.8 | 1.05 | -0.2340 | 0.7977 | 0.0434 | True | 0.30 | Medium |
| 20 | FH | 0.8 | 0.8 | 1.1 | 0.8 | 0.8 | 0.8 | 0.8 | 1.05 | -0.2539 | 1.1478 | 0.0459 | True | 0.30 | Medium |
| 21 | FH | 0.8 | 0.8 | 1.1 | 0.8 | 0.8 | 0.8 | 0.8 | 1.05 | -0.3401 | 0.8968 | 0.0296 | True | 0.29 | Medium |
| 22 | FH | 0.8 | 0.8 | 1.1 | 0.8 | 0.8 | 0.8 | 0.8 | 1.05 | -0.3218 | 1.1070 | -0.0111 | True | 0.29 | Medium |
| 23 | BH | 0.9 | 0.9 | 0.9 | 1.08 | 0.9 | 0.9 | 0.9 | 0.9 | -0.0617 | 0.7514 | -0.0206 | True | 0.27 | Medium |
| 24 | FH | 0.8 | 0.8 | 1.1 | 0.8 | 0.8 | 0.8 | 0.8 | 1.05 | -0.3652 | 1.0083 | 0.0244 | True | 0.27 | Medium |
| 25 | FH | 0.9 | 0.9 | 0.9 | 0.9 | 0.9 | 1.1 | 1.1 | 1.25 | 0.0797 | 0.9861 | -0.0120 | True | 0.26 | Medium |
| 26 | FH | 0.9 | 0.9 | 0.9 | 0.9 | 1.0 | 1.1 | 1.1 | 1.25 | 0.0357 | 0.8687 | -0.0272 | True | 0.26 | Medium |
| 27 | FH | 0.9 | 0.9 | 0.9 | 0.9 | 0.8 | 1.1 | 1.1 | 1.35 | 0.0200 | 1.1711 | -0.4000 | True | 0.25 | Medium |
| 28 | FH | 0.95 | 0.95 | 1.15 | 1.08 | 1.0 | 1.1 | 1.0 | 1.3 | -0.0170 | 1.5435 | -0.0223 | False | 0.24 | Medium |
| 29 | FH | 0.9 | 0.9 | 1.0 | 0.9 | 0.9 | 1.1 | 1.2 | 1.25 | 0.1132 | 1.4299 | -0.0298 | False | 0.23 | Medium |

**Analysis:**

* **Parameter 'g' and 'h':** Increasing these parameters generally pushes the ball further in the y direction (towards the opponent's side).  However, an extremely high 'h' value can also lead to the ball landing off the table, as seen in examples 28 and 29.
* **Parameter 'f':** Increasing this parameter seems to slightly influence the landing position in the x direction, but this influence is minimal compared to the other parameters.
* **Parameter 'a':** This parameter seems to primarily affect the ball's initial trajectory. It's difficult to determine a clear relationship to the landing position, though it might influence the spin applied.
* **Parameter 'b', 'c', 'd', 'e':** These parameters seem to influence the overall speed and trajectory of the ball, with a more noticeable impact in the y direction.  The exact impact of each parameter is difficult to isolate. 

## Step 2: Closest Parameters to Objective

Based on the table, example **25** with **a:0.9, b:0.9, c:0.9, d:0.9, e:0.9, f:1.1, g:1.1, h:1.25** and a **FH stroke** comes closest to hitting the ball as far right as possible while still landing on the table. The ball landed at x:0.0797, which is a positive x value, indicating a rightward hit.

## Step 3: Analysis of Parameter Effects

Based on the previous analysis and the provided examples, here's a more detailed look at the parameter effects:

* **'g' and 'h':** These parameters are the most influential for hitting the ball further towards the opponent's side (positive y). Increasing these parameters results in a longer trajectory and, therefore, a further landing position.
* **'f':** This parameter seems to have a smaller impact on the landing position, primarily influencing the ball's initial trajectory and possibly spin.
* **'a':** This parameter primarily affects the initial trajectory and might influence the spin applied.
* **'b', 'c', 'd', 'e':** These parameters influence the ball's overall speed and trajectory, with a more noticeable impact in the y direction.  The exact impact of each parameter is difficult to isolate.

## Step 4: Proposed Parameters 

Proposed params: **a:0.9 b:0.9 c:0.9 d:0.9 e:0.9 f:1.1 g:1.2 h:1.2**
Best strokestyle: **FH** 

<q> Hit the ball as far right as possible
## Step 1: Summary Table

| Example | Stroke | a | b | c | d | e | f | g | h | x (landing) | y (landing) | z (peak) | Estimated Speed |
|---|---|---|---|---|---|---|---|---|---|---|---|---|---|
| 1 | FH | 0.75 | 0.75 | 0.75 | 0.75 | 1.1 | 0.75 | 0.75 | 0.75 | -0.2978 | 0.4482 | 0.3763 | Moderate |
| 2 | FH | 0.9 | 0.9 | 0.9 | 0.9 | 0.8 | 0.9 | 0.9 | 0.9 | -0.2155 | 0.9221 | 0.3952 | Moderate |
| 3 | FH | 0.75 | 0.75 | 0.75 | 0.75 | 0.75 | 0.75 | 1.1 | 0.75 | -0.1632 | 0.4586 | 0.3898 | Moderate |
| 4 | FH | 0.87 | 0.87 | 0.87 | 0.87 | 0.87 | 0.87 | 0.87 | 1.23 | -0.0872 | 0.7329 | 0.3898 | Moderate |
| 5 | FH | 0.9 | 0.9 | 0.9 | 0.9 | 0.9 | 0.6 | 0.9 | 0.9 | -0.3773 | 1.2431 | 0.3639 | Moderate |
| 6 | FH | 0.9 | 0.9 | 0.9 | 0.9 | 0.9 | 1.1 | 0.9 | 0.9 | -0.1330 | 0.6830 | 0.3363 | Moderate |
| 7 | FH | 0.87 | 0.87 | 0.87 | 0.87 | 0.87 | 0.87 | 0.87 | 1.2 | -0.2439 | 0.7760 | 0.2464 | Moderate |
| 8 | FH | 0.8 | 0.8 | 1.1 | 0.8 | 0.8 | 0.8 | 0.8 | 0.8 | -0.1013 | 0.5102 | 0.3609 | Moderate |
| 9 | FH | 0.95 | 0.95 | 0.95 | 0.8 | 0.95 | 0.95 | 0.95 | 0.95 | -0.1778 | 1.2526 | 0.3666 | Moderate |
| 10 | FH | 0.9 | 0.9 | 0.9 | 0.9 | 0.9 | 0.8 | 0.9 | 0.9 | -0.1086 | 0.9854 | 0.3734 | Moderate |
| 11 | FH | 0.75 | 0.75 | 0.75 | 0.75 | 0.8 | 0.75 | 0.75 | 0.75 | -0.3085 | 0.3680 | 0.3963 | Moderate |
| 12 | FH | 0.9 | 0.9 | 0.9 | 0.9 | 1.1 | 0.9 | 0.9 | 0.9 | -0.2369 | 0.9637 | 0.3278 | Moderate |
| 13 | FH | 0.9 | 0.9 | 0.9 | 0.8 | 0.9 | 0.9 | 0.9 | 0.9 | -0.1976 | 1.3006 | 0.4008 | Moderate |
| 14 | FH | 0.8 | 0.8 | 1.1 | 0.8 | 0.8 | 0.8 | 0.8 | 1.05 | -0.1948 | 0.9218 | 0.3903 | Moderate |
| 15 | FH | 0.8 | 0.8 | 1.1 | 0.8 | 0.8 | 0.8 | 0.8 | 1.05 | -0.2249 | 1.1705 | 0.3760 | Moderate |
| 16 | FH | 0.8 | 0.8 | 1.1 | 0.8 | 0.8 | 0.8 | 0.8 | 1.05 | -0.3200 | 1.2490 | 0.3427 | Moderate |
| 17 | FH | 0.8 | 0.8 | 1.1 | 0.8 | 0.8 | 0.8 | 0.8 | 1.05 | -0.3083 | 0.8977 | 0.4120 | Moderate |
| 18 | FH | 0.8 | 0.8 | 1.1 | 0.8 | 0.8 | 0.8 | 0.8 | 1.05 | -0.2808 | 1.0771 | 0.3800 | Moderate |
| 19 | FH | 0.8 | 0.8 | 1.1 | 0.8 | 0.8 | 0.8 | 0.8 | 1.05 | -0.2340 | 0.7977 | 0.3716 | Moderate |
| 20 | FH | 0.8 | 0.8 | 1.1 | 0.8 | 0.8 | 0.8 | 0.8 | 1.05 | -0.2539 | 1.1478 | 0.3833 | Moderate |
| 21 | FH | 0.8 | 0.8 | 1.1 | 0.8 | 0.8 | 0.8 | 0.8 | 1.05 | -0.3401 | 0.8968 | 0.3822 | Moderate |
| 22 | FH | 0.8 | 0.8 | 1.1 | 0.8 | 0.8 | 0.8 | 0.8 | 1.05 | -0.3218 | 1.1070 | 0.3755 | Moderate |
| 23 | FH | 0.9 | 0.9 | 0.9 | 1.08 | 0.9 | 0.9 | 0.9 | 0.9 | -0.0617 | 0.7514 | 0.3539 | Moderate |
| 24 | FH | 0.8 | 0.8 | 1.1 | 0.8 | 0.8 | 0.8 | 0.8 | 1.05 | -0.3652 | 1.0083 | 0.3628 | Moderate |
| 25 | BH | 0.9 | 0.9 | 0.9 | 0.9 | 0.9 | 1.1 | 1.1 | 1.25 | 0.0797 | 0.9861 | 0.3474 | Moderate |
| 26 | BH | 0.8 | 0.8 | 0.8 | 0.8 | 1.0 | 1.1 | 1.0 | 1.3 | -0.2800 | 0.9900 | 0.3745 | Moderate |
| 27 | BH | 0.9 | 0.9 | 0.9 | 0.9 | 0.8 | 1.1 | 1.1 | 1.35 | 0.0200 | 1.1711 | 1.4708 | Fast |
| 28 | BH | 0.95 | 0.95 | 1.15 | 1.08 | 1.0 | 1.1 | 1.0 | 1.3 | -0.0170 | 1.5435 | 0.3548 | Moderate |
| 29 | BH | 0.9 | 0.9 | 1.0 | 0.9 | 0.9 | 1.1 | 1.2 | 1.25 | 0.1132 | 1.4299 | 0.3727 | Moderate |
| 30 | BH | 0.9 | 0.9 | 0.9 | 0.9 | 0.9 | 1.1 | 1.2 | 1.2 | 0.2176 | 1.2533 | 0.3985 | Moderate |

**Explanation:**

The table summarizes the landing position of the ball for each example.  

* **x (landing):** This represents the lateral position of the ball landing on the table, with positive values indicating a right-side landing and negative values indicating a left-side landing. 
* **y (landing):** This represents the depth of the ball landing on the table, with positive values indicating a successful return to the opponent's side and negative values indicating the ball landing on our side.
* **z (peak):** This represents the peak height reached by the ball during its trajectory.
* **Estimated Speed:** This is a subjective assessment of the ball's speed based on its trajectory and landing position.  

**Evidence:**

The landing position information is directly from the provided data. The peak height is calculated by finding the maximum value of 'ball z' in the ball motion data. The estimated speed is based on the observed trajectory. A ball with a high peak height and a long trajectory is considered fast.

## Step 2: Parameters with Best Rightward Landing

Based on the table above, the example with the best rightward landing position is **Example 25**, with a landing position of **x = 0.0797**.  This example corresponds to the following parameters:

* a: 0.9
* b: 0.9
* c: 0.9
* d: 0.9
* e: 0.9
* f: 1.1
* g: 1.1
* h: 1.25

**Stroke style:** **BH (backhand)**

## Step 3: Analysis of Parameter Effects

Analyzing the table above, we can observe the following trends:

* **Parameter 'a':**  Doesn't appear to have a significant impact on the landing position on the x-axis. 
* **Parameter 'b':**  Doesn't appear to have a significant impact on the landing position on the x-axis. 
* **Parameter 'c':**  Seems to increase the rightward landing position (positive x) when increased. However, it also affects the peak height and might lead to balls landing off the table. 
* **Parameter 'd':**  Doesn't appear to have a significant impact on the landing position on the x-axis. 
* **Parameter 'e':**  Doesn't appear to have a significant impact on the landing position on the x-axis. 
* **Parameter 'f':**  Doesn't appear to have a significant impact on the landing position on the x-axis. 
* **Parameter 'g':**  Seems to increase the rightward landing position (positive x) when increased. However, it also affects the peak height and might lead to balls landing off the table.
* **Parameter 'h':**  Seems to significantly influence the rightward landing position (positive x) when increased. Increasing this parameter often results in higher peak heights as well. 

**Conclusion:**

Parameters 'c' and 'g' have a positive influence on the rightward landing position but also affect the peak height. Parameter 'h' has the most significant impact on the rightward landing position but also affects the peak height. 

## Step 4: Proposed Parameters

Proposed params: **a:0.9 b:0.9 c:0.9 d:0.9 e:0.9 f:1.1 g:1.2 h:1.35**
Best strokestyle: **BH** 

<q> Hit the ball as far right as possible
## Step 1: Summary Table

| Example | Stroke | a | b | c | d | e | f | g | h | x (landing) | y (landing) | z (peak) | Estimated Speed |
|---|---|---|---|---|---|---|---|---|---|---|---|---|---|
| 1 | FH | 0.75 | 0.75 | 0.75 | 0.75 | 1.1 | 0.75 | 0.75 | 0.75 | -0.2978 | 0.4482 | 0.3763 | Moderate |
| 2 | FH | 0.9 | 0.9 | 0.9 | 0.9 | 0.8 | 0.9 | 0.9 | 0.9 | -0.2155 | 0.9221 | 0.3952 | Moderate |
| 3 | FH | 0.75 | 0.75 | 0.75 | 0.75 | 0.75 | 0.75 | 1.1 | 0.75 | -0.1632 | 0.4586 | 0.3898 | Moderate |
| 4 | FH | 0.87 | 0.87 | 0.87 | 0.87 | 0.87 | 0.87 | 0.87 | 1.23 | -0.0872 | 0.7329 | 0.3898 | Moderate |
| 5 | FH | 0.9 | 0.9 | 0.9 | 0.9 | 0.9 | 0.6 | 0.9 | 0.9 | -0.3773 | 1.2431 | 0.3639 | Moderate |
| 6 | FH | 0.9 | 0.9 | 0.9 | 0.9 | 0.9 | 1.1 | 0.9 | 0.9 | -0.1330 | 0.6830 | 0.3363 | Moderate |
| 7 | FH | 0.87 | 0.87 | 0.87 | 0.87 | 0.87 | 0.87 | 0.87 | 1.2 | -0.2439 | 0.7760 | 0.2464 | Moderate |
| 8 | FH | 0.8 | 0.8 | 1.1 | 0.8 | 0.8 | 0.8 | 0.8 | 0.8 | -0.1013 | 0.5102 | 0.3609 | Moderate |
| 9 | FH | 0.95 | 0.95 | 0.95 | 0.8 | 0.95 | 0.95 | 0.95 | 0.95 | -0.1778 | 1.2526 | 0.3666 | Moderate |
| 10 | FH | 0.9 | 0.9 | 0.9 | 0.9 | 0.9 | 0.8 | 0.9 | 0.9 | -0.1086 | 0.9854 | 0.3734 | Moderate |
| 11 | FH | 0.75 | 0.75 | 0.75 | 0.75 | 0.8 | 0.75 | 0.75 | 0.75 | -0.3085 | 0.3680 | 0.3963 | Moderate |
| 12 | FH | 0.9 | 0.9 | 0.9 | 0.9 | 1.1 | 0.9 | 0.9 | 0.9 | -0.2369 | 0.9637 | 0.3278 | Moderate |
| 13 | FH | 0.9 | 0.9 | 0.9 | 0.8 | 0.9 | 0.9 | 0.9 | 0.9 | -0.1976 | 1.3006 | 0.4008 | Moderate |
| 14 | FH | 0.8 | 0.8 | 1.1 | 0.8 | 0.8 | 0.8 | 0.8 | 1.05 | -0.1948 | 0.9218 | 0.3903 | Moderate |
| 15 | FH | 0.8 | 0.8 | 1.1 | 0.8 | 0.8 | 0.8 | 0.8 | 1.05 | -0.2249 | 1.1705 | 0.3760 | Moderate |
| 16 | FH | 0.8 | 0.8 | 1.1 | 0.8 | 0.8 | 0.8 | 0.8 | 1.05 | -0.3200 | 1.2490 | 0.3427 | Moderate |
| 17 | FH | 0.8 | 0.8 | 1.1 | 0.8 | 0.8 | 0.8 | 0.8 | 1.05 | -0.3083 | 0.8977 | 0.4120 | Moderate |
| 18 | FH | 0.8 | 0.8 | 1.1 | 0.8 | 0.8 | 0.8 | 0.8 | 1.05 | -0.2808 | 1.0771 | 0.3800 | Moderate |
| 19 | FH | 0.8 | 0.8 | 1.1 | 0.8 | 0.8 | 0.8 | 0.8 | 1.05 | -0.2340 | 0.7977 | 0.3716 | Moderate |
| 20 | FH | 0.8 | 0.8 | 1.1 | 0.8 | 0.8 | 0.8 | 0.8 | 1.05 | -0.2539 | 1.1478 | 0.3833 | Moderate |
| 21 | FH | 0.8 | 0.8 | 1.1 | 0.8 | 0.8 | 0.8 | 0.8 | 1.05 | -0.3401 | 0.8968 | 0.3822 | Moderate |
| 22 | FH | 0.8 | 0.8 | 1.1 | 0.8 | 0.8 | 0.8 | 0.8 | 1.05 | -0.3218 | 1.1070 | 0.3755 | Moderate |
| 23 | FH | 0.9 | 0.9 | 0.9 | 1.08 | 0.9 | 0.9 | 0.9 | 0.9 | -0.0617 | 0.7514 | 0.3539 | Moderate |
| 24 | FH | 0.8 | 0.8 | 1.1 | 0.8 | 0.8 | 0.8 | 0.8 | 1.05 | -0.3652 | 1.0083 | 0.3628 | Moderate |
| 25 | FH | 0.9 | 0.9 | 0.9 | 0.9 | 0.9 | 1.1 | 1.1 | 1.25 | 0.0797 | 0.9861 | 0.3474 | Moderate |
| 26 | FH | 0.8 | 0.8 | 1.0 | 0.8 | 0.9 | 1.0 | 1.1 | 1.2 | -0.2757 | 1.0145 | 0.3367 | Moderate |
| 27 | FH | 0.9 | 0.9 | 0.9 | 0.9 | 0.8 | 1.1 | 1.1 | 1.35 | 0.0200 | 1.1711 | 1.4708 | High |
| 28 | FH | 0.95 | 0.95 | 1.15 | 1.08 | 1.0 | 1.1 | 1.0 | 1.3 | -0.0170 | 1.5435 | 0.3548 | Moderate |
| 29 | FH | 0.9 | 0.9 | 1.0 | 0.9 | 0.9 | 1.1 | 1.2 | 1.25 | 0.1132 | 1.4299 | 0.3727 | Moderate |
| 30 | FH | 0.9 | 0.9 | 0.9 | 0.9 | 0.9 | 1.1 | 1.2 | 1.2 | 0.2176 | 1.2533 | 0.3985 | Moderate |
| 31 | FH | 0.9 | 0.9 | 0.9 | 0.9 | 0.9 | 1.1 | 1.2 | 1.35 | 0.4302 | 1.2174 | 0.3668 | Moderate |

**Analysis:**

* **x (landing):**  The landing position along the width of the table is heavily influenced by the parameters **g** and **h**. Higher values for **g** and **h** generally result in the ball landing further to the right. 
* **y (landing):**  The landing position along the depth of the table is affected by the parameters **a**, **b**, **c**, and **d**. Higher values for these parameters tend to push the ball deeper into the opponent's side. Parameter **e** also plays a role, with higher values generally leading to a longer return.
* **z (peak):**  The peak height of the ball is primarily influenced by the parameters **g**, **h**, and **e**.  Higher values for **g** and **h** usually produce a higher ball arc, and parameter **e** controls the duration of the contact, contributing to the peak height. 
* **Estimated Speed:** While the table doesn't provide precise speed values, we can infer that higher values of **g**, **h**, and **e** generally lead to a faster ball speed.

**Notes:**

* This is based on a limited number of examples, so further analysis with more data might be needed.
*  The influence of each parameter can interact with others, meaning a change in one parameter may significantly alter the effect of another.

## Step 2: Parameters Closest to Objective

The parameters closest to fulfilling the objective of hitting the ball as far right as possible are:

* **Example 27:** a:0.9, b:0.9, c:0.9, d:0.9, e:0.8, f:1.1, g:1.1, h:1.35  (x = 0.02)
* **Example 29:** a:0.9, b:0.9, c:1.0, d:0.9, e:0.9, f:1.1, g:1.2, h:1.25 (x = 0.1132)
* **Example 31:** a:0.9, b:0.9, c:0.9, d:0.9, e:0.9, f:1.1, g:1.2, h:1.35 (x = 0.4302) 

These examples have the highest positive x (landing) values, indicating a more rightward landing position.

## Step 3: Analysis of Parameters

Based on the summary table and examples, we can observe the following trends:

* **Parameter g:**  Increasing **g** significantly shifts the landing position to the right.
* **Parameter h:** Increasing **h** also shifts the landing position to the right, but the effect is less pronounced than **g**.
* **Parameter e:** Increasing **e** seems to increase the duration of contact, resulting in higher ball trajectory and potentially influencing the speed and landing position.
* **Parameters a, b, c, d:**  These parameters primarily influence the depth of the return and have a lesser impact on the lateral position.

## Step 4: Proposed Parameters

Proposed params: a:0.9 b:0.9 c:0.9 d:0.9 e:0.9 f:1.1 g:1.3 h:1.4 
Best strokestyle: FH 

<q> Hit the ball as far right as possible
## Step 1: Summary Table

| Example | Stroke | a | b | c | d | e | f | g | h | x (landing) |  y (landing) |  z (landing) |  On Table | Peak Height (z) | Estimated Speed |
|---|---|---|---|---|---|---|---|---|---|---|---|---|---|---|
| 1 | FH | 0.75 | 0.75 | 0.75 | 0.75 | 1.1 | 0.75 | 0.75 | 0.75 | -0.2978 | 0.4482 | 0.0089 | True | 0.4059 | Medium |
| 2 | FH | 0.9 | 0.9 | 0.9 | 0.9 | 0.8 | 0.9 | 0.9 | 0.9 | -0.2155 | 0.9221 | 0.0056 | True | 0.4211 | Medium |
| 3 | FH | 0.75 | 0.75 | 0.75 | 0.75 | 0.75 | 0.75 | 1.1 | 0.75 | -0.1632 | 0.4586 | -0.0168 | True | 0.4246 | Medium |
| 4 | FH | 0.87 | 0.87 | 0.87 | 0.87 | 0.87 | 0.87 | 0.87 | 1.23 | -0.0872 | 0.7329 | 0.0464 | True | 0.4131 | Medium |
| 5 | FH | 0.9 | 0.9 | 0.9 | 0.9 | 0.9 | 0.6 | 0.9 | 0.9 | -0.3773 | 1.2431 | 0.0208 | True | 0.4167 | Medium |
| 6 | FH | 0.9 | 0.9 | 0.9 | 0.9 | 0.9 | 1.1 | 0.9 | 0.9 | -0.1330 | 0.6830 | 0.0013 | True | 0.4210 | Medium |
| 7 | FH | 0.87 | 0.87 | 0.87 | 0.87 | 0.87 | 0.87 | 0.87 | 1.2 | -0.2439 | 0.7760 | 0.0533 | True | 0.4076 | Medium |
| 8 | FH | 0.8 | 0.8 | 1.1 | 0.8 | 0.8 | 0.8 | 0.8 | 0.8 | -0.1013 | 0.5102 | 0.0424 | True | 0.4134 | Medium |
| 9 | FH | 0.95 | 0.95 | 0.95 | 0.8 | 0.95 | 0.95 | 0.95 | 0.95 | -0.1778 | 1.2526 | -0.0383 | True | 0.4177 | Medium |
| 10 | FH | 0.9 | 0.9 | 0.9 | 0.9 | 0.9 | 0.8 | 0.9 | 0.9 | -0.1086 | 0.9854 | 0.0585 | True | 0.4154 | Medium |
| 11 | FH | 0.75 | 0.75 | 0.75 | 0.75 | 0.8 | 0.75 | 0.75 | 0.75 | -0.3085 | 0.3680 | 0.0325 | True | 0.4118 | Medium |
| 12 | FH | 0.9 | 0.9 | 0.9 | 0.9 | 1.1 | 0.9 | 0.9 | 0.9 | -0.2369 | 0.9637 | 0.0904 | True | 0.4156 | Medium |
| 13 | FH | 0.9 | 0.9 | 0.9 | 0.8 | 0.9 | 0.9 | 0.9 | 0.9 | -0.1976 | 1.3006 | 0.0735 | True | 0.4179 | Medium |
| 14 | FH | 0.8 | 0.8 | 1.1 | 0.8 | 0.8 | 0.8 | 0.8 | 1.05 | -0.1948 | 0.9218 | -0.0248 | True | 0.4150 | Medium |
| 15 | FH | 0.8 | 0.8 | 1.1 | 0.8 | 0.8 | 0.8 | 0.8 | 1.05 | -0.2249 | 1.1705 | 0.0667 | True | 0.4130 | Medium |
| 16 | FH | 0.8 | 0.8 | 1.1 | 0.8 | 0.8 | 0.8 | 0.8 | 1.05 | -0.3200 | 1.2490 | 0.0716 | True | 0.4142 | Medium |
| 17 | FH | 0.8 | 0.8 | 1.1 | 0.8 | 0.8 | 0.8 | 0.8 | 1.05 | -0.3083 | 0.8977 | -0.0202 | True | 0.4148 | Medium |
| 18 | FH | 0.8 | 0.8 | 1.1 | 0.8 | 0.8 | 0.8 | 0.8 | 1.05 | -0.2808 | 1.0771 | 0.0277 | True | 0.4154 | Medium |
| 19 | FH | 0.8 | 0.8 | 1.1 | 0.8 | 0.8 | 0.8 | 0.8 | 1.05 | -0.2340 | 0.7977 | 0.0434 | True | 0.4130 | Medium |
| 20 | FH | 0.8 | 0.8 | 1.1 | 0.8 | 0.8 | 0.8 | 0.8 | 1.05 | -0.2539 | 1.1478 | 0.0459 | True | 0.4142 | Medium |
| 21 | FH | 0.8 | 0.8 | 1.1 | 0.8 | 0.8 | 0.8 | 0.8 | 1.05 | -0.3401 | 0.8968 | 0.0296 | True | 0.4153 | Medium |
| 22 | FH | 0.8 | 0.8 | 1.1 | 0.8 | 0.8 | 0.8 | 0.8 | 1.05 | -0.3218 | 1.1070 | -0.0111 | True | 0.4131 | Medium |
| 23 | FH | 0.9 | 0.9 | 0.9 | 1.08 | 0.9 | 0.9 | 0.9 | 0.9 | -0.0617 | 0.7514 | -0.0206 | True | 0.3800 | Medium |
| 24 | FH | 0.8 | 0.8 | 1.1 | 0.8 | 0.8 | 0.8 | 0.8 | 1.05 | -0.3652 | 1.0083 | 0.0244 | True | 0.4076 | Medium |
| 25 | BH | 0.9 | 0.9 | 0.9 | 0.9 | 0.9 | 1.1 | 1.1 | 1.25 | 0.0797 | 0.9861 | -0.0120 | True | 0.4248 | Medium |
| 26 | BH | 0.95 | 0.95 | 1.05 | 1.05 | 0.95 | 1.1 | 1.1 | 1.3 | 0.0710 | 1.0737 | -0.0172 | True | 0.4284 | Medium |
| 27 | BH | 0.9 | 0.9 | 0.9 | 0.9 | 0.8 | 1.1 | 1.1 | 1.35 | 0.0200 | 1.1711 | -0.4000 | True | 0.3939 | Medium |
| 28 | BH | 0.95 | 0.95 | 1.15 | 1.08 | 1.0 | 1.1 | 1.0 | 1.3 | -0.0170 | 1.5435 | -0.0223 | False | 0.4246 | Medium |
| 29 | BH | 0.9 | 0.9 | 1.0 | 0.9 | 0.9 | 1.1 | 1.2 | 1.25 | 0.1132 | 1.4299 | -0.0298 | False | 0.4311 | Medium |
| 30 | BH | 0.9 | 0.9 | 0.9 | 0.9 | 0.9 | 1.1 | 1.2 | 1.2 | 0.2176 | 1.2533 | -0.0202 | True | 0.4262 | Medium |
| 31 | BH | 0.9 | 0.9 | 0.9 | 0.9 | 0.9 | 1.1 | 1.2 | 1.35 | 0.4302 | 1.2174 | -0.0298 | True | 0.4280 | Medium |
| 32 | BH | 0.9 | 0.9 | 0.9 | 0.9 | 0.9 | 1.1 | 1.3 | 1.4 | 0.3523 | 1.0616 | -0.0071 | True | 0.4296 | Medium |

**Explanation:** 
The table summarizes the landing position, peak height, and estimated speed of the ball for each example. 

* **Landing Position:** 
    * **x:**  Indicates how far right/left the ball landed, with positive values being on the right side of the table.
    * **y:** Indicates how far forward/backward the ball landed, with positive values being on the opponent's side.
    * **z:** Indicates the height at which the ball landed.
* **On Table:** Indicates whether the ball landed on the table (True) or not (False).
* **Peak Height:** Represents the maximum height (z-value) reached by the ball during its trajectory.
* **Estimated Speed:** This is a subjective estimation based on the trajectory and the time taken by the ball to land. 

**Note:** The table does not include all possible parameters that could influence the robot's performance, but it provides a general overview of the results achieved with the given parameters.

## Step 2: Closest Parameters

The parameters closest to fulfilling the objective of hitting the ball as far right as possible are:

**a:0.9 b:0.9 c:0.9 d:0.9 e:0.9 f:1.1 g:1.3 h:1.4** (Example 32, BH)

**Reasoning:** Example 32 has the highest x value (0.3523) among all examples, indicating that the ball landed furthest to the right.

## Step 3: Parameter Analysis

**Parameter Analysis:**

* **a & b:** These parameters mainly influence the initial position and orientation of the paddle. They have a minor impact on the ball's landing position, primarily affecting the paddle's starting point and angle.
* **c & d:** These parameters determine the paddle's swing speed and power. Higher values generally lead to a faster swing and more powerful hit, resulting in a faster ball with a longer trajectory. 
* **e & f:** These parameters adjust the paddle's contact point and angle.  Higher values can lead to a more open face angle, influencing the ball's spin and direction.
* **g & h:** These parameters adjust the robot's overall swing speed and force. Higher values usually result in faster swings, potentially influencing the ball's velocity and direction.

**Observations from the Examples:**

* **Higher values of "g" and "h"** generally lead to a higher x-value (further right), indicating that the robot hits the ball more powerfully and with more force. 
* **Higher values of "f"** seem to increase the x-value for backhand strokes.
* **Combinations of parameters** play a role. For example, a combination of higher "g" and "h" with a moderate "f" seems to be effective in pushing the ball further right.

## Step 4: Parameter Proposal

Proposed params: **a:0.9 b:0.9 c:0.9 d:0.9 e:0.9 f:1.2 g:1.3 h:1.4**
Best strokestyle: **BH** 

**Explanation:**

* Based on the analysis, we increase the value of "f" to 1.2 to further enhance the x-value for backhand strokes.  
* We keep "g" and "h" at 1.3 and 1.4 respectively to maintain the powerful swing. 

This proposed parameter set aims to achieve a higher x-value than Example 32 while keeping the stroke style as backhand. 

<q> Hit the ball as far right as possible
## Step 1: Summary Table

| Example | Stroke | a | b | c | d | e | f | g | h | x (landing) |  y (landing) |  z (landing) | On Table | Peak Height (estimated) | Speed (estimated) |
|---|---|---|---|---|---|---|---|---|---|---|---|---|---|---|---|
| 1 | FH | 0.75 | 0.75 | 0.75 | 0.75 | 1.1 | 0.75 | 0.75 | 0.75 | -0.2978 | 0.4482 | 0.0089 | True | 0.37 | Moderate |
| 2 | FH | 0.9 | 0.9 | 0.9 | 0.9 | 0.8 | 0.9 | 0.9 | 0.9 | -0.2155 | 0.9221 | 0.0056 | True | 0.36 | Moderate |
| 3 | FH | 0.75 | 0.75 | 0.75 | 0.75 | 0.75 | 0.75 | 1.1 | 0.75 | -0.1632 | 0.4586 | -0.0168 | True | 0.35 | Moderate |
| 4 | FH | 0.87 | 0.87 | 0.87 | 0.87 | 0.87 | 0.87 | 0.87 | 1.23 | -0.0872 | 0.7329 | 0.0464 | True | 0.35 | Moderate |
| 5 | FH | 0.9 | 0.9 | 0.9 | 0.9 | 0.9 | 0.6 | 0.9 | 0.9 | -0.3773 | 1.2431 | 0.0208 | True | 0.35 | Moderate |
| 6 | FH | 0.9 | 0.9 | 0.9 | 0.9 | 0.9 | 1.1 | 0.9 | 0.9 | -0.1330 | 0.6830 | 0.0013 | True | 0.35 | Moderate |
| 7 | FH | 0.87 | 0.87 | 0.87 | 0.87 | 0.87 | 0.87 | 0.87 | 1.2 | -0.2439 | 0.7760 | 0.0533 | True | 0.34 | Moderate |
| 8 | FH | 0.8 | 0.8 | 1.1 | 0.8 | 0.8 | 0.8 | 0.8 | 0.8 | -0.1013 | 0.5102 | 0.0424 | True | 0.33 | Moderate |
| 9 | FH | 0.95 | 0.95 | 0.95 | 0.8 | 0.95 | 0.95 | 0.95 | 0.95 | -0.1778 | 1.2526 | -0.0383 | True | 0.33 | Moderate |
| 10 | FH | 0.9 | 0.9 | 0.9 | 0.9 | 0.9 | 0.8 | 0.9 | 0.9 | -0.1086 | 0.9854 | 0.0585 | True | 0.33 | Moderate |
| 11 | FH | 0.75 | 0.75 | 0.75 | 0.75 | 0.8 | 0.75 | 0.75 | 0.75 | -0.3085 | 0.3680 | 0.0325 | True | 0.33 | Moderate |
| 12 | FH | 0.9 | 0.9 | 0.9 | 0.9 | 1.1 | 0.9 | 0.9 | 0.9 | -0.2369 | 0.9637 | 0.0904 | True | 0.33 | Moderate |
| 13 | FH | 0.9 | 0.9 | 0.9 | 0.8 | 0.9 | 0.9 | 0.9 | 0.9 | -0.1976 | 1.3006 | 0.0735 | True | 0.32 | Moderate |
| 14 | FH | 0.8 | 0.8 | 1.1 | 0.8 | 0.8 | 0.8 | 0.8 | 1.05 | -0.1948 | 0.9218 | -0.0248 | True | 0.32 | Moderate |
| 15 | FH | 0.8 | 0.8 | 1.1 | 0.8 | 0.8 | 0.8 | 0.8 | 1.05 | -0.2249 | 1.1705 | 0.0667 | True | 0.32 | Moderate |
| 16 | FH | 0.8 | 0.8 | 1.1 | 0.8 | 0.8 | 0.8 | 0.8 | 1.05 | -0.3200 | 1.2490 | 0.0716 | True | 0.31 | Moderate |
| 17 | FH | 0.8 | 0.8 | 1.1 | 0.8 | 0.8 | 0.8 | 0.8 | 1.05 | -0.3083 | 0.8977 | -0.0202 | True | 0.31 | Moderate |
| 18 | FH | 0.8 | 0.8 | 1.1 | 0.8 | 0.8 | 0.8 | 0.8 | 1.05 | -0.2808 | 1.0771 | 0.0277 | True | 0.31 | Moderate |
| 19 | FH | 0.8 | 0.8 | 1.1 | 0.8 | 0.8 | 0.8 | 0.8 | 1.05 | -0.2340 | 0.7977 | 0.0434 | True | 0.30 | Moderate |
| 20 | FH | 0.8 | 0.8 | 1.1 | 0.8 | 0.8 | 0.8 | 0.8 | 1.05 | -0.2539 | 1.1478 | 0.0459 | True | 0.30 | Moderate |
| 21 | FH | 0.8 | 0.8 | 1.1 | 0.8 | 0.8 | 0.8 | 0.8 | 1.05 | -0.3401 | 0.8968 | 0.0296 | True | 0.29 | Moderate |
| 22 | FH | 0.8 | 0.8 | 1.1 | 0.8 | 0.8 | 0.8 | 0.8 | 1.05 | -0.3218 | 1.1070 | -0.0111 | True | 0.29 | Moderate |
| 23 | FH | 0.9 | 0.9 | 0.9 | 1.08 | 0.9 | 0.9 | 0.9 | 0.9 | -0.0617 | 0.7514 | -0.0206 | True | 0.27 | Moderate |
| 24 | FH | 0.8 | 0.8 | 1.1 | 0.8 | 0.8 | 0.8 | 0.8 | 1.05 | -0.3652 | 1.0083 | 0.0244 | True | 0.27 | Moderate |
| 25 | BH | 0.9 | 0.9 | 0.9 | 0.9 | 0.9 | 1.1 | 1.1 | 1.25 | 0.0797 | 0.9861 | -0.0120 | True | 0.36 | Moderate |
| 26 | BH | 0.9 | 0.9 | 0.9 | 0.9 | 0.8 | 1.1 | 1.1 | 1.3 | -0.0182 | 0.7405 | 0.0439 | True | 0.35 | Moderate |
| 27 | BH | 0.9 | 0.9 | 0.9 | 0.9 | 0.8 | 1.1 | 1.1 | 1.35 | 0.0200 | 1.1711 | -0.4000 | True | 0.34 | Moderate |
| 28 | BH | 0.95 | 0.95 | 1.15 | 1.08 | 1.0 | 1.1 | 1.0 | 1.3 | -0.0170 | 1.5435 | -0.0223 | False | 0.34 | Moderate |
| 29 | BH | 0.9 | 0.9 | 1.0 | 0.9 | 0.9 | 1.1 | 1.2 | 1.25 | 0.1132 | 1.4299 | -0.0298 | False | 0.33 | Moderate |
| 30 | BH | 0.9 | 0.9 | 0.9 | 0.9 | 0.9 | 1.1 | 1.2 | 1.2 | 0.2176 | 1.2533 | -0.0202 | True | 0.32 | Moderate |
| 31 | BH | 0.9 | 0.9 | 0.9 | 0.9 | 0.9 | 1.1 | 1.2 | 1.35 | 0.4302 | 1.2174 | -0.0298 | True | 0.31 | Moderate |
| 32 | BH | 0.9 | 0.9 | 0.9 | 0.9 | 0.9 | 1.1 | 1.3 | 1.4 | 0.3523 | 1.0616 | -0.0071 | True | 0.30 | Moderate |
| 33 | BH | 0.9 | 0.9 | 0.9 | 0.9 | 0.9 | 1.2 | 1.3 | 1.4 | 0.4928 | 1.2380 | 0.0181 | True | 0.29 | Moderate |

**Analysis:**

The table shows that higher values for the parameter 'h' generally result in a further landing position to the right. This is due to the parameter 'h' controlling the lateral force applied to the ball during the stroke. Similarly, higher values for 'g' and 'f' tend to increase the distance the ball travels towards the opponent's side. This is because they control the stroke's strength and the amount of forward force applied to the ball respectively. The parameter 'e' controls the vertical force applied to the ball during the stroke. Its effect on landing position is less significant compared to 'h', 'g', and 'f'. However, it appears to contribute to a slightly higher peak height.

## Step 2: Parameters for Best Landing Position

The examples with the highest right-most landing positions are:

* **Example 33 (BH):** x = 0.4928 (a:0.9, b:0.9, c:0.9, d:0.9, e:0.9, f:1.2, g:1.3, h:1.4)
* **Example 31 (BH):** x = 0.4302 (a:0.9, b:0.9, c:0.9, d:0.9, e:0.9, f:1.1, g:1.2, h:1.35)

## Step 3: Parameter Analysis

The most influential parameters for achieving a right-most landing position are:

* **'h':** Controls lateral force. Higher values lead to a further right landing position.
* **'g':** Controls stroke strength. Higher values result in a longer trajectory and a further right landing position.

The other parameters have a less significant impact on the landing position but still contribute to the overall trajectory:

* **'f':** Controls forward force. Higher values increase the distance traveled towards the opponent's side.
* **'e':** Controls vertical force. Higher values lead to a slightly higher peak height.

## Step 4: Proposed Parameters

Proposed params: **a:0.9 b:0.9 c:0.9 d:0.9 e:0.9 f:1.3 g:1.4 h:1.5**
Best strokestyle: **BH** 

**Explanation:**

Based on the analysis, we propose increasing 'h' to 1.5 and 'g' to 1.4 to maximize the lateral force and stroke strength respectively. We also increase 'f' to 1.3 to further contribute to a longer trajectory. The other parameters remain the same, as they have less impact on the landing position in the desired direction. This combination aims to maximize the right-most landing position while avoiding hitting the ball outside of the table. 

<q> Hit the ball as far right as possible
## Step 1: Summary Table

| Example | Stroke | a | b | c | d | e | f | g | h | x (landing) |  y (landing) |  z (landing) |  On Table | Peak Height (z) | Estimated Speed |
|---|---|---|---|---|---|---|---|---|---|---|---|---|---|---|
| 1 | FH | 0.75 | 0.75 | 0.75 | 0.75 | 1.1 | 0.75 | 0.75 | 0.75 | -0.2978 | 0.4482 | 0.0089 | True | 0.4025 | Medium |
| 2 | FH | 0.9 | 0.9 | 0.9 | 0.9 | 0.8 | 0.9 | 0.9 | 0.9 | -0.2155 | 0.9221 | 0.0056 | True | 0.4211 | Medium |
| 3 | FH | 0.75 | 0.75 | 0.75 | 0.75 | 0.75 | 0.75 | 1.1 | 0.75 | -0.1632 | 0.4586 | -0.0168 | True | 0.4246 | Medium |
| 4 | FH | 0.87 | 0.87 | 0.87 | 0.87 | 0.87 | 0.87 | 0.87 | 1.23 | -0.0872 | 0.7329 | 0.0464 | True | 0.4131 | Medium |
| 5 | FH | 0.9 | 0.9 | 0.9 | 0.9 | 0.9 | 0.6 | 0.9 | 0.9 | -0.3773 | 1.2431 | 0.0208 | True | 0.4167 | Medium |
| 6 | FH | 0.9 | 0.9 | 0.9 | 0.9 | 0.9 | 1.1 | 0.9 | 0.9 | -0.1330 | 0.6830 | 0.0013 | True | 0.4210 | Medium |
| 7 | FH | 0.87 | 0.87 | 0.87 | 0.87 | 0.87 | 0.87 | 0.87 | 1.2 | -0.2439 | 0.7760 | 0.0533 | True | 0.4076 | Medium |
| 8 | FH | 0.8 | 0.8 | 1.1 | 0.8 | 0.8 | 0.8 | 0.8 | 0.8 | -0.1013 | 0.5102 | 0.0424 | True | 0.4050 | Medium |
| 9 | FH | 0.95 | 0.95 | 0.95 | 0.8 | 0.95 | 0.95 | 0.95 | 0.95 | -0.1778 | 1.2526 | -0.0383 | True | 0.4177 | Medium |
| 10 | FH | 0.9 | 0.9 | 0.9 | 0.9 | 0.9 | 0.8 | 0.9 | 0.9 | -0.1086 | 0.9854 | 0.0585 | True | 0.4154 | Medium |
| 11 | FH | 0.75 | 0.75 | 0.75 | 0.75 | 0.8 | 0.75 | 0.75 | 0.75 | -0.3085 | 0.3680 | 0.0325 | True | 0.4118 | Medium |
| 12 | FH | 0.9 | 0.9 | 0.9 | 0.9 | 1.1 | 0.9 | 0.9 | 0.9 | -0.2369 | 0.9637 | 0.0904 | True | 0.4156 | Medium |
| 13 | FH | 0.9 | 0.9 | 0.9 | 0.8 | 0.9 | 0.9 | 0.9 | 0.9 | -0.1976 | 1.3006 | 0.0735 | True | 0.4179 | Medium |
| 14 | FH | 0.8 | 0.8 | 1.1 | 0.8 | 0.8 | 0.8 | 0.8 | 1.05 | -0.1948 | 0.9218 | -0.0248 | True | 0.4150 | Medium |
| 15 | FH | 0.8 | 0.8 | 1.1 | 0.8 | 0.8 | 0.8 | 0.8 | 1.05 | -0.2249 | 1.1705 | 0.0667 | True | 0.4130 | Medium |
| 16 | FH | 0.8 | 0.8 | 1.1 | 0.8 | 0.8 | 0.8 | 0.8 | 1.05 | -0.3200 | 1.2490 | 0.0716 | True | 0.4142 | Medium |
| 17 | FH | 0.8 | 0.8 | 1.1 | 0.8 | 0.8 | 0.8 | 0.8 | 1.05 | -0.3083 | 0.8977 | -0.0202 | True | 0.4148 | Medium |
| 18 | FH | 0.8 | 0.8 | 1.1 | 0.8 | 0.8 | 0.8 | 0.8 | 1.05 | -0.2808 | 1.0771 | 0.0277 | True | 0.4154 | Medium |
| 19 | FH | 0.8 | 0.8 | 1.1 | 0.8 | 0.8 | 0.8 | 0.8 | 1.05 | -0.2340 | 0.7977 | 0.0434 | True | 0.4130 | Medium |
| 20 | FH | 0.8 | 0.8 | 1.1 | 0.8 | 0.8 | 0.8 | 0.8 | 1.05 | -0.2539 | 1.1478 | 0.0459 | True | 0.4142 | Medium |
| 21 | FH | 0.8 | 0.8 | 1.1 | 0.8 | 0.8 | 0.8 | 0.8 | 1.05 | -0.3401 | 0.8968 | 0.0296 | True | 0.4153 | Medium |
| 22 | FH | 0.8 | 0.8 | 1.1 | 0.8 | 0.8 | 0.8 | 0.8 | 1.05 | -0.3218 | 1.1070 | -0.0111 | True | 0.4131 | Medium |
| 23 | FH | 0.9 | 0.9 | 0.9 | 1.08 | 0.9 | 0.9 | 0.9 | 0.9 | -0.0617 | 0.7514 | -0.0206 | True | 0.3905 | Medium |
| 24 | FH | 0.8 | 0.8 | 1.1 | 0.8 | 0.8 | 0.8 | 0.8 | 1.05 | -0.3652 | 1.0083 | 0.0244 | True | 0.4076 | Medium |
| 25 | FH | 0.9 | 0.9 | 0.9 | 0.9 | 0.9 | 1.1 | 1.1 | 1.25 | 0.0797 | 0.9861 | -0.0120 | True | 0.4248 | Medium |
| 26 | FH | 0.95 | 0.95 | 1.05 | 1.05 | 1.05 | 1.1 | 1.1 | 1.3 | 0.1190 | 1.1193 | -0.0173 | True | 0.4284 | Medium |
| 27 | FH | 0.9 | 0.9 | 0.9 | 0.9 | 0.8 | 1.1 | 1.1 | 1.35 | 0.0200 | 1.1711 | -0.4000 | True | 0.3939 | Medium |
| 28 | FH | 0.95 | 0.95 | 1.15 | 1.08 | 1.0 | 1.1 | 1.0 | 1.3 | -0.0170 | 1.5435 | -0.0223 | False | 0.4246 | Medium |
| 29 | FH | 0.9 | 0.9 | 1.0 | 0.9 | 0.9 | 1.1 | 1.2 | 1.25 | 0.1132 | 1.4299 | -0.0298 | False | 0.4311 | Medium |
| 30 | FH | 0.9 | 0.9 | 0.9 | 0.9 | 0.9 | 1.1 | 1.2 | 1.2 | 0.2176 | 1.2533 | -0.0202 | True | 0.4262 | Medium |
| 31 | FH | 0.9 | 0.9 | 0.9 | 0.9 | 0.9 | 1.1 | 1.2 | 1.35 | 0.4302 | 1.2174 | -0.0298 | True | 0.4280 | Medium |
| 32 | FH | 0.9 | 0.9 | 0.9 | 0.9 | 0.9 | 1.1 | 1.3 | 1.4 | 0.3523 | 1.0616 | -0.0071 | True | 0.4296 | Medium |
| 33 | FH | 0.9 | 0.9 | 0.9 | 0.9 | 0.9 | 1.2 | 1.3 | 1.4 | 0.4928 | 1.2380 | 0.0181 | True | 0.4279 | Medium |
| 34 | FH | 0.9 | 0.9 | 0.9 | 0.9 | 0.9 | 1.3 | 1.4 | 1.5 | 0.4065 | 1.2939 | -0.0213 | True | 0.4324 | Medium |
| 1 | BH | 0.75 | 0.75 | 0.75 | 0.75 | 1.1 | 0.75 | 0.75 | 0.75 | -0.2978 | 0.4482 | 0.0089 | True | 0.4025 | Medium |
| 2 | BH | 0.9 | 0.9 | 0.9 | 0.9 | 0.8 | 0.9 | 0.9 | 0.9 | -0.2155 | 0.9221 | 0.0056 | True | 0.4211 | Medium |
| 3 | BH | 0.75 | 0.75 | 0.75 | 0.75 | 0.75 | 0.75 | 1.1 | 0.75 | -0.1632 | 0.4586 | -0.0168 | True | 0.4246 | Medium |
| 4 | BH | 0.87 | 0.87 | 0.87 | 0.87 | 0.87 | 0.87 | 0.87 | 1.23 | -0.0872 | 0.7329 | 0.0464 | True | 0.4131 | Medium |
| 5 | BH | 0.9 | 0.9 | 0.9 | 0.9 | 0.9 | 0.6 | 0.9 | 0.9 | -0.3773 | 1.2431 | 0.0208 | True | 0.4167 | Medium |
| 6 | BH | 0.9 | 0.9 | 0.9 | 0.9 | 0.9 | 1.1 | 0.9 | 0.9 | -0.1330 | 0.6830 | 0.0013 | True | 0.4210 | Medium |
| 7 | BH | 0.87 | 0.87 | 0.87 | 0.87 | 0.87 | 0.87 | 0.87 | 1.2 | -0.2439 | 0.7760 | 0.0533 | True | 0.4076 | Medium |
| 8 | BH | 0.8 | 0.8 | 1.1 | 0.8 | 0.8 | 0.8 | 0.8 | 0.8 | -0.1013 | 0.5102 | 0.0424 | True | 0.4050 | Medium |
| 9 | BH | 0.95 | 0.95 | 0.95 | 0.8 | 0.95 | 0.95 | 0.95 | 0.95 | -0.1778 | 1.2526 | -0.0383 | True | 0.4177 | Medium |
| 10 | BH | 0.9 | 0.9 | 0.9 | 0.9 | 0.9 | 0.8 | 0.9 | 0.9 | -0.1086 | 0.9854 | 0.0585 | True | 0.4154 | Medium |
| 11 | BH | 0.75 | 0.75 | 0.75 | 0.75 | 0.8 | 0.75 | 0.75 | 0.75 | -0.3085 | 0.3680 | 0.0325 | True | 0.4118 | Medium |
| 12 | BH | 0.9 | 0.9 | 0.9 | 0.9 | 1.1 | 0.9 | 0.9 | 0.9 | -0.2369 | 0.9637 | 0.0904 | True | 0.4156 | Medium |
| 13 | BH | 0.9 | 0.9 | 0.9 | 0.8 | 0.9 | 0.9 | 0.9 | 0.9 | -0.1976 | 1.3006 | 0.0735 | True | 0.4179 | Medium |
| 14 | BH | 0.8 | 0.8 | 1.1 | 0.8 | 0.8 | 0.8 | 0.8 | 1.05 | -0.1948 | 0.9218 | -0.0248 | True | 0.4150 | Medium |
| 15 | BH | 0.8 | 0.8 | 1.1 | 0.8 | 0.8 | 0.8 | 0.8 | 1.05 | -0.2249 | 1.1705 | 0.0667 | True | 0.4130 | Medium |
| 16 | BH | 0.8 | 0.8 | 1.1 | 0.8 | 0.8 | 0.8 | 0.8 | 1.05 | -0.3200 | 1.2490 | 0.0716 | True | 0.4142 | Medium |
| 17 | BH | 0.8 | 0.8 | 1.1 | 0.8 | 0.8 | 0.8 | 0.8 | 1.05 | -0.3083 | 0.8977 | -0.0202 | True | 0.4148 | Medium |
| 18 | BH | 0.8 | 0.8 | 1.1 | 0.8 | 0.8 | 0.8 | 0.8 | 1.05 | -0.2808 | 1.0771 | 0.0277 | True | 0.4154 | Medium |
| 19 | BH | 0.8 | 0.8 | 1.1 | 0.8 | 0.8 | 0.8 | 0.8 | 1.05 | -0.2340 | 0.7977 | 0.0434 | True | 0.4130 | Medium |
| 20 | BH | 0.8 | 0.8 | 1.1 | 0.8 | 0.8 | 0.8 | 0.8 | 1.05 | -0.2539 | 1.1478 | 0.0459 | True | 0.4142 | Medium |
| 21 | BH | 0.8 | 0.8 | 1.1 | 0.8 | 0.8 | 0.8 | 0.8 | 1.05 | -0.3401 | 0.8968 | 0.0296 | True | 0.4153 | Medium |
| 22 | BH | 0.8 | 0.8 | 1.1 | 0.8 | 0.8 | 0.8 | 0.8 | 1.05 | -0.3218 | 1.1070 | -0.0111 | True | 0.4131 | Medium |
| 23 | BH | 0.9 | 0.9 | 0.9 | 1.08 | 0.9 | 0.9 | 0.9 | 0.9 | -0.0617 | 0.7514 | -0.0206 | True | 0.3905 | Medium |
| 24 | BH | 0.8 | 0.8 | 1.1 | 0.8 | 0.8 | 0.8 | 0.8 | 1.05 | -0.3652 | 1.0083 | 0.0244 | True | 0.4076 | Medium |

**Analysis:**

The examples show that landing position is influenced by several parameters. The most significant parameter appears to be **g** (the horizontal paddle velocity). Larger **g** values generally lead to a greater x landing position (hitting the ball further right). Other parameters, such as **h** (paddle contact height), also seem to play a role, but to a lesser extent. The combination of **g**, **h**, **c** (ball vertical velocity), **d** (ball horizontal velocity) and **e** (paddle vertical velocity) determines the ball trajectory and hence the landing position. For example, increasing the paddle contact height **h** leads to a greater peak height (z) of the ball during its trajectory. A higher peak height can potentially affect the landing position depending on the values of the other parameters.

**Important Note:** This analysis is based on a limited dataset. Further experimentation and analysis are needed to draw more robust conclusions.

## Step 2: Parameters closest to objective

The examples with the highest x landing position (farthest right) are:
* Example 25: x = 0.0797
* Example 26: x = 0.1190
* Example 29: x = 0.1132
* Example 30: x = 0.2176
* Example 31: x = 0.4302
* Example 32: x = 0.3523
* Example 33: x = 0.4928
* Example 34: x = 0.4065

Out of these, examples 33 and 31 have the highest x landing position.

## Step 3: Analyzing parameter effects

Looking at the parameters for examples 33 and 31, we can observe:

* **g** (horizontal paddle velocity): Both examples have high **g** values (1.3 and 1.2 respectively), which contributes to the rightward landing position.
* **h** (paddle contact height): Both examples have relatively high **h** values (1.4 and 1.35), which potentially contribute to the ball's peak height and landing position.
* **c** (ball vertical velocity), **d** (ball horizontal velocity) and **e** (paddle vertical velocity) : The combination of these parameters contributes to the overall trajectory of the ball. 

## Step 4: Proposed parameters and strokestyle

Proposed params: a:0.9 b:0.9 c:0.9 d:0.9 e:0.9 f:1.2 g:1.4 h:1.5
Best strokestyle: FH 

<q> Hit the ball as far right as possible
## Step 1: Summary Table

| Example | Stroke | a | b | c | d | e | f | g | h | x (Landing Position) | z (Peak Height) | Estimated Speed |
|---|---|---|---|---|---|---|---|---|---|---|---|---|
| 1 | FH | 0.75 | 0.75 | 0.75 | 0.75 | 1.1 | 0.75 | 0.75 | 0.75 | -0.2978 | 0.3763 | Medium |
| 2 | FH | 0.9 | 0.9 | 0.9 | 0.9 | 0.8 | 0.9 | 0.9 | 0.9 | -0.2155 | 0.3952 | Medium |
| 3 | FH | 0.75 | 0.75 | 0.75 | 0.75 | 0.75 | 0.75 | 1.1 | 0.75 | -0.1632 | 0.3898 | Medium |
| 4 | FH | 0.87 | 0.87 | 0.87 | 0.87 | 0.87 | 0.87 | 0.87 | 1.23 | -0.0872 | 0.3898 | Medium |
| 5 | FH | 0.9 | 0.9 | 0.9 | 0.9 | 0.9 | 0.6 | 0.9 | 0.9 | -0.3773 | 0.3639 | Medium |
| 6 | FH | 0.9 | 0.9 | 0.9 | 0.9 | 0.9 | 1.1 | 0.9 | 0.9 | -0.1330 | 0.3363 | Medium |
| 7 | FH | 0.87 | 0.87 | 0.87 | 0.87 | 0.87 | 0.87 | 0.87 | 1.2 | -0.2439 | 0.2464 | Medium |
| 8 | FH | 0.8 | 0.8 | 1.1 | 0.8 | 0.8 | 0.8 | 0.8 | 0.8 | -0.1013 | 0.3609 | Medium |
| 9 | FH | 0.95 | 0.95 | 0.95 | 0.8 | 0.95 | 0.95 | 0.95 | 0.95 | -0.1778 | 0.3666 | Medium |
| 10 | FH | 0.9 | 0.9 | 0.9 | 0.9 | 0.9 | 0.8 | 0.9 | 0.9 | -0.1086 | 0.3734 | Medium |
| 11 | FH | 0.75 | 0.75 | 0.75 | 0.75 | 0.8 | 0.75 | 0.75 | 0.75 | -0.3085 | 0.3963 | Medium |
| 12 | FH | 0.9 | 0.9 | 0.9 | 0.9 | 1.1 | 0.9 | 0.9 | 0.9 | -0.2369 | 0.3278 | Medium |
| 13 | FH | 0.9 | 0.9 | 0.9 | 0.8 | 0.9 | 0.9 | 0.9 | 0.9 | -0.1976 | 0.4008 | Medium |
| 14 | FH | 0.8 | 0.8 | 1.1 | 0.8 | 0.8 | 0.8 | 0.8 | 1.05 | -0.1948 | 0.3903 | Medium |
| 15 | FH | 0.8 | 0.8 | 1.1 | 0.8 | 0.8 | 0.8 | 0.8 | 1.05 | -0.2249 | 0.3760 | Medium |
| 16 | FH | 0.8 | 0.8 | 1.1 | 0.8 | 0.8 | 0.8 | 0.8 | 1.05 | -0.3200 | 0.3427 | Medium |
| 17 | FH | 0.8 | 0.8 | 1.1 | 0.8 | 0.8 | 0.8 | 0.8 | 1.05 | -0.3083 | 0.4120 | Medium |
| 18 | FH | 0.8 | 0.8 | 1.1 | 0.8 | 0.8 | 0.8 | 0.8 | 1.05 | -0.2808 | 0.3800 | Medium |
| 19 | FH | 0.8 | 0.8 | 1.1 | 0.8 | 0.8 | 0.8 | 0.8 | 1.05 | -0.2340 | 0.3716 | Medium |
| 20 | FH | 0.8 | 0.8 | 1.1 | 0.8 | 0.8 | 0.8 | 0.8 | 1.05 | -0.2539 | 0.3833 | Medium |
| 21 | FH | 0.8 | 0.8 | 1.1 | 0.8 | 0.8 | 0.8 | 0.8 | 1.05 | -0.3401 | 0.3822 | Medium |
| 22 | FH | 0.8 | 0.8 | 1.1 | 0.8 | 0.8 | 0.8 | 0.8 | 1.05 | -0.3218 | 0.3755 | Medium |
| 23 | FH | 0.9 | 0.9 | 0.9 | 1.08 | 0.9 | 0.9 | 0.9 | 0.9 | -0.0617 | 0.3539 | Medium |
| 24 | FH | 0.8 | 0.8 | 1.1 | 0.8 | 0.8 | 0.8 | 0.8 | 1.05 | -0.3652 | 0.3628 | Medium |

**Analysis of Landing Position:**

The objective is to hit the ball as far right as possible.  Looking at the 'x (Landing Position)' column, we can see that none of the examples consistently hit the ball far to the right. Most examples land the ball in the negative x range, indicating they land on the left side of the table. 

**Peak Height and Estimated Speed:**

The 'z (Peak Height)' and 'Estimated Speed' columns are not directly related to the objective. These parameters are likely influencing the trajectory of the ball and its overall distance traveled, but not necessarily its lateral position on the table.

**Parameter a, b, c, d, e, f, g, h and Stroke Style:**

The parameters 'a' through 'h' control the robot's movements and directly impact the ball's trajectory.  It is not possible to determine the exact effect of each parameter on landing position without further analysis and experimentation. 

**Stroke Style:**

All examples used a forehand stroke (FH). 

## Step 2: Closest Parameters

The closest parameters to fulfilling the objective are found in **Example 34**, where the ball landed at **x = 0.4065**. This is the furthest right landing position among the examples.

## Step 3: Analysis of Parameter Effects

We can analyze the effect of the parameters on landing position by comparing the values of 'a' through 'h' across the examples, especially focusing on Examples 34 (best result) and the other examples with similar parameter values. 

**Parameter 'g' and 'h':**

* Example 34 has a higher 'g' value (1.3) and a higher 'h' value (1.5) compared to most other examples. This suggests that higher values of 'g' and 'h' may contribute to a greater lateral deviation of the ball, potentially pushing it further to the right.

**Parameter 'f':**

* Example 34 has a higher 'f' value (1.3) than most other examples. This could be influencing the angle at which the ball is hit, possibly causing it to move further right.

**Parameter 'e':**

* Example 34 has a value of 'e' at 0.9, while some examples that land further left (e.g., Example 28) have higher 'e' values.  This might indicate that lower 'e' values could help in hitting the ball further right.

**Other Parameters:**

* It is difficult to establish a definitive correlation between the other parameters ('a', 'b', 'c', 'd') and landing position based on this limited data.

## Step 4: Proposed Parameters and Stroke Style

Proposed params: **a:0.9 b:0.9 c:0.9 d:0.9 e:0.8 f:1.4 g:1.4 h:1.6**
Best strokestyle: **FH** 

<q> Hit the ball as far right as possible
## Step 1: Summary Table

| Example | Stroke | a | b | c | d | e | f | g | h | x (landing) |  y (landing) |  z (landing) | On Table | Peak Height (estimated) | Speed (estimated) |
|---|---|---|---|---|---|---|---|---|---|---|---|---|---|---|---|
| 1 | FH | 0.75 | 0.75 | 0.75 | 0.75 | 1.1 | 0.75 | 0.75 | 0.75 | -0.2978 | 0.4482 | 0.0089 | True | 0.3763 | 0.27 |
| 2 | FH | 0.9 | 0.9 | 0.9 | 0.9 | 0.8 | 0.9 | 0.9 | 0.9 | -0.2155 | 0.9221 | 0.0056 | True | 0.3952 | 0.31 |
| 3 | FH | 0.75 | 0.75 | 0.75 | 0.75 | 0.75 | 0.75 | 1.1 | 0.75 | -0.1632 | 0.4586 | -0.0168 | True | 0.3898 | 0.28 |
| 4 | FH | 0.87 | 0.87 | 0.87 | 0.87 | 0.87 | 0.87 | 0.87 | 1.23 | -0.0872 | 0.7329 | 0.0464 | True | 0.3898 | 0.28 |
| 5 | FH | 0.9 | 0.9 | 0.9 | 0.9 | 0.9 | 0.6 | 0.9 | 0.9 | -0.3773 | 1.2431 | 0.0208 | True | 0.3639 | 0.31 |
| 6 | FH | 0.9 | 0.9 | 0.9 | 0.9 | 0.9 | 1.1 | 0.9 | 0.9 | -0.1330 | 0.6830 | 0.0013 | True | 0.3363 | 0.28 |
| 7 | FH | 0.87 | 0.87 | 0.87 | 0.87 | 0.87 | 0.87 | 0.87 | 1.2 | -0.2439 | 0.7760 | 0.0533 | True | 0.2464 | 0.23 |
| 8 | FH | 0.8 | 0.8 | 1.1 | 0.8 | 0.8 | 0.8 | 0.8 | 0.8 | -0.1013 | 0.5102 | 0.0424 | True | 0.3609 | 0.27 |
| 9 | FH | 0.95 | 0.95 | 0.95 | 0.8 | 0.95 | 0.95 | 0.95 | 0.95 | -0.1778 | 1.2526 | -0.0383 | True | 0.3666 | 0.31 |
| 10 | FH | 0.9 | 0.9 | 0.9 | 0.9 | 0.9 | 0.8 | 0.9 | 0.9 | -0.1086 | 0.9854 | 0.0585 | True | 0.3734 | 0.27 |
| 11 | FH | 0.75 | 0.75 | 0.75 | 0.75 | 0.8 | 0.75 | 0.75 | 0.75 | -0.3085 | 0.3680 | 0.0325 | True | 0.3963 | 0.27 |
| 12 | FH | 0.9 | 0.9 | 0.9 | 0.9 | 1.1 | 0.9 | 0.9 | 0.9 | -0.2369 | 0.9637 | 0.0904 | True | 0.3278 | 0.29 |
| 13 | FH | 0.9 | 0.9 | 0.9 | 0.8 | 0.9 | 0.9 | 0.9 | 0.9 | -0.1976 | 1.3006 | 0.0735 | True | 0.4008 | 0.28 |
| 14 | FH | 0.8 | 0.8 | 1.1 | 0.8 | 0.8 | 0.8 | 0.8 | 1.05 | -0.1948 | 0.9218 | -0.0248 | True | 0.3903 | 0.28 |
| 15 | FH | 0.8 | 0.8 | 1.1 | 0.8 | 0.8 | 0.8 | 0.8 | 1.05 | -0.2249 | 1.1705 | 0.0667 | True | 0.3760 | 0.27 |
| 16 | FH | 0.8 | 0.8 | 1.1 | 0.8 | 0.8 | 0.8 | 0.8 | 1.05 | -0.3200 | 1.2490 | 0.0716 | True | 0.3427 | 0.26 |
| 17 | FH | 0.8 | 0.8 | 1.1 | 0.8 | 0.8 | 0.8 | 0.8 | 1.05 | -0.3083 | 0.8977 | -0.0202 | True | 0.4120 | 0.28 |
| 18 | FH | 0.8 | 0.8 | 1.1 | 0.8 | 0.8 | 0.8 | 0.8 | 1.05 | -0.2808 | 1.0771 | 0.0277 | True | 0.3800 | 0.27 |
| 19 | FH | 0.8 | 0.8 | 1.1 | 0.8 | 0.8 | 0.8 | 0.8 | 1.05 | -0.2340 | 0.7977 | 0.0434 | True | 0.3716 | 0.27 |
| 20 | FH | 0.8 | 0.8 | 1.1 | 0.8 | 0.8 | 0.8 | 0.8 | 1.05 | -0.2539 | 1.1478 | 0.0459 | True | 0.3833 | 0.27 |
| 21 | FH | 0.8 | 0.8 | 1.1 | 0.8 | 0.8 | 0.8 | 0.8 | 1.05 | -0.3401 | 0.8968 | 0.0296 | True | 0.3822 | 0.27 |
| 22 | FH | 0.8 | 0.8 | 1.1 | 0.8 | 0.8 | 0.8 | 0.8 | 1.05 | -0.3218 | 1.1070 | -0.0111 | True | 0.3755 | 0.27 |
| 23 | FH | 0.9 | 0.9 | 0.9 | 1.08 | 0.9 | 0.9 | 0.9 | 0.9 | -0.0617 | 0.7514 | -0.0206 | True | 0.3539 | 0.22 |
| 24 | FH | 0.8 | 0.8 | 1.1 | 0.8 | 0.8 | 0.8 | 0.8 | 1.05 | -0.3652 | 1.0083 | 0.0244 | True | 0.3628 | 0.26 |
| 25 | BH | 0.9 | 0.9 | 0.9 | 0.9 | 0.9 | 1.1 | 1.1 | 1.25 | 0.0797 | 0.9861 | -0.0120 | True | 0.3474 | 0.27 |
| 26 | BH | 0.9 | 0.9 | 0.9 | 0.9 | 0.9 | 1.1 | 1.1 | 1.3 | 0.1086 | 1.0978 | -0.0135 | True | 0.3666 | 0.32 |
| 27 | BH | 0.9 | 0.9 | 0.9 | 0.9 | 0.8 | 1.1 | 1.1 | 1.35 | 0.0200 | 1.1711 | -0.4000 | True | -0.3113 | 0.24 |
| 28 | BH | 0.95 | 0.95 | 1.15 | 1.08 | 1.0 | 1.1 | 1.0 | 1.3 | -0.0170 | 1.5435 | -0.0223 | False | 0.3548 | 0.25 |
| 29 | BH | 0.9 | 0.9 | 1.0 | 0.9 | 0.9 | 1.1 | 1.2 | 1.25 | 0.1132 | 1.4299 | -0.0298 | False | 0.3727 | 0.33 |
| 30 | BH | 0.9 | 0.9 | 0.9 | 0.9 | 0.9 | 1.1 | 1.2 | 1.2 | 0.2176 | 1.2533 | -0.0202 | True | 0.3985 | 0.37 |
| 31 | BH | 0.9 | 0.9 | 0.9 | 0.9 | 0.9 | 1.1 | 1.2 | 1.35 | 0.4302 | 1.2174 | -0.0298 | True | 0.3668 | 0.32 |
| 32 | BH | 0.9 | 0.9 | 0.9 | 0.9 | 0.9 | 1.1 | 1.3 | 1.4 | 0.3523 | 1.0616 | -0.0071 | True | 0.3772 | 0.37 |
| 33 | BH | 0.9 | 0.9 | 0.9 | 0.9 | 0.9 | 1.2 | 1.3 | 1.4 | 0.4928 | 1.2380 | 0.0181 | True | 0.3728 | 0.39 |
| 34 | BH | 0.9 | 0.9 | 0.9 | 0.9 | 0.9 | 1.3 | 1.4 | 1.5 | 0.4065 | 1.2939 | -0.0213 | True | 0.3976 | 0.37 |
| 35 | BH | 0.9 | 0.9 | 0.9 | 0.9 | 0.9 | 1.2 | 1.4 | 1.5 | 0.3354 | 1.2801 | -0.0272 | True | 0.4054 | 0.38 |
| 36 | BH | 0.9 | 0.9 | 0.9 | 0.9 | 0.8 | 1.4 | 1.4 | 1.6 | 0.5400 | 1.0472 | -0.0376 | True | 0.3869 | 0.38 |

The table summarizes the landing position, estimated peak height, and estimated speed of the ball for each example. The estimated peak height and speed are calculated based on the ball's trajectory. For example, in Example 1, the ball reaches a peak height of 0.3763 and an estimated speed of 0.27. The speed is estimated based on the distance covered by the ball in the time period observed.

## Step 2: Parameters Closest to Objective

The parameters closest to fulfilling the objective of hitting the ball as far right as possible are:

* **Example 36:** a:0.9 b:0.9 c:0.9 d:0.9 e:0.8 f:1.4 g:1.4 h:1.6 

The ball lands at x = 0.5400, which is furthest to the right compared to other examples.

## Step 3: Analysis of Parameter Effects

**a, b, c, d:** These parameters seem to influence the initial trajectory of the ball. Higher values of these parameters tend to lead to a flatter trajectory, while lower values create a more curved trajectory. 

**e:** This parameter impacts the ball's trajectory after contact with the paddle. Higher values seem to cause a more pronounced upward arc, resulting in a higher peak and potentially a longer flight time.

**f:**  This parameter controls the paddle's horizontal movement.  Higher values indicate a more pronounced horizontal paddle swing, potentially leading to a wider range of ball landing positions.

**g:** This parameter influences the paddle's vertical movement.  Higher values lead to a more pronounced upward swing, resulting in a higher ball peak. 

**h:** This parameter controls the paddle's speed.  Higher values indicate a faster paddle swing, potentially leading to a faster ball speed.

## Step 4: New Parameter Proposal

Proposed params: a:0.8 b:0.9 c:0.9 d:0.9 e:0.9 f:1.4 g:1.4 h:1.7 
Best strokestyle: BH

By increasing the value of 'h' while maintaining the other parameters of Example 36, we aim to further increase the ball's speed, potentially leading to a longer flight time and an even further right landing position. This proposed set of parameters avoids hitting the ball outside of the table based on the observed patterns in the previous examples. 

<q> Hit the ball as far right as possible
## Step 1: Summary Table

| Example | Stroke | a | b | c | d | e | f | g | h | x (landing) | y (landing) | z (peak) | Estimated Speed |
|---|---|---|---|---|---|---|---|---|---|---|---|---|---|
| 1 | FH | 0.75 | 0.75 | 0.75 | 0.75 | 1.1 | 0.75 | 0.75 | 0.75 | -0.2978 | 0.4482 | 0.3763 | Moderate |
| 2 | FH | 0.9 | 0.9 | 0.9 | 0.9 | 0.8 | 0.9 | 0.9 | 0.9 | -0.2155 | 0.9221 | 0.3952 | Moderate |
| 3 | FH | 0.75 | 0.75 | 0.75 | 0.75 | 0.75 | 0.75 | 1.1 | 0.75 | -0.1632 | 0.4586 | 0.3898 | Moderate |
| 4 | FH | 0.87 | 0.87 | 0.87 | 0.87 | 0.87 | 0.87 | 0.87 | 1.23 | -0.0872 | 0.7329 | 0.3898 | Moderate |
| 5 | FH | 0.9 | 0.9 | 0.9 | 0.9 | 0.9 | 0.6 | 0.9 | 0.9 | -0.3773 | 1.2431 | 0.3639 | Fast |
| 6 | FH | 0.9 | 0.9 | 0.9 | 0.9 | 0.9 | 1.1 | 0.9 | 0.9 | -0.1330 | 0.6830 | 0.3363 | Fast |
| 7 | FH | 0.87 | 0.87 | 0.87 | 0.87 | 0.87 | 0.87 | 0.87 | 1.2 | -0.2439 | 0.7760 | 0.2464 | Moderate |
| 8 | FH | 0.8 | 0.8 | 1.1 | 0.8 | 0.8 | 0.8 | 0.8 | 0.8 | -0.1013 | 0.5102 | 0.3609 | Moderate |
| 9 | FH | 0.95 | 0.95 | 0.95 | 0.8 | 0.95 | 0.95 | 0.95 | 0.95 | -0.1778 | 1.2526 | 0.3666 | Moderate |
| 10 | FH | 0.9 | 0.9 | 0.9 | 0.9 | 0.9 | 0.8 | 0.9 | 0.9 | -0.1086 | 0.9854 | 0.3734 | Moderate |
| 11 | FH | 0.75 | 0.75 | 0.75 | 0.75 | 0.8 | 0.75 | 0.75 | 0.75 | -0.3085 | 0.3680 | 0.3963 | Moderate |
| 12 | FH | 0.9 | 0.9 | 0.9 | 0.9 | 1.1 | 0.9 | 0.9 | 0.9 | -0.2369 | 0.9637 | 0.3278 | Moderate |
| 13 | FH | 0.9 | 0.9 | 0.9 | 0.8 | 0.9 | 0.9 | 0.9 | 0.9 | -0.1976 | 1.3006 | 0.4008 | Moderate |
| 14 | FH | 0.8 | 0.8 | 1.1 | 0.8 | 0.8 | 0.8 | 0.8 | 1.05 | -0.1948 | 0.9218 | 0.3903 | Moderate |
| 15 | FH | 0.8 | 0.8 | 1.1 | 0.8 | 0.8 | 0.8 | 0.8 | 1.05 | -0.2249 | 1.1705 | 0.3760 | Moderate |
| 16 | FH | 0.8 | 0.8 | 1.1 | 0.8 | 0.8 | 0.8 | 0.8 | 1.05 | -0.3200 | 1.2490 | 0.3427 | Moderate |
| 17 | FH | 0.8 | 0.8 | 1.1 | 0.8 | 0.8 | 0.8 | 0.8 | 1.05 | -0.3083 | 0.8977 | 0.4120 | Moderate |
| 18 | FH | 0.8 | 0.8 | 1.1 | 0.8 | 0.8 | 0.8 | 0.8 | 1.05 | -0.2808 | 1.0771 | 0.3800 | Moderate |
| 19 | FH | 0.8 | 0.8 | 1.1 | 0.8 | 0.8 | 0.8 | 0.8 | 1.05 | -0.2340 | 0.7977 | 0.3716 | Moderate |
| 20 | FH | 0.8 | 0.8 | 1.1 | 0.8 | 0.8 | 0.8 | 0.8 | 1.05 | -0.2539 | 1.1478 | 0.3833 | Moderate |
| 21 | FH | 0.8 | 0.8 | 1.1 | 0.8 | 0.8 | 0.8 | 0.8 | 1.05 | -0.3401 | 0.8968 | 0.3822 | Moderate |
| 22 | FH | 0.8 | 0.8 | 1.1 | 0.8 | 0.8 | 0.8 | 0.8 | 1.05 | -0.3218 | 1.1070 | 0.3755 | Moderate |
| 23 | FH | 0.9 | 0.9 | 0.9 | 1.08 | 0.9 | 0.9 | 0.9 | 0.9 | -0.0617 | 0.7514 | 0.3539 | Moderate |
| 24 | FH | 0.8 | 0.8 | 1.1 | 0.8 | 0.8 | 0.8 | 0.8 | 1.05 | -0.3652 | 1.0083 | 0.3628 | Moderate |
| 25 | FH | 0.9 | 0.9 | 0.9 | 0.9 | 0.9 | 1.1 | 1.1 | 1.25 | 0.0797 | 0.9861 | 0.3474 | Moderate |
| 26 | FH | 0.8 | 0.8 | 0.9 | 0.8 | 0.9 | 1.1 | 1.0 | 1.2 | -0.2710 | 0.9861 | 0.3268 | Moderate |
| 27 | FH | 0.9 | 0.9 | 0.9 | 0.9 | 0.8 | 1.1 | 1.1 | 1.35 | 0.0200 | 1.1711 | 1.4708 | Moderate |
| 28 | FH | 0.95 | 0.95 | 1.15 | 1.08 | 1.0 | 1.1 | 1.0 | 1.3 | -0.0170 | 1.5435 | 0.3548 | Moderate |
| 29 | FH | 0.9 | 0.9 | 1.0 | 0.9 | 0.9 | 1.1 | 1.2 | 1.25 | 0.1132 | 1.4299 | 0.3727 | Moderate |
| 30 | FH | 0.9 | 0.9 | 0.9 | 0.9 | 0.9 | 1.1 | 1.2 | 1.2 | 0.2176 | 1.2533 | 0.3985 | Moderate |
| 31 | FH | 0.9 | 0.9 | 0.9 | 0.9 | 0.9 | 1.1 | 1.2 | 1.35 | 0.4302 | 1.2174 | 0.3668 | Moderate |
| 32 | FH | 0.9 | 0.9 | 0.9 | 0.9 | 0.9 | 1.1 | 1.3 | 1.4 | 0.3523 | 1.0616 | 0.3772 | Moderate |
| 33 | FH | 0.9 | 0.9 | 0.9 | 0.9 | 0.9 | 1.2 | 1.3 | 1.4 | 0.4928 | 1.2380 | 0.3728 | Moderate |
| 34 | FH | 0.9 | 0.9 | 0.9 | 0.9 | 0.9 | 1.3 | 1.4 | 1.5 | 0.4065 | 1.2939 | 0.3976 | Moderate |
| 35 | FH | 0.9 | 0.9 | 0.9 | 0.9 | 0.9 | 1.2 | 1.4 | 1.5 | 0.3354 | 1.2801 | 0.4054 | Moderate |
| 36 | FH | 0.9 | 0.9 | 0.9 | 0.9 | 0.8 | 1.4 | 1.4 | 1.6 | 0.5400 | 1.0472 | 0.3869 | Moderate |
| 37 | FH | 0.8 | 0.9 | 0.9 | 0.9 | 0.9 | 1.4 | 1.4 | 1.7 | 0.4238 | 0.6527 | 0.3899 | Moderate |

* **x (landing)**:  The landing position along the width of the table, with positive values indicating a landing on the right side of the table.
* **y (landing)**: The landing position along the depth of the table, with positive values indicating a landing on the opponent's side.
* **z (peak)**: The peak height of the ball during the trajectory.
* **Estimated Speed**: This is a subjective estimation based on the ball trajectory and the values of parameters a, b, c, d, e, f, g, and h. 

**Analysis**:

* **Parameter 'a' and 'b'**: These parameters influence the initial paddle position. While they are important, they don't directly affect the landing position along the x-axis (left/right).
* **Parameter 'c' and 'd'**: These parameters control the angle and strength of the initial paddle motion, respectively. A higher value of 'd' generally leads to a faster hit and a faster ball trajectory, possibly resulting in a wider landing position.
* **Parameter 'e' and 'f'**: These parameters control the angle and strength of the paddle motion during the contact point. A higher value of 'e' generally leads to a wider landing position on the table.
* **Parameter 'g' and 'h'**: These parameters control the angle and strength of the paddle motion during the follow-through. They have a smaller influence on the landing position compared to 'e' and 'f'.

## Step 2: Parameters Closest to the Objective

Based on the table, the following examples land the ball closest to the right side of the table:

* **Example 25:** a:0.9 b:0.9 c:0.9 d:0.9 e:0.9 f:1.1 g:1.1 h:1.25 - **x (landing) = 0.0797** 
* **Example 27:** a:0.9 b:0.9 c:0.9 d:0.9 e:0.8 f:1.1 g:1.1 h:1.35 - **x (landing) = 0.0200**
* **Example 29:** a:0.9 b:0.9 c:1.0 d:0.9 e:0.9 f:1.1 g:1.2 h:1.25 - **x (landing) = 0.1132**
* **Example 30:** a:0.9 b:0.9 c:0.9 d:0.9 e:0.9 f:1.1 g:1.2 h:1.2 - **x (landing) = 0.2176**
* **Example 31:** a:0.9 b:0.9 c:0.9 d:0.9 e:0.9 f:1.1 g:1.2 h:1.35 - **x (landing) = 0.4302**
* **Example 32:** a:0.9 b:0.9 c:0.9 d:0.9 e:0.9 f:1.1 g:1.3 h:1.4 - **x (landing) = 0.3523**
* **Example 33:** a:0.9 b:0.9 c:0.9 d:0.9 e:0.9 f:1.2 g:1.3 h:1.4 - **x (landing) = 0.4928**
* **Example 34:** a:0.9 b:0.9 c:0.9 d:0.9 e:0.9 f:1.3 g:1.4 h:1.5 - **x (landing) = 0.4065**
* **Example 35:** a:0.9 b:0.9 c:0.9 d:0.9 e:0.9 f:1.2 g:1.4 h:1.5 - **x (landing) = 0.3354**
* **Example 36:** a:0.9 b:0.9 c:0.9 d:0.9 e:0.8 f:1.4 g:1.4 h:1.6 - **x (landing) = 0.5400** 
* **Example 37:** a:0.8 b:0.9 c:0.9 d:0.9 e:0.9 f:1.4 g:1.4 h:1.7 - **x (landing) = 0.4238** 

## Step 3: Analyzing Parameter Effects

Based on the table and the previous analysis, the following observations can be made:

* **Parameter 'e'**: A higher value of 'e' generally leads to a wider landing position. This is evident in examples where 'e' is higher (e.g., examples 31, 33, 34, 35) and the ball lands closer to the right side.
* **Parameter 'f'**: While 'f' controls the strength of the paddle during contact, it doesn't seem to have a direct and significant impact on the landing position along the x-axis.
* **Parameter 'g' and 'h'**: These parameters seem to have a smaller influence on the landing position compared to 'e' and 'f'.

## Step 4: Proposed Parameter Values

Proposed params: a:0.9 b:0.9 c:0.9 d:0.9 e:1.2 f:1.1 g:1.3 h:1.5
Best strokestyle: FH 

<q> Hit the ball as far right as possible
## Step 1: Summary Table

| Example | Stroke | a | b | c | d | e | f | g | h | x (landing) |  y (landing) |  z (landing) |  On Table | Peak Height (z) | Estimated Speed |
|---|---|---|---|---|---|---|---|---|---|---|---|---|---|---|
| 1 | FH | 0.75 | 0.75 | 0.75 | 0.75 | 1.1 | 0.75 | 0.75 | 0.75 | -0.2978 | 0.4482 | 0.0089 | True | 0.4025 | Medium |
| 2 | FH | 0.9 | 0.9 | 0.9 | 0.9 | 0.8 | 0.9 | 0.9 | 0.9 | -0.2155 | 0.9221 | 0.0056 | True | 0.4211 | Medium |
| 3 | FH | 0.75 | 0.75 | 0.75 | 0.75 | 0.75 | 0.75 | 1.1 | 0.75 | -0.1632 | 0.4586 | -0.0168 | True | 0.4246 | Medium |
| 4 | FH | 0.87 | 0.87 | 0.87 | 0.87 | 0.87 | 0.87 | 0.87 | 1.23 | -0.0872 | 0.7329 | 0.0464 | True | 0.4128 | Medium |
| 5 | FH | 0.9 | 0.9 | 0.9 | 0.9 | 0.9 | 0.6 | 0.9 | 0.9 | -0.3773 | 1.2431 | 0.0208 | True | 0.4167 | Medium |
| 6 | FH | 0.9 | 0.9 | 0.9 | 0.9 | 0.9 | 1.1 | 0.9 | 0.9 | -0.1330 | 0.6830 | 0.0013 | True | 0.4210 | Medium |
| 7 | FH | 0.87 | 0.87 | 0.87 | 0.87 | 0.87 | 0.87 | 0.87 | 1.2 | -0.2439 | 0.7760 | 0.0533 | True | 0.4076 | Medium |
| 8 | FH | 0.8 | 0.8 | 1.1 | 0.8 | 0.8 | 0.8 | 0.8 | 0.8 | -0.1013 | 0.5102 | 0.0424 | True | 0.4134 | Medium |
| 9 | FH | 0.95 | 0.95 | 0.95 | 0.8 | 0.95 | 0.95 | 0.95 | 0.95 | -0.1778 | 1.2526 | -0.0383 | True | 0.4177 | Medium |
| 10 | FH | 0.9 | 0.9 | 0.9 | 0.9 | 0.9 | 0.8 | 0.9 | 0.9 | -0.1086 | 0.9854 | 0.0585 | True | 0.4154 | Medium |
| 11 | FH | 0.75 | 0.75 | 0.75 | 0.75 | 0.8 | 0.75 | 0.75 | 0.75 | -0.3085 | 0.3680 | 0.0325 | True | 0.4118 | Medium |
| 12 | FH | 0.9 | 0.9 | 0.9 | 0.9 | 1.1 | 0.9 | 0.9 | 0.9 | -0.2369 | 0.9637 | 0.0904 | True | 0.4156 | Medium |
| 13 | FH | 0.9 | 0.9 | 0.9 | 0.8 | 0.9 | 0.9 | 0.9 | 0.9 | -0.1976 | 1.3006 | 0.0735 | True | 0.4179 | Medium |
| 14 | FH | 0.8 | 0.8 | 1.1 | 0.8 | 0.8 | 0.8 | 0.8 | 1.05 | -0.1948 | 0.9218 | -0.0248 | True | 0.4150 | Medium |
| 15 | FH | 0.8 | 0.8 | 1.1 | 0.8 | 0.8 | 0.8 | 0.8 | 1.05 | -0.2249 | 1.1705 | 0.0667 | True | 0.4130 | Medium |
| 16 | FH | 0.8 | 0.8 | 1.1 | 0.8 | 0.8 | 0.8 | 0.8 | 1.05 | -0.3200 | 1.2490 | 0.0716 | True | 0.4142 | Medium |
| 17 | FH | 0.8 | 0.8 | 1.1 | 0.8 | 0.8 | 0.8 | 0.8 | 1.05 | -0.3083 | 0.8977 | -0.0202 | True | 0.4148 | Medium |
| 18 | FH | 0.8 | 0.8 | 1.1 | 0.8 | 0.8 | 0.8 | 0.8 | 1.05 | -0.2808 | 1.0771 | 0.0277 | True | 0.4154 | Medium |
| 19 | FH | 0.8 | 0.8 | 1.1 | 0.8 | 0.8 | 0.8 | 0.8 | 1.05 | -0.2340 | 0.7977 | 0.0434 | True | 0.4130 | Medium |
| 20 | FH | 0.8 | 0.8 | 1.1 | 0.8 | 0.8 | 0.8 | 0.8 | 1.05 | -0.2539 | 1.1478 | 0.0459 | True | 0.4142 | Medium |
| 21 | FH | 0.8 | 0.8 | 1.1 | 0.8 | 0.8 | 0.8 | 0.8 | 1.05 | -0.3401 | 0.8968 | 0.0296 | True | 0.4153 | Medium |
| 22 | FH | 0.8 | 0.8 | 1.1 | 0.8 | 0.8 | 0.8 | 0.8 | 1.05 | -0.3218 | 1.1070 | -0.0111 | True | 0.4131 | Medium |
| 23 | FH | 0.9 | 0.9 | 0.9 | 1.08 | 0.9 | 0.9 | 0.9 | 0.9 | -0.0617 | 0.7514 | -0.0206 | True | 0.3905 | Medium |
| 24 | FH | 0.8 | 0.8 | 1.1 | 0.8 | 0.8 | 0.8 | 0.8 | 1.05 | -0.3652 | 1.0083 | 0.0244 | True | 0.4138 | Medium |
| 25 | BH | 0.9 | 0.9 | 0.9 | 0.9 | 0.9 | 1.1 | 1.1 | 1.25 | 0.0797 | 0.9861 | -0.0120 | True | 0.4248 | Medium |
| 26 | BH | 0.9 | 0.9 | 0.9 | 0.9 | 0.9 | 1.1 | 1.1 | 1.25 | 0.0797 | 0.9861 | -0.0120 | True | 0.4248 | Medium |
| 27 | BH | 0.9 | 0.9 | 0.9 | 0.9 | 0.8 | 1.1 | 1.1 | 1.35 | 0.0200 | 1.1711 | -0.4000 | True | 0.3939 | Medium |
| 28 | BH | 0.95 | 0.95 | 1.15 | 1.08 | 1.0 | 1.1 | 1.0 | 1.3 | -0.0170 | 1.5435 | -0.0223 | False | 0.4246 | Medium |
| 29 | BH | 0.9 | 0.9 | 1.0 | 0.9 | 0.9 | 1.1 | 1.2 | 1.25 | 0.1132 | 1.4299 | -0.0298 | False | 0.4311 | Medium |
| 30 | BH | 0.9 | 0.9 | 0.9 | 0.9 | 0.9 | 1.1 | 1.2 | 1.2 | 0.2176 | 1.2533 | -0.0202 | True | 0.4262 | Medium |
| 31 | BH | 0.9 | 0.9 | 0.9 | 0.9 | 0.9 | 1.1 | 1.2 | 1.35 | 0.4302 | 1.2174 | -0.0298 | True | 0.4280 | Medium |
| 32 | BH | 0.9 | 0.9 | 0.9 | 0.9 | 0.9 | 1.1 | 1.3 | 1.4 | 0.3523 | 1.0616 | -0.0071 | True | 0.4296 | Medium |
| 33 | BH | 0.9 | 0.9 | 0.9 | 0.9 | 0.9 | 1.2 | 1.3 | 1.4 | 0.4928 | 1.2380 | 0.0181 | True | 0.4279 | Medium |
| 34 | BH | 0.9 | 0.9 | 0.9 | 0.9 | 0.9 | 1.3 | 1.4 | 1.5 | 0.4065 | 1.2939 | -0.0213 | True | 0.4324 | Medium |
| 35 | BH | 0.9 | 0.9 | 0.9 | 0.9 | 0.9 | 1.2 | 1.4 | 1.5 | 0.3354 | 1.2801 | -0.0272 | True | 0.4340 | Medium |
| 36 | BH | 0.9 | 0.9 | 0.9 | 0.9 | 0.8 | 1.4 | 1.4 | 1.6 | 0.5400 | 1.0472 | -0.0376 | True | 0.4381 | Medium |
| 37 | BH | 0.8 | 0.9 | 0.9 | 0.9 | 0.9 | 1.4 | 1.4 | 1.7 | 0.4238 | 0.6527 | -0.0138 | True | 0.4417 | Medium |
| 38 | BH | 0.9 | 0.9 | 0.9 | 0.9 | 1.2 | 1.1 | 1.3 | 1.5 | 0.4102 | 1.1394 | -0.0185 | True | 0.4206 | Medium |

 **Explanation of the table:**

* **Stroke:** Indicates whether the stroke is a forehand (FH) or backhand (BH).
* **a, b, c, d, e, f, g, h:** These parameters control the robot's movements and ball trajectory. 
* **x (landing), y (landing), z (landing):**  These are the coordinates of the ball's landing position. 
* **On Table:**  Indicates if the ball landed on the table (True) or went off the table (False).
* **Peak Height (z):** The maximum height reached by the ball during its trajectory.
* **Estimated Speed:** A subjective estimate of the ball's speed, based on the trajectory and landing position.  "Medium" indicates a speed that is neither very slow nor very fast.

## Step 2: Parameters closest to the objective

The examples with the most positive x values (landing furthest to the right) are: 

* **Example 36:** x = 0.5400 (BH)
* **Example 33:** x = 0.4928 (BH)
* **Example 34:** x = 0.4065 (BH)

Therefore, these examples are the closest to fulfilling the objective of hitting the ball as far right as possible. All of these examples are backhand strokes.

## Step 3: Analysis of parameter effects

**a, b, c, d:** These parameters mostly affect the initial position and direction of the paddle.  They do not have a strong direct influence on the landing position, especially in the x-dimension.

**e:** This parameter influences the speed of the paddle swing.  A higher "e" value generally results in a faster swing and, consequently, a faster ball. This, in turn, can affect the x-dimension landing position.

**f:** This parameter controls the "lift" of the ball.  A higher "f" value generally results in a higher arc for the ball's trajectory, and can affect the landing position in both x and y dimensions.

**g:** This parameter is primarily responsible for the "spin" applied to the ball. A higher "g" value will result in more topspin. This can affect both the x and y landing position, as topspin causes the ball to curve downwards and can potentially alter the ball's path in the x-direction. 

**h:**  This parameter seems to be the most influential on the x-dimension landing position.  A higher "h" value typically results in the ball landing further to the right. This suggests "h" might be related to the paddle's angle or a specific motion that pushes the ball towards the right.

## Step 4: Proposed parameters

Proposed params: a:0.9 b:0.9 c:0.9 d:0.9 e:1.2 f:1.1 g:1.3 h:1.7
Best strokestyle: BH

**Explanation of the proposed parameters:**

* **a, b, c, d:** These are set to 0.9 for consistency, as they do not appear to have a significant effect on the x-dimension landing position. 
* **e:**  Increased to 1.2 for a slightly faster swing, potentially impacting the landing position.
* **f:**  Increased to 1.1 for a slightly higher arc, which might help with controlling the ball's trajectory.
* **g:**  Increased to 1.3 to increase topspin, aiming to potentially influence the ball's x-dimension curve.
* **h:**  Increased to 1.7 to further enhance the ball's rightward movement, based on its significant impact observed in the previous examples.

The proposed parameters are based on the analysis of the previous examples and aim to improve upon the existing results while avoiding hitting the ball off the table.  This combination of parameters leverages the strengths of the previous successful examples, with a focus on maximizing the "h" parameter for a potentially wider x-dimension landing position.
